# Supplementary material for: StartLux-Decision: AutoThink Decision Models with Reinforcement Learning for Calibrated Deliberative Decisions
Source: arXiv:2610.17309 source file (2026-10-20)
Supplement: Supplementary file 1 [file appendix_A_proofs.tex]

\mdBibliography
\clearpage
\appendix
\section{Propositions and proofs}\label{sec:A}

This appendix gives the formal statements behind Chapter~\ref{sec:7}: the setting and notation, five
propositions with their proofs, the checks of their assumptions in our data, the predictions they
make, and a simulation that reproduces the effect and both remedies. Section~\ref{sec:7.1} states
the rule in words.

\subsection{Setting and notation}\label{sec:A.1}

\textbf{Typed decisions.} A question is a choice, a yes/no question or an ordinal score over a
state. The model returns a distribution over the options, in one pass or after its own reasoning.
Its \emph{confidence} is the probability of the option it returns.

\textbf{Policies.} Four policies spend extra computation where a confidence says it is needed.

\begin{itemize}
\item \emph{Think-gate.} Reason if and only if the plain confidence c0 is below a threshold $\tau$, and
report the thought answer with its confidence c1. Otherwise report the plain answer with c0.
\item \emph{Cascade.} Escalate if and only if the small model's confidence is below $\tau$, and report the
large model's answer with the large model's confidence.
\item \emph{Best-of-N.} Draw N responses, return the one to which a verifier gives the highest probability
of being correct, and report that probability.
\item \emph{Select-then-think.} Best-of-N, after which the verifier reasons about its k favourites.
\end{itemize}

\textbf{Two calibrations.} \emph{Marginal} calibration, which Chapter~\ref{sec:7} calls the usual
calibration, is what a calibration set gives by default: all thought answers, all answers of the
large model, single judged responses. \emph{Per-policy} calibration uses the answers that the
deployed policy returns on the calibration problems: the winners of the selection, the answers that
took the route.

\textbf{Notation.} x is an item and y its correct option. p0 is the plain readout of the model (one
forward pass, also called the fast readout) and p1 the readout after reasoning (the thought
readout). c(p) is the largest probability of a readout, its confidence, and a(p) the option that has
it. For selection among samples, a problem has a latent easiness $\theta$ with density p($\theta$).
Given $\theta$ its N responses are independent pairs ($Y_{i}$, $S_{i}$) of correctness and verifier
score, with score density f(s \textbar{} $\theta$) and distribution function F(s \textbar{}
$\theta$). We write m(s \textbar{} $\theta$) = P(Y = 1 \textbar{} S = s, $\theta$), and m(s) =
E{[}m(s \textbar{} $\theta$) \textbar{} S = s{]} for the calibration curve of single responses. The
system returns the response I{*} with the highest score.

\subsection{Proposition 1: selection by the reported score}\label{sec:A.2}

\textbf{Proposition 1.} Suppose (i) m(s \textbar{} $\theta$) is non-decreasing in $\theta$, and (ii)
F(s \textbar{} $\theta$) is non-increasing in $\theta$ for every s. Then $a_{N}(s)$ = P($Y_{I*}$ = 1
\textbar{} $S_{I*}$ = s) is non-increasing in N, and $a_{1}(s)$ = m(s).

\emph{In words.} Let a problem have a latent easiness, and let its N responses be independent draws
of a correctness and a verifier score given that easiness. Suppose (i) at the same score, responses
to easier problems are right at least as often, and (ii) easier problems score higher (their score
distribution dominates). Then the accuracy of the returned response at a given score, $a_{N}(s)$, is
non-increasing in N, and $a_{1}(s)$ is the calibration curve of single responses. In particular, a
verifier that is calibrated on single responses is overconfident on its selected responses at every
score and for every N \textgreater{} 1, unless (i) or (ii) holds with equality.

\emph{Proof.} Given $\theta$, the event \{$S_{I*}$ = s\} has density N f(s \textbar{} $\theta$) F(s
\textbar{} $\theta$)$^{(N-1)}$, and given this event and $\theta$ the returned response is right
with probability m(s \textbar{} $\theta$), because the other N $-$ 1 responses are independent of it
given $\theta$. Hence $a_{N}(s)$ = $\int$ m(s \textbar{} $\theta$) $w_{N}(\theta )$ d$\theta$ with
weights $w_{N}(\theta )$ $\propto$ p($\theta$) f(s \textbar{} $\theta$) F(s \textbar{}
$\theta$)$^{(N-1)}$. Going from N to N + 1 multiplies the weights by F(s \textbar{} $\theta$), which
is non-increasing in $\theta$ by (ii), so $w_{N+1}$ is smaller than $w_{N}$ in the monotone
likelihood ratio order, and the expectation of the non-decreasing function m(s \textbar{}
\textperiodcentered{}) cannot rise. $\blacksquare$

\emph{Reading.} The winner has score s. Its N $-$ 1 rivals all scored lower. The more rivals fell
below s, the more likely the problem is one on which scores run low, a hard one, and on a hard
problem a response with score s is right less often. The losing candidates are data about the
problem, and a confidence calibrated on single responses has not seen them.

\emph{Checks of the assumptions.} We estimated easiness for each response from the verifier's mean
score on the other responses of its problem. At a 9B verifier score of .8--.9 a response is right
75.6 / 93.4 / 98.3\% of the time on problems of low / middle / high easiness (27B verifier: 69.4 /
81.0 / 90.5), and the share of scores below .9 is 97.4 / 70.3 / 25.7\%. Assumption (i) fails only in
the lowest score bin of a fine-tuned verifier, which selection never returns.

\subsection{Proposition 2: routing by a second score}\label{sec:A.3}

\textbf{Proposition 2.} Let G = \{c(p0) \textless{} t\} be the routed set and let ``correct'' mean y
= a(p1). For every q with P(G \textbar{} c(p1) = q) \textgreater{} 0,

P(correct \textbar{} c(p1) = q, G) $-$ P(correct \textbar{} c(p1) = q) = P(correct \textbar{} c(p1)
= q) \textperiodcentered{} {[}P(G \textbar{} correct, c(p1) = q) $-$ P(G \textbar{} c(p1) = q){]} /
P(G \textbar{} c(p1) = q).

If P(correct \textbar{} c(p1) = q, c(p0)) is non-decreasing in c(p0), then P(correct \textbar{}
c(p1) = q, G) $\leq$ P(correct \textbar{} c(p1) = q) $\leq$ P(correct \textbar{} c(p1) = q, not G).
With a non-increasing dependence the inequalities reverse. In particular, if p1 is calibrated on all
items, it is calibrated on the routed items if and only if the correctness of the reported answer is
conditionally independent of the route given c(p1).

\emph{In words.} Let a gate route the items with c0 below a threshold and let the system report an
answer with confidence c1. If, at a given c1, the probability that the reported answer is correct is
non-decreasing in c0, then at that c1 the routed items are less accurate than the kept ones. If it
is non-increasing, they are more accurate. The size of the gap is given by Bayes' rule: accuracy on
the routed items at confidence q, minus accuracy on all items at q, equals the accuracy at q times
{[}P(routed \textbar{} correct, q) $-$ P(routed \textbar{} q){]} / P(routed \textbar{} q).

\emph{Proof.} The identity is Bayes' rule on the event G at fixed c(p1) = q. For the inequalities,
the two conditional accuracies are averages of the same non-decreasing function of c(p0) over
\{c(p0) \textless{} t\} and over \{c(p0) $\geq$ t\}. $\blacksquare$

\textbf{The residual AUROC.} The premise can be measured without choosing a threshold, as the AUROC
of c(p0) for the correctness of the reported answer within quintiles of c(p1). We call it the
\emph{residual AUROC}. At 0.5 the reported confidence already contains what the routing confidence
knows. Above 0.5 the routed answers are overconfident relative to the kept ones, and below 0.5 the
reverse. Across 36 pairs of a model and an item set it predicts the size and the sign of the route
effect (Spearman $-$0.88 {[}$-$0.92, $-$0.77{]}, same sign in 31 of 36). The same statement holds
for a cascade, with the small model's confidence as c(p0) and the large model's readout as p1.

\subsection{Proposition 3: a certificate for the mixture is silent about the route}\label{sec:A.4}

\textbf{Proposition 3.} A system reports p0 on kept items and p1 on routed items and accepts an
answer if and only if its confidence C is at least $\lambda$. Let e = P(wrong \textbar{} C $\geq$
$\lambda$), $e_{r}$ = P(wrong \textbar{} C $\geq$ $\lambda$, route r) and $w_{r}$ = P(route r
\textbar{} C $\geq$ $\lambda$). Then e = $w_{\mathrm{plain}}$ $e_{\mathrm{plain}}$ +
$w_{\mathrm{thought}}$ $e_{\mathrm{thought}}$. A certificate e $\leq$ $\alpha$ therefore bounds
$e_{\mathrm{thought}}$ only by ($\alpha$ $-$ $w_{\mathrm{plain}}$ $e_{\mathrm{plain}}$) /
$w_{\mathrm{thought}}$, which exceeds $\alpha$ whenever $e_{\mathrm{plain}}$ \textless{} $\alpha$.
If P(correct \textbar{} C = c, thought) \textless{} P(correct \textbar{} C = c, plain) for all c
$\geq$ $\lambda$, then $e_{\mathrm{thought}}$ \textgreater{} $e_{\mathrm{plain}}$, and a certificate
that is tight (e = $\alpha$) has $e_{\mathrm{thought}}$ \textgreater{} $\alpha$ \textgreater{}
$e_{\mathrm{plain}}$. Thresholds certified per route bound $e_{r}$ $\leq$ $\alpha$ for each route,
hence e $\leq$ $\alpha$.

\emph{Proof.} The law of total probability on \{C $\geq$ $\lambda$\}. The second claim integrates
the pointwise inequality over c $\geq$ $\lambda$. $\blacksquare$

\subsection{Proposition 4: calibration on the policy's statistics}\label{sec:A.5}

\textbf{Proposition 4.} Let T be a statistic of an item and of the computation done on it (scores of
candidates, their number, a routing confidence), and let a confidence q for the returned answer
satisfy P(correct \textbar{} q, T) = q. Then for every policy whose decision to return this answer
is a function of T, the answers it returns are calibrated: P(correct \textbar{} q, returned) = q.

\emph{Proof.} The event ``returned'' is determined by T, so P(correct \textbar{} q, returned) =
E{[}P(correct \textbar{} q, T) \textbar{} q, returned{]} = q by the tower property. $\blacksquare$

Marginal calibration is the case in which T is empty. The policy-aware map of Section~\ref{sec:7.5}
estimates P(correct \textbar{} reported confidence, T) from the policy's outputs on calibration
problems. Propositions 1 and 2 are the converse in the two cases studied: when T is left out and is
informative about correctness given the reported confidence, the returned answers are not
calibrated.

\subsection{Proposition 5: the objective of a gated system}\label{sec:A.6}

A system that reasons only sometimes is scored on what it reports: with probability g(x) the thought
distribution p1, at a cost c, and otherwise the plain distribution p0.

\textbf{Proposition 5.} Let S be a proper score, p0(x) the plain distribution, p1(x, $\tau$) the
distribution after a trace $\tau$ \textasciitilde{} $\pi$(\textperiodcentered{} \textbar{} x) of
cost c($\tau$), and g(x) $\in$ {[}0, 1{]} the probability of reasoning, and let

J = E{[}(1 $-$ g(x)) S(p0(x), y) + g(x) (S(p1(x, $\tau$), y) $-$ c($\tau$)){]}.

(a) For fixed p0, p1 and $\pi$, J is linear in g, with $\partial$J/$\partial$g(x) = v(x) = E{[}S(p1,
y) $-$ c \textbar{} x{]} $-$ E{[}S(p0, y) \textbar{} x{]}. The gate g{*}(x) = 1\{v(x) \textgreater{}
0\} maximises J. (b) For a fixed gate and $\pi$ and a strictly proper S, among thought readouts that
are functions of a statistic $\phi$(x, $\tau$), J is maximised by the conditional distribution of y
given $\phi$ under the measure that weights each item by g(x). It coincides with the conditional
distribution fitted on all items if and only if y is independent of the route given $\phi$. (c)
$\nabla$\_$\pi$ J = E{[}g(x) (S(p1, y) $-$ c) $\nabla$ log $\pi$($\tau$ \textbar{} x){]}.

\emph{Proof.} (a) J is affine in g(x) at every x. (b) Strict propriety under the g-weighted measure.
The two conditional distributions agree exactly when the weighting does not change the law of y
given $\phi$. (c) The score-function identity. $\blacksquare$

In this proposition $\tau$ denotes a reasoning trace, not the routing threshold of A.1.

\emph{Training target of the gate.} If a training target for the gate is P(yes) = A / (A + B), with
A and B the expected positive and negative parts of the realised value S(p1, y) $-$ c $-$ S(p0, y),
then P(yes) \textgreater{} 1/2 if and only if v(x) \textgreater{} 0, for every cost.

\emph{Reading.} Three facts follow. First, J is linear in the gate, and its derivative at an item is
the value of computation v(x). The optimal gate reasons exactly where v is positive. Both terms can
be computed for every training item, so the gate is learned from exact labels, without sampling its
own decisions. Second, the best confidence for the thought answer is the posterior on the items the
gate routes, not on all items: the population on which Chapter~\ref{sec:7} certifies and calibrates.
Third, only the reasoning itself has a sampled gradient. The value gate of Appendix~\ref{sec:B} is
built on (a).

\subsection{What the propositions predict}\label{sec:A.7}

Propositions 1 and 2 make four predictions, which Chapter~\ref{sec:7} and Appendix~\ref{sec:B} test.

\begin{enumerate}
\item The confidence of a selected response is optimistic, more so with more candidates and with a weaker
verifier.
\item The confidence reported after a route depends on the route, with the sign and size of the residual
AUROC, including a reversal where a low plain confidence marks the items that reasoning solves.
\item A threshold certified on the marginal population does not bound the error of the answers a policy
returns.
\item The remedies are the ones the propositions point to: calibrate on the population the policy returns,
give the calibration map what the losers know, or route on a score whose residual AUROC is 0.5.
\end{enumerate}

\subsection{A simulation of Proposition 1 and of the recipe}\label{sec:A.8}

The reference implementation of the recipe of Section~\ref{sec:7.5} (about 150 lines of numpy: the
selection map, the route map and the certificate) carries a simulation that reproduces the effect
and both remedies in a few seconds. Problems have an easiness $\theta$ \textasciitilde{} N($-$0.5,
2). A response is right with probability $\sigma$($\theta$). The verifier sees a noisy signal of the
correctness of a response and nothing of $\theta$, and its score is calibrated on single responses.
\todo{where the reference implementation is published}

\begin{table}[!htbp]
\renewcommand{\thetable}{A.1}
\centering
\caption{In simulation the selected response grows overconfident with N under single-response calibration and stays near calibrated under the set-aware map. Simulated best-of-N selection: accuracy of the selected response and its overconfidence (mean reported confidence minus accuracy, in points) under calibration on single responses and under the set-aware map fitted at N = 1, 4 and 16. Simulation only. No model is involved.}\label{tab:A.1}
{\small\setlength{\tabcolsep}{6pt}\renewcommand{\arraystretch}{1.1}
\noindent\begin{adjustbox}{max width=\linewidth}
\begin{tabular}{rrrr}
\toprule
\textbf{N} & {\begin{tabular}[b]{@{}r@{}}\textbf{accuracy of}\\\textbf{the selected}\\\textbf{response}\end{tabular}} & {\begin{tabular}[b]{@{}r@{}}\textbf{overconfidence,}\\\textbf{single-response}\\\textbf{calibration}\end{tabular}} & {\begin{tabular}[b]{@{}r@{}}\textbf{overconfidence,}\\\textbf{set-aware map fitted}\\\textbf{at N = 1, 4, 16}\end{tabular}} \\
\midrule
1 & 42.5 & $-$0.2 & +0.5 \\
2 & 54.1 & +4.7 & $-$0.3 \\
4 & 63.9 & +9.4 & $-$0.7 \\
8 & 71.8 & +12.0 & $-$0.5 \\
16 & 77.5 & +13.0 & $-$0.0 \\
32 & 82.1 & +12.3 & +0.0 \\
64 & 86.3 & +10.4 & $-$0.3 \\
\bottomrule
\end{tabular}
\end{adjustbox}\par}
\end{table}

In the same simulation a threshold certified for 5\% error on single responses accepts 79.7\% of the
best-of-32 answers at 6.9\% error. Certified on the policy's own answers it accepts 68.7\% at 4.2\%.
