# Supplementary material for: StartLux-Decision: AutoThink Decision Models with Reinforcement Learning for Calibrated Deliberative Decisions
Source: arXiv:2610.17309 source file (2026-10-20)
Supplement: Supplementary file 2 [file appendix_B_policy_calibration.tex]

\section{Policy-aware calibration: details}\label{sec:B}

Chapter~\ref{sec:7} states the rule and the recipe, and this appendix holds the evidence behind
them. Propositions 1 to 5 are in Appendix~\ref{sec:A} (A.2 to A.6). All numbers come from our own
runs, with models of other teams run by us from their public weights and code, except the public
records of another group's system described below.

\subsection{Policies and protocols}\label{sec:B.1}

\textbf{Policies.} A \emph{think-gate} reasons exactly when the one-pass (``plain'') confidence c0
is below a threshold, and then reports the answer after reasoning with its confidence c1, otherwise
the plain answer with c0. At a think rate of 30\% the least confident 30\% of the items are
\emph{routed} to reasoning and the rest are \emph{kept}. A \emph{cascade} escalates exactly when the
small model's confidence is below a threshold, and reports the large model's answer and confidence.
\emph{Best-of-N} draws N responses, lets a verifier (a decision model asked whether a response is
correct) score each, and returns the best-scored response with that score as its confidence.
\emph{Select-then-think} is best-of-N after which the verifier reasons about its three favourites,
and the answers that follow this reasoning are its thought answers. The select-then-think maps of
Section~\ref{sec:B.5} were fitted on runs in which the verifier reasoned about the three favourites
of every problem. The certificates of Table~\ref{tab:B.3} come from runs in which it reasoned only
on the half of the problems on which the best one-pass score among the candidates was lowest (a
think rate of 50\%), and the other half kept the one-pass winner with its one-pass score.

\textbf{Systems and problems.} The verifiers were the released StartLux-Decision 4B, 9B and 27B, two
decision models of another team (Clef 27B, Clef-flash 9B) and four chat models (Phi-4-mini-instruct,
Gemma-3-4b-it, Gemma-3-12b-it, Phi-4), with generators of 0.8B, 2B and 4B of ours and the same chat
models. Best-of-N ran on the held-out problems (arithmetic), the arithmetic problems of five unseen
datasets (5,761 problems, among them MAWPS and GSM-Hard), reasoning sets and closed-book question
answering (8,000 questions). The gates were run on twelve models: our 4B and 9B, the four chat
models with zero-shot chain of thought, two reasoning models (DeepSeek-R1-Distill-Llama-8B, called
R1-distill, and Phi-4-mini-reasoning), Jeeves-9B (another team's decision model with a built-in
think gate) and three controls (our two base models and Granite-3.3-2b). They were evaluated on the
\emph{decision suite} (5,710 diagnostic decisions of 39 task families, 150 per family except the 10
of SimpleBench, of the type of the Decision Index benchmarks and not held-out), on 4,648 reasoning
decisions and on CJ-Bench, a third-party benchmark of 304,822 hard decisions in Chinese.

\textbf{Checkpoints, problem sets and sampling.} The generators of ours were the instruction-tuned
Qwen3.5-0.8B, Qwen3.5-2B and Qwen3.5-4B. The 4B and 9B that reasoned, as think-gates and as
select-then-think verifiers, were the released StartLux-Decision-4B and StartLux-Decision-9B, each
after a reader round that trains a model to read its own thoughts. Their thought budget was 4,096
tokens on the decision suite, 1,024 on CJ-Bench and 256 as select-then-think verifiers. The held-out
problems were 1,550 variants of 801 problems of the GSM8K training split, with changed numbers and
recomputed answers, so the StartLux-Decision models had trained on the original problems but not on
the variants, and the sources are disjoint from the problems used for reinforcement learning and
verifier tuning. The unseen datasets were SVAMP (1,000 problems), ASDiv (1,200), GSM-Hard (1,162),
GSM-Plus (1,199) and MAWPS (1,200). The 5,988 problems of the reasoning sets came from BIG-Bench
Hard (2,700), StrategyQA (687), FOLIO (203), ProofWriter (1,198) and DROP (1,200) with numbered
options, so that every answer is a number, and the 4,648 reasoning decisions of the gates were posed
from the BIG-Bench Hard, StrategyQA, FOLIO and ProofWriter problems among them. Generators were
sampled at temperature 1 with thinking off and at most 400 new tokens on the arithmetic problems and
1,024 on the reasoning sets, and they drew 64 responses per held-out problem, 32 per problem of the
unseen datasets and 16 per problem of the reasoning sets, and 256 for the larger runs on the first
two. \todo{mark which of the 39 families have training data in the mix of each model.}

\textbf{Measures.} \emph{Overconfidence} is the mean reported confidence of the returned answers
minus their accuracy, in points, after the \emph{usual calibration} (an isotonic map fitted on
single judged responses). The \emph{route effect} is the accuracy of the reported answer at matched
reported confidence, routed minus kept (negative: routed answers are overconfident). The
\emph{residual AUROC} is the AUROC of the routing confidence for the correctness of the reported
answer within quintiles of the reported confidence (0.5: nothing is left). Confidence is matched in
five bins of equal width on the confidence after reasoning: each bin with at least 30 routed and 30
kept answers contributes the accuracy of the routed answers minus that of the kept answers, weighted
by the smaller of the two counts, and both groups are compared on their answers after reasoning,
which the stored runs hold for every item. The intervals of the route effect are 95\% percentile
intervals of a bootstrap over items with 500 resamples (300 on CJ-Bench). A certificate is a
threshold on the reported confidence, above which answers are accepted without review, certified for
error $\leq$ $\alpha$ on a calibration half of the problems (fixed-sequence Clopper--Pearson test at
95\%) and applied to the answers on the other half, over 20 splits by source problem. Best-of-N
intervals are 95\% cluster bootstrap intervals over source problems.

\subsection{Selection among samples}\label{sec:B.2}

The response a verifier selects is overconfident after the usual calibration in 111 of the 113 pairs
of a generator and a verifier at N = 16 (Figure~\ref{fig:B.1}a). The gap grows with N in all 126
runs (Proposition 1) and is larger the weaker the verifier (Table~\ref{tab:B.1}).

\begin{table}[!htbp]
\renewcommand{\thetable}{B.1}
\centering
\caption{For every verifier but one saturated judge the selected response is overconfident after calibration on single responses, and more so with more candidates. Accuracy of best-of-N with a 2B generator (\%) and overconfidence of the selected response after calibration on single responses (points), by verifier. Best accuracy per column in bold.}\label{tab:B.1}
{\small\setlength{\tabcolsep}{6pt}\renewcommand{\arraystretch}{1.1}
\noindent\begin{adjustbox}{max width=\linewidth}
\begin{tabular}{lrrrr}
\toprule
\textbf{verifier} & {\begin{tabular}[b]{@{}r@{}}\textbf{held-out,}\\\textbf{best-of-64}\end{tabular}} & {\begin{tabular}[b]{@{}r@{}}\textbf{unseen}\\\textbf{datasets,}\\\textbf{best-of-32}\end{tabular}} & {\begin{tabular}[b]{@{}r@{}}\textbf{reasoning}\\\textbf{sets,}\\\textbf{best-of-16}\end{tabular}} & {\begin{tabular}[b]{@{}r@{}}\textbf{overconfidence,}\\\textbf{held-out, N = 4 $\rightarrow$ 64}\end{tabular}} \\
\midrule
\mdourrow StartLux-Decision-4B & 92.52 & 82.07 & 77.32 & +1.6 $\rightarrow$ +3.8 \\
\mdourrow StartLux-Decision-9B & 94.19 & 83.34 & 78.02 & +1.5 $\rightarrow$ +2.9 \\
\mdourrow StartLux-Decision-27B & \textbf{95.48} & \textbf{86.04} & \textbf{82.97} & +0.5 $\rightarrow$ +1.4 \\
Clef 27B (another team) & 93.01 & 83.13 & 77.01 & +1.0 $\rightarrow$ +3.5 \\
Phi-4-mini-instruct (chat model) & 83.17 & 74.16 & 66.45 & +4.3 $\rightarrow$ +11.4 \\
Phi-4 (14B, chat model) & 90.57 & 78.44 & -- & $-$1.9 $\rightarrow$ $-$0.5 (saturated score) \\
\bottomrule
\end{tabular}
\end{adjustbox}\par}
\end{table}

\begin{figure}[!htbp]
\renewcommand{\thefigure}{B.1}
\centering
\adjincludegraphics[max width=\linewidth,max height=0.5\textheight]{figures/fig4_grid.pdf}
\caption{The selection effect appears in nearly every run at N = 16, and a threshold certified on single responses breaks its level in most pairs. (a) Overconfidence of the selected response against the verifier's within-problem AUROC on single responses. (b) Error of the accepted answers at $\alpha$ = .05 for a threshold certified on single responses (horizontal) and under the same best-of-16 policy (vertical), for the 67 pairs that accept at least 5\% of the answers. Dashed lines: the level.}\label{fig:B.1}
\end{figure}

The two exceptions are the judge Phi-4 with two generators on the held-out problems. It puts 59\% of
the responses above .9999 and almost all others below .5, so it approves or rejects and does not
rank, and its accuracy at the top score does not depend on N (90.6\% at N = 1, 91.1\% at N = 4, 16
and 64). On the unseen datasets it shows the effect (+2.6 $\rightarrow$ +7.5).

A weaker verifier can also lose accuracy as N grows: on one unseen dataset our 4B verifier loses 6.0
points {[}$-$7.4, $-$4.6{]} from N = 8 to 256 (85.2 $\rightarrow$ 79.2) while the 27B gains 1.7
{[}+0.7, +2.8{]} on the same samples. At equal size our 4B is 8 to 11 points above
Phi-4-mini-instruct as judge, and it is also above Phi-4 (14B). Our 27B is ahead of Clef 27B by +2.5
{[}+1.6, +3.4{]} and +2.9 {[}+2.3, +3.5{]} points on the held-out and unseen sets and by 6.0 points
on the reasoning sets. In closed-book question answering, where the verifier lacks the facts,
best-of-16 is 0.1--2.7 points above the vote with the 4B generator and 0.9--2.3 points below it with
Phi-4 as generator, and the selection effect is largest (+6.9 to +17.5 points).

\subsection{Think-gates and cascades}\label{sec:B.3}

At equal reported confidence, an answer reasoned about because the plain confidence was low is less
accurate than a kept answer, for eleven of twelve models on the decision suite and for every model
we ran on CJ-Bench (Table~\ref{tab:B.2}). Ten cascades of a small and a large model have the same
sign ($-$.10 to $-$.17).

\begin{table}[!htbp]
\renewcommand{\thetable}{B.2}
\centering
\caption{After a think-gate, routed answers are less accurate than kept ones at equal reported confidence for most models, and on reasoning items the sign reverses. Route effect: accuracy at matched reported confidence, routed minus kept, with 95\% intervals where computed. Negative: routed answers are overconfident.}\label{tab:B.2}
{\footnotesize\setlength{\tabcolsep}{5pt}\renewcommand{\arraystretch}{1.1}
\noindent\begin{adjustbox}{max width=\linewidth}
\begin{tabular}{>{\raggedright\arraybackslash}p{\mdw{0.3309}}>{\raggedright\arraybackslash}p{\mdw{0.2558}}>{\raggedright\arraybackslash}p{\mdw{0.3992}}}
\toprule
\textbf{models} & \textbf{policy, think rate, items} & \textbf{routed minus kept {[}95\%{]}} \\
\midrule
\mdourrow StartLux-Decision 4B / 9B & think-gate, 30\%, decision suite & $-$.194 {[}$-$.230, $-$.158{]} / $-$.214 {[}$-$.254, $-$.171{]} \\
Phi-4 (14B) / Gemma-3-4b, zero-shot chain of thought & think-gate, 30\%, decision suite & $-$.176 {[}$-$.203, $-$.149{]} / $-$.028 {[}$-$.057, .000{]} \\
Jeeves-9B (another team) & think-gate, 30\%, decision suite & $-$.037 {[}$-$.071, $-$.006{]} \\
\mdourrow StartLux-Decision-4B & think-gate, 10\% / 20\% / 40\%, CJ-Bench & $-$.114 {[}$-$.122, $-$.108{]} / $-$.163 {[}$-$.168, $-$.156{]} / $-$.241 {[}$-$.245, $-$.236{]} \\
\mdourrow StartLux-Decision-4B, Jeeves-9B & think-gate, 30\% / 50\%, reasoning items & +.057 / +.021, +.032 / +.025 (reversed) \\
\bottomrule
\end{tabular}
\end{adjustbox}\par}
\end{table}

The route effect follows the residual AUROC (Proposition 2). On the decision suite the residual
AUROC is .69 and .64 for our 9B and 4B (route effects $-$.214 and $-$.194) and .49--.50 for three
models ($-$.038 \ldots{} +.021). One line fits all three item sets (Figure~\ref{fig:B.2}: Spearman
$-$0.88 {[}$-$0.92, $-$0.77{]} over 36 pairs of a model and an item set, same sign in 31 of 36), and
the cascades lie on average .04 above it.

\begin{figure}[!htbp]
\renewcommand{\thefigure}{B.2}
\centering
\adjincludegraphics[max width=\linewidth,max height=0.5\textheight]{figures/fig6_gate_info.pdf}
\caption{The residual AUROC of the routing confidence predicts the size and the sign of the route effect. Horizontal: residual AUROC of the routing confidence for the correctness of the thought answer, given the thought confidence (0.5 = nothing left). Vertical: accuracy of thought answers at matched thought confidence, routed minus kept. One point per model and item set, triangles are cascades.}\label{fig:B.2}
\end{figure}

Training on decision data makes the effect larger. The base models that ours are tuned from show
little of it on the decision suite ($-$.069 for the base 9B, +.021 for the base 4B, against $-$.214
and $-$.194), because training sharpens the plain confidence and the thought confidence does not
absorb what the plain one now knows. A reader round, the stage that teaches a model to read its own
reasoning and state a probability, narrows the gap between the routes but leaves a route effect of
$-$.14 to $-$.19.

The sign is not universal. On the reasoning items a low plain confidence marks items that thinking
solves: the residual AUROC is below .5 for five models (our 4B .39, Jeeves .37, R1-distill .43, the
two base models .36 and .41), whose routed answers are the more accurate ones, and above .5 for four
others (.55--.58), which stay negative. Thinking lifts our 4B from 59.6\% to 86.5\%, so the kept
items carry the residual errors.

One decision model has almost none of the effect: the thought confidence of Jeeves-9B absorbs most
of what its plain confidence knows (residual AUROC .56 on the decision suite). Its reasoning was
trained by reinforcement learning with the probability of the correct option after thinking as
reward, which suggests that the route-dependence comes from how that confidence was trained. We ran
no ablation of another team's model, and in our closest experiment (a two-model baseline whose
separate reasoner we trained by reinforcement learning, Section~\ref{sec:5.5}) the route effect
stays where it was ($-$.279 {[}$-$.311, $-$.248{]} before, $-$.272 {[}$-$.302, $-$.243{]} after 100
iterations).

The gates above report the thought distribution alone, whereas the gate of the released models
(Section~\ref{sec:2.2}) reports the equal mixture of the plain and the thought distribution. On
3,021 held-out routed items the plain readout is underconfident ($-$3.5 to $-$7.1 points) and the
readout after the thought overconfident (+5.1 to +9.3) for four 4B training designs, and the mixture
lands within $-$0.7 to $-$2.7 because the two cancel. It ranks badly although it is more accurate
than the readout after the thought (75.4\% against 74.7\%): for the 4B trained to end its thoughts
where they are finished, 5\% of its routed answers can be accepted at 5\% error, against 21\% after
the thought.

\subsection{Certificates per policy}\label{sec:B.4}

A threshold certified on the usual calibration data is exceeded by the answers a policy acts on, and
a threshold certified on the policy's own answers is not (Table~\ref{tab:B.3}). For gates the reason
is Proposition 3: the error of all accepted answers is the weighted mean of the errors of the
routes, and the kept answers are many and safe, so a certificate for all answers is silent about the
thought answers, which are accepted at several times the level.

\begin{table}[!htbp]
\renewcommand{\thetable}{B.3}
\centering
\caption{A threshold certified on the usual calibration data is exceeded by the answers a policy returns, and one certified on the policy's own answers is not. Error of the accepted answers (and splits above the level $\alpha$) for a threshold certified on the usual calibration data and on the answers of the same policy or route.}\label{tab:B.3}
{\footnotesize\setlength{\tabcolsep}{5pt}\renewcommand{\arraystretch}{1.1}
\noindent\begin{adjustbox}{max width=\linewidth}
\begin{tabular}{>{\raggedright\arraybackslash}p{\mdw{0.4404}}>{\raggedright\arraybackslash}p{\mdw{0.2714}}>{\raggedleft\arraybackslash}p{\mdw{0.2742}}}
\toprule
\textbf{setting} & \textbf{usual calibration data: error (splits above $\alpha$)} & \textbf{the policy's own answers: error (splits above $\alpha$)} \\
\midrule
\mdourrow StartLux-Decision 4B / 9B / 27B, best-of-N, unseen datasets, $\alpha$ = .05, N = 32 & 10.05\% / 9.27\% / 7.57\% (19 / 20 / 20 of 20) & 3.5--4.3\% (0--4 of 20) \\
\mdourrow StartLux-Decision 4B / 9B / 27B, best-of-N, unseen datasets, 0.8B generator, $\alpha$ = .05, N = 256 & 12.9 / 11.6 / 7.8\% (20 of 20 each) & 3.4 / 3.3 / 3.7\% (0--1 of 20) \\
all 67 pairs with coverage, best-of-16, $\alpha$ = .05 & above the level in 44 of 67 pairs & above the level in 0 of 67 pairs \\
\mdourrow StartLux-Decision-4B, think-gate, CJ-Bench, $\alpha$ = .05, 10\% / 20\% think rate & thought answers 27.9\% / 27.3\% (20 / 20) & no thought answer accepted, system 4.6\% (0) \\
\mdourrow StartLux-Decision-9B, select-then-think, reasoning sets, $\alpha$ = .10, N = 2 / 4 / 8 & thought answers 22.2 / 18.6 / 15.8\% (20 / 20 / 14) & 6.9--7.8\% (0) \\
\bottomrule
\end{tabular}
\end{adjustbox}\par}
\end{table}

\subsection{The policy-aware map in every pipeline}\label{sec:B.5}

\textbf{Best-of-N.} The \emph{set-aware map} g(s, m, N) (Proposition 4) is told the selected score
s, the mean score m of the N candidates and N. We fitted it at N = 1, 4 and 16 only and evaluated it
on other problems at every N (Figure~\ref{fig:B.3}). On the unseen datasets with the 2B generator it
stays within $-$0.7 \ldots{} +0.3 points for five verifiers ($-$1.2 for Phi-4-mini-instruct at N =
32), including N = 2, 8 and 32, which it never saw. On the same problems at N = 32 the rule ``accept
iff confidence $\geq$ .95'' accepts answers at 5.4\% to 8.0\% error under the single-response map
(above the level in 17 to 20 of 20 splits) and at 1.0--2.9\% under the set-aware map (in none). At N
= 256, sixteen times the largest fitted N, the set-aware map is underconfident by 0.1 to 2.6 points
over three generators and three verifiers.

\begin{figure}[!htbp]
\renewcommand{\thefigure}{B.3}
\centering
\adjincludegraphics[max width=\linewidth,max height=0.5\textheight]{figures/fig5x_setaware.pdf}
\caption{The set-aware map stays near calibrated at values of N it never saw, and the single-response map does not. Set-aware calibration for best-of-N on the unseen datasets. (a, b) Overconfidence of the selected response against N under the single-response map (solid) and the set-aware map fitted at N = 1, 4 and 16 (dashed, with filled markers at the fitted N and open markers at N it never saw), with the 2B generator (a) and the 0.8B generator (b). (c) Error of the accepted answers at $\alpha$ = .05 for a threshold certified on single responses (solid), once on the set-aware confidence at N = 1, 4 and 16 (dashed) and per N (dotted), 2B generator. Means over 20 splits, bars the 10th--90th percentile.}\label{fig:B.3}
\end{figure}

A single threshold on the set-aware confidence, certified once on outputs pooled over N = 1, 4 and
16, accepts answers at $\alpha$ = .05 for N = 1 \ldots{} 32 at 3.4--4.5\% error for our three
verifiers and Clef 27B (above the level in 0--6 of 20 splits), against up to 7.2--9.9\% for the
single-response threshold (18--20 of 20 from N = 4 on). It does not extrapolate: with the 0.8B
generator it accepts answers at 4.4--5.2\% error for N = 32 \ldots{} 256, above the level in 5--14
of 20 splits. The mean score of the candidates matters for weak verifiers (Phi-4-mini-instruct at N
= 64, $\alpha$ = .05: 11.1\% error without it, 3.5\% with it). The map has to be fitted in the
deployment distribution: fitted on the held-out set and applied to the unseen datasets it is
overconfident by up to +6.1 points (4B verifier, N = 1 $\rightarrow$ 32).

\textbf{Think-gates.} The route-aware map g(c1, c0) is an isotonic map of the thought confidence c1
within eight quantile strata of the plain confidence c0 that the gate routes on, fitted on the
thought answers of all calibration items without knowing the threshold. It brings the overconfidence
of thought answers on routed items to within about $\pm$.02 of zero for all nine models at think
rates of 10, 30 and 50\% on the decision suite (up to +.16 with the usual map of c1 alone). It
repairs the calibration and not the certificate: one threshold for all final answers still lets
thought answers through above the level at $\alpha$ = .10 and a 30\% think rate (our 4B at 12.6\%
error with the usual map and 10.7\% with the route-aware map, above the level in 16 and in 9 of 20
splits), so the guarantee is certified per route.

\textbf{Cascades and select-then-think.} With 30\% of the items escalated, the large model's answers
on the escalated items are overconfident by 11 to 18 points raw and by 2.3 to 8.4 points after the
usual calibration, and a map that also sees the small model's confidence leaves $-$0.6 to +0.5. For
select-then-think the usual map is overconfident by +2.1 to +7.3 points at the largest N of each
setting, and the policy-aware map, fitted at the two or three smallest N, stays within $-$1.4
\ldots{} +0.7 at every N, including values it never saw.

Records of a system we did not build. System Switch \citep{bailo2026systemswitch} sends the least
confident decisions of a typed-decision actor to a separate vision reasoner and publishes per
question the actor's confidence and whether actor and reasoner are right (eleven actors under two
option orders, 600 held-out decisions, 21 settings). We used the records, public since 5 October
2026, for evaluation only. The reasoner states no confidence, so a user has its accuracy: 69.0\%
over all questions, but 49.4\% to 78.9\% on the 30\% of the questions that an actor defers.
Estimated on other games, the overall accuracy misses the accuracy on the deferred questions by
$-$10.7 to +18.1 points (8.3 in mean absolute value), and the route-aware map, the reasoner's
accuracy within five strata of the actor's confidence, by $-$7.4 to +4.4 (2.1), the closer estimate
in 19 of the 21 settings. A system of two models is a baseline here, not our method.

\subsection{The value gate}\label{sec:B.6}

Instead of routing on uncertainty, the \emph{value gate} asks whether reasoning is worth its cost on
this item. It is a typed yes/no question of the same model, read in the same pass as the one-pass
answer, with a cost level as input. Its labels are exact, because for every training item the plain
answer and the answer after reasoning both exist: four reasoning samples give the gain in negative
Brier score that reasoning brings net of the cost of its tokens, and the target is the share of the
positive part of that gain (Proposition 5). We trained it from the released 4B. It is a research
result on diagnostic decisions and not the default control. \todo{say whether a checkpoint that
answers the value question is released.}

At an equal think rate, the thought answers on the items it routes are 75\% accurate where those
routed by uncertainty are 30\% accurate (4B, think rate 15.9\%), and they become certifiable: on the
4B, 192 thought answers per split are accepted at 5.5\% error (target 10\%) without a violation,
where the uncertainty rule and the confidence gate accept none per route. In a two-model control its
score has a residual AUROC of .48--.51 at 4B against .69 for the plain confidence, so it says where
thinking pays and not where the thought answer will be wrong.

It does not raise the accuracy of the whole system at a middling think rate (at 45\% within half a
point of routing by confidence at all three sizes), but it asks for shorter reasoning (349 against
436 tokens per item at 4B) and is ahead at a low think rate at 4B (+1.26 points at 16\%). A public
system (TypeLLM's automatic mode, 1--2 October 2026) routes with a typed question about how much
reasoning an item needs. At a 20\% think rate the value gate is +1.23 {[}+0.76, +1.71{]} (4B) and
+0.76 {[}+0.42, +1.11{]} (9B) points above that question answered by the base model.
