# Supplementary material for: StartLux-Decision: AutoThink Decision Models with Reinforcement Learning for Calibrated Deliberative Decisions
Source: arXiv:2610.17309 source file (2026-10-20)
Supplement: Supplementary file 3 [file appendix_B_selection.tex]

\clearpage
\section{Selection among samples: details}\label{sec:B}

The details behind the selection results of Section~\ref{sec:7.3} and the verifier results of
Section~\ref{sec:7.7} are collected here: the protocol, the table by verifier in full, every finding
with its interval, the two cases without the effect, the runs with 256 samples, generators of other
families, the certificates for best-of-N, and verification in closed-book question answering.
Section~\ref{sec:B.7} lists what is not yet written out.

\subsection{Protocol}\label{sec:B.1}

\textbf{Policy.} Best-of-N (A.1): a generator draws N responses to a problem, a verifier scores each
response, and the system returns the response with the highest score and reports that score. A
verifier is a decision model asked one typed question about a candidate response: is it correct? The
StartLux-Decision verifiers are used as released, without training for verification, unless stated.

\textbf{Systems.} Verifiers: StartLux-Decision-4B, $-$9B and $-$27B, two decision models of another
team (Clef 27B and Clef-flash 9B), generalist chat models used as judges (Phi-4-mini-instruct,
Gemma-3-4b-it, Gemma-3-12b-it and Phi-4, 14B), and, in Figure~\ref{fig:B.3}, the base models ours
are tuned from. Generators: a 0.8B, a 2B and a 4B generator of ours, and Phi-4-mini-instruct,
Gemma-3-4b-it, Gemma-3-12b-it and Phi-4. All runs are our own. Models of other teams were run by us
from their public weights and code in the documented configuration. \todo{say which checkpoints the
0.8B, 2B and 4B generators are; v4 writes only ``2B generator'' (part2.md:77) and ``our decision
models at five sizes'' (part1.md:18).}

\textbf{Problems.} Four task domains: an arithmetic set called the held-out problems, the arithmetic
problems of five unseen datasets (5,761 problems, two of the datasets being MAWPS and GSM-Hard),
reasoning sets, and closed-book question answering (8,000 questions from NQ-open, PopQA,
WebQuestions and TriviaQA, N = 16). \todo{describe the problem sets --- what the held-out problems
are held out from, names and sizes of the held-out problems and of the reasoning sets, the other
three unseen datasets, sampling settings of the generators. v4 leaves this to an unwritten appendix
(``B. The full grid'', part3b.md:838-839); the grid file gives 1,550 held-out problems and 5,988
reasoning problems.}

\textbf{Measures.} \emph{Accuracy} is that of the returned response. \emph{Overconfidence} is the
mean reported confidence of the returned responses minus their accuracy, in points, after
calibration on single responses: an isotonic map fitted on single judged responses, which is the
usual calibration of a verifier. The \emph{within-problem AUROC} of a verifier is computed on single
responses. Certificates follow the protocol of Section~\ref{sec:7.4}.

\textbf{Statistics.} Every rule is evaluated on the same random N-subsets of the samples of a
problem. Intervals are 95\% intervals from a cluster bootstrap over source problems. Differences
between two values of N are paired over problems, with the exact expectation over N-subsets and 95\%
bootstrap intervals over sources. Calibration and certification use 20 splits by source problem.
Where a range of splits is shown it is the 10th--90th percentile.

\subsection{Accuracy and overconfidence by verifier}\label{sec:B.2}

In every pair of a generator and a verifier that we ran, the response selected by the verifier's
score is overconfident after calibration on single responses (111 of 113 pairs at N = 16, with the
two exceptions explained in B.4), the gap grows with N (all 126 pairs of Table~\ref{tab:B.2}), and
it is larger the weaker the verifier (Figure~\ref{fig:B.3}a). With weak verifiers more samples also
lower the accuracy of the returned answer, and very large N does not wash the effect out.
Table~\ref{tab:B.1} gives the summary rows for the 2B generator, and Table~\ref{tab:7.1}a is a
selection of them.

\begin{table}[!htbp]
\renewcommand{\thetable}{B.1}
\centering
\caption{Accuracy of best-of-N with a 2B generator (\%), and overconfidence of the selected response after calibration on single responses (points), for nine verifiers. The last column gives the overconfidence from N = 4 to the largest N, with one entry per problem set in the order of the accuracy columns (two entries where the reasoning sets were not run). Own runs. Best accuracy per column in bold.}\label{tab:B.1}
{\scriptsize\setlength{\tabcolsep}{4pt}\renewcommand{\arraystretch}{1.1}
\noindent\begin{adjustbox}{max width=\linewidth}
\begin{tabular}{lrrrl}
\toprule
\textbf{verifier (2B generator)} & {\begin{tabular}[b]{@{}r@{}}\textbf{held-out,}\\\textbf{best-of-64}\end{tabular}} & {\begin{tabular}[b]{@{}r@{}}\textbf{unseen}\\\textbf{datasets,}\\\textbf{best-of-32}\end{tabular}} & {\begin{tabular}[b]{@{}r@{}}\textbf{reasoning,}\\\textbf{best-of-16}\end{tabular}} & {\begin{tabular}[b]{@{}l@{}}\textbf{overconfidence after calibration}\\\textbf{on single responses, N = 4 $\rightarrow$ max}\end{tabular}} \\
\midrule
\mdourrow StartLux-Decision-4B & 92.52 & 82.07 & 77.32 & +1.6 $\rightarrow$ +3.8, +4.7 $\rightarrow$ +9.4, +3.5 $\rightarrow$ +6.4 \\
\mdourrow StartLux-Decision-9B & 94.19 & 83.34 & 78.02 & +1.5 $\rightarrow$ +2.9, +4.2 $\rightarrow$ +8.4, +3.4 $\rightarrow$ +6.1 \\
\mdourrow StartLux-Decision-27B & \textbf{95.48} & \textbf{86.04} & \textbf{82.97} & +0.5 $\rightarrow$ +1.4, +1.8 $\rightarrow$ +3.8, +2.4 $\rightarrow$ +3.2 \\
Clef 27B (another team's decision model) & 93.01 & 83.13 & 77.01 & +1.0 $\rightarrow$ +3.5, +3.0 $\rightarrow$ +7.0, +2.4 $\rightarrow$ +5.3 \\
Clef-flash 9B (another team's decision model) & 85.14 & 78.47 & 67.23 & +2.1 $\rightarrow$ +9.3, +4.6 $\rightarrow$ +11.7, +3.1 $\rightarrow$ +9.6 \\
Phi-4-mini-instruct (generalist chat model) & 83.17 & 74.16 & 66.45 & +4.3 $\rightarrow$ +11.4, +6.8 $\rightarrow$ +14.9, +5.7 $\rightarrow$ +10.8 \\
Gemma-3-12b-it (generalist chat model) & 89.93 & 78.33 & -- & +0.9 $\rightarrow$ +3.8, +3.6 $\rightarrow$ +9.3 \\
Gemma-3-4b-it (generalist chat model) & 83.29 & 73.73 & 65.78 & +3.5 $\rightarrow$ +10.2, +5.8 $\rightarrow$ +14.7, +2.7 $\rightarrow$ +4.1 \\
Phi-4 (14B, generalist chat model) & 90.57 & 78.44 & -- & $-$1.9 $\rightarrow$ $-$0.5 (saturated score, B.4), +2.6 $\rightarrow$ +7.5 \\
\bottomrule
\end{tabular}
\end{adjustbox}\par}
\end{table}

\todo{two estimates of the same overconfidence differ in the last digit --- unseen datasets, 2B
generator, N = 32: +8.4 (9B), +3.8 (27B), +7.0 (Clef 27B), +14.9 (Phi-4-mini) in v4 Table 3
(part2.md:83-87) against +8.3, +3.6, +6.7 and +14.6 in v4 Appendix D.1 and Table 6
(part3b.md:543-544, part2.md:358). The two come from different table files; choose one protocol or
say that they differ.}

Figure~\ref{fig:B.1} shows accuracy and certified error against N for the 2B generator,
Figure~\ref{fig:B.2} extends the accuracy panel to 256 samples, and Figure~\ref{fig:B.3} places
every run on two axes.

\begin{figure}[!htbp]
\renewcommand{\thefigure}{B.1}
\centering
\adjincludegraphics[max width=\linewidth,max height=0.5\textheight]{figures/fig3_bon.pdf}
\caption{Selection among samples. (a) Accuracy of the returned answer against the number of samples N on held-out problems for one generator: majority vote, the response with the highest verifier probability for several verifiers (``judge'' in the labels), and the oracle (a correct response exists), the same random N-subsets for every rule, 95\% intervals from a cluster bootstrap over source problems. (b) Error of the accepted answers against N when the acceptance threshold is certified for error $\leq$ $\alpha$ on single judged responses or under the same best-of-N policy, means over 20 splits by source, bars the 10th--90th percentile of the splits. Own runs.}\label{fig:B.1}
\end{figure}

\todo{the v4 caption (part2.md:94) does not say that panel (b) is on the unseen datasets at $\alpha$
= .05; the figure metadata and the first row of Table D.1 say so. Add it.}

\begin{figure}[!htbp]
\renewcommand{\thefigure}{B.2}
\centering
\adjincludegraphics[max width=\linewidth,max height=0.5\textheight]{figures/fig3L_bon.pdf}
\caption{Selection among samples with 256 samples per held-out problem. (a) As Figure~\ref{fig:B.1}a, with three verifiers and N up to 256. (b) The certificate panel of Figure~\ref{fig:B.1}, repeated unchanged.}\label{fig:B.2}
\end{figure}

\begin{figure}[!htbp]
\renewcommand{\thefigure}{B.3}
\centering
\adjincludegraphics[max width=\linewidth,max height=0.5\textheight]{figures/fig4_grid.pdf}
\caption{The selection effect across verifiers, generators and task domains, every run at N = 16. (a) Overconfidence of the selected response after calibration on single responses against the verifier's within-problem AUROC on single responses. One marker per run and verifier. (b) Error of the accepted answers at level $\alpha$ with the threshold certified on single responses (horizontal axis) against the threshold certified under the same best-of-16 policy (vertical axis). Dashed lines mark the level. One column per task domain, marker the kind of verifier.}\label{fig:B.3}
\end{figure}

\subsection{Findings in detail}\label{sec:B.3}

\textbf{The same verifier confidence is worth less the more candidates it was chosen from, in every
pair.} A 9B confidence of .80--.90 is right 92.3\% of the time for a single response, 86.2\% for the
best of four and 78.2\% for the best of 32. For Clef 27B the figures are 74.8, 67.4 and 63.7, and
for Phi-4-mini as verifier 87.5, 78.0 and 64.2. With 256 samples per held-out problem, a 9B
confidence of .80--.90 is worth 95.6 / 93.2 / 90.1 / 88.1 / 87.9\% for N = 1 / 4 / 16 / 64 / 256 (2B
generator, 95.5 $\rightarrow$ 83.7\% with Phi-4-mini as generator).

\textbf{More samples can lower accuracy.} Weak verifiers peak and fall.

\begin{itemize}
\item Clef-flash on the held-out set: 86.7 (N = 16) $\rightarrow$ 85.1 (N = 64), $-$1.6 {[}$-$2.6,
$-$0.6{]}.
\item Phi-4-mini as judge: 84.2 $\rightarrow$ 83.2, $-$1.0 {[}$-$2.0, $-$0.1{]}.
\item Clef-flash on the reasoning sets with the 4B generator: 82.2 (N = 4) $\rightarrow$ 80.4 (N = 16),
$-$1.8 {[}$-$2.4, $-$1.2{]}.
\item StartLux-Decision-4B and $-$9B on MAWPS with the 0.8B generator, from N = 8 to 32: 84.9
$\rightarrow$ 82.8, $-$2.2 {[}$-$3.2, $-$1.1{]}, and 86.2 $\rightarrow$ 84.8, $-$1.4 {[}$-$2.3,
$-$0.5{]}.
\item With 256 samples per problem the fall continues. From N = 8 to 256 the 4B verifier loses 6.0 points
{[}$-$7.4, $-$4.6{]} (85.2 $\rightarrow$ 79.2) and the 9B 3.9 {[}$-$5.0, $-$2.8{]} (86.2
$\rightarrow$ 82.3), while the 27B still gains +1.7 {[}+0.7, +2.8{]} (89.3 $\rightarrow$ 91.0) on
the same samples, and with the 2B generator on the same problems $-$2.5 {[}$-$3.5, $-$1.6{]} (4B)
and $-$2.6 {[}$-$3.5, $-$1.7{]} (9B) against +2.5 {[}+1.5, +3.5{]} (27B).
\item The fall is not universal: the same Clef-flash still gains from N = 4 to 16 with the weaker 2B
generator on the reasoning sets (64.0 $\rightarrow$ 67.2).
\end{itemize}

\textbf{Large N does not wash the effect out.} With 256 samples per held-out problem and three
generators (Figure~\ref{fig:B.2}), the overconfidence after calibration on single responses does not
go away with more samples.

\begin{itemize}
\item \emph{Held-out problems.} It keeps growing with the 2B generator (4B verifier +3.4 $\rightarrow$
+4.8 from N = 64 to 256, +1.4 {[}+0.8, +2.0{]}, 9B +0.5 {[}+0.0, +1.0{]}, 27B +0.6 {[}+0.3, +1.1{]})
and sits on a plateau with the 0.8B generator (+5.2 / +4.4 / +2.1 at N = 64, +4.9 / +4.2 / +2.5 at N
= 256) and the Phi-4-mini generator (+3.1 / +3.3 / +2.1 $\rightarrow$ +3.3 / +3.9 / +2.2). What the
extra samples buy depends on the generator: nothing for the 4B verifier with the 2B generator (92.9
$\rightarrow$ 92.5, $-$0.4 {[}$-$1.0, +0.1{]}), +2.4 to +2.9 points with the weak 0.8B generator,
+0.4 to +0.9 with Phi-4-mini. At N = 256 the single-response certificate at $\alpha$ = .05 runs at
5.7--6.1\% error for the 4B verifier with each of the three generators (above the level in 5--10 of
20 splits) and at 4.7--5.5\% for the 9B (6--9 of 20), and per policy 3.1--4.6\% and 3.4--4.1\%.
\item \emph{Unseen datasets, 0.8B generator (5,761 problems).} The effect is larger and still growing at N
= 256. Accuracy rises from N = 64 to 256 by +1.3 / +1.8 / +2.5 points (4B / 9B / 27B verifier) and
the overconfidence after single-response calibration by +2.0 {[}+1.5, +2.4{]} / +1.5 {[}+1.1,
+1.9{]} / +1.1 {[}+0.8, +1.5{]}, to +15.1 / +12.8 / +6.5 points (hardest set, GSM-Hard: +22.9 /
+18.5 / +9.0). The single-response certificate at $\alpha$ = .05 then accepts answers at 12.9 / 11.6
/ 7.8\% error (above the level in 20 of 20 splits each), and per policy 3.4 / 3.3 / 3.7\% (0--1 of
20).
\item \emph{Unseen datasets, 2B generator, the same 5,761 problems.} The two smaller verifiers gain
nothing from four times the samples (N = 64 $\rightarrow$ 256: +0.1 {[}$-$0.3, +0.5{]} and +0.3
{[}$-$0.0, +0.6{]}, 27B +1.4 {[}+1.0, +1.7{]}) while the overconfidence still rises by +2.1 {[}+1.8,
+2.5{]} / +1.9 {[}+1.6, +2.2{]} / +1.0 {[}+0.8, +1.3{]}, to +12.7 / +11.5 / +5.5, single-response
certificate 12.5 / 11.4 / 8.0\% (20 of 20 each), per policy 3.0 / 2.7 / 3.5\% (0--1 of 20).
\end{itemize}

\todo{v4 gives +15.1 / +12.8 / +6.5 and +12.7 / +11.5 / +5.5 here (part3b.md:415, 419; part2.md:123)
and +15.0 / +12.7 / +6.4 and +12.6 / +11.5 / +5.4 for the same quantity in Appendix D.1
(part3b.md:549, 552); see the TODO under Table B.1.}

\textbf{Generators of other families behave the same.} Phi-4-mini-instruct and Gemma-3-4b-it on the
held-out set (87\% / 86\% single accuracy) give +1.2 to +3.7 at N = 64. On the unseen datasets
Phi-4-mini, Gemma-3-4b, Gemma-3-12b and Phi-4 (75--82\% single accuracy) give +3.4 to +8.5 at N =
32, with the single-response certificate at $\alpha$ = .05 above the level in 19--20 of 20 splits
for every one of our three verifiers (6.5--9.2\% error, per policy 3.2--4.3\%). On the reasoning
sets Phi-4-mini and Gemma-3-4b give +4.0 to +6.8, and the two strongest generators, Gemma-3-12b and
Phi-4 (80\% and 82\% single accuracy, which our 27B verifier lifts to 89.6 and 90.3, 6.5 and 5.1
points above their vote), +2.9 to +5.9 with the single-response certificate at 5.8--7.4\% error
(above the level in 13--19 of 20 splits in five of the six pairs, per policy 3.7--4.3\%, 0--2 of
20).

\textbf{Fine-tuning the verifier does not remove the effect.} A LoRA-tuned 4B verifier equals the
zero-shot 27B in distribution (95.0 against 95.5, the ``fine-tuned'' curve of Figure~\ref{fig:B.1}a)
and keeps the selection gap. Training on the distribution its own selection induces (order
statistics, top-k, selection gradients) is no better than training on uniform pairs. \todo{the
details were announced for an appendix that v4 does not contain (``F. Verifiers'',
part3b.md:844-845; referenced at part2.md:130).}

\subsection{The two pairs without the effect}\label{sec:B.4}

The two pairs without the effect are the same judge, Phi-4, with the 2B and the Gemma-3-4b generator
on the held-out set, and they are instructive. Phi-4 as judge puts 59\% of the held-out responses
above .9999 (94\% of them right) and almost all others below .5: it approves or rejects, it does not
rank. Best-of-N then returns a random approved response and its accuracy at the top score does not
depend on N (90.6\% for N = 1, 91.1\% for N = 4, 16 and 64). On the unseen datasets, where the share
of approved-but-wrong responses varies with the problem, the same judge shows the effect (+2.6
$\rightarrow$ +7.5).

\subsection{Certificates for best-of-N}\label{sec:B.5}

Table~\ref{tab:D.1} has the certificate rows of all pipelines. For best-of-N on the unseen datasets
at $\alpha$ = .05 and N = 32, a threshold certified on single responses accepts answers at 10.05\% /
9.27\% / 7.57\% error for the 4B / 9B / 27B verifier (above the level in 19 / 20 / 20 of 20 splits),
and certified under the same policy, at 3.5--4.3\% (0--4 of 20). Over all 67 pairs with coverage at
N = 16 and $\alpha$ = .05 (Figure~\ref{fig:B.3}b), the single-response threshold is above the level
in 44 pairs and the per-policy threshold in none. A per-policy certificate also refuses a system
that cannot be trusted: Clef-flash on the reasoning sets at $\alpha$ = .20 accepts 17--28\% of the
answers at 21.5--26.7\% error under the single-response threshold and nothing per policy.

\subsection{Verifiers: comparisons and the limit of verification}\label{sec:B.6}

\textbf{Against chat models as judges.} At equal size, StartLux-Decision-4B is 8 to 11 points above
Phi-4-mini-instruct used as judge: 92.5 / 82.1 / 77.3 against 83.2 / 74.2 / 66.5 on the held-out
problems, the unseen datasets and the reasoning sets. Three times the size does not close the gap:
Gemma-3-12b reaches 89.9 / 78.3 and Phi-4 (14B) 90.6 / 78.4 against the 4B's 92.5 / 82.1.

\textbf{Against another team's decision models.} Our 9B is at least level with Clef 27B. Our 27B is
ahead of Clef 27B by +2.5 {[}+1.6, +3.4{]} and +2.9 {[}+2.3, +3.5{]} points, and by 6.0 points on
the reasoning sets (82.97 against 77.01), where Clef 27B is level with our 4B (77.32).

\textbf{Against voting.} A 9B verifying 8 samples of a 2B generator beats the 64-sample majority
vote (91.0 against 89.1). On five unseen datasets verification adds 5.6 (9B) to 8.3 (27B) points. On
the reasoning sets the 27B adds 8.1 (2B generator). Adaptive sampling reaches 93.4 with 5.4 samples
on average. \todo{adaptive sampling is described only by this sentence; its protocol was announced
for the unwritten v4 appendix ``F. Verifiers'' (part2.md:590, part3b.md:844-845).}

\textbf{Where verification stops.} In closed-book question answering (8,000 questions from NQ-open,
PopQA, WebQuestions and TriviaQA, N = 16) a verifier that does not know the fact cannot check it.
Best-of-16 is 0.1--2.7 points above the vote with the 4B generator (31.0 / 32.3 / 33.6 against
30.9), 2.7--6.8 with the 2B and Phi-4-mini generators, 0.2--1.6 with Gemma-3-12b, and 0.9--2.3
points \emph{below} the vote with Phi-4 (43.0 / 43.6 / 44.4 against 45.3). The verifier's confidence
is poor already for single responses (27B: 58\% right at .80--.90). The selection effect is at its
largest there: +6.9 to +17.5 points at N = 16, and at $\alpha$ = .30 the single-response threshold
accepts answers at 29--35\% error, in up to 20 of 20 splits, where the per-policy threshold accepts
them at 25--26.5\%, in 0--2. \todo{the largest overconfidence in question answering at N = 16 is
+17.5 here (part2.md:597) and +18.0 in the set-aware experiment (part2.md:278, part3b.md:561); say
whether the two use different splits.}

\subsection{The full grid, and what is not yet written out}\label{sec:B.7}

\begingroup
\renewcommand{\thetable}{B.2}
\scriptsize\setlength{\tabcolsep}{3pt}\renewcommand{\arraystretch}{1.1}
\begin{longtable}{>{\raggedright\arraybackslash}p{\mdw{0.0921}}>{\raggedright\arraybackslash}p{\mdw{0.0879}}>{\raggedright\arraybackslash}p{\mdw{0.0855}}>{\raggedleft\arraybackslash}p{\mdw{0.0364}}>{\raggedleft\arraybackslash}p{\mdw{0.0571}}>{\raggedleft\arraybackslash}p{\mdw{0.0486}}>{\raggedleft\arraybackslash}p{\mdw{0.0522}}>{\raggedleft\arraybackslash}p{\mdw{0.0590}}>{\raggedleft\arraybackslash}p{\mdw{0.0848}}>{\raggedleft\arraybackslash}p{\mdw{0.1313}}>{\raggedleft\arraybackslash}p{\mdw{0.0543}}>{\raggedleft\arraybackslash}p{\mdw{0.0993}}>{\raggedleft\arraybackslash}p{\mdw{0.0990}}}
\caption{One row per run and verifier (126 rows): domain, generator, verifier, N, single-sample accuracy, vote, best-of-N, oracle, within-problem AUROC, overconfidence at N = 4 and at the largest N, accuracy at a confidence of .80--.90 for N = 1 and N = 16, and the certificates at $\alpha$ = .05 and $\alpha$ = .10 on single responses and per policy. A dash marks a value that is not available.}\label{tab:B.2}\\
\toprule
\textbf{domain} & \textbf{generator} & \textbf{verifier} & \textbf{N} & \textbf{single} & \textbf{vote} & \textbf{best-of-N} & \textbf{oracle} & \textbf{within-problem AUROC} & \textbf{overconfidence N=4 $\rightarrow$ N} & \textbf{at .80--.90: N=1 $\rightarrow$ 16} & \textbf{$\alpha$=0.05: single-response threshold err (viol) / per policy} & \textbf{$\alpha$=0.1: single-response threshold err (viol) / per policy} \\
\midrule
\endfirsthead
\multicolumn{13}{l}{\textit{Table~\thetable{} (continued)}}\\
\toprule
\textbf{domain} & \textbf{generator} & \textbf{verifier} & \textbf{N} & \textbf{single} & \textbf{vote} & \textbf{best-of-N} & \textbf{oracle} & \textbf{within-problem AUROC} & \textbf{overconfidence N=4 $\rightarrow$ N} & \textbf{at .80--.90: N=1 $\rightarrow$ 16} & \textbf{$\alpha$=0.05: single-response threshold err (viol) / per policy} & \textbf{$\alpha$=0.1: single-response threshold err (viol) / per policy} \\
\midrule
\endhead
\bottomrule
\endfoot
arithmetic, held-out & 0.8B & 0.8B (ours, decision) & 64 & 40.9 & 74.71 & 59.48 & 95.61 & 0.782 & +6.2 $\rightarrow$ +20.3 & -- & -- (0/20) / -- (0/20) & -- (0/20) / -- (0/20) \\
arithmetic, held-out & 0.8B & 27B (ours, decision) & 64 & 40.9 & 74.71 & 90.97 & 95.61 & 0.964 & +1.8 $\rightarrow$ +2.8 & 91.37 $\rightarrow$ 82.75 & 3.56\% (1/20) / 3.95\% (3/20) & 5.12\% (0/20) / 5.12\% (0/20) \\
arithmetic, held-out & 0.8B & 2B (ours, decision) & 64 & 40.9 & 74.71 & 77.74 & 95.61 & 0.861 & +4.5 $\rightarrow$ +11.6 & 95.16 $\rightarrow$ 94.37 & -- (0/20) / 7.73\% (1/20) & 13.01\% (8/20) / 6.23\% (0/20) \\
arithmetic, held-out & 0.8B & 4B (ours, decision) & 64 & 40.9 & 74.71 & 86.9 & 95.61 & 0.933 & +3.5 $\rightarrow$ +6.1 & 93.21 $\rightarrow$ 87.78 & 4.61\% (2/20) / 3.91\% (1/20) & 7.89\% (1/20) / 7.9\% (2/20) \\
arithmetic, held-out & 0.8B & 9B (ours, decision) & 64 & 40.9 & 74.71 & 88.39 & 95.61 & 0.948 & +3.0 $\rightarrow$ +5.7 & 95.64 $\rightarrow$ 89.33 & 4.62\% (5/20) / 4.33\% (0/20) & 7.66\% (0/20) / 8.33\% (4/20) \\
arithmetic, held-out & 0.8B & Clef-flash 9B, external decision & 64 & 40.9 & 74.71 & 76.14 & 95.61 & 0.908 & +3.6 $\rightarrow$ +13.5 & 72.08 $\rightarrow$ 59.65 & -- (0/20) / -- (0/20) & 15.88\% (4/20) / -- (0/20) \\
arithmetic, held-out & 2B & 0.8B (ours, decision) & 64 & 69.55 & 89.03 & 78.65 & 97.81 & 0.813 & +4.7 $\rightarrow$ +13.6 & -- & -- (0/20) / -- (0/20) & 17.99\% (9/20) / -- (0/20) \\
arithmetic, held-out & 2B & 27B (ours, decision) & 64 & 69.55 & 89.03 & 95.48 & 97.81 & 0.976 & +0.5 $\rightarrow$ +1.4 & 89.0 $\rightarrow$ 85.45 & 3.59\% (1/20) / 3.84\% (1/20) & 4.02\% (0/20) / 4.02\% (0/20) \\
arithmetic, held-out & 2B & 2B (ours, decision) & 64 & 69.55 & 89.03 & 85.23 & 97.81 & 0.873 & +4.0 $\rightarrow$ +9.8 & 96.94 $\rightarrow$ 94.32 & 8.23\% (5/20) / 4.87\% (1/20) & 11.56\% (17/20) / 7.07\% (0/20) \\
arithmetic, held-out & 2B & 4B (ours, decision) & 64 & 69.55 & 89.03 & 92.52 & 97.81 & 0.947 & +1.6 $\rightarrow$ +3.8 & 93.99 $\rightarrow$ 88.5 & 5.02\% (4/20) / 4.08\% (1/20) & 7.02\% (0/20) / 7.24\% (0/20) \\
arithmetic, held-out & 2B & 9B (ours, decision) & 64 & 69.55 & 89.03 & 94.19 & 97.81 & 0.960 & +1.5 $\rightarrow$ +2.9 & 95.27 $\rightarrow$ 90.32 & 4.65\% (5/20) / 3.86\% (2/20) & 5.44\% (0/20) / 5.52\% (0/20) \\
arithmetic, held-out & 2B & base4B (base 4B, no decision training) & 64 & 69.55 & 89.03 & 88.06 & 97.81 & 0.878 & +2.1 $\rightarrow$ +6.0 & 95.17 $\rightarrow$ 88.41 & 5.7\% (3/20) / 3.61\% (0/20) & 9.42\% (8/20) / 7.75\% (2/20) \\
arithmetic, held-out & 2B & base9B (base 9B, no decision training) & 64 & 69.55 & 89.03 & 91.35 & 97.81 & 0.919 & +1.5 $\rightarrow$ +3.7 & 90.18 $\rightarrow$ 83.27 & 4.28\% (3/20) / 3.74\% (0/20) & 7.19\% (0/20) / 7.17\% (0/20) \\
arithmetic, held-out & 2B & Clef 27B, external decision & 64 & 69.55 & 89.03 & 93.01 & 97.81 & 0.955 & +1.0 $\rightarrow$ +3.5 & 89.03 $\rightarrow$ 80.29 & 5.43\% (6/20) / 3.54\% (1/20) & 6.45\% (0/20) / 6.47\% (0/20) \\
arithmetic, held-out & 2B & Clef-flash 9B, external decision & 64 & 69.55 & 89.03 & 85.14 & 97.81 & 0.907 & +2.1 $\rightarrow$ +9.3 & 83.94 $\rightarrow$ 74.52 & 7.54\% (1/20) / -- (0/20) & 13.51\% (18/20) / 9.48\% (3/20) \\
arithmetic, held-out & 2B & Gemma-3-12b, generalist & 64 & 69.55 & 89.03 & 89.93 & 97.81 & 0.910 & +0.9 $\rightarrow$ +3.8 & 52.31 $\rightarrow$ -- & -- (0/20) / -- (0/20) & 9.35\% (1/20) / 9.91\% (0/20) \\
arithmetic, held-out & 2B & Gemma-3-4b, generalist & 64 & 69.55 & 89.03 & 83.29 & 97.81 & 0.834 & +3.5 $\rightarrow$ +10.2 & 53.94 $\rightarrow$ -- & -- (0/20) / -- (0/20) & -- (0/20) / -- (0/20) \\
arithmetic, held-out & 2B & Phi-4, generalist & 64 & 69.55 & 89.03 & 90.57 & 97.81 & 0.882 & $-$1.9 $\rightarrow$ $-$0.5 & 50.23 $\rightarrow$ 54.58 & -- (0/20) / -- (0/20) & 8.67\% (1/20) / 9.2\% (4/20) \\
arithmetic, held-out & 2B & Phi-4-mini, generalist & 64 & 69.55 & 89.03 & 83.17 & 97.81 & 0.842 & +4.3 $\rightarrow$ +11.4 & 85.59 $\rightarrow$ 72.15 & 8.69\% (1/20) / -- (0/20) & 14.75\% (15/20) / 7.87\% (3/20) \\
arithmetic, held-out & 4B & 0.8B (ours, decision) & 64 & 89.95 & 94.65 & 91.48 & 97.61 & 0.784 & +2.0 $\rightarrow$ +4.8 & -- & 7.84\% (5/20) / -- (0/20) & 8.68\% (2/20) / 8.39\% (1/20) \\
arithmetic, held-out & 4B & 27B (ours, decision) & 64 & 89.95 & 94.65 & 95.55 & 97.61 & 0.960 & +0.7 $\rightarrow$ +2.2 & 90.36 $\rightarrow$ 78.76 & 4.46\% (3/20) / 3.9\% (3/20) & 4.38\% (0/20) / 4.38\% (0/20) \\
arithmetic, held-out & 4B & 2B (ours, decision) & 64 & 89.95 & 94.65 & 91.94 & 97.61 & 0.816 & +2.5 $\rightarrow$ +5.6 & 97.99 $\rightarrow$ 96.55 & 6.77\% (14/20) / 3.06\% (2/20) & 8.1\% (1/20) / 7.82\% (1/20) \\
arithmetic, held-out & 4B & 4B (ours, decision) & 64 & 89.95 & 94.65 & 94.39 & 97.61 & 0.915 & +1.1 $\rightarrow$ +2.7 & 93.55 $\rightarrow$ 89.38 & 5.56\% (11/20) / 3.66\% (0/20) & 5.63\% (0/20) / 5.63\% (0/20) \\
arithmetic, held-out & 4B & 9B (ours, decision) & 64 & 89.95 & 94.65 & 94.84 & 97.61 & 0.935 & +1.3 $\rightarrow$ +3.1 & 94.64 $\rightarrow$ 89.35 & 5.37\% (10/20) / 4.26\% (3/20) & 5.25\% (0/20) / 5.25\% (0/20) \\
arithmetic, held-out & Phi-4-mini & 27B (ours, decision) & 64 & 86.87 & 91.03 & 94.77 & 96.52 & 0.960 & +1.2 $\rightarrow$ +2.1 & 91.02 $\rightarrow$ 81.28 & 3.75\% (0/20) / 3.65\% (0/20) & 3.83\% (0/20) / 3.83\% (0/20) \\
arithmetic, held-out & Phi-4-mini & 4B (ours, decision) & 64 & 86.87 & 91.03 & 93.55 & 96.52 & 0.906 & +1.7 $\rightarrow$ +2.9 & 94.19 $\rightarrow$ 92.07 & 4.92\% (6/20) / 3.58\% (3/20) & 5.37\% (0/20) / 5.37\% (0/20) \\
arithmetic, held-out & Phi-4-mini & 9B (ours, decision) & 64 & 86.87 & 91.03 & 93.87 & 96.52 & 0.934 & +1.8 $\rightarrow$ +3.1 & 95.5 $\rightarrow$ 90.03 & 4.71\% (2/20) / 3.45\% (2/20) & 4.89\% (0/20) / 4.89\% (0/20) \\
arithmetic, held-out & Phi-4-mini & Clef-flash 9B, external decision & 64 & 86.87 & 91.03 & 90.15 & 96.52 & 0.847 & +2.4 $\rightarrow$ +5.7 & 90.87 $\rightarrow$ 82.66 & 8.55\% (7/20) / 5.42\% (1/20) & 9.92\% (9/20) / 8.12\% (3/20) \\
arithmetic, held-out & Phi-4-mini & Gemma-3-12b, generalist & 64 & 86.87 & 91.03 & 93.13 & 96.52 & 0.872 & +1.8 $\rightarrow$ +2.9 & -- & 5.74\% (7/20) / -- (0/20) & 5.45\% (0/20) / 5.45\% (0/20) \\
arithmetic, held-out & Phi-4-mini & Phi-4, generalist & 64 & 86.87 & 91.03 & 90.2 & 96.52 & 0.806 & $-$0.0 $\rightarrow$ +2.0 & 67.84 $\rightarrow$ 63.58 & -- (0/20) / -- (0/20) & 9.95\% (9/20) / 10.38\% (2/20) \\
arithmetic, held-out & Gemma-3-4b & 27B (ours, decision) & 64 & 86.2 & 89.42 & 94.0 & 95.48 & 0.955 & +0.9 $\rightarrow$ +2.1 & 93.18 $\rightarrow$ 84.94 & 4.32\% (4/20) / 4.09\% (1/20) & 4.49\% (0/20) / 4.49\% (0/20) \\
arithmetic, held-out & Gemma-3-4b & 4B (ours, decision) & 64 & 86.2 & 89.42 & 92.0 & 95.48 & 0.881 & +1.4 $\rightarrow$ +3.7 & 92.09 $\rightarrow$ 88.76 & 6.26\% (14/20) / 3.84\% (0/20) & 7.56\% (0/20) / 7.37\% (0/20) \\
arithmetic, held-out & Gemma-3-4b & 9B (ours, decision) & 64 & 86.2 & 89.42 & 93.16 & 95.48 & 0.910 & +1.2 $\rightarrow$ +2.8 & 95.83 $\rightarrow$ 93.62 & 5.16\% (12/20) / 3.75\% (1/20) & 6.23\% (0/20) / 6.23\% (0/20) \\
arithmetic, held-out & Gemma-3-4b & Gemma-3-12b, generalist & 64 & 86.2 & 89.42 & 91.65 & 95.48 & 0.834 & +0.5 $\rightarrow$ +1.6 & -- & 6.97\% (2/20) / -- (0/20) & 6.92\% (0/20) / 6.9\% (0/20) \\
arithmetic, held-out & Gemma-3-4b & Phi-4, generalist & 64 & 86.2 & 89.42 & 91.72 & 95.48 & 0.831 & $-$2.4 $\rightarrow$ $-$1.3 & 61.61 $\rightarrow$ 66.29 & 6.76\% (7/20) / -- (0/20) & 7.5\% (0/20) / 7.4\% (0/20) \\
arithmetic, held-out & Gemma-3-12b & 27B (ours, decision) & 64 & 92.41 & 94.06 & 95.74 & 97.1 & 0.915 & +0.6 $\rightarrow$ +1.7 & 91.39 $\rightarrow$ 84.83 & 3.94\% (0/20) / 3.66\% (0/20) & 4.01\% (0/20) / 4.01\% (0/20) \\
arithmetic, held-out & Gemma-3-12b & 4B (ours, decision) & 64 & 92.41 & 94.06 & 94.13 & 97.1 & 0.780 & +1.1 $\rightarrow$ +2.9 & 93.4 $\rightarrow$ 91.33 & 5.7\% (12/20) / 3.83\% (3/20) & 6.03\% (0/20) / 6.03\% (0/20) \\
arithmetic, held-out & Gemma-3-12b & 9B (ours, decision) & 64 & 92.41 & 94.06 & 94.9 & 97.1 & 0.847 & +1.0 $\rightarrow$ +2.5 & 95.65 $\rightarrow$ 92.95 & 4.87\% (9/20) / 3.86\% (1/20) & 5.01\% (0/20) / 5.01\% (0/20) \\
arithmetic, held-out & Phi-4 & 27B (ours, decision) & 64 & 91.57 & 92.52 & 94.97 & 96.06 & 0.920 & +1.0 $\rightarrow$ +1.8 & 92.58 $\rightarrow$ 82.62 & 3.95\% (0/20) / 3.67\% (0/20) & 3.85\% (0/20) / 3.85\% (0/20) \\
arithmetic, held-out & Phi-4 & 4B (ours, decision) & 64 & 91.57 & 92.52 & 93.68 & 96.06 & 0.841 & +1.4 $\rightarrow$ +2.9 & 95.21 $\rightarrow$ 90.69 & 5.35\% (10/20) / 3.86\% (2/20) & 5.28\% (0/20) / 5.28\% (0/20) \\
arithmetic, held-out & Phi-4 & 9B (ours, decision) & 64 & 91.57 & 92.52 & 94.39 & 96.06 & 0.876 & +1.6 $\rightarrow$ +2.6 & 96.39 $\rightarrow$ 91.8 & 4.51\% (1/20) / 3.99\% (1/20) & 4.39\% (0/20) / 4.39\% (0/20) \\
arithmetic, held-out, N=256 & 0.8B & 27B (ours, decision) & 256 & 41.01 & 76.0 & 94.39 & 98.77 & 0.959 & +1.6 $\rightarrow$ +2.5 & 91.4 $\rightarrow$ 83.93 & 3.69\% (2/20) / 3.46\% (3/20) & 4.29\% (0/20) / 4.3\% (0/20) \\
arithmetic, held-out, N=256 & 0.8B & 4B (ours, decision) & 256 & 41.01 & 76.0 & 90.71 & 98.77 & 0.928 & +3.2 $\rightarrow$ +4.9 & 93.68 $\rightarrow$ 88.07 & 5.67\% (5/20) / 3.07\% (4/20) & 7.88\% (0/20) / 8.1\% (0/20) \\
arithmetic, held-out, N=256 & 0.8B & 9B (ours, decision) & 256 & 41.01 & 76.0 & 92.39 & 98.77 & 0.943 & +2.5 $\rightarrow$ +4.2 & 95.59 $\rightarrow$ 91.06 & 4.7\% (6/20) / 4.06\% (2/20) & 6.47\% (0/20) / 6.95\% (0/20) \\
arithmetic, held-out, N=256 & 2B & 27B (ours, decision) & 256 & 69.78 & 89.35 & 95.87 & 98.58 & 0.973 & +0.4 $\rightarrow$ +2.0 & 89.53 $\rightarrow$ 83.15 & 3.59\% (1/20) / 3.32\% (2/20) & 3.74\% (0/20) / 3.74\% (0/20) \\
arithmetic, held-out, N=256 & 2B & 4B (ours, decision) & 256 & 69.78 & 89.35 & 92.45 & 98.58 & 0.945 & +1.7 $\rightarrow$ +4.8 & 93.85 $\rightarrow$ 88.9 & 6.12\% (10/20) / 4.63\% (2/20) & 7.18\% (0/20) / 7.13\% (0/20) \\
arithmetic, held-out, N=256 & 2B & 9B (ours, decision) & 256 & 69.78 & 89.35 & 94.52 & 98.58 & 0.958 & +1.6 $\rightarrow$ +3.4 & 95.6 $\rightarrow$ 90.03 & 4.95\% (6/20) / 3.82\% (3/20) & 5.24\% (0/20) / 5.31\% (0/20) \\
arithmetic, held-out, N=256 & Phi-4-mini & 27B (ours, decision) & 256 & 86.87 & 91.1 & 95.48 & 97.81 & 0.962 & +1.3 $\rightarrow$ +2.2 & 92.28 $\rightarrow$ 79.88 & 3.68\% (0/20) / 3.27\% (0/20) & 3.69\% (0/20) / 3.66\% (0/20) \\
arithmetic, held-out, N=256 & Phi-4-mini & 4B (ours, decision) & 256 & 86.87 & 91.1 & 93.87 & 97.81 & 0.920 & +1.7 $\rightarrow$ +3.3 & 94.69 $\rightarrow$ 90.59 & 5.72\% (7/20) / 4.02\% (2/20) & 5.51\% (0/20) / 5.51\% (0/20) \\
arithmetic, held-out, N=256 & Phi-4-mini & 9B (ours, decision) & 256 & 86.87 & 91.1 & 93.94 & 97.81 & 0.942 & +1.8 $\rightarrow$ +3.9 & 95.74 $\rightarrow$ 89.91 & 5.45\% (9/20) / 3.43\% (3/20) & 5.52\% (0/20) / 5.52\% (0/20) \\
arithmetic, unseen sets & 0.8B & 27B (ours, decision) & 32 & 46.49 & 69.71 & 81.81 & 88.06 & 0.953 & +2.1 $\rightarrow$ +4.6 & 86.67 $\rightarrow$ 73.55 & 7.34\% (20/20) / 4.22\% (1/20) & 9.02\% (0/20) / 8.86\% (0/20) \\
arithmetic, unseen sets & 0.8B & 4B (ours, decision) & 32 & 46.49 & 69.71 & 76.65 & 88.06 & 0.918 & +5.7 $\rightarrow$ +11.8 & 91.66 $\rightarrow$ 76.42 & 9.68\% (20/20) / 4.17\% (0/20) & 15.95\% (20/20) / 9.0\% (2/20) \\
arithmetic, unseen sets & 0.8B & 9B (ours, decision) & 32 & 46.49 & 69.71 & 78.34 & 88.06 & 0.933 & +4.7 $\rightarrow$ +10.3 & 94.67 $\rightarrow$ 82.27 & 9.76\% (20/20) / 3.96\% (3/20) & 14.94\% (20/20) / 8.45\% (5/20) \\
arithmetic, unseen sets & 2B & 27B (ours, decision) & 32 & 63.02 & 77.85 & 86.04 & 92.4 & 0.939 & +1.8 $\rightarrow$ +3.8 & 77.43 $\rightarrow$ 63.15 & 7.26\% (20/20) / 4.13\% (1/20) & 9.7\% (8/20) / 9.09\% (7/20) \\
arithmetic, unseen sets & 2B & 4B (ours, decision) & 32 & 63.02 & 77.85 & 82.07 & 92.4 & 0.905 & +4.7 $\rightarrow$ +9.4 & 89.49 $\rightarrow$ 73.15 & 9.8\% (19/20) / 3.95\% (3/20) & 14.43\% (20/20) / 9.22\% (5/20) \\
arithmetic, unseen sets & 2B & 9B (ours, decision) & 32 & 63.02 & 77.85 & 83.34 & 92.4 & 0.917 & +4.2 $\rightarrow$ +8.4 & 92.33 $\rightarrow$ 80.42 & 9.23\% (20/20) / 4.04\% (4/20) & 13.32\% (20/20) / 9.1\% (1/20) \\
arithmetic, unseen sets & 2B & base9B (base 9B, no decision training) & 32 & 63.02 & 77.85 & 80.7 & 92.4 & 0.884 & +3.8 $\rightarrow$ +8.1 & 90.69 $\rightarrow$ 78.01 & 7.8\% (20/20) / 4.31\% (2/20) & 11.73\% (20/20) / 9.16\% (3/20) \\
arithmetic, unseen sets & 2B & Clef 27B, external decision & 32 & 63.02 & 77.85 & 83.13 & 92.4 & 0.918 & +3.0 $\rightarrow$ +7.0 & 75.71 $\rightarrow$ 63.52 & 9.02\% (20/20) / 4.05\% (1/20) & 12.95\% (20/20) / 8.95\% (0/20) \\
arithmetic, unseen sets & 2B & Clef-flash 9B, external decision & 32 & 63.02 & 77.85 & 78.47 & 92.4 & 0.884 & +4.6 $\rightarrow$ +11.7 & 74.97 $\rightarrow$ 57.69 & 9.55\% (16/20) / 2.9\% (0/20) & 17.26\% (20/20) / 6.62\% (0/20) \\
arithmetic, unseen sets & 2B & Gemma-3-12b, generalist & 32 & 63.02 & 77.85 & 78.33 & 92.4 & 0.869 & +3.5 $\rightarrow$ +9.2 & 42.53 $\rightarrow$ 20.89 & -- (0/20) / -- (0/20) & 15.91\% (17/20) / -- (0/20) \\
arithmetic, unseen sets & 2B & Gemma-3-4b, generalist & 32 & 63.02 & 77.85 & 73.73 & 92.4 & 0.806 & +5.8 $\rightarrow$ +14.7 & 41.55 $\rightarrow$ 13.39 & -- (0/20) / -- (0/20) & -- (0/20) / -- (0/20) \\
arithmetic, unseen sets & 2B & Phi-4, generalist & 32 & 63.02 & 77.85 & 78.44 & 92.4 & 0.844 & +2.6 $\rightarrow$ +7.5 & 39.24 $\rightarrow$ 22.18 & -- (0/20) / -- (0/20) & 16.07\% (19/20) / -- (0/20) \\
arithmetic, unseen sets & 2B & Phi-4-mini, generalist & 32 & 63.02 & 77.85 & 74.16 & 92.4 & 0.794 & +6.8 $\rightarrow$ +14.9 & 86.91 $\rightarrow$ 64.37 & 9.46\% (4/20) / -- (0/20) & 17.34\% (18/20) / 8.5\% (0/20) \\
arithmetic, unseen sets & 4B & 27B (ours, decision) & 32 & 79.15 & 85.54 & 88.3 & 93.87 & 0.898 & +2.1 $\rightarrow$ +4.5 & 72.88 $\rightarrow$ 56.06 & 7.74\% (20/20) / 3.89\% (1/20) & 10.68\% (19/20) / 9.22\% (6/20) \\
arithmetic, unseen sets & 4B & 4B (ours, decision) & 32 & 79.15 & 85.54 & 84.83 & 93.87 & 0.828 & +4.4 $\rightarrow$ +8.8 & 85.85 $\rightarrow$ 69.34 & 10.09\% (20/20) / 3.83\% (3/20) & 14.14\% (20/20) / 8.68\% (2/20) \\
arithmetic, unseen sets & 4B & 9B (ours, decision) & 32 & 79.15 & 85.54 & 86.36 & 93.87 & 0.860 & +4.1 $\rightarrow$ +7.6 & 89.6 $\rightarrow$ 76.84 & 9.25\% (20/20) / 4.18\% (4/20) & 12.93\% (20/20) / 8.71\% (4/20) \\
arithmetic, unseen sets & 4B & base9B (base 9B, no decision training) & 32 & 79.15 & 85.54 & 85.02 & 93.87 & 0.812 & +3.2 $\rightarrow$ +7.0 & 90.3 $\rightarrow$ 76.64 & 8.02\% (15/20) / 4.35\% (3/20) & 11.15\% (20/20) / 9.12\% (4/20) \\
arithmetic, unseen sets & 4B & Clef-flash 9B, external decision & 32 & 79.15 & 85.54 & 84.26 & 93.87 & 0.815 & +3.9 $\rightarrow$ +8.0 & 81.93 $\rightarrow$ 70.29 & -- (0/20) / -- (0/20) & 14.64\% (20/20) / -- (0/20) \\
arithmetic, unseen sets & Phi-4-mini & 27B (ours, decision) & 32 & 75.35 & 80.51 & 84.92 & 89.5 & 0.924 & +3.2 $\rightarrow$ +6.3 & 83.22 $\rightarrow$ 66.63 & 8.26\% (20/20) / 4.12\% (0/20) & 11.45\% (20/20) / 9.16\% (4/20) \\
arithmetic, unseen sets & Phi-4-mini & 9B (ours, decision) & 32 & 75.35 & 80.51 & 83.15 & 89.5 & 0.887 & +4.0 $\rightarrow$ +8.5 & 94.23 $\rightarrow$ 83.31 & 8.94\% (19/20) / 4.19\% (1/20) & 13.78\% (20/20) / 8.72\% (4/20) \\
arithmetic, unseen sets & Phi-4-mini & Clef-flash 9B, external decision & 32 & 75.35 & 80.51 & 79.49 & 89.5 & 0.801 & +5.9 $\rightarrow$ +12.3 & 79.81 $\rightarrow$ 61.51 & 10.97\% (18/20) / 2.75\% (0/20) & 17.83\% (20/20) / 7.77\% (0/20) \\
arithmetic, unseen sets & Phi-4-mini & Phi-4, generalist & 32 & 75.35 & 80.51 & 78.59 & 89.5 & 0.747 & +2.7 $\rightarrow$ +7.5 & 44.54 $\rightarrow$ 34.75 & -- (0/20) / -- (0/20) & 18.17\% (10/20) / -- (0/20) \\
arithmetic, unseen sets & Gemma-3-4b & 27B (ours, decision) & 32 & 75.33 & 78.3 & 84.69 & 88.75 & 0.885 & +1.7 $\rightarrow$ +3.4 & 77.38 $\rightarrow$ 65.15 & 6.77\% (20/20) / 4.0\% (0/20) & 11.1\% (20/20) / 9.18\% (1/20) \\
arithmetic, unseen sets & Gemma-3-4b & 9B (ours, decision) & 32 & 75.33 & 78.3 & 82.83 & 88.75 & 0.836 & +2.7 $\rightarrow$ +5.8 & 87.48 $\rightarrow$ 83.25 & 6.54\% (19/20) / 3.62\% (3/20) & 12.72\% (20/20) / 8.79\% (0/20) \\
arithmetic, unseen sets & Gemma-3-4b & Phi-4, generalist & 32 & 75.33 & 78.3 & 80.0 & 88.75 & 0.739 & +0.9 $\rightarrow$ +3.9 & 43.89 $\rightarrow$ 37.88 & 11.02\% (1/20) / -- (0/20) & 14.05\% (20/20) / 12.11\% (1/20) \\
arithmetic, unseen sets & Gemma-3-12b & 27B (ours, decision) & 32 & 81.89 & 83.13 & 87.02 & 91.62 & 0.859 & +1.9 $\rightarrow$ +4.1 & 80.26 $\rightarrow$ 63.63 & 7.38\% (20/20) / 3.98\% (4/20) & 11.08\% (20/20) / 9.19\% (6/20) \\
arithmetic, unseen sets & Gemma-3-12b & 4B (ours, decision) & 32 & 81.89 & 83.13 & 84.55 & 91.62 & 0.726 & +4.0 $\rightarrow$ +7.5 & 87.45 $\rightarrow$ 74.89 & 8.99\% (20/20) / 4.34\% (3/20) & 13.95\% (20/20) / 8.94\% (6/20) \\
arithmetic, unseen sets & Gemma-3-12b & 9B (ours, decision) & 32 & 81.89 & 83.13 & 85.42 & 91.62 & 0.759 & +3.3 $\rightarrow$ +6.6 & 91.47 $\rightarrow$ 82.9 & 8.35\% (19/20) / 3.67\% (3/20) & 13.3\% (20/20) / 8.75\% (0/20) \\
arithmetic, unseen sets & Phi-4 & 27B (ours, decision) & 32 & 79.25 & 80.91 & 85.96 & 89.72 & 0.868 & +2.2 $\rightarrow$ +4.2 & 74.53 $\rightarrow$ 61.0 & 7.67\% (20/20) / 4.07\% (3/20) & 11.71\% (20/20) / 9.34\% (8/20) \\
arithmetic, unseen sets & Phi-4 & 4B (ours, decision) & 32 & 79.25 & 80.91 & 83.06 & 89.72 & 0.785 & +4.4 $\rightarrow$ +8.5 & 89.65 $\rightarrow$ 76.04 & 9.22\% (20/20) / 4.13\% (3/20) & 14.51\% (20/20) / 9.13\% (2/20) \\
arithmetic, unseen sets & Phi-4 & 9B (ours, decision) & 32 & 79.25 & 80.91 & 83.58 & 89.72 & 0.794 & +3.7 $\rightarrow$ +7.2 & 93.31 $\rightarrow$ 83.16 & 9.21\% (20/20) / 3.2\% (2/20) & 13.67\% (20/20) / 9.04\% (1/20) \\
reasoning & 0.8B & 27B (ours, decision) & 16 & 35.52 & 56.73 & 77.62 & 92.97 & 0.867 & +2.1 $\rightarrow$ +4.5 & 91.0 $\rightarrow$ 83.42 & 4.58\% (8/20) / 3.86\% (2/20) & 9.52\% (8/20) / 8.57\% (1/20) \\
reasoning & 0.8B & 4B (ours, decision) & 16 & 35.52 & 56.73 & 66.02 & 92.97 & 0.744 & +2.4 $\rightarrow$ +5.0 & 77.59 $\rightarrow$ 73.65 & 6.84\% (1/20) / -- (0/20) & 8.47\% (2/20) / 7.81\% (0/20) \\
reasoning & 0.8B & 9B (ours, decision) & 16 & 35.52 & 56.73 & 68.79 & 92.97 & 0.779 & +2.5 $\rightarrow$ +4.7 & 88.16 $\rightarrow$ 82.05 & 5.06\% (1/20) / 4.77\% (2/20) & 8.53\% (8/20) / 7.64\% (2/20) \\
reasoning & 2B & 27B (ours, decision) & 16 & 49.46 & 74.87 & 82.97 & 90.58 & 0.915 & +2.4 $\rightarrow$ +3.2 & 86.41 $\rightarrow$ 79.32 & 4.45\% (2/20) / 4.02\% (2/20) & 8.71\% (2/20) / 8.76\% (3/20) \\
reasoning & 2B & 4B (ours, decision) & 16 & 49.46 & 74.87 & 77.32 & 90.58 & 0.865 & +3.5 $\rightarrow$ +6.4 & 83.42 $\rightarrow$ 73.72 & 4.15\% (1/20) / 3.56\% (1/20) & 11.25\% (17/20) / 8.32\% (1/20) \\
reasoning & 2B & 9B (ours, decision) & 16 & 49.46 & 74.87 & 78.02 & 90.58 & 0.872 & +3.4 $\rightarrow$ +6.1 & 88.67 $\rightarrow$ 80.05 & 5.48\% (6/20) / 4.56\% (0/20) & 10.47\% (7/20) / 8.64\% (4/20) \\
reasoning & 2B & Clef 27B, external decision & 16 & 49.46 & 74.87 & 77.01 & 90.58 & 0.867 & +2.4 $\rightarrow$ +5.3 & 70.28 $\rightarrow$ 59.38 & 5.35\% (8/20) / 3.55\% (0/20) & 11.33\% (16/20) / 8.48\% (2/20) \\
reasoning & 2B & Clef-flash 9B, external decision & 16 & 49.46 & 74.87 & 67.23 & 90.58 & 0.807 & +3.1 $\rightarrow$ +9.6 & 53.19 $\rightarrow$ 45.44 & -- (0/20) / -- (0/20) & -- (0/20) / -- (0/20) \\
reasoning & 2B & Gemma-3-4b, generalist & 16 & 49.46 & 74.87 & 65.78 & 90.58 & 0.746 & +2.7 $\rightarrow$ +4.1 & 23.75 $\rightarrow$ -- & -- (0/20) / -- (0/20) & -- (0/20) / -- (0/20) \\
reasoning & 2B & Phi-4-mini, generalist & 16 & 49.46 & 74.87 & 66.45 & 90.58 & 0.783 & +5.7 $\rightarrow$ +10.8 & 56.66 $\rightarrow$ 37.7 & -- (0/20) / -- (0/20) & -- (0/20) / -- (0/20) \\
reasoning & 4B & 27B (ours, decision) & 16 & 77.65 & 88.41 & 91.88 & 95.88 & 0.914 & +1.8 $\rightarrow$ +2.3 & 83.24 $\rightarrow$ 74.48 & 4.73\% (4/20) / 4.24\% (4/20) & 7.2\% (0/20) / 7.56\% (0/20) \\
reasoning & 4B & 4B (ours, decision) & 16 & 77.65 & 88.41 & 89.18 & 95.88 & 0.848 & +2.7 $\rightarrow$ +3.8 & 81.12 $\rightarrow$ 75.4 & 6.7\% (10/20) / 4.48\% (0/20) & 9.63\% (7/20) / 8.99\% (1/20) \\
reasoning & 4B & 9B (ours, decision) & 16 & 77.65 & 88.41 & 88.94 & 95.88 & 0.856 & +2.7 $\rightarrow$ +4.2 & 85.36 $\rightarrow$ 74.76 & 6.7\% (9/20) / 4.26\% (0/20) & 9.83\% (8/20) / 8.66\% (0/20) \\
reasoning & 4B & Clef-flash 9B, external decision & 16 & 77.65 & 88.41 & 80.37 & 95.88 & 0.732 & +1.9 $\rightarrow$ +7.2 & 68.07 $\rightarrow$ 57.19 & -- (0/20) / -- (0/20) & 17.37\% (6/20) / -- (0/20) \\
reasoning & Phi-4-mini & 27B (ours, decision) & 16 & 64.09 & 73.76 & 86.69 & 97.11 & 0.863 & +2.6 $\rightarrow$ +4.0 & 88.99 $\rightarrow$ 77.79 & 5.65\% (16/20) / 4.0\% (4/20) & 10.33\% (15/20) / 8.89\% (2/20) \\
reasoning & Phi-4-mini & 4B (ours, decision) & 16 & 64.09 & 73.76 & 79.73 & 97.11 & 0.757 & +4.0 $\rightarrow$ +6.8 & 81.69 $\rightarrow$ 71.41 & 4.06\% (3/20) / 3.57\% (3/20) & 11.68\% (18/20) / 8.59\% (3/20) \\
reasoning & Phi-4-mini & 9B (ours, decision) & 16 & 64.09 & 73.76 & 82.25 & 97.11 & 0.794 & +3.4 $\rightarrow$ +5.9 & 91.05 $\rightarrow$ 81.75 & 6.46\% (4/20) / 3.56\% (0/20) & 11.45\% (17/20) / 8.51\% (2/20) \\
reasoning & Gemma-3-4b & 27B (ours, decision) & 16 & 69.51 & 72.8 & 84.47 & 92.85 & 0.823 & +2.6 $\rightarrow$ +4.0 & 89.93 $\rightarrow$ 81.57 & 6.51\% (20/20) / 4.15\% (5/20) & 10.75\% (18/20) / 9.15\% (4/20) \\
reasoning & Gemma-3-4b & 4B (ours, decision) & 16 & 69.51 & 72.8 & 79.99 & 92.85 & 0.727 & +3.9 $\rightarrow$ +6.4 & 83.06 $\rightarrow$ 72.03 & 6.21\% (18/20) / 4.06\% (2/20) & 13.01\% (20/20) / 8.51\% (0/20) \\
reasoning & Gemma-3-4b & 9B (ours, decision) & 16 & 69.51 & 72.8 & 81.3 & 92.85 & 0.759 & +3.8 $\rightarrow$ +6.2 & 91.88 $\rightarrow$ 83.0 & 7.09\% (5/20) / 4.11\% (0/20) & 13.19\% (20/20) / 7.97\% (4/20) \\
reasoning & Gemma-3-12b & 27B (ours, decision) & 16 & 80.47 & 83.07 & 89.55 & 95.07 & 0.816 & +2.1 $\rightarrow$ +2.9 & 88.03 $\rightarrow$ 78.91 & 5.76\% (19/20) / 4.26\% (0/20) & 8.66\% (0/20) / 8.62\% (0/20) \\
reasoning & Gemma-3-12b & 4B (ours, decision) & 16 & 80.47 & 83.07 & 85.57 & 95.07 & 0.706 & +3.5 $\rightarrow$ +5.9 & 85.09 $\rightarrow$ 69.69 & 6.55\% (13/20) / 3.94\% (0/20) & 12.36\% (20/20) / 8.69\% (3/20) \\
reasoning & Gemma-3-12b & 9B (ours, decision) & 16 & 80.47 & 83.07 & 86.86 & 95.07 & 0.736 & +3.2 $\rightarrow$ +5.0 & 92.59 $\rightarrow$ 82.79 & 7.43\% (2/20) / 4.05\% (0/20) & 11.48\% (19/20) / 8.75\% (0/20) \\
reasoning & Phi-4 & 27B (ours, decision) & 16 & 82.39 & 85.15 & 90.25 & 94.99 & 0.845 & +2.0 $\rightarrow$ +3.2 & 87.66 $\rightarrow$ 75.53 & 5.81\% (16/20) / 4.03\% (2/20) & 8.56\% (0/20) / 8.51\% (0/20) \\
reasoning & Phi-4 & 4B (ours, decision) & 16 & 82.39 & 85.15 & 87.11 & 94.99 & 0.736 & +3.4 $\rightarrow$ +5.7 & 81.58 $\rightarrow$ 62.87 & 6.9\% (19/20) / 3.85\% (0/20) & 11.56\% (19/20) / 8.57\% (2/20) \\
reasoning & Phi-4 & 9B (ours, decision) & 16 & 82.39 & 85.15 & 88.61 & 94.99 & 0.775 & +2.9 $\rightarrow$ +4.4 & 90.52 $\rightarrow$ 77.98 & 6.6\% (18/20) / 3.73\% (0/20) & 10.47\% (13/20) / 8.51\% (1/20) \\
reasoning, N=32 & 2B & 27B (ours, decision) & 32 & 49.45 & 76.05 & 85.64 & 93.92 & 0.913 & +2.6 $\rightarrow$ +3.8 & 86.91 $\rightarrow$ 78.19 & 4.59\% (4/20) / 3.85\% (0/20) & 8.92\% (0/20) / 8.65\% (2/20) \\
reasoning, N=32 & 2B & 9B (ours, decision) & 32 & 49.45 & 76.05 & 80.73 & 93.92 & 0.873 & +3.5 $\rightarrow$ +6.7 & 88.81 $\rightarrow$ 79.78 & 5.77\% (6/20) / 4.15\% (0/20) & 10.22\% (10/20) / 8.46\% (1/20) \\
reasoning, N=32 & 4B & 27B (ours, decision) & 32 & 77.69 & 89.03 & 92.74 & 97.19 & 0.918 & +1.8 $\rightarrow$ +2.6 & 82.25 $\rightarrow$ 72.52 & 5.01\% (10/20) / 4.1\% (2/20) & 7.01\% (0/20) / 7.23\% (0/20) \\
reasoning, N=32 & 4B & 9B (ours, decision) & 32 & 77.69 & 89.03 & 88.88 & 97.19 & 0.862 & +2.7 $\rightarrow$ +5.5 & 85.58 $\rightarrow$ 73.46 & 7.65\% (13/20) / 3.79\% (1/20) & 10.55\% (18/20) / 8.95\% (5/20) \\
question answering & 2B & 27B (ours, decision) & 16 & 10.79 & 16.88 & 23.67 & 32.06 & 0.874 & +2.2 $\rightarrow$ +6.9 & 58.41 $\rightarrow$ 42.59 & -- (0/20) / -- (0/20) & -- (0/20) / -- (0/20) \\
question answering & 2B & 4B (ours, decision) & 16 & 10.79 & 16.88 & 20.55 & 32.06 & 0.816 & +4.7 $\rightarrow$ +12.7 & 41.79 $\rightarrow$ 20.92 & -- (0/20) / -- (0/20) & -- (0/20) / -- (0/20) \\
question answering & 2B & 9B (ours, decision) & 16 & 10.79 & 16.88 & 21.41 & 32.06 & 0.835 & +4.4 $\rightarrow$ +12.5 & 60.09 $\rightarrow$ 41.61 & -- (0/20) / -- (0/20) & -- (0/20) / -- (0/20) \\
question answering & 4B & 27B (ours, decision) & 16 & 23.97 & 30.88 & 33.59 & 45.25 & 0.806 & +6.0 $\rightarrow$ +13.2 & 57.8 $\rightarrow$ 37.51 & -- (0/20) / -- (0/20) & -- (0/20) / -- (0/20) \\
question answering & 4B & 4B (ours, decision) & 16 & 23.97 & 30.88 & 31.01 & 45.25 & 0.742 & +8.7 $\rightarrow$ +17.5 & 38.98 $\rightarrow$ 15.8 & -- (0/20) / -- (0/20) & -- (0/20) / -- (0/20) \\
question answering & 4B & 9B (ours, decision) & 16 & 23.97 & 30.88 & 32.29 & 45.25 & 0.765 & +8.4 $\rightarrow$ +17.0 & 54.3 $\rightarrow$ 31.18 & -- (0/20) / -- (0/20) & -- (0/20) / -- (0/20) \\
question answering & Phi-4-mini & 27B (ours, decision) & 16 & 22.38 & 29.18 & 35.29 & 48.09 & 0.826 & +4.5 $\rightarrow$ +10.6 & 56.12 $\rightarrow$ 38.27 & -- (0/20) / -- (0/20) & -- (0/20) / -- (0/20) \\
question answering & Phi-4-mini & 4B (ours, decision) & 16 & 22.38 & 29.18 & 31.84 & 48.09 & 0.772 & +6.3 $\rightarrow$ +14.6 & 44.98 $\rightarrow$ 24.43 & -- (0/20) / -- (0/20) & -- (0/20) / -- (0/20) \\
question answering & Phi-4-mini & 9B (ours, decision) & 16 & 22.38 & 29.18 & 33.38 & 48.09 & 0.795 & +6.1 $\rightarrow$ +13.6 & 52.89 $\rightarrow$ 33.13 & -- (0/20) / -- (0/20) & -- (0/20) / -- (0/20) \\
question answering & Gemma-3-12b & 27B (ours, decision) & 16 & 38.8 & 40.31 & 41.9 & 49.88 & 0.704 & +5.1 $\rightarrow$ +9.7 & 56.12 $\rightarrow$ 41.69 & -- (0/20) / -- (0/20) & 7.9\% (1/20) / 7.14\% (0/20) \\
question answering & Gemma-3-12b & 4B (ours, decision) & 16 & 38.8 & 40.31 & 40.46 & 49.88 & 0.627 & +6.0 $\rightarrow$ +11.7 & 50.31 $\rightarrow$ 32.61 & -- (0/20) / -- (0/20) & -- (0/20) / -- (0/20) \\
question answering & Gemma-3-12b & 9B (ours, decision) & 16 & 38.8 & 40.31 & 41.1 & 49.88 & 0.665 & +6.3 $\rightarrow$ +11.8 & 55.75 $\rightarrow$ 39.76 & -- (0/20) / -- (0/20) & -- (0/20) / -- (0/20) \\
question answering & Phi-4 & 27B (ours, decision) & 16 & 39.58 & 45.3 & 44.4 & 59.84 & 0.719 & +6.4 $\rightarrow$ +12.8 & 54.21 $\rightarrow$ 37.67 & -- (0/20) / -- (0/20) & 9.09\% (0/20) / 11.04\% (1/20) \\
question answering & Phi-4 & 4B (ours, decision) & 16 & 39.58 & 45.3 & 42.95 & 59.84 & 0.662 & +7.1 $\rightarrow$ +14.2 & 48.94 $\rightarrow$ 29.69 & -- (0/20) / -- (0/20) & -- (0/20) / -- (0/20) \\
question answering & Phi-4 & 9B (ours, decision) & 16 & 39.58 & 45.3 & 43.59 & 59.84 & 0.684 & +7.2 $\rightarrow$ +13.9 & 51.63 $\rightarrow$ 35.61 & -- (0/20) / -- (0/20) & -- (0/20) / 10.39\% (1/20) \\
\end{longtable}
\endgroup

\todo{Table B.2 is announced in v4 (part2.md:75) and not printed there (part3b.md:838-839). The rows
are copied from the table file tables/bon\_grid\_all\_runs.md (126 rows), with empty values shown as
a dash; they agree with Table B.1 in all cells but one (Gemma-3-12b-it on the unseen datasets:
overconfidence +3.5 $\rightarrow$ +9.2 here, +3.6 $\rightarrow$ +9.3 in Table B.1) and with the 113
points of Figure B.3. Of the 126 rows, 113 are at N = 16 in Figure B.3; the other 13 are the same
pairs at N = 256 or N = 32 --- say so where ``126'' is quoted.}

\todo{also announced in v4 and not written (part3b.md:838-839, 844-845): every certificate with its
20 splits; the runs with N = 256 on held-out and unseen problems as tables; fine-tuning a verifier
and why training on its own selection distribution does not help; adaptive sampling; closed-book
question answering by generator. Write from the table files or drop the pointers.}
