# Supplementary material for: StartLux-Decision: AutoThink Decision Models with Reinforcement Learning for Calibrated Deliberative Decisions
Source: arXiv:2610.17309 source file (2026-10-20)
Supplement: Supplementary file 4 [file appendix_C_gates_cascades.tex]

\clearpage
\section{Think-gates, cascades, select-then-think: details}\label{sec:C}

Here are the details behind the routing results of Section~\ref{sec:7.3}: the protocol, every row of
the matched-confidence comparison, the residual AUROC by model, the reversals, the one decision
model with almost no effect, cascades, and the policy in which one model selects among samples and
then reasons. Certificates for these policies are in Table~\ref{tab:D.1} and the calibration maps in
Appendix~\ref{sec:D}.

\subsection{Protocol}\label{sec:C.1}

\textbf{Policies.} A think-gate reasons if and only if the plain confidence c0 is below a threshold
and reports the thought answer with its confidence c1. A cascade escalates if and only if the small
model's confidence is below a threshold and reports the large model's answer with the large model's
confidence (A.1). A \emph{think rate} of 30\% means that the least confident 30\% of the items are
routed. Cascades are reported at a threshold of .7 (Table~\ref{tab:C.1}) and, in the calibration
experiment of Appendix~\ref{sec:D.5}, with 30\% of the items escalated. \todo{the think-gate
analysed here reports the thought distribution alone (v4 part2.md:11-12); the default control of
Section 3.4 averages the plain and the thought distribution (v4 part1.md:337-338,
part3b.md:813-814). v4 gives no matched-confidence comparison for the averaged distribution; say so
in Section 3.4 or measure it.}

\textbf{Measures.} The \emph{route effect} is the accuracy of the reported answer at matched
reported confidence, routed items minus kept items. A negative value means that the routed answers
are overconfident relative to the kept ones. The \emph{residual AUROC} is the AUROC of the routing
confidence for the correctness of the reported answer within quintiles of the reported confidence
(A.3). Intervals are 95\%. \todo{v4 does not say how confidence is matched between routed and kept
items, nor how the intervals are obtained; add one sentence from the analysis script.}

\textbf{Items.} Three item sets.

\begin{itemize}
\item \emph{The decision suite:} 5,710 diagnostic decisions of 39 task families, of the type of the index
benchmarks (150 per family, not held-out families).
\item \emph{Reasoning items:} 4,648 reasoning decisions.
\item \emph{A third-party benchmark,} CJ-Bench: 304,822 hard decisions in Chinese (general, medical,
legal, finance), and a stratified subset of 47,298 decisions on which nine models were run.
\end{itemize}

\todo{v4 counts the third-party benchmark as 307,900 decisions in the abstract (part1.md:17) and as
304,822 hard decisions here (part2.md:156); say how the second is obtained from the first. Also add
the in-domain marker required for every table: which of the 39 families have training data in the
mix of the model under test (v4 Table 9, part3a.md:428-459).}

\textbf{Models.} StartLux-Decision-4B and $-$9B as one model that decides and reads its own
reasoning (``single model''). Generalist chat models with zero-shot chain of thought: Phi-4 (14B),
Gemma-3-12b, Phi-4-mini and Gemma-3-4b. Reasoning models, for which the plain answer is the answer
after an empty think block: DeepSeek-R1-Distill-Llama-8B and Phi-4-mini-reasoning. Jeeves-9B,
another team's decision model with a built-in think gate. Three controls: the two base models ours
are tuned from, reading their own reasoning, and Granite-3.3-2b. Models of other teams were run by
us from their public weights and code in the documented configuration. We made no ablation of
another team's model. \todo{name the checkpoints behind ``single model'' --- released weights with a
reader round, or models after data rounds. v4 says only ``ours 4B / 9B single model''
(part2.md:153); Appendix F (v4 Table G2, part3b.md:789-804) lists reader rounds on later bases
only.}

\subsection{All rows}\label{sec:C.2}

At equal reported confidence, an answer that was reasoned about because the plain confidence was low
is less accurate than an answer that was kept, for eleven of twelve models on the decision suite and
for every model on the third-party benchmark. On reasoning items the sign is mixed.
Table~\ref{tab:C.1} has all fifteen rows, and Table~\ref{tab:7.1}b is a selection.

\begingroup
\renewcommand{\thetable}{C.1}
\footnotesize\setlength{\tabcolsep}{5pt}\renewcommand{\arraystretch}{1.1}
\begin{longtable}{>{\raggedright\arraybackslash}p{\mdw{0.1232}}>{\raggedright\arraybackslash}p{\mdw{0.2500}}>{\raggedright\arraybackslash}p{\mdw{0.2012}}>{\raggedright\arraybackslash}p{\mdw{0.4119}}}
\caption{Accuracy of the reported answer at matched reported confidence, routed minus kept (negative = routed overconfident), with 95\% intervals in brackets where they were computed. ``Ours'' = StartLux-Decision models, ``single model'' = one model that decides and reads its own reasoning. Own runs.}\label{tab:C.1}\\
\toprule
\textbf{pipeline} & \textbf{models} & \textbf{items} & \textbf{value {[}95\%{]}} \\
\midrule
\endfirsthead
\multicolumn{4}{l}{\textit{Table~\thetable{} (continued)}}\\
\toprule
\textbf{pipeline} & \textbf{models} & \textbf{items} & \textbf{value {[}95\%{]}} \\
\midrule
\endhead
\bottomrule
\endfoot
think-gate, 30\% think rate & ours 4B / 9B single model & 5,710 decisions, 39 families & $-$.194 {[}$-$.230, $-$.158{]} / $-$.214 {[}$-$.254, $-$.171{]} \\
think-gate, 30\% & Phi-4 (14B) / Gemma-3-12b / Phi-4-mini / Gemma-3-4b, zero-shot chain of thought & same & $-$.176 {[}$-$.203, $-$.149{]} / $-$.112 {[}$-$.138, $-$.086{]} / $-$.099 {[}$-$.126, $-$.070{]} / $-$.028 {[}$-$.057, .000{]} \\
think-gate, 30\% & DeepSeek-R1-Distill-Llama-8B / Phi-4-mini-reasoning (reasoning models, plain = empty think block) & same & $-$.082 {[}$-$.109, $-$.051{]} / $-$.038 {[}$-$.066, $-$.012{]} \\
think-gate, 30\% & Jeeves-9B (another team's decision model with a built-in think gate) & same & $-$.037 {[}$-$.071, $-$.006{]} \\
think-gate, 10\% / 20\% / 40\% & ours 4B single model & CJ-Bench, 304,822 hard decisions (Chinese: general, medical, legal, finance) & $-$.114 {[}$-$.122, $-$.108{]} / $-$.163 {[}$-$.168, $-$.156{]} / $-$.241 {[}$-$.245, $-$.236{]} \\
think-gate, 10\% / 20\% / 40\% & ours 9B single model & same & $-$.168 {[}$-$.175, $-$.161{]} / $-$.190 {[}$-$.197, $-$.183{]} / $-$.240 {[}$-$.244, $-$.235{]} \\
think-gate, 30\% / 50\% & Phi-4-mini / Gemma-3-4b / Gemma-3-12b / Phi-4-mini-reasoning & 4,648 reasoning decisions & $-$.051 / $-$.105, $-$.041 / $-$.072, $-$.044 / $-$.029, $-$.069 / $-$.043 (all intervals exclude zero) \\
think-gate, 30\% / 50\% & ours 9B single model & same & $-$.011 {[}$-$.033, +.015{]} / $-$.050 {[}$-$.070, $-$.032{]} \\
think-gate, 30\% / 50\% & ours 4B single model, Jeeves-9B, Phi-4, R1-Distill-Llama-8B & same & \textbf{+.057 / +.021, +.032 / +.025, +.055 / +.009, +.075 / +.076} (reversed) \\
think-gate, 20\% think rate & nine models on the same items & 47,298 CJ-Bench decisions (stratified subset) & R1-distill $-$.272, Phi-4-mini $-$.268, Phi-4 $-$.248, Gemma-3-12b $-$.212, ours 9B $-$.168, ours 4B $-$.137, Phi-4-mini-reasoning $-$.122, Gemma-3-4b $-$.121, Jeeves $-$.033 {[}$-$.047, $-$.018{]} (every interval excludes zero) \\
think-gate, 30\% & controls: the two base models ours are tuned from (base 9B / base 4B, own reasoning), Granite-3.3-2b & 5,710 decisions & $-$.069 {[}$-$.099, $-$.040{]} / +.021 {[}$-$.006, +.052{]}, $-$.178 {[}$-$.204, $-$.149{]} \\
think-gate, 30\% & same controls & 4,648 reasoning decisions & +.017 {[}+.002, +.034{]} / +.029 {[}+.010, +.046{]}, $-$.113 {[}$-$.142, $-$.083{]} \\
think-gate, 20\% & same controls & 47,298 CJ-Bench decisions & $-$.130 {[}$-$.142, $-$.119{]} / $-$.109 {[}$-$.118, $-$.098{]}, $-$.230 {[}$-$.241, $-$.220{]} \\
cascade, $\tau$ = .7 & Clef-flash $\rightarrow$ Clef 27B (another team) & 5,710 decisions & $-$.123 {[}$-$.164, $-$.083{]} \\
cascade, $\tau$ = .7 & ours 4B $\rightarrow$ ours 27B, ours 4B $\rightarrow$ Clef 27B, Clef-flash $\rightarrow$ ours 27B & same & $-$.139, $-$.160, $-$.154 \\
\end{longtable}
\endgroup

\subsection{What the route effect is made of}\label{sec:C.3}

The route effect is the information the routing confidence keeps about the thought answer once the
thought confidence is known. On the decision suite the residual AUROC is

\begin{itemize}
\item .69 and .64 for our 9B and 4B (matched difference $-$.214, $-$.194),
\item .63--.65 for Phi-4 and Granite-3.3-2b ($-$.176, $-$.178),
\item .55--.59 for Gemma-3-12b, Phi-4-mini, R1-distill, Jeeves and the base 9B ($-$.112 \ldots{} $-$.037),
\item .49--.50 for Gemma-3-4b, Phi-4-mini-reasoning and the base 4B ($-$.038 \ldots{} +.021).
\end{itemize}

One line fits all three item sets (slope $-$0.91 per unit of AUROC). Cascades obey it too, with the
small model's confidence in the role of the routing score and the large model's answer as the
reported one: ten pairs of a small and a large model (ours and another team's) have residual AUROCs
of .58--.71 and matched differences of $-$.10 to $-$.17, on average .04 above the line fitted to the
gates (with them 46 points, Spearman $-$0.87).

\todo{the residual AUROC is given for ten cascade pairs here (part2.md:171-173, part3b.md:464-466)
and the calibration map of Appendix D.5 is tested on seven pairs (part2.md:351, 361); v4 does not
say that these are different sets of pairs. The table files show six pairs in common.}

\subsection{Findings in detail}\label{sec:C.4}

\textbf{Decision training makes the route effect larger.} The base models that our decision models
are tuned from show little of it on the decision suite (base 9B $-$.069, base 4B +.021). After
decision training it is $-$.214 and $-$.194 ($-$.203 {[}$-$.243, $-$.160{]} and $-$.226 {[}$-$.258,
$-$.188{]} when ours are given the base models' 1,024-token budget, residual AUROC .67 and .63
against .57 and .50). On the third-party benchmark, where the base models already have it ($-$.130
and $-$.109), the step is smaller ($-$.168 and $-$.137). Decision training sharpens the plain
confidence (its AUROC for the plain answer rises from .78 to .87 at 9B and from .72 to .85 at 4B),
and the thought confidence does not absorb what the plain one now knows. The better the routing
signal, the larger the bias of what is reported after routing.

\textbf{The reversals are the same law with the sign of the premise flipped.} On the reasoning items
the residual AUROC is below .5 for our 4B (.39), Jeeves (.37), R1-distill (.43) and both base models
(.36, .41). A low plain confidence there marks items that thinking solves, and their matched
difference is positive. It is above .5 for Gemma-3-12b, Phi-4-mini, Gemma-3-4b and Granite
(.55--.58), which are negative. Among the first nine models at a 30\% think rate, four are negative,
one is null and four are positive (our 4B, Jeeves, Phi-4 and R1-distill). Thinking lifts our 4B from
59.6\% to 86.5\%. The routed items are those the model knows it cannot answer at a glance, and the
kept items carry the residual errors. In ProofWriter the thought answers are overconfident by +.205
on kept against +.109 on routed items, and a confident plain answer that is wrong stays wrong after
thinking. The premise of Proposition 2 holds there with the opposite sign, and so does its
conclusion. The reported confidence is route-dependent either way.

\textbf{The third-party benchmark by domain shows the same pattern.} At a 20\% think rate (4B):
medical $-$.203 {[}$-$.211, $-$.195{]}, general $-$.151 {[}$-$.161, $-$.141{]}, finance $-$.137
{[}$-$.181, $-$.095{]}, legal $-$.025 {[}$-$.065, +.007{]}. Legal is the domain where thinking helps
most (63.5\% $\rightarrow$ 72.3\%), the same pattern as the reversal above.

\textbf{One decision model has almost none.} Jeeves' thought confidence absorbs most of what its
plain confidence knows (residual AUROC .56 on the decision suite and .57 on the benchmark, with a
plain confidence as sharp as ours: AUROC .83). Its thought answers on routed items are overconfident
by +.06 (the other eight models: +.17 to +.45), the matched difference is $-$.037 (not significant
at a 50\% think rate), and one threshold at $\alpha$ = .10 is not violated (at $\alpha$ = .25 it is,
in 18--20 of 20 splits). Its reasoning was trained by reinforcement learning with the probability of
the correct option after thinking as reward, on data with unknowable items. The route-dependence is
therefore a property of how the confidence after thinking was trained, not a law of gates, which is
consistent with Appendix~\ref{sec:E} (E.8, E.9), where calibrating the thought path on real-task
items reduces it.

The attribution to its training is a hypothesis. We ran no ablation of another team's model. Our
closest experiment does not support the simple version of it: in a two-model baseline (a separate
reasoner, our 4B as reader), training the reasoner alone by reinforcement learning with the reader's
proper score as reward leaves the matched difference where it was, $-$.279 {[}$-$.311, $-$.248{]}
before and $-$.272 {[}$-$.302, $-$.243{]} after 100 iterations. Expert iteration, which shortens the
reasoning, moves it to $-$.220. If training is the cause, it is the joint training of the readout,
which that experiment kept frozen.

\textbf{Fusing the two readouts is not the answer.} A product p0\textasciicircum{}a
\textperiodcentered{} p1\textasciicircum{}b fitted by likelihood puts a at 0--0.2 for every one of
twelve models and leaves the accuracy of the thought answer unchanged. What the plain confidence
adds is knowledge of how hard the item is, not of which option is right. Its place is in the
calibration map (Appendix~\ref{sec:D.4}). A learned, input-dependent choice between the two answers
(a classifier on both distributions, cross-fitted over task families) gains +0.3 points over the
thought answer on the 4B and on the 9B, not significantly, where an oracle choice would gain 2.8 to
3.0. Its fused confidence is calibrated on both routes (+0.7 / $-$1.1 and +0.4 / $-$0.8 points on
routed / kept items, against +4.0 / $-$2.2 and +3.5 / $-$1.9 for the usual map). Training the
readout to see the plain answer would buy the calibration that the map already gives, and no
accuracy.

\textbf{Generalist chat models cannot be certified.} At no level up to 25\% on the decision suite
(raw overconfidence +.35 to +.45), with or without routing.

\subsection{Select, then think}\label{sec:C.5}

One model can select among samples and then reason about its favourites. It gains accuracy at every
size we ran, and the route it adds is the one whose confidence can be trusted least.

\textbf{Accuracy.} Table~\ref{tab:C.2} lists the settings. With the 4B single model as verifier of
64 samples and a 256-token budget, reasoning about its three favourites raises accuracy from 92.3 to
93.5 at 316 reasoning tokens per problem, and reasoning about every candidate to 94.2 (2B
generator). The 9B model does the same one size up, at about 700 reasoning tokens per problem for
the top three, and reaches the level of the fast 27B verifier. The gain holds on the reasoning sets
and on the unseen datasets, where every step is significant.

\begin{table}[!htbp]
\renewcommand{\thetable}{C.2}
\centering
\caption{Select-then-think: accuracy (\%) of the returned answer when the verifier answers in one pass (``fast''), reasons about its three favourites, or reasons about every candidate. One model verifies and reasons. Paired differences to ``fast'' with 95\% intervals where they were computed. ``--'' = not reported. Own runs.}\label{tab:C.2}
{\footnotesize\setlength{\tabcolsep}{4pt}\renewcommand{\arraystretch}{1.1}
\noindent\begin{adjustbox}{max width=\linewidth}
\begin{tabular}{llrrrrrr}
\toprule
{\begin{tabular}[b]{@{}l@{}}\textbf{verifier}\\\textbf{that also}\\\textbf{reasons}\end{tabular}} & \textbf{problems, generator, N} & \textbf{fast} & {\begin{tabular}[b]{@{}r@{}}\textbf{top}\\\textbf{three}\end{tabular}} & {\begin{tabular}[b]{@{}r@{}}\textbf{all}\\\textbf{candidates}\end{tabular}} & {\begin{tabular}[b]{@{}r@{}}\textbf{fast verifier}\\\textbf{one size up}\end{tabular}} & \textbf{top three $-$ fast} & \textbf{all $-$ fast} \\
\midrule
4B & held-out, 2B, 64 & 92.28 & 93.54 & 94.21 & -- & -- & -- \\
4B & held-out, 0.8B, 64 & 86.84 & 88.83 & 90.38 & 9B: 88.39 & -- & -- \\
9B & held-out, 2B, 64 & 94.42 & 95.10 & 95.42 & 27B: 95.48 & +0.68 {[}+0.19, +1.20{]} & +1.00 {[}+0.48, +1.55{]} \\
9B & held-out, 0.8B, 64 & 88.97 & 90.81 & 91.23 & 27B: 90.97 & +1.84 {[}+1.14, +2.61{]} & +2.25 {[}+1.45, +3.10{]} \\
9B & reasoning sets, N = 8 & 74.36 & 75.43 & -- & -- & -- & -- \\
4B & unseen datasets, 0.8B, 8 & 70.53 & 71.88 & 72.26 & 27B: 73.74 & -- & -- \\
9B & unseen datasets, 0.8B, 8 & 72.35 & 73.22 & 73.43 & 27B: 73.74 & -- & -- \\
\bottomrule
\end{tabular}
\end{adjustbox}\par}
\end{table}

\textbf{Reported confidence by route.} The price is the reported confidence. After calibration on
single responses, on the held-out problems the thought route of the 4B is overconfident by +1.1 (N =
2) $\rightarrow$ +5.7 (N = 64) with the 2B generator and by +1.0 $\rightarrow$ +10.4 with the 0.8B
generator, and its fast route by +0.3 to +1.8. For the 9B the thought route is at +1.2 $\rightarrow$
+4.2 and +0.4 $\rightarrow$ +8.0 (N = 2 $\rightarrow$ 64) and the fast route at +0.3 to +0.8. On the
unseen datasets the thought route is at its worst: overconfident by +2.8 $\rightarrow$ +13.7 (4B)
and +2.3 $\rightarrow$ +11.2 (9B) from N = 2 to 8, against +0.9 to +1.7 on the fast route. One
threshold at $\alpha$ = .10 lets thought answers through at 22--24\% error at N = 2 (15 and 20 of 20
splits), while per route no thought answer is accepted and the fast answers are certified (52--56\%
coverage). Table~\ref{tab:D.1} has the certificate rows for the reasoning sets, and
Appendix~\ref{sec:D.5} the calibration map for this policy. \todo{v4 speaks of a ``thought route''
and a ``fast route'' of select-then-think (part2.md:213-217, part3b.md:516-526) without saying which
problems take which; the table files (tables/think\_verify\_{*}.txt, section C) give these numbers
for ``gated top-3 at a 50\% think rate''. State the rule.}

\subsection{Serving path of the diagnostic readouts}\label{sec:C.6}

The diagnostic readouts behind Chapter~\ref{sec:7} and Appendices~\ref{sec:B} to \ref{sec:E} were
produced by an offline engine. That engine has the same default as the inference server described in
Section~\ref{sec:8.4}: it prefills prompts in chunks, and for this architecture a prompt whose
prefill is split between two scheduler steps is read wrongly. We re-read the stored traces of the 4B
and the 9B with the prefill in one piece. The top option changes in 0.4--0.9\% of the answers, a
probability moves by more than 0.05 in 0.02--0.14\% of them, the accuracy stays within 0.1 points,
and the route effect at matched confidence stays where it was ($-$.093 and $-$.094 at 4B, $-$.103
and $-$.102 at 9B). The results of Chapter~\ref{sec:7} therefore stand as measured: its numbers are
those of the original readouts, and the check covers the stored traces of the 4B and the 9B.
\todo{the route effects quoted for the re-read ($-$.093 / $-$.103, part3a.md:415-416) are not the
values of Table C.1 ($-$.194 / $-$.214, part2.md:153); say which traces and which think rate were
re-read.}

\subsection{Not yet written out}\label{sec:C.7}

Per-model tables for the three item sets are not part of this draft. \todo{v4 announces, and does
not contain (part3b.md:840-841), per-model tables for the decision suite, the reasoning items and
the third-party benchmark, the residual AUROC for every pair of a model and an item set, and the
budget-matched comparison with the base models in full. Write from the table files
(tables/gate\_info\_\emph{.txt, tables/think\_gate\_}.txt) or drop the pointers.}
