# Supplementary material for: StartLux-Decision: AutoThink Decision Models with Reinforcement Learning for Calibrated Deliberative Decisions
Source: arXiv:2610.17309 source file (2026-10-20)
Supplement: Supplementary file 5 [file appendix_C_stage2_ablations.tex]

\section{Stage 2 ablations and what did not work}\label{sec:C}

Each row of Table~\ref{tab:C.1} is one 4B adapter round on the v1 weights with the settings of the
round on the earlier mix, changed only in what the row names.

\subsection{Measures and the spread between runs}\label{sec:C.1}

Five measures read each round: Decision Index 0.2.1, the plain mean of the 20 twin test sets, the 35
reused tasks of DecisionPivot on unseen items, three generated tasks of DecisionPivot (accuracy, chance
50), and the skill on the rebuilt GSM8K rows. A second run of the earlier-mix round moved single
twins by up to 4.9 points and the reused tasks by $-$0.7, more than the paired interval over items
allows. We read a change on the reused tasks as real only beyond about one point, and on a single
twin only beyond about five.

\begingroup
\renewcommand{\thetable}{C.1}
\footnotesize\setlength{\tabcolsep}{5pt}\renewcommand{\arraystretch}{1.1}
\begin{longtable}{>{\raggedright\arraybackslash}p{\mdw{0.4354}}>{\raggedleft\arraybackslash}p{\mdw{0.0701}}>{\raggedleft\arraybackslash}p{\mdw{0.0696}}>{\raggedleft\arraybackslash}p{\mdw{0.1299}}>{\raggedleft\arraybackslash}p{\mdw{0.1511}}>{\raggedleft\arraybackslash}p{\mdw{0.1307}}}
\caption{A group of data helps only the task families it contains, and bidirectional attention over the prompt is the one change that raised every measure without new data. Ablations at 4B, one pass. Reused tasks: paired difference to the earlier-mix round with its 95\% bootstrap interval over items. Generated tasks: answerable facts / filter match / tool-call validity.}\label{tab:C.1}\\
\toprule
\textbf{4B checkpoint} & \textbf{index} & \textbf{twins} & \textbf{reused tasks} & \textbf{generated tasks} & \textbf{rebuilt GSM8K} \\
\midrule
\endfirsthead
\multicolumn{6}{l}{\textit{Table~\thetable{} (continued)}}\\
\toprule
\textbf{4B checkpoint} & \textbf{index} & \textbf{twins} & \textbf{reused tasks} & \textbf{generated tasks} & \textbf{rebuilt GSM8K} \\
\midrule
\endhead
\bottomrule
\endfoot
\mdourrow StartLux-Decision-4B (v1) & 52.76 & 61.9 & -- & 65.5 / 57.5 / 56.0 & 37.2 \\
Stage 2 on the earlier mix & 64.78 & 61.6 & 0 & 61.5 / 63.2 / 57.2 & 23.0 \\
\ldots{} second run, mix sampled again & 64.91 & 61.8 & $-$0.7 {[}$-$1.3, 0.0{]} & 59.7 / 64.0 / 57.0 & 25.2 \\
\midrule
\multicolumn{6}{l}{\emph{one group added or removed}} \\
+ our procedural families (97,001 rows) & 65.03 & 61.7 & $-$0.5 {[}$-$1.2, +0.2{]} & 75.8 / 66.3 / 67.0 & 28.3 \\
+ benchmark-source families (143,157) & 65.04 & 61.8 & +1.9 {[}+1.1, +2.6{]} \textsuperscript{f} & 61.2 / 62.7 / 57.2 & 26.4 \\
+ six weak-area training sets (117,167) & 65.14 & 64.4 \textsuperscript{f} & $-$1.5 {[}$-$2.3, $-$0.9{]} \textsuperscript{f} & 59.0 / 62.5 / 58.0 & 34.1 \\
$-$ the 13,776 rows of VAST & 64.77 & 61.6 & $-$0.3 {[}$-$0.8, +0.3{]} & 58.7 / 65.2 / 56.5 & 28.9 \\
+ twin-reserved families at all rows (121,204), breadth and single-skill files & 65.16 & 65.6 \textsuperscript{f} & $-$1.0 {[}$-$1.7, $-$0.3{]} & 61.7 / 65.2 / 60.2 & 28.1 \\
+ public procedural corpus (90,000 rows, 10 families) & 65.69 & 62.4 & $-$0.6 {[}$-$1.2, 0.0{]} & 59.3 / 64.0 / 57.3 & 21.9 \\
+ original training splits of twin sources (368,053) & 65.00 & 69.7 \textsuperscript{f} & $-$2.0 {[}$-$2.7, $-$1.2{]} & 59.7 / 64.7 / 58.3 & 24.7 \\
+ stance and sarcasm contrast pairs, filtered (8,859) & 64.74 & 63.2 & +0.1 {[}$-$0.5, +0.8{]} & $-$3.2 / $-$0.2 / +2.5 \textsuperscript{d} & 23.1 \\
+ the same pairs, unfiltered (16,036) & 65.16 & 61.4 & $-$0.3 {[}$-$0.9, +0.4{]} & 58.8 / 62.2 / 59.0 & -- \\
hygiene package: GSM8K rows replaced, ANLI and select-all cut, 45 groups dropped & 64.11 & 62.7 & $-$1.0 {[}$-$1.7, $-$0.2{]} & level \textsuperscript{d} & 51.1 \\
full coverage & 64.82 & 67.6 \textsuperscript{f} & +0.8 {[}+0.1, +1.7{]} \textsuperscript{f} & 77.3 / 66.8 / 68.2 & 33.3 \\
full coverage, from Stage 1 alone & 65.39 & 67.6 \textsuperscript{f} & +1.7 {[}+1.0, +2.5{]} \textsuperscript{f} & 76.0 / 68.3 / 78.0 & 27.9 \\
\midrule
\multicolumn{6}{l}{\emph{bidirectional attention over the prompt}} \\
earlier mix & 66.31 & 64.1 & +1.0 {[}+0.2, +1.8{]} & 62.7 / 66.8 / 58.8 & 25.0 \\
full coverage & 66.97 & 70.8 \textsuperscript{f} & +3.9 {[}+2.9, +4.8{]} \textsuperscript{f} & 92.2 / 71.7 / 66.7 & 35.8 \\
Instant recipe (C.4), first run & 65.81 & 72.1 \textsuperscript{f} & +3.8 {[}+2.9, +4.8{]} \textsuperscript{f} & 90.7 / 71.0 / 66.3 & 61.5 \\
Instant recipe, second run & 66.23 & 72.2 \textsuperscript{f} & +3.6 {[}+2.6, +4.6{]} \textsuperscript{f} & 88.8 / 69.7 / 67.2 & 60.4 \\
Instant recipe, from Stage 1 alone & 66.00 & 71.7 \textsuperscript{f} & level \textsuperscript{g} & 89.8 / 69.2 / 65.2 & 62.1 \\
Instant recipe + public procedural corpus & 65.96 & 71.0 \textsuperscript{f} & level \textsuperscript{g} & 91.0 / 68.0 / 63.0 & 61.8 \\
\midrule
\multicolumn{6}{l}{\emph{all weights from the untrained 4B, settings of the leading entries}} \\
2e-6, breadth and procedural rows only (825,000) & 40.87 & 55.6 & $-$3.3 {[}$-$4.3, $-$2.2{]} & -- & 27.2 \\
the same at 5e-6 & 44.71 & 59.2 & $-$2.9 {[}$-$3.9, $-$1.8{]} & -- & 46.4 \\
half blend of the 2e-6 run with v1 & 49.60 & 61.1 & $-$0.7 {[}$-$1.4, +0.1{]} & -- & 35.8 \\
\end{longtable}
\endgroup
\par\smallskip
{\footnotesize\raggedright\noindent \textsuperscript{f} In-family: the round trains on the family or the training split of some of these
test sets. \textsuperscript{d} Difference to the earlier-mix round. \textsuperscript{g} Measured
against the two Instant runs: mean of the reused layers 54.5 against 55.7 and 53.3, and $-$0.3 and
$-$0.1 for the corpus row.\par}

\subsection{What the ablations show}\label{sec:C.2}

The public index cannot tell data rounds apart. Most rounds that change only the data lie within 0.4
index points of the earlier-mix round, while the other measures move by several points. The public
procedural corpus adds 0.9 index points and nothing on the generated tasks: it fits the index, not
the decisions behind it.

Each gain sits in the families a group contains. Our procedural families raise the generated tasks
by 3.1 to 14.3 points, and the arithmetic part of the weak-area files raises the rebuilt GSM8K rows
by 11.1. The benchmark-source families raise the 18 reused tasks of their own families by 8.6 points
(+7.1 to +10.1) and the 16 others by 0.3 ($-$0.7 to +1.3). No group of data raised a reused task
whose family it does not contain.

Bidirectional attention raises tasks for which no data were added. On the earlier mix its gain on
the reused tasks lies in the 16 tasks outside the families of every round (+3.0, interval +1.5 to
+4.5). On the full-coverage data it adds 2.15 index points and 3.1 points on the reused tasks over
the same round without it. Set already in Stage 1 it raises Stage 1 from 54.70 to 57.48, but after
Stage 2 it ends where the round with the flag alone does (67.04 against 66.97). From the untrained
4B it raises the index from 40.87 to 44.76.

\subsection{What did not work}\label{sec:C.3}

Each item is a result for our models, data and settings, not proof that the idea cannot work
elsewhere.

\begin{itemize}
\item \emph{All weights from the untrained 4B with the settings of the leading entries}: below v1 on the
index, at one size where the leading entries train at 27B.
\item \emph{More rows of the same families}: 1.7 times the twin-reserved rows give 65.6 on the twins
against 65.7 with the cap.
\item \emph{Sarcasm data labelled by a mark of the writer} (a hashtag, ``/s'') lowers the sarcasm twin to
34.6 against 39.2 for v1.
\item \emph{Removing VAST against the stance bias}: the stance twin falls from 38.7 to 29.5. The untrained
4B already answers ``none'' in 65\% of the items whose target is not named.
\item \emph{Breadth rows alone}: reused tasks $-$0.6 ($-$1.4 to +0.1).
\item \emph{The original training splits of the twin sources}: twins up by 8.1, all on their own families
(ProofWriter 43.3 to 95.6), reused tasks down by 2.0.
\item \emph{Contrast pairs written by other models}: filtered against surface cues they raise the stance
twin from 38.7 to 45.5, and they help sarcasm in neither version.
\item \emph{Sources tested and removed}: generated code-execution rows (24.9--27.1 $\rightarrow$
13.4--15.1 on the benchmark), the official tool-retrieval training set (63.3 $\rightarrow$ 36.5), a
rebuild of the API-Bank training dialogues (85.4 $\rightarrow$ 32.4), long documents up to 32,000
tokens (0.448 $\rightarrow$ 0.428) and about 307,000 items from visual question answering (81.2
$\rightarrow$ 80.3).
\item \emph{The Instant recipe at 0.8B}: 51.21 against 51.60 for the earlier mix.
\end{itemize}

Evidence-removal rows (6,201) leave the index at 64.76 but make the answer change after 92.0\% of
removals of needed evidence instead of 69.2\% (Appendix~\ref{sec:F}). They are kept for a later
recipe.

\subsection{The Instant recipe}\label{sec:C.4}

Start from v1 or from Stage 1 alone, which score the same, and train one Stage 2 round with
bidirectional attention over the prompt on the final mix: the full-coverage data, with the old GSM8K
rows replaced by 1,452 clean problems in the rebuilt layout and 45 groups dropped that the current
leak scan flags.

The GSM8K replacement raises the skill on the rebuilt rows from 23.0 to 51.1 in the hygiene package
and costs 0.67 index points, all of them on the old GSM8K rows. For the same reason the first run of
the recipe lies 1.16 points below the full-coverage round without the replacement, and with the
rebuilt rows in place the two score the same (65.87 against 65.84). At 9B one run of the recipe
raises the index from 67.75 to 68.29, the reused tasks from 51.9 to 59.1 and the twins from 66.2 to
73.0 \todo[TODO(Instant)]{2B and 27B rounds, the 9B round from Stage 1 alone, the repair round of
the shortcut audit}.

\todo[TODO(appendix)]{add moved-out material from sections 1-6}
