# Supplementary material for: StartLux-Decision: AutoThink Decision Models with Reinforcement Learning for Calibrated Deliberative Decisions
Source: arXiv:2610.17309 source file (2026-10-20)
Supplement: Supplementary file 6 [file appendix_C_training_settings.tex]

\section{Training settings}\label{sec:C}

\subsection{Settings by stage}\label{sec:C.1}

All training ran on one cluster of eight nodes with eight H200 GPUs each. Table~\ref{tab:C.1} lists
the stages in training order (Chapters~\ref{sec:4} and \ref{sec:5}).

\begingroup
\renewcommand{\thetable}{C.1}
\footnotesize\setlength{\tabcolsep}{5pt}\renewcommand{\arraystretch}{1.1}
\begin{longtable}{>{\raggedright\arraybackslash}p{\mdw{0.1421}}>{\raggedright\arraybackslash}p{\mdw{0.1524}}>{\raggedright\arraybackslash}p{\mdw{0.1916}}>{\raggedright\arraybackslash}p{\mdw{0.1201}}>{\raggedright\arraybackslash}p{\mdw{0.1638}}>{\raggedright\arraybackslash}p{\mdw{0.1139}}>{\raggedright\arraybackslash}p{\mdw{0.1033}}}
\caption{Full fine-tuning is the one stage that trains all text parameters, and the other supervised stages train rank-64 adapters on fewer rows. Training settings by stage. Stages 1 to 3 make the released models, stage 4 is a decision data round, stages 5 to 7 are the reasoning stages and stage 8 is a reinforcement-learning variant. Ranges run over the sizes that have the stage.}\label{tab:C.1}\\
\toprule
\textbf{stage} & \textbf{trained} & \textbf{data} & \textbf{epochs, steps} & \textbf{peak learning rate, schedule} & \textbf{batch} & \textbf{GPUs, GPU-hours \textsuperscript{a}} \\
\midrule
\endfirsthead
\multicolumn{7}{l}{\textit{Table~\thetable{} (continued)}}\\
\toprule
\textbf{stage} & \textbf{trained} & \textbf{data} & \textbf{epochs, steps} & \textbf{peak learning rate, schedule} & \textbf{batch} & \textbf{GPUs, GPU-hours \textsuperscript{a}} \\
\midrule
\endhead
\bottomrule
\endfoot
1 Full fine-tuning & all text parameters and the output layer & broad mix, 2,726,203 rows (27B: 791,992) & 1 epoch, 3,535--14,198 steps & 2e-5 (0.8B), 1e-5 (2B, 4B), 5e-6 (9B), 2e-6 (27B). 3\% warm-up, cosine to zero (27B: to 10\% of the peak) & 192--384 rows & 8--56 GPUs, 8.2 (0.8B) to 178.6 (27B) \\
2 Adapter fine-tuning & rank-64 adapter, merged & curated mix, 190,418 rows (4B: 92,228) & 2 epochs, 1,002--3,966 steps & 1e-4 (27B: 5e-5), 5\% warm-up, cosine decay & 96--256 rows & 8--16 GPUs, 4.0 (4B) to 38.7 (27B) \\
3 Averaging & none, equal-weight average (0.5 each) of stages 1 and 2 & -- & -- & -- & -- & CPU \\
4 Decision data round & rank-64 adapter on the released weights, merged & 1,078,788 rows: sample of the release mix, anchor rows, teacher-labelled decisions, general multiple choice, targeted sources & 1 epoch, 5,862 steps (9B: 11,235, 27B: 8,408) & 5e-5, 5\% warm-up, cosine to zero & 184 rows (9B: 96, 27B: 128) & 8 GPUs, 6.0 (0.8B) to 98.4 (27B) \\
5 Thinking replay & rank-64 adapter, language-model loss on the thought and its closing tag & best thought per item written by the starting model: 15,870 targets (4B), 16,369 (9B), 4,395 (27B) & 1 epoch, 247 steps (4B) & 1e-4 & 64 sequences & 8 GPUs, 4.0 (4B), 4.8 (9B), 4.9 (27B) \textsuperscript{b} \\
6 Reader round & rank-64 adapter, soft cross-entropy on the answer letter & items after the model's own thought (label as target), items alone (earlier one-pass distribution as target) & 1 epoch, 481 steps (4B) & 5e-5 & 184 rows (27B: 128) & 8 GPUs, 6.5 (4B), 8.2 (9B), 16.7 (27B) \\
7 Stop step & rank-64 adapter after the reader round, language-model loss on the target & 5,311 targets from 59,644 thoughts of 14,911 items, cut where the answer stops changing & 1 epoch, 82 steps (4B) & 5e-5 & 64 sequences & 8 GPUs, 14.1 (4B), 15.4 (9B) \\
8 Reinforcement learning & the thought tokens by group-relative policy gradient, read-out fixed & pool of 26,931 items with a one-pass top probability below 0.9 & 120 iterations & 1e-5 & 8 thoughts for each of 64 prompts & 8 GPUs, 9.6 (4B) \\
\end{longtable}
\endgroup
\par\smallskip
{\footnotesize\raggedright\noindent \textsuperscript{a} H200 GPU-hours. Stages 1 and 2: trainer hours $\times$ GPUs. Stages 4 to 8: the
scheduled step on one node (8 GPUs). Stage 4 at 4B to 27B includes the evaluation of the checkpoint,
and stage 7 the writing of thoughts and read-outs.\par}
\par\smallskip
{\footnotesize\raggedright\noindent \textsuperscript{b} Without the starting model's writing of the thoughts, which was not timed on its
own.\par}

Stages 1, 2, 4 and 6 used one loss: the soft cross-entropy between the target distribution of a row
and the softmax over its listed options, computed in FP32 on the 26 letter rows of the output layer
at the last prompt position. No parameter was added, so the quantity trained is the quantity served.
Anchor rows (three times the weight of an ordinary row) and the one-pass rows of the reader round
are ordinary rows whose target is the model's own earlier distribution.

In stages 1, 2 and 4 we used AdamW with no weight decay and gradients clipped at norm 1.0, with
$\beta$2 0.95 for full fine-tuning and 0.999 for the adapters. Computation was in bf16. Full
fine-tuning at 9B and 27B kept FP32 master weights (ZeRO stage 2), and adapter weights were kept in
FP32. The adapters of stages 2 and 4 had rank 64, $\alpha$ 128 and no dropout and sat on every
projection of the text layers. Rows longer than 12,288 tokens were dropped when the mix was packed.

In reinforcement learning a thought was reinforced by how far its reward lay above that of the other
thoughts for its prompt. The first arms rewarded the gain of the read-out after the thought over the
one-pass read-out (log score or bounded proper score), minus 1e-4 per token, with a penalty of 0.02
towards the starting policy.

Thinking replay and the stop step, whose targets are text, used a trainer of their own: a rank-64
adapter with $\alpha$ 128 and no dropout on every projection of the text layers, AdamW with no
weight decay and $\beta$2 0.999, 5\% warm-up and cosine decay to zero, gradients clipped at 1.0. The
reader round used the trainer and optimiser of stage 4 on 88,512 rows at 4B and 88,492 at 27B, with
5\% warm-up and cosine decay to zero. Policy-gradient updates went into a low-rank adapter that the
generation workers loaded after every iteration, and the read-out was not trained in that stage.

\subsection{Per-size choices of the release recipe}\label{sec:C.2}

A single learning rate did not suit all sizes, so the peak rate of full fine-tuning fell from 2e-5
(0.8B) to 2e-6 (27B). At 9B, 2e-5 from the Base checkpoint scored 51.68 on the Decision Index 0.2.1,
1e-5 scored 56.07 and 5e-6 from the post-trained checkpoint scored 58.78, but the 4B from the
instruction-tuned checkpoint scored 54.70 at 1e-5 and 51.79 at 5e-6. For the adapter on the 4B, rank
64 at 1e-4 got 205 of the 231 public items right, against 201 at 5e-5 and 199 for rank 16.

Both halves of the 2B and 4B started from the instruction-tuned Qwen3.5-2B and Qwen3.5-4B, those of
the 9B from the post-trained Qwen3.5-9B and those of the 27B from Qwen3.8-27B. The 0.8B started from
Qwen3.5-0.8B-Base and is stage 1 alone, because the Base checkpoint was the better start (38.86
against 36.76 for the instruction-tuned one). The 35B-A3B started from Qwen3.6-35B-A3B and went
through the same two halves: full fine-tuning on the broad mix of the 27B (791,992 rows, one epoch,
3,093 steps of 256 sequences, peak rate 5e-6 with 3\% warm-up and cosine decay to 10\%), then an
adapter on the curated mix (190,418 rows, two epochs, peak rate 5e-5 with 5\% warm-up and cosine
decay to zero), merged and averaged half and half with the first half (run configurations of 1
October 2026).

We scored five adapter weights from 0 to 1 and released the equal-weight average at 2B to 27B, which
keeps most of both parents. At 27B it scored 63.88 on the index and 208 of 231 public items, against
64.02 and 207 for the fully fine-tuned model and 61.39 and 205 for the adapter model alone.

A second-stage adapter on the fully fine-tuned weights was tried and left out (Section~\ref{sec:4.6}
lists the main failures). It scored below its parent in all eleven runs of the second and third day,
by 0.50 to 2.86 index points, although a development set from the source of its new rows rose in
every one.

\subsection{Calibration temperatures}\label{sec:C.3}

One temperature per question type (yes/no, choice, score) divides the letter scores before the
softmax. It changes how sure the model is, never which option it picks. After every merge or average
we fitted the three values with one script on the development splits of three sets of an open
decision-model project (3,077 rows). For each type the script searched 1,201 logarithmically spaced
values between 0.2 and 5 for the lowest mean cross-entropy to the targets. A type with fewer than
200 rows (score) took the value fitted on all rows pooled.

The released values (yes/no / choice / score) are 3.29 / 1.756 / 1.893 at 0.8B, 2.291 / 1.532 /
1.616 at 2B, 1.591 / 1.387 / 1.417 at 4B, 1.724 / 1.229 / 1.294 at 9B 1.421 / 1.21 / 1.229 at 27B
and 1.376 / 1.19 / 1.213 at 35B-A3B. All exceed 1, so the models are overconfident on the fit
source. Over the 47 checkpoints of the release campaign the mean calibration error fell from 0.0956
to 0.0246 on the test splits of the fit source (all 47 better) and from 0.1219 to 0.0924 on the 111
hard public JevBench items (37 better). On a check set of 17,402 rows close to the training
distribution it rose from 0.0285 to 0.0491, worse for 36 of the 47, because at temperature 1 the
models are already close to calibrated on their own distribution.

\subsection{Compute}\label{sec:C.4}

The nine training runs behind the five dense released models took 363 GPU-hours, and the whole
release campaign, with rejected and aborted runs, about 827. A data round of the final recipe cost
19.6 GPU-hours at 4B and 98.4 at 27B, with the evaluation of its checkpoint, and the three reasoning
stages about 25 GPU-hours in total at 4B, not counting the starting model's writing of the replay
samples.
