# Supplementary material for: StartLux-Decision: AutoThink Decision Models with Reinforcement Learning for Calibrated Deliberative Decisions
Source: arXiv:2610.17309 source file (2026-10-20)
Supplement: Supplementary file 7 [file appendix_D_data_sources.tex]

\section{Data sources}\label{sec:D}

\subsection{Record format and conversion}\label{sec:D.1}

One converter per source maps its fields to the record of Chapter~\ref{sec:3}. A single label
becomes a one-hot target, a probability dictionary of the source is mapped to the options, and
targets are normalised and rounded to six decimals with the rounding error added to the largest
entry. A choice with more than 26 options keeps every option with positive probability and is filled
to 26 at random, and a score with more than ten levels becomes a choice. A single-letter option
identifier is hidden, so that a prompt never shows two letters for one option.

Rows with a uniform target are dropped as placeholders (137,203 rows of one community corpus),
except program labels and questions that are undecidable by design. Splits of benchmarks are rebuilt
from their train and development files only. Rows longer than 12,288 tokens are dropped, not
truncated.

Two label kinds are looser than their names suggest. Of the rows counted as written by a model,
10,447 are dialogue-intent distributions derived from human labels, and the 5,978 rows of the
typed-decisions set counted as provided by the source are means of three samples of a teacher model.

\subsection{Sources}\label{sec:D.2}

The release pool has 25 source files and the final data round 30, listed by source family in
Table~\ref{tab:D.1}.

\begingroup
\renewcommand{\thetable}{D.1}
\footnotesize\setlength{\tabcolsep}{5pt}\renewcommand{\arraystretch}{1.1}
\begin{longtable}{>{\raggedright\arraybackslash}p{\mdw{0.2947}}>{\raggedleft\arraybackslash}p{\mdw{0.1185}}>{\raggedright\arraybackslash}p{\mdw{0.1044}}>{\raggedright\arraybackslash}p{\mdw{0.2661}}>{\raggedright\arraybackslash}p{\mdw{0.2029}}}
\caption{Most rows of the release pool come from community corpora and public training splits, and more than half of the final data round is training splits aimed at single benchmarks. Sources. Block A: the release pool (rows in the pool $\rightarrow$ rows in the full-fine-tuning mix of the 0.8B to 9B models, where known). Block B: the final decision data round (4B build, rows after de-duplication). Label: H = human or source gold label, T = written or labelled by a model, P = computed by a program. Licences as stated on the official card or repository on 7 October 2026 (``none stated'': no licence there, ``unknown'': the card says so, ``not confirmed'': no official page opened, ``mixed'': differs within the family).}\label{tab:D.1}\\
\toprule
\textbf{source} & \textbf{rows} & \textbf{label} & \textbf{licence} & \textbf{aimed at} \\
\midrule
\endfirsthead
\multicolumn{5}{l}{\textit{Table~\thetable{} (continued)}}\\
\toprule
\textbf{source} & \textbf{rows} & \textbf{label} & \textbf{licence} & \textbf{aimed at} \\
\midrule
\endhead
\bottomrule
\endfoot
\textbf{A. Release: candidate pool} & \textbf{6,397,500} &  &  &  \\
Community corpora of typed decisions (four) & 2,224,874 $\rightarrow$ 664,849 & T, P, H & Apache-2.0, CC0-1.0 / CC BY 4.0 by source, mixed per row, one ``unknown'' & -- \\
General public mixture: train splits of public classification, inference, question-answering, safety, preference and tool sets & 1,976,644 $\rightarrow$ 1,189,277 & H, P, T & mixed, with non-commercial and share-alike sets & BANKING77, CLINC150, WinoGrande, HellaSwag \\
Program-generated: a public procedural corpus (729,910) and our exact-probability questions (39,995) & 769,905 $\rightarrow$ 157,045 & P & Apache-2.0, own & -- \\
Train and development splits of 15 index benchmarks, rebuilt in the layout of the index's public kit & 441,457 $\rightarrow$ 273,022 & H & mixed: one CC BY-NC 4.0, two CC BY-SA 4.0, four without a stated licence & those benchmarks \\
Tool-use decisions: three function-calling corpora, agent traces, API-Bank training dialogues & 340,899 & source labels & Apache-2.0, CC BY 4.0, MIT & BFCL (layout), API-Bank \\
Knowledge and commonsense multiple choice (twelve public sets) and When2Call preference pairs & 292,428 $\rightarrow$ 194,029 & H & mixed: one CC BY-NC 3.0, one non-commercial research only, one CC BY-SA 4.0, two ``unknown'' & WinoGrande, HellaSwag, When2Call, layout of MMLU-Pro and GPQA \\
Public train splits from an earlier project of ours & 238,469 & H & mixed, with CC BY-NC and CC BY-NC-SA sets & -- \\
Small hard decision sets (four public sets, one a typed-decisions train split) & 39,281 $\rightarrow$ 25,444 & T, P & Apache-2.0, CC BY 4.0 & -- \\
Teacher-written hard decisions (adapter mixes only) & 38,150 & T & own & -- \\
Safety judgments (WildJailbreak) & 31,997 & source labels & ODC-BY, gated & -- \\
Colour-palette preference pairs & 3,396 & H & not confirmed & cfcolor \\
\textbf{B. Final decision data round} & \textbf{1,078,788} &  &  &  \\
Teacher-labelled workplace decisions & 41,687 & T & own & -- \\
Sample of the release adapter mix & 29,993 & as in A & mixed & -- \\
Anchor rows: the released model's own distribution, weight 3 & 25,191 & the model & own & -- \\
General multiple choice (seven public sets) & 29,296 & H & mixed & layout of MMLU-Pro and GPQA \\
\textbf{Targeted: train splits and upstream training sides} & \textbf{588,673} &  &  &  \\
Aspect-category sentiment in the benchmark's enumeration, weight 0.2 & 234,504 & H & none stated & ACOS \\
Replay of the train splits of 13 index benchmarks & 100,679 & H & mixed & those 13 benchmarks \\
Select-all questions, training side of six upstream sources & 100,595 & H, classifier scores & mixed & SATA-Bench \\
Shopping-query relevance, square-root label shares & 89,904 & H & Apache-2.0 & Amazon ESCI \\
Sarcasm categories for every training text, weight 0.5 & 20,736 & H & MIT & iSarcasmEval \\
WinoGrande train (20,000 of 40,398) & 20,000 & H & none on the card, repository Apache-2.0 & WinoGrande \\
When-to-call decisions, official training set & 8,798 & source labels & CC BY 4.0 & When2Call \\
Forecasting questions resolved before the test window & 7,825 & outcomes & CC BY-SA 4.0 & ForecastBench \\
Colour-palette preference pairs & 3,396 & H & not confirmed & cfcolor \\
Group-statement preference, training questions & 2,236 & H & CC BY 4.0 & Habermas Machine \\
\textbf{Targeted: generators} & \textbf{296,060} &  &  &  \\
Phishing decisions on e-mails with a link, weight 0.5 & 63,000 & P & own & PhishNChips \\
Appliance simulator & 52,401 & P & own & home appliance simulator \\
Select-all on synthetic paragraphs & 48,019 & P & own & SATA-Bench \\
Chess positions with engine labels (40,000 of 65,555) & 40,000 & P & own, engine GPL-3.0 & ChessBench \\
State tracking and deduction & 39,730 & P & own & BBH \\
Causal reasoning & 31,363 & P & own & CLadder \\
Chord recognition on generated arrangements & 12,000 & P & own & POP909-CL \\
Narrative reasoning: planned by program, written by a model, verified & 9,547 & P, T & own & MuSR \\
\textbf{Targeted: written by API models.} Retrieval items 35,567, limerick minimal pairs 17,855 (written by an API model, corrupted by program) & \textbf{53,422} & T, P & own \todo{provider terms} & BRIGHT, BPoMP \\
\textbf{Related public data.} Entity-level financial sentiment (SEntFiN) 13,975, long-document questions of 20,000--46,000 characters 491 & \textbf{14,466} & H & MIT, not confirmed for the long documents (built from 2WikiMultihopQA, CUAD and QuALITY) & FinEntity \\
\end{longtable}
\endgroup

\subsection{What is aimed at each index benchmark}\label{sec:D.3}

For each of the 38 benchmarks of Decision Index 0.2.1, Table~\ref{tab:D.2} gives the training data
aimed at it. The released models of every size from 0.8B to 27B have official training splits for 18
of them, and for 19 by the count of the internal record of the release, which includes Humicroedit
although only one of its 12,240 training rows survived the duplicate filter. The public repository
marks 14 and leaves out WinoGrande, HellaSwag, API-Bank, When2Call and the palette ratings. The
final rounds aim data at 33 benchmarks, 35 with the two layout-only cases, and tool retrieval, HLE
and CRUXEval stay zero-shot.

\begin{table}[!htbp]
\renewcommand{\thetable}{D.2}
\centering
\caption{The final data rounds aim data at 33 of the 38 benchmarks, and tool retrieval, HLE and CRUXEval stay zero-shot. Training data aimed at each benchmark. T = official training split or training set of the benchmark's source. G = our generator or written data in the benchmark's layout, with nothing of the benchmark in it. R = related public data in the benchmark's layout. -- = nothing aimed at it.}\label{tab:D.2}
{\footnotesize\setlength{\tabcolsep}{5pt}\renewcommand{\arraystretch}{1.1}
\noindent\begin{adjustbox}{max width=\linewidth}
\begin{tabular}{>{\raggedright\arraybackslash}p{\mdw{0.6112}}>{\raggedright\arraybackslash}p{\mdw{0.1809}}>{\raggedright\arraybackslash}p{\mdw{0.1939}}}
\toprule
\textbf{benchmarks} & \textbf{released models} & \textbf{final data rounds} \\
\midrule
BANKING77, CLINC150, HoVer, ContractNLI, ANLI, VAST, NLI4CT, RAGTruth, iSarcasmEval, GSM8K, New Yorker caption matching & T & T \\
WinoGrande, HellaSwag, cfcolor & T \textsuperscript{a} & T \\
Amazon ESCI, aspect-category sentiment (ACOS) & T & T (resampled) \\
When2Call & T (preference pairs, 2,700 rows) & T \\
API-Bank & T \textsuperscript{a}, R & R \\
function calling (BFCL) & R & R \\
GPQA Diamond, MMLU-Pro & R \textsuperscript{b} & R \textsuperscript{b} \\
Habermas Machine, ForecastBench & -- & T \\
Humicroedit & -- (1 row survived the duplicate filter) & T \\
home appliance simulator, phishing decisions (PhishNChips), causal reasoning (CLadder), MuSR, chess (ChessBench), chord recognition (POP909-CL), limerick minimal pairs (BPoMP) & -- & G \\
reasoning-intensive retrieval (BRIGHT) & -- & G (written items, none of its documents) \\
BBH fixed-option tasks & -- & G (later rounds, no held-out claim) \\
select all that apply (SATA-Bench) & -- & G, and T of its upstream sources \\
FinEntity & -- & R \\
tool retrieval (ToolRet) & -- & -- (T in earlier rounds, removed) \\
HLE, CRUXEval & -- & -- \\
\bottomrule
\end{tabular}
\end{adjustbox}\par}
\par\smallskip
{\footnotesize\raggedright\noindent \textsuperscript{a} The full-fine-tuning mixes of every size hold these files: the 0.8B, 2B, 4B and
9B trained that stage on one mix, an earlier 4B mix extended by the 399,000 rows of the 27B mix that
it lacked and by three smaller sets (run manifests and the internal record of the release).
\textsuperscript{b} Layout only: general multiple-choice questions from other sources, in the two
layouts in which the suite stores these benchmarks.\par}
\end{table}

\subsection{Data groups of 7 October 2026}\label{sec:D.4}

We built the data of Table~\ref{tab:D.3} on 7 October 2026 for decision data rounds that test
breadth in place of index-targeted sources. None of it is in a released model or in the final data
round, and Section~\ref{sec:4.4} reports the 4B rounds that add these groups.

\begin{table}[!htbp]
\renewcommand{\thetable}{D.3}
\centering
\caption{None of the data groups of 7 October 2026 is in a released model, and three of them make evaluation sets in-family. Data groups of 7 October 2026 (rows after cleaning). Licence by rows: commercial use allowed / no licence stated / non-commercial, in the most restrictive reading of the collection's own records. Labels are source labels, except in the procedural families (computed by a program).}\label{tab:D.3}
{\footnotesize\setlength{\tabcolsep}{5pt}\renewcommand{\arraystretch}{1.1}
\noindent\begin{adjustbox}{max width=\linewidth}
\begin{tabular}{>{\raggedright\arraybackslash}p{\mdw{0.6227}}>{\raggedright\arraybackslash}p{\mdw{0.0961}}>{\raggedleft\arraybackslash}p{\mdw{0.1144}}>{\raggedleft\arraybackslash}p{\mdw{0.1530}}}
\toprule
\textbf{group} & \textbf{data sets} & \textbf{rows} & \textbf{licence by rows} \\
\midrule
Breadth: tasks of a public collection (tasksource), at most 3,000 rows per task & 343 tasks & 642,628 & 340,383 / 251,494 / 50,751 \\
Breadth, multilingual: at most 600 rows per task & 102 tasks & 47,784 & 30,390 / 14,394 / 3,000 \\
Single skill: stance (repeated rows of the two files above) & 18 tasks & 17,378 & 10,721 / 5,344 / 1,313 \\
Single skill: sarcasm and irony (likewise repeated) & 10 tasks & 18,158 & 8,152 / 10,006 / 0 \\
Single skill: select-all, one yes/no question per candidate label & 3 tasks & 8,995 & 8,995 / 0 / 0 \\
Twin-reserved families: training rows of families behind the twin test sets (Section~\ref{sec:6.3}) & 33 tasks & 72,426 & 32,672 / 30,813 / 8,941 \\
Twin-reserved: three tasks sharing text with twin items (Corr2Cause, CODAH, ReClor) & 3 tasks & 7,758 & 4,777 / 2,981 / 0 \\
Benchmark-source families: tasks held back to protect the reused tasks of our benchmark (Section~\ref{sec:6.4}) and other protected sets & 58 tasks & 143,157 & 73,502 / 54,562 / 15,093 \\
Procedural families: twelve generated families, and three more & 15 families & 108,005 + 27,001 & own \\
Weak-area training sets: arithmetic 19,954, answerability 32,000, sarcasm 29,750, financial sentiment 10,777, phishing e-mail 11,621, paraphrase 13,065 & 20 data sets & 117,167 & recorded per data set \\
GSM8K training problems without protected text (1,456 problems), kept in a file of their own & 1 data set & 2,912 & MIT \\
\bottomrule
\end{tabular}
\end{adjustbox}\par}
\end{table}

Whole tasks were excluded before any row was read: 91 that are, or feed, an evaluation set of ours,
38 reserved for the twin test sets and 8 in Chinese, and a first scan against the evaluation index
dropped 21 more families. Every finished file then passed the scan of Section~\ref{sec:3.2}, which
removed 664 rows over the breadth and single-skill files and 1,164 in the benchmark-source file.
Three groups make an evaluation set in-family, so that the model has trained on the family the set
comes from: the twin-reserved files for the twin test sets, the benchmark-source file for the reused
tasks of our benchmark, and the weak-area files, on purpose, for SQuAD 2.0 and the FiQA card, whose
evaluation sides are a reused task and a twin. The test items themselves were removed or never read,
and scores on such sets are reported as in-family. No person has audited the new rows. In the
phishing file the label is the corpus a message comes from, and positives and negatives come from
different corpora and years, so part of that decision can be made from style.

\subsection{Licences}\label{sec:D.5}

The released weights are under CC BY-NC 4.0 and the code under Apache-2.0, and this section states
facts, not legal advice. Non-commercial terms apply to ANLI, SciQ, toxic-chat, a set of support
tickets, BeaverTails, PKU-SafeRLHF and a collection of phishing mail. Financial PhraseBank and QuAIL
are non-commercial and share-alike. RACE, MS MARCO, MRPC and Quora Question Pairs are marked by
their source for research use only, and ARC, SNLI, HoVer and ForecastBench are share-alike. One
community corpus (409,937 rows in the pool), OpenBookQA, ACOS, VAST and NLI4CT state no licence or
say ``unknown'', and we did not confirm those of the palette ratings, EURLEX57K, ShARC and the 491
long-document rows. The remaining sources are permissive or carry terms of their own, and the
teacher-written decisions, generators and anchor rows are ours. The retrieval items and the
limericks were written by third-party API models \todo{terms of the provider for training on and
releasing the outputs}.

\subsection{Generators, written data and sources tested and removed}\label{sec:D.6}

\textbf{Teacher-written decisions.} The release batch had thirteen families of hard decisions over
45 domains, written by Qwen3.8-27B (a quarter of the seeds by Qwen3.6-35B-A3B) with no benchmark
item shown to a writer. Of 80,000 seeds, 55,272 items passed the structural checks, 69.1\% of those
passed both verifiers, and 38,150 rows entered the pool, in the adapter mix of the 2B, 9B and 27B
only. We have no comparison that isolates their effect. The data-round batch had eleven families,
led by five workplace families. Of its first 48,000 seeds, 28,381 items were structurally valid and
27,939 passed both verifiers, and two smaller batches gave 6,908 items (from 12,000 seeds) and 6,953
items \todo{the seed count of the third batch and the pass rates of both}. The filter cannot see a
skew in what is asked: the invoice family holds 1,142 ``escalate'', 716 ``hold'' and 35 ``approve''
labels. A 4B trained on the batch fell on a third-party invoice set (exact-action agreement 39.8
$\rightarrow$ 26.0), and routine cases written to repair this reached only 30.2 and 32.4 and are not
in the final mix.

\textbf{Generators.} No evaluation item is read into a generator, only category-level error tables.
Labels come from a program for the exact-probability, chord, phishing (9,000 e-mails with seven
questions each), state-tracking (52,000 rows built) and select-all generators, and from Stockfish
for chess (65,555 positions built). The chord generator reads no song of the benchmark's corpus,
because all 907 of its songs are in the evaluation pool. Narrative stories were planned by program
in three kinds (murder, team and object placement), written by Qwen3.8-27B and kept if verified
\todo{verification rule}. A verified story came from 6,155 of the 12,000 plans of the first batch
and from 3,617 of the 4,000 object-placement plans of the second. Two further generators make causal
reasoning, with yes/no questions in 46 families (23 combinations of question type and graph setting,
each in a story wording and with nonsense names), and the appliance simulator, with 2,475 simulated
states, cases in nine families and 2 to 9 options, and a program computes the label in both.

\textbf{Written by API models.} GLM-5.3 and DeepSeek-V4-Pro wrote the retrieval items in 6,000
calls, and a blind verifier of the other model family confirmed 99.0\% and 97.0\% of their
positives, leaving 5,162 items. Of 13,510 limericks written anew, 6,167 passed a rhyme check against
a pronouncing dictionary.

\textbf{Tested and removed.} Four sources were removed after a test: two generators of
code-execution functions (24.9--27.1 $\rightarrow$ 13.4--15.1 at 4B, 33.8 $\rightarrow$ 26.0 at 9B),
the official tool-retrieval training set (63.3 $\rightarrow$ 36.5, index $-$0.9), a rebuild of the
API-Bank training dialogues (85.4 $\rightarrow$ 32.4) and chord rows from human lead sheets, which
added nothing over the generator (80.5 against 78.3). Long documents up to 32,000 tokens
(long-document benchmark 0.448 $\rightarrow$ 0.428), about 307,000 items converted from visual
question answering (mean of eight image benchmarks 81.2 $\rightarrow$ 80.3) and a third phishing
generator did not raise the score in one or two 4B rounds and were not adopted. Evidence-removal
rows (6,201) left the index at 64.76 against 64.78 but changed the answer after 92.0\% of removals
instead of 69.2\%, so they are kept for the next recipe. Two search-relevance sets gave 65.67
against 64.78 in the first arm, inside the spread of repeated rounds, and are undecided.
