# Supplementary material for: StartLux-Decision: AutoThink Decision Models with Reinforcement Learning for Calibrated Deliberative Decisions
Source: arXiv:2610.17309 source file (2026-10-20)
Supplement: Supplementary file 8 [file appendix_D_policy_calibration.tex]

\clearpage
\section{Policy-aware calibration: details, and certificates across task families}\label{sec:D}

The details behind Sections~\ref{sec:7.4} and \ref{sec:7.5} follow: the certificate protocol with
every setting, the calibration recipe with all pipelines, the set-aware map for best-of-N, the
route-aware map for the think-gate, the maps for cascades and for select-then-think, a test on the
public records of a system we did not build, and the limits of certificates across task families.

\subsection{Certificates: protocol and all settings}\label{sec:D.1}

A threshold certified on the data one would normally calibrate on (single responses, or all answers
of the system) is exceeded by the answers the policy acts on. A threshold certified on the policy's
own answers is not.

\textbf{Protocol.} A threshold on the reported confidence is certified for error $\leq$ $\alpha$ on
a calibration half of the problems (fixed-sequence Clopper--Pearson test at 95\% on a fixed grid of
thresholds, at least 100 accepted answers), then applied to the answers the system returns on the
other half. We repeated this over 20 splits by source problem.

\begin{table}[!htbp]
\renewcommand{\thetable}{D.1}
\centering
\caption{Certified thresholds in all settings: error of the accepted (acted-on) answers and the number of splits in which it is above the level $\alpha$, for a threshold certified on the usual calibration data (first line of each setting) and on the answers of the same policy or route (second line). ``Ours'' = StartLux-Decision models. Own runs.}\label{tab:D.1}
{\footnotesize\setlength{\tabcolsep}{5pt}\renewcommand{\arraystretch}{1.1}
\noindent\begin{adjustbox}{max width=\linewidth}
\begin{tabular}{>{\raggedright\arraybackslash}p{\mdw{0.3945}}>{\raggedright\arraybackslash}p{\mdw{0.1791}}>{\raggedright\arraybackslash}p{\mdw{0.2545}}>{\raggedleft\arraybackslash}p{\mdw{0.1583}}}
\toprule
\textbf{setting} & \textbf{calibration data} & \textbf{error of accepted (acted-on) answers} & \textbf{splits above the level} \\
\midrule
best-of-N, unseen datasets, $\alpha$ = .05, N = 32, ours 4B / 9B / 27B & single responses & 10.05\% / 9.27\% / 7.57\% & 19 / 20 / 20 of 20 \\
 & same policy & 3.5--4.3\% & 0--4 of 20 \\
best-of-N, unseen datasets, $\alpha$ = .10, Clef 27B, N = 4 / 8 / 16 / 32 & single responses & 10.7 / 11.4 / 12.2 / 13.0\% & 16 / 19 / 20 / 20 \\
 & same policy & 8.6--9.0\% & 0--2 \\
best-of-N, unseen datasets, $\alpha$ = .10, Phi-4-mini as verifier, N = 4 \ldots{} 32 & single responses & 11.3 $\rightarrow$ 17.3\% & 15--20 \\
 & same policy & 8.4--8.5\% & 0--2 \\
best-of-16, all 67 pairs with coverage, $\alpha$ = .05 (Figure~\ref{fig:B.3}b) & single responses & above the level in 44 of 67 pairs & $\geq$ 10 of 20 in 32 pairs \\
 & same policy & above the level in 0 of 67 pairs & $\geq$ 10 of 20 in 0 pairs \\
think-gate, decision suite, $\alpha$ = .10, ours 4B / 9B & all answers of the system & thought answers 18.2\% / 26.3\% & 20 / 20 \\
 & per route & 14.7\% (few accepted) / none accepted & 1 / 0 \\
think-gate, CJ-Bench, $\alpha$ = .05, ours 4B, 10\% / 20\% think rate & all answers & thought answers 27.9\% / 27.3\% & 20 / 20 \\
 & per route & no thought answer accepted, system 4.6\% & 0 \\
think-gate, CJ-Bench, $\alpha$ = .10, ours 9B, 10\% think rate & all answers & thought answers 56.0\% & 20 \\
 & per route & no thought answer accepted, system 8.4\% & 0 \\
select-then-think, reasoning sets, $\alpha$ = .10, 9B, N = 2 / 4 / 8 & all returned answers & thought answers 22.2 / 18.6 / 15.8\% & 20 / 20 / 14 \\
 & per route & 6.9--7.8\% & 0 \\
\bottomrule
\end{tabular}
\end{adjustbox}\par}
\end{table}

\todo{the think rate of the two decision-suite rows is not stated in v4 Table 5 (part2.md:238-239),
and their values (18.2\% / 26.3\%; per route 14.7\% / none) could not be found in the table files:
tables/think\_gate\_di\_families.txt gives 21.33\% / 36.51\% at a 30\% think rate and 18.12\% /
24.28\% at 50\% (per route none / none, and 14.21\% / none), and v4 Appendix D.2 gives 12.6\% /
22.2\% after a map of c1 alone at 30\% (part3b.md:611-613). Re-derive the two rows or state their
source.}

A certificate for all answers of a gated system is a statement about a mixture of routes and is
silent about each route (Proposition 3, A.4). A per-policy certificate also \emph{refuses} a system
that cannot be trusted: Clef-flash on the reasoning sets at $\alpha$ = .20 accepts 17--28\% of the
answers at 21.5--26.7\% error under the single-response threshold and nothing per policy. More
certificate results are with their pipelines: best-of-N at N = 256 in B.3, question answering in
B.6, the value gate in E.4.

\subsection{The recipe, and all pipelines}\label{sec:D.2}

The maps of D.3 and D.4 are instances of one rule: \emph{calibrate the reported confidence on the
statistics the policy used to produce the answer.} Proposition 4 (A.5) says why this is the right
target: if a confidence q is calibrated conditionally on a statistic T, P(correct \textbar{} q, T) =
q, then it is calibrated on the answers returned by every policy whose decision is a function of T.
Marginal calibration is the case in which T is empty, and Propositions 1 and 2 say when that is not
enough.

The recipe has three steps and needs no knowledge of a threshold.

\begin{enumerate}
\item Run the policy on calibration problems and record, with every returned answer, its confidence and
what the policy looked at: for selection, the mean score of the candidates and N. For a gate or a
cascade, the confidence that decided the route. For select-then-think, the fast score of the
returned candidate, the mean fast score and N.
\item Fit the map. For a single routing score: an isotonic map of the reported confidence within quantile
strata of that score (eight strata here). For selection, where N is among the statistics: a logistic
model in the logits of the quantities and log N, followed by an isotonic map.
\item Report the mapped confidence and certify thresholds per route (Proposition 3).
\end{enumerate}

Table~\ref{tab:D.2} and Figure~\ref{fig:7.4} collect what the recipe does. Best-of-N and the
think-gate are detailed in D.3 and D.4. Cascades and select-then-think use the same code with other
inputs (D.5). The last row of the table is a system we did not build (D.6). Over all 184 settings of
the figure (verifiers, generators, models of other teams, think rates, values of N up to 256), the
usual calibration is off by $-$11.7 to +20.5 points and the policy-aware map by $-$2.7 to +2.1.

\begin{table}[!htbp]
\renewcommand{\thetable}{D.2}
\centering
\caption{Overconfidence of the returned answers (points) under the usual calibration and under the policy-aware map, all pipelines. Own runs, except the last row, which uses the public records of another group.}\label{tab:D.2}
{\footnotesize\setlength{\tabcolsep}{5pt}\renewcommand{\arraystretch}{1.1}
\noindent\begin{adjustbox}{max width=\linewidth}
\begin{tabular}{>{\raggedright\arraybackslash}p{\mdw{0.1612}}>{\raggedright\arraybackslash}p{\mdw{0.2179}}>{\raggedright\arraybackslash}p{\mdw{0.3057}}>{\raggedright\arraybackslash}p{\mdw{0.1869}}>{\raggedleft\arraybackslash}p{\mdw{0.1149}}}
\toprule
\textbf{pipeline} & \textbf{what the map is given besides the reported confidence} & \textbf{settings} & \textbf{usual calibration} & \textbf{policy-aware map} \\
\midrule
best-of-N & mean score of the candidates, N & unseen datasets, five verifiers, N = 2 \ldots{} 32, fitted at N = 1, 4, 16 & +0.8 \ldots{} +14.6, growing with N & $-$1.2 \ldots{} +0.3 \\
 &  & the same up to N = 256, two generators, our three verifiers (Figure~\ref{fig:7.4}) & $-$0.2 \ldots{} +15.0 & $-$2.0 \ldots{} +0.4 \\
think-gate & the plain confidence & decision suite, nine models, think rates 10--50\% & up to +16 on the routed answers & $-$1.5 \ldots{} +2.1 \\
cascade & the small model's confidence & decision suite, seven pairs of models of two teams, 30\% escalated & +2.3 \ldots{} +8.4 on the escalated answers & $-$0.6 \ldots{} +0.5 \\
select-then-think & fast score of the returned candidate, mean fast score, N & ten settings: two verifiers on held-out, unseen and reasoning problems, fitted at the two or three smallest N & +2.1 \ldots{} +7.3 at the largest N, growing with N & $-$1.4 \ldots{} +0.7 at every N \\
actor $\rightarrow$ reasoner, records of another group & the actor's confidence & 21 settings: eleven actors, two option orders, 30\% deferred, 180 deferred questions each & $-$10.7 \ldots{} +18.1 on the deferred answers & $-$7.4 \ldots{} +4.4 \\
\bottomrule
\end{tabular}
\end{adjustbox}\par}
\end{table}

\subsection{Set-aware calibration for best-of-N}\label{sec:D.3}

Per-policy thresholds have to be certified again for every N. Proposition 1 says why the
single-response map fails (the losing candidates carry information about the difficulty of the
problem) and so what to condition on. We fitted \emph{one} map g(s, m, N) of the selected score s,
the mean score m of the N candidates and N (a logistic model, then an isotonic map) on the best-of-N
outputs of the calibration problems at N = 1, 4 and 16 only, and evaluated it on other problems at
every N.

\begin{figure}[!htbp]
\renewcommand{\thefigure}{D.1}
\centering
\adjincludegraphics[max width=\linewidth,max height=0.5\textheight]{figures/fig5x_setaware.pdf}
\caption{Set-aware calibration for best-of-N. (a, b) Overconfidence of the selected response against N on unseen datasets under the single-response map (solid) and under the set-aware map fitted at N = 1, 4 and 16 (dashed, where filled markers are fitted values of N and open markers values it never saw), for two generators. (c) Error of the accepted answers with a threshold certified on single responses (solid), one threshold on the set-aware confidence certified at N = 1, 4 and 16 (dashed), and a threshold certified per N (dotted). Means over 20 splits by source problem, bars the 10th--90th percentile.}\label{fig:D.1}
\end{figure}

\todo{the caption does not say which generator and verifiers panel (c) shows; v4 Figure 7 caption
(part2.md:262).}

\textbf{It gives the reported number its meaning back.} Table~\ref{tab:D.3} gives the accuracy of
the answers reported in a confidence bin. Under the single-response map, answers reported at
80--90\% are right 86\% of the time for one candidate and 62--71\% for the best of 32, where answers
reported at 70--80\% are right 44--56\% of the time. Under the set-aware map the two figures at N =
32 are 79--86\% and 73--78\%. The repair is not exact bin by bin beyond the fitted range: at N = 32
the 80--90\% bin of the 9B verifier is at 79\%.

\begin{table}[!htbp]
\renewcommand{\thetable}{D.3}
\centering
\caption{Share of correct answers (\%) among the answers a verifier selects from N candidates and reports inside a confidence bin. Unseen datasets, 2B generator. Each cell N = 1 / 4 / 32. Own runs.}\label{tab:D.3}
{\small\setlength{\tabcolsep}{6pt}\renewcommand{\arraystretch}{1.1}
\noindent\begin{adjustbox}{max width=\linewidth}
\begin{tabular}{lrrrr}
\toprule
\textbf{map} & {\begin{tabular}[b]{@{}r@{}}\textbf{reported}\\\textbf{confidence}\end{tabular}} & \textbf{4B verifier} & \textbf{9B verifier} & \textbf{27B verifier} \\
\midrule
single-response & .70--.80 & 74.2 / 64.0 / 43.6 & 75.0 / 62.1 / 45.1 & 75.2 / 68.2 / 55.8 \\
single-response & .80--.90 & 86.3 / 75.2 / 61.6 & 85.9 / 76.4 / 63.0 & 86.6 / 80.1 / 70.5 \\
single-response & .90--.95 & 93.2 / 86.8 / 75.4 & 93.2 / 87.4 / 77.9 & 94.2 / 89.6 / 82.9 \\
set-aware & .70--.80 & 76.3 / 76.2 / 72.9 & 73.4 / 76.2 / 78.3 & 73.4 / 77.8 / 77.9 \\
set-aware & .80--.90 & 87.7 / 86.3 / 82.5 & 88.4 / 86.7 / 79.2 & 84.8 / 87.5 / 86.1 \\
set-aware & .90--.95 & 93.3 / 93.8 / 90.7 & 94.3 / 92.6 / 90.0 & 92.7 / 93.6 / 91.6 \\
\bottomrule
\end{tabular}
\end{adjustbox}\par}
\end{table}

\textbf{It is calibrated at values of N it never saw.} On the unseen datasets with the 2B generator
the single-response map is overconfident by +2.4 $\rightarrow$ +9.4 points (4B verifier, N = 2
$\rightarrow$ 32), +2.1 $\rightarrow$ +8.3 (9B), +0.8 $\rightarrow$ +3.6 (27B), +1.3 $\rightarrow$
+6.7 (Clef 27B) and +3.5 $\rightarrow$ +14.6 (Phi-4-mini as verifier). The set-aware map stays
within $-$0.7 \ldots{} +0.3 ($-$1.2 for Phi-4-mini at N = 32), including N = 2, 8 and 32, which it
never saw. \todo{the table file behind these numbers (tables/bon\_set\_aware\_calibration.txt,
unseen datasets, 2B generator) has a sixth verifier, Gemma-3-12b as judge, with set-aware values of
+1.64 at N = 1, $-$2.14 at N = 8 and $-$2.52 at N = 32 (single-response map +9.83 at N = 32). v4
reports ``five verifiers'' within $-$1.2 \ldots{} +0.3 (part2.md:276-277, 358; part3b.md:543-545).
Report the sixth or say why it is left out.}

Far outside the fitted range it errs on the safe side. At N = 256, sixteen times the largest fitted
N, it is underconfident by 0.1 to 2.6 points over three generators and three verifiers, where the
single-response map is overconfident by up to 15.0.

\begin{itemize}
\item \emph{Held-out problems:} $-$1.1 / $-$1.8 / $-$0.1 for the 4B / 9B / 27B verifier with the 2B
generator (single-response map +4.3 / +2.9 / +1.7), $-$2.6 / $-$2.4 / $-$1.5 with the 0.8B
generator, $-$1.3 / $-$1.2 / $-$1.3 with the Phi-4-mini generator.
\item \emph{Unseen datasets, 0.8B generator:} the single-response map is off by +15.0 / +12.7 / +6.4
points at N = 256 and the set-aware map is at $-$1.2 / $-$2.1 / $-$1.2 (+0.2 \ldots{} $-$0.9 up to N
= 64). The rule ``accept iff confidence $\geq$ .95'' accepts answers at 0.9 / 1.2 / 1.4\% error (0
of 20 splits above 5\%) against 8.0 / 8.1 / 4.1\% (20 / 20 / 1 of 20) for the single-response map.
\item \emph{Unseen datasets, 2B generator, the same problems:} single-response +12.6 / +11.5 / +5.4 at N =
256, set-aware $-$1.8 / $-$1.3 / $-$0.3, accept rule 1.2 / 1.2 / 1.5\% error at 50.8 / 53.2 / 69.5\%
coverage (0 of 20) against 7.7 / 7.6 / 3.2\% (20 / 20 / 0 of 20), and against 39.0 / 33.0 / 66.0\%
coverage for a map recalibrated at N = 256.
\end{itemize}

Acting on it is safe, and it accepts more. With the rule ``accept iff confidence $\geq$ 1 $-$
$\alpha$'' and $\alpha$ = .05 on the unseen datasets at N = 32, the single-response map accepts
answers at 5.4\% error with the 4B verifier (above the level in 17 of 20 splits), 5.8\% with the 9B
(20 of 20) and 8.0\% with Phi-4-mini (20 of 20), and the set-aware map at 1.0--2.9\% for all five
verifiers (0 of 20). Because the set mean is informative, it also accepts more answers than a map
recalibrated at that N: 50.7\% against 40.8\% (4B), 52.6\% against 29.3\% (9B).

Other domains behave the same. Reasoning sets, N = 32: +6.7 $\rightarrow$ 0.0 (9B), +3.8
$\rightarrow$ +0.2 (27B). Closed-book question answering, where the effect is largest, fitted at N =
1 and 4 only: +18.0 $\rightarrow$ +2.3 at N = 16 (4B verifier).

\textbf{One threshold can be certified for a range of N, not beyond it.} A single threshold on the
set-aware confidence was certified once on calibration outputs pooled over N = 1, 4 and 16 (map
fitted on one quarter of the problems, threshold certified on another).

\begin{itemize}
\item \emph{Unseen datasets, $\alpha$ = .05, N = 1 \ldots{} 32, our three verifiers and Clef 27B:}
accepted answers at 3.4--4.5\% error (above the level in 0--6 of 20 splits), against 3.7--4.2\% for
a threshold certified separately at each N (0--3 of 20) and up to 7.2--9.9\% for the single-response
threshold (18--20 of 20 from N = 4 on), at similar coverage (4B: 53--68\% against 53--64\%, 9B:
54--68\% against 51--64\%).
\item \emph{Held-out problems:} it holds up to N = 256 (4B verifier: 3.3--3.7\% error at 40--58\%
coverage). Thresholds certified per N on the raw score reach 16--39\% coverage, because the top of
the raw score is not monotone.
\item \emph{Other domains:} reasoning sets at $\alpha$ = .10: 7.2--9.1\%, and question answering at
$\alpha$ = .30: 25.9--28.1\% (single-response threshold: up to 39.3\%).
\item \emph{It is not exact for weak verifiers:} with Clef-flash on the held-out set the accepted answers
are at 4.7--5.6\% for $\alpha$ = .05 (single-response threshold: 5.1 $\rightarrow$ 11.7\%), and with
Phi-4-mini as verifier at 5.0\% at N = 1 (3.7--4.4\% for N $\geq$ 2).
\item \emph{It does not extrapolate as a certificate:} on the unseen datasets with the 0.8B generator the
threshold certified on N $\leq$ 16 accepts answers at 3.5--4.1\% error up to N = 8, but at
4.4--4.9\% (4B), 4.8--5.2\% (9B) and 4.5--5.0\% (27B) for N = 32 \ldots{} 256, above the level in
5--14 of 20 splits, where thresholds certified per policy stay at 3.5--4.2\% (0--2 of 20). With the
2B generator the same threshold holds for the 4B verifier at every N (3.4--3.9\%, at most 4 of 20),
runs at 4.3--4.6\% for the 9B from N = 16 on (5--7 of 20) and reaches 5.1--5.2\% for the 27B at N =
128 and 256 (11--12 of 20). The map's slight underconfidence at large N does not make a pooled
threshold safe there. A certificate for N far above the fitted range needs calibration outputs at
that N.
\end{itemize}

\todo{v4 Appendix D.1 titles this result ``One certificate for every N'' and says the threshold
``holds at every N'' (part3b.md:562-564), while v4 \S{}5.1 titles it ``One certificate for a range
of N, not beyond it'' (part2.md:288-292) and the same appendix paragraph ends with the failure
beyond N = 16 (part3b.md:572-578). The text above follows \S{}5.1; confirm.}

\textbf{What each ingredient does} (ablation: the same map without the set mean). Letting the map
depend on N is what repairs the mean calibration: a map of the selected score and N alone stays
within $\pm$0.9 points at every N on the unseen datasets. The mean score of the candidates adds
\emph{resolution} where the verifier is weak or the problems are unfamiliar. On the unseen datasets
the accept rule then covers 50.7\% instead of 39.1\% of the answers (4B) and 52.6\% instead of
34.7\% (9B), at lower error. With Clef-flash and Phi-4-mini as verifiers the N-only map lets answers
through above the level (7.1\% and 11.1\% error at N = 64 for $\alpha$ = .05, 14.1\% for $\alpha$ =
.10 on the reasoning sets), the set-aware map does not (4.5\%, 3.5\%, 7.9\%) and covers two to three
times as many answers (Brier score 12.9 $\rightarrow$ 11.8 for Phi-4-mini at N = 64). For our
verifiers on the held-out set, on the reasoning sets and in question answering the set mean adds
nothing (Brier scores within 0.1).

\textbf{Limits.} The map is fitted on best-of-N outputs, so it needs the same calibration problems
as per-policy certification. What it saves is the repetition per N. Like any calibration it has to
be fitted on problems from the deployment distribution: fitted on the held-out set and applied to
the unseen datasets it is overconfident by +1.0 $\rightarrow$ +6.1 points (4B verifier, N = 1
$\rightarrow$ 32, +0.3 $\rightarrow$ +5.6 for the 9B, +1.1 $\rightarrow$ +4.2 for the 27B), 30--40\%
less growth with N than the single-response map transferred the same way (+1.4 $\rightarrow$ +10.3,
+0.8 $\rightarrow$ +9.5, +1.3 $\rightarrow$ +5.6) but far from the $\pm$0.6 of the map fitted
in-domain. Its accept rule at $\alpha$ = .05 still holds (1.0--3.9\% error for five verifiers,
against up to 7.3\% for the transferred single-response map). Fitted at only two values of N it
extrapolates poorly when the verifier's accuracy falls with N (Clef-flash on the reasoning sets:
+6.1 at N = 16 against +7.4 for the single-response map, although its accepted answers stay below
the level, 7.9\% at $\alpha$ = .10). At N = 1 the two generalist judges with saturated scores are
fitted badly (accepted error 5.8--6.4\% at $\alpha$ = .05, on 6--9\% coverage).

\subsection{The route-aware map for the think-gate}\label{sec:D.4}

Per-route thresholds have to be redone for every think rate, so we tried the analogous map g(c1,
c0): a function of the thought confidence c1 \emph{and} of the plain confidence c0 that the gate
routes on (isotonic in c1 within eight quantile strata of c0), fitted on the thought answers of all
calibration items with no knowledge of the threshold.

\textbf{It repairs the calibration.} One such map brings the overconfidence of thought answers on
routed items to within $\pm$.02 of zero for all nine models at think rates of 10, 30 and 50\% on the
decision suite (map of c1 alone: up to +.16) and at 10, 20 and 40\% on the third-party benchmark (up
to +.21), and to within $\pm$.03 on the reasoning items, where the map of c1 alone errs in either
direction ($-$.12 to +.05). The difference in accuracy at equal mapped confidence, routed minus
kept, shrinks by roughly half on the decision suite (ours 4B $-$.194 $\rightarrow$ $-$.098, Phi-4
$-$.176 $\rightarrow$ $-$.017, ours 9B $-$.214 $\rightarrow$ $-$.167) and to between +.01 and $-$.11
on the benchmark (from $-$.02 \ldots{} $-$.30). \todo{``within $\pm$.02'' here (part2.md:309-310,
part3b.md:605-606) against ``$-$1.5 \ldots{} +2.1'' points for the same setting in v4 Table 6
(part2.md:360); the upper end is +.021.}

\textbf{It does not repair the certificate.} One threshold for all final answers still lets thought
answers through above the level. Ours 4B at $\alpha$ = .10 and a 30\% think rate: 12.6\% error with
the map of c1 alone (above the level in 16 of 20 splits), 10.7\% with the route-aware map (9 of 20).
Ours 9B 22.2\% $\rightarrow$ 20.5\% (20 $\rightarrow$ 18 of 20). On the benchmark at a 20\% think
rate 15.3\% $\rightarrow$ 14.6\% and 27.1\% $\rightarrow$ 22.0\% (19--20 of 20 throughout).
Per-route thresholds: 0--1 of 20 on the decision suite, 0--3 on the benchmark, mostly by accepting
no thought answer at all.

\textbf{Acting on the mapped confidence directly} (accept a thought answer iff its mapped confidence
$\geq$ 1 $-$ $\alpha$, third-party benchmark, ours 9B). The map of c1 alone accepts thought answers
at 27--32\% error for $\alpha$ = .25 (above the level in 18--19 of 20 splits at think rates of 10
and 20\%) and at 16--23\% for $\alpha$ = .10 (20 of 20). The route-aware map accepts fewer and is
above the level in 0--2 of 20 splits at $\alpha$ = .25, like a map fitted on the routed items alone
(0--3 of 20), without knowing the threshold. At $\alpha$ = .10 both accept almost nothing (at most
0.7\% of the routed items), and the few they accept are still at 15--21\% error: the top bin of an
isotonic map is not a certificate. For the 4B model every map passes this rule (at most 8.6\% error
at $\alpha$ = .10).

\textbf{Why.} The reason is not residual miscalibration but Proposition 3. A certificate for the
mixture is carried by the kept answers, which are many and safe. It bounds the error of the pool and
is silent about the route, however well calibrated the confidence. A route-aware map is the right
confidence to \emph{report}. The guarantee for the answers the system paid extra for still has to be
certified per route.

\subsection{Cascades and select-then-think}\label{sec:D.5}

The same code with other inputs gives the maps for the two remaining policies.

\textbf{Cascades.} With 30\% of the items escalated, the large model's answers on the escalated
items are overconfident by 11 to 18 points raw, and still by 2.3 to 8.4 points after the usual
calibration on all of its answers. A map that also sees the small model's confidence leaves $-$0.6
to +0.5: for cascades of our models, of another team's models (Clef-flash $\rightarrow$ Clef 27B:
+3.3 $\rightarrow$ +0.1), and across teams. The difference in accuracy at matched confidence between
escalated and kept items shrinks from $-$.10 \ldots{} $-$.22 to $-$.03 \ldots{} $-$.10. As for
gates, one threshold for all answers still lets escalated answers through above the level, and
thresholds certified per route hold (Proposition 3).

\textbf{Select-then-think.} The usual map is fitted on the thought confidence of single responses.
It is overconfident by +0.4 to +2.2 points at N = 2 and by +2.1 to +7.3 at the largest N of each
setting (64 on held-out problems, 8 on the unseen datasets and the reasoning sets). The policy-aware
map, fitted at N = 2 and 4 (and 16 on held-out problems), stays within $-$1.4 \ldots{} +0.7 at every
N, including values it never saw. Acting on it is safer and stricter: with the weaker generator at N
= 64, the rule ``accept iff confidence $\geq$ .95'' accepts 90\% of the answers at 4.4\% error under
the usual map, above the level in 8 of 20 splits, and 56\% at 2.7\% error under the policy-aware
map, in none. On these problems a map of the confidence and N alone does as well. The statistics of
the candidate set matter where the verifier is weak or the problems are unfamiliar (D.3).

\subsection{A system we did not build, and tables published by other groups}\label{sec:D.6}

\textbf{Public records of a two-model system.} System Switch {[}REF: System Switch, code and
per-question records public, 5 October 2026, preprint announced, not peer-reviewed{]} lets a
typed-decision actor play a first-person game and sends its least confident decisions to a separate
vision reasoner. Its authors publish, per question, the actor's confidence and whether actor and
reasoner are right, for eleven actors under two orders of the options and for two reasoners, on 600
held-out decisions. That makes 21 distinct settings, one actor being indifferent to the order. We
used the records for evaluation only.

The reasoner states no confidence, so what a user has for it is its accuracy: 69.0\% over all
questions for the study's reasoner. On the 30\% of the questions that an actor defers (the study's
own rate) it is right between 49.4\% and 78.9\% of the time, depending on the actor. In 9 of the 21
settings the difference from the overall figure lies outside a 95\% interval that resamples games,
and in all nine the deferred questions are the harder ones for the reasoner, by 8 to 20 points. As
in Proposition 2, one number says which way it goes: the AUROC of the actor's confidence for the
\emph{reasoner's} correctness ranges from 0.44 to 0.72 and orders the settings almost exactly
(Spearman 0.92). The reasoner does worse on the deferred questions in 15 of the 16 settings above
0.5 and better in all 5 below.

Estimated on other games, the overall accuracy misses the accuracy on the deferred questions by
$-$10.7 to +18.1 points, 8.3 in mean absolute value. The route-aware map for a model that reports a
constant is its accuracy within strata of the actor's confidence (five strata at this sample size).
It misses by $-$7.4 to +4.4 points, 2.1 in mean absolute value, which is within the sampling error
of 180 questions, and is the closer estimate in 19 of the 21 settings (in 110 of 126 over the
study's six reasoner records, 2.8 against 10.7 points). The control behaves as Proposition 4 says:
the actor's own confidence, calibrated without the gate, is off by only $-$4.0 to +1.7 points (1.1
in mean absolute value) on the answers the actor keeps, because the gate is a function of that
confidence. A system of two models is a baseline in this report and not our method. The effect and
the remedy do not depend on who built the models. \todo{cite the preprint when it appears and
re-read it for the figures taken from its repository (paper\_v4\_todo.md:60-63); decide whether the
analysis script, which contains the record file names, is released.}

\textbf{Tables already published by other groups.} The gap is also visible in tables that other
groups have published, without being named. In one accept-or-escalate judge {[}REF{]}  the reasoning
model is right on 94.4\% of the items the first stage keeps and on 75.0\% of the items escalated to
it, 90.0\% overall. In a study of rubric judges {[}REF{]}  the fallback is right on 54--72\% of the
deferred pairs against 76--85\% of the kept ones on five panels, with one panel level and one
reversed. The sign is not universal there either. \todo{these two sets of figures were read from the
cited papers by an assistant, not by an author; check them against the PDFs before release
(paper\_v4\_todo.md:64-70).}

\subsection{Certificates across task families}\label{sec:D.7}

Certificates are marginal over the calibration distribution. They do not transfer across task
families. A certificate has to be repeated when the policy changes (another N, another think rate,
another generator) and when the task family changes. \todo{v4 states this in its limitations
(part3b.md:7, ``Appendix D'') and in \S{}5.4 (part2.md:424-425) and announces the evidence for an
appendix section that it does not contain (``D (continued). Certificates across task families'',
part3b.md:842). The measurements exist in the lab notebook (paper\_draft.md:467-468 and 484-487) and
in tables/t3\_risk\_family\_4b.txt; they were not copied here because v4 has no text for them.}

\subsection{Calibrating the confidence after reasoning on real-task items}\label{sec:D.8}

One temperature fitted on 3,700 unseen real-task traces transfers to 32 unseen task families. Every
correction fitted on synthetic data fails. Table~\ref{tab:E.1} reports thought distributions after
one temperature. Fusing the plain and the thought readout is treated in C.4. \todo{the details were
announced for the same unwritten appendix section (``calibration on unseen real-task items'',
part3b.md:842-843); the lab notebook has the measurements (paper\_draft.md:473-482,
tables/s33\_cal\_size.txt).}
