# Supplementary material for: StartLux-Decision: AutoThink Decision Models with Reinforcement Learning for Calibrated Deliberative Decisions
Source: arXiv:2610.17309 source file (2026-10-20)
Supplement: Supplementary file 9 [file appendix_D_reasoning.tex]

\section{Stage 3 designs and reinforcement learning}\label{sec:D}

Unless a table says otherwise, Stage 3 here starts from the 4B Stage 2 checkpoint on the earlier mix
and uses causal attention. Held-out results are on the 3,021 items of the training distribution that
the 4B routes to reasoning, 13 of which were also in Stage 3 training lists, an effect of at most
about 0.4 points \todo[TODO(clean held-out)]{repeat on the 3,008 clean items}.

\subsection{The closing probability per step}\label{sec:D.1}

The probe feeds the item's prompt and a stored thought to a model and reads the probability that the
closing tag follows within two tokens, at the natural end of a thought that its writer closed.
Control points inside the thoughts have a median of 0.00 for every model.

\begin{table}[!htbp]
\renewcommand{\thetable}{D.1}
\centering
\caption{The closing probability falls with a loss on the answer alone and returns after thinking replay at every size. Median probability of closing a thought at its natural end over 400, 300 and 200 thoughts (4B, 9B, 27B), whose intervals Figure~\ref{fig:4} draws for the base-written thoughts. Writer: the base model, or the model after thinking replay.}\label{tab:D.1}
{\small\setlength{\tabcolsep}{6pt}\renewcommand{\arraystretch}{1.1}
\noindent\begin{adjustbox}{max width=\linewidth}
\begin{tabular}{lrrrrr}
\toprule
\textbf{size, writer} & {\begin{tabular}[b]{@{}r@{}}\textbf{base}\\\textbf{model}\end{tabular}} & {\begin{tabular}[b]{@{}r@{}}\textbf{Stage}\\\textbf{2}\end{tabular}} & {\begin{tabular}[b]{@{}r@{}}\textbf{Stage 2}\\\textbf{+ reader}\\\textbf{round}\end{tabular}} & {\begin{tabular}[b]{@{}r@{}}\textbf{Stage}\\\textbf{2 +}\\\textbf{replay}\end{tabular}} & {\begin{tabular}[b]{@{}r@{}}\textbf{replay,}\\\textbf{then reader}\\\textbf{round}\end{tabular}} \\
\midrule
4B, base & 0.52 & 0.52 & 0.47 & 0.73 & 0.26 \\
4B, replayed & 0.72 & 0.59 & 0.64 & 0.89 & 0.39 \\
9B, base & 0.54 & 0.06 & 0.02 & 0.81 & 0.18 \\
9B, replayed & 0.65 & 0.05 & 0.02 & 0.93 & 0.27 \\
27B, base & -- & 0.84 & -- & 0.97 & 0.54 \\
27B, replayed & -- & 0.86 & -- & 0.98 & 0.87 \\
\bottomrule
\end{tabular}
\end{adjustbox}\par}
\end{table}

A loop sustains itself: inside a loop the median closing probability is 0.00 for every 4B step, the
base model included. The weight update of the reader round is close to orthogonal to that of
thinking replay (cosine $-$0.0022), so it does not undo the replay but moves something else that the
closing decision depends on.

\subsection{Every reasoning design on the index}\label{sec:D.2}

\begin{table}[!htbp]
\renewcommand{\thetable}{D.2}
\centering
\caption{Replay followed by the reader round scores highest among the causal designs, and the stop step keeps most of the gain at 43\% of the reasoning tokens. Decision Index 0.2.1 at 4B, gate 0.9, one run each. Reasoning tokens per answer: mean over all answers.}\label{tab:D.2}
{\footnotesize\setlength{\tabcolsep}{6pt}\renewcommand{\arraystretch}{1.1}
\noindent\begin{adjustbox}{max width=\linewidth}
\begin{tabular}{lrrrrr}
\toprule
\textbf{design (4B)} & \textbf{index} & \textbf{knowledge} & {\begin{tabular}[b]{@{}r@{}}\textbf{tokens}\\\textbf{per}\\\textbf{thought}\end{tabular}} & {\begin{tabular}[b]{@{}r@{}}\textbf{at}\\\textbf{the}\\\textbf{limit}\end{tabular}} & {\begin{tabular}[b]{@{}r@{}}\textbf{reasoning}\\\textbf{tokens per}\\\textbf{answer}\end{tabular}} \\
\midrule
one pass, Stage 2 on the earlier mix & 64.78 & 45.4 & -- & -- & -- \\
reader round only & 66.38 & 50.0 & 388 & 0.6\% & 125 \\
replay, then reader round & \textbf{67.72} & 57.0 & 3,439 & 57.5\% & 1,144 \\
\ldots{} thought cut at 1,024 tokens & 66.93 & 53.8 & 1,003 & -- & 333 \\
\ldots{} + stop step (Auto-Think) & 67.37 & 55.7 & 1,585 & 10.4\% & 497 \\
\ldots{} + stop step + RL, rollouts at temperature 1 & 67.23 & 55.1 & 1,053 & 3.2\% & 330 \\
\ldots{} + stop step + RL, rollouts as at inference & 66.80 & 53.5 & 617 & 0.4\% & 200 \\
base model writes the thought, the replay-then-reader model reads it & 67.62 & 57.7 & 1,316 & 8.7\% & 438 \\
joint stage (D.4) & 67.11 & 57.0 & 2,666 & 39.9\% & 1,254 \\
RL from the Stage 2 checkpoint \textsuperscript{e} & 67.18 & 53.5 & 184 & 0.7\% & 57 \\
Instant recipe, bidirectional: replay, then reader round \textsuperscript{b} & 68.33 & -- & 3,394 & -- & 1,032 \\
\ldots{} + stop step \textsuperscript{b} & 67.99 & -- & 1,652 & -- & 478 \\
\bottomrule
\end{tabular}
\end{adjustbox}\par}
\par\smallskip
{\footnotesize\raggedright\noindent \textsuperscript{e} 78.5\% of its thoughts have fewer than 16 tokens: it skips most questions it is
asked to reason about. \textsuperscript{b} Reference runner, on which the causal replay-then-reader
model scores 67.58.\par}
\end{table}

\subsection{Limit, cut and gate}\label{sec:D.3}

On the held-out items the default answer of the replay-then-reader 4B is 75.54 at the 4,096-token
limit. A limit of 16,384 tokens leaves it where it was (+0.07 against its own reference, interval
$-$0.56 to +0.73), with 87.4\% of the thoughts still running. A cut at 1,024 tokens changes it by
+0.00 ($-$0.60 to +0.63), and a repetition penalty with a loop check by $-$0.53 ($-$1.16 to +0.10).
On the index a limit of 8,192 tokens scores 67.52, and the cut at 1,024 tokens costs 0.79 points.
Thoughts written by the base model need a reader trained on thoughts: read by a reader round without
replay the default answer is 75.47, read by the Stage 2 checkpoint 67.06. A gate of 0.7 is free on
8,598 held-out items but costs half a point on the index (67.20), and 0.98 gives 67.51. No rule that
sets the weight of the thought from the one-pass confidence beats the flat 0.5 / 0.5 mixture (90.12
at 4B, 92.96 at 9B on held-out items).

\subsection{The joint stage}\label{sec:D.4}

The joint stage replaces the three steps by one with thinking and read-out targets in every step
(747 steps). It gives the best default answer on diagnostic items (76.5) but trails the sequence on
held-out items (74.91 against 75.54), and on the index it scores 67.11 with the gate firing on 47\%
of the answers instead of 33\%.

\subsection{Reinforcement learning}\label{sec:D.5}

The thought tokens are trained through a low-rank adapter for 120 iterations (learning rate 1e-5,
penalty 0.02 towards the starting policy) with the read-out fixed, on prompts from 26,931 items
whose one-pass top probability is below 0.9. Rollouts are sampled at temperature 1 or as at
inference (temperature 0.6, top-p 0.95, top-k 20).

\begin{table}[!htbp]
\renewcommand{\thetable}{D.3}
\centering
\caption{With a price for length, reinforcement learning ends nearly every thought at about a third of the tokens, and no arm that starts from a model that reasons beats its start. Held-out items, one thought per item with the decoding of inference. Last column: paired difference to the arm's start with its 95\% interval, for the answer after the thought (T) or the default answer (D), on the test part of the items (2,132 at 4B) for arms that start after the stop step.}\label{tab:D.3}
{\footnotesize\setlength{\tabcolsep}{4pt}\renewcommand{\arraystretch}{1.1}
\noindent\begin{adjustbox}{max width=\linewidth}
\begin{tabular}{llrrrrr}
\toprule
\textbf{start and arm} & \textbf{rollouts} & {\begin{tabular}[b]{@{}r@{}}\textbf{thoughts}\\\textbf{that end}\end{tabular}} & {\begin{tabular}[b]{@{}r@{}}\textbf{tokens}\\\textbf{per}\\\textbf{thought}\end{tabular}} & {\begin{tabular}[b]{@{}r@{}}\textbf{after the}\\\textbf{thought}\end{tabular}} & {\begin{tabular}[b]{@{}r@{}}\textbf{default}\\\textbf{answer}\end{tabular}} & \textbf{difference to the start} \\
\midrule
4B, Stage 2 checkpoint (start) & -- & 92.4\% & 639 & 72.29 & 74.02 & -- \\
\ldots{} log score & temperature 1 & 97.6\% \textsuperscript{a} & 255 & 74.25 & 75.41 & T +1.95 {[}+0.73, +3.21{]} \\
4B, replay, reader round, stop step (start) & -- & 85.9\% & 1,413 & 74.38 & 75.31 & -- \\
\ldots{} bounded proper score & as at inference & 99.7\% & 503 & 74.11 & 75.07 & T $-$1.17 {[}$-$2.11, $-$0.28{]} \\
\ldots{} the same, second run & as at inference & 100\% & 485 & 74.21 & 75.31 & T $-$1.03 {[}$-$2.06, $-$0.28{]} \\
\ldots{} accuracy reward & as at inference & 99.8\% & 433 & 73.78 & 74.71 & T $-$1.64 {[}$-$2.67, $-$0.66{]} \\
\ldots{} the same, second run & as at inference & 99.8\% & 439 & 73.72 & 74.74 & T $-$1.03 {[}$-$2.11, $-$0.09{]} \\
\ldots{} no price for length & as at inference & 59.4\% & 2,581 & 74.58 & 75.50 & T $-$0.70 {[}$-$1.69, +0.19{]} \\
\ldots{} closing bonus in place of the price & as at inference & 98.4\% & 971 & 74.28 & 75.07 & T $-$0.75 {[}$-$1.78, +0.14{]} \\
\ldots{} noise as reward & temperature 1 & 99.2\% & 600 & 73.68 & 74.08 & T $-$1.22 {[}$-$2.25, $-$0.14{]} \\
4B, replay, then reader round (start) & -- & 11.4\% & 3,764 & 75.04 & 75.54 & -- \\
\ldots{} bounded proper score & as at inference & 58.0\% & 2,753 & 74.18 & 74.94 & T $-$0.86 {[}$-$1.82, +0.03{]} \\
9B, replay, reader round, stop step (start) & -- & 77.7\% & 1,677 & 81.20 & 82.06 & -- \\
\ldots{} bounded proper score & as at inference & 99.8\% & 544 & 80.87 & 81.60 & D $-$0.75 {[}$-$1.27, $-$0.14{]} \\
\ldots{} accuracy reward & as at inference & 99.7\% & 612 & 81.17 & 82.03 & D $-$0.28 {[}$-$0.84, +0.28{]} \\
\bottomrule
\end{tabular}
\end{adjustbox}\par}
\par\smallskip
{\footnotesize\raggedright\noindent \textsuperscript{a} 66.3\% of the thoughts are closed at once.\par}
\end{table}

Read before any temperature is fitted, the calibration error of the 4B's answer after the thought
falls from 9.48 to 6.93 and 6.54 in the two runs of the proper score and to 7.79 and 7.28 with the
accuracy reward. It stays at 9.10 with the closing bonus and rises to 11.19 without a price. The
ranking does not improve: with the proper score the share of 4B answers that can be accepted at an
error of 5\% is 20.5\% before and 18.0\% after. Every arm was trained with the rank-initialisation
fault of Section~\ref{sec:5}. The port to slime (all weights, two nodes) matches our loop over its
first five steps, with accuracy after the thought 0.876 against 0.873 \todo[TODO(RL corrected)]{the
accuracy-reward arm with the fixed loop and the slime run}.

\todo[TODO(appendix)]{add moved-out material from sections 1-6}
