# Supplementary material for: StartLux-Decision: AutoThink Decision Models with Reinforcement Learning for Calibrated Deliberative Decisions
Source: arXiv:2610.17309 source file (2026-10-20)
Supplement: Supplementary file 10 [file appendix_E_evaluation.tex]

\section{Evaluation details}\label{sec:E}

\subsection{The index suite and its settings}\label{sec:E.1}

Decision Index 0.2.1 averages 38 benchmarks in five areas (weights in Table~\ref{tab:E.1}). Inside
an area the benchmarks marked $\bigstar$ weigh 1.2 and the others 1.0. Each score is corrected for
chance, (score $-$ chance) / (1 $-$ chance) clipped to 0--1, and for coverage, so an unanswered
request counts as wrong.

All benchmarks use one prompt and the letter read-out, without benchmark-specific prompts,
instructions or temperatures. Lists of more than 26 options go through a knock-out: groups of at
most 25 options, and the best three of each group meet in a final round. The retrieval benchmarks
are stored as one yes/no question per candidate (about 3\% relevant) and ranked by the probability
of yes.

Evaluation items were never trained on, but data aimed at a benchmark can be in the mix. For the
released weights of every size 18 of the 38 benchmarks have an official training split in it, and
after the data rounds (adapter training on targeted typed decisions) 33 have aimed-at data. For GPQA
Diamond and MMLU-Pro the mix holds only general multiple-choice rows in their layout, and tool
retrieval, HLE and CRUXEval are read zero-shot.

Repeating a reasoning run with thoughts sampled anew moves the index by 0.05 and the areas by at
most 0.24, and 97.0\% of the 337,742 answers are the same choice. Retraining moves it more: the same
recipe trained twice gives 60.69 and 60.87, with single benchmarks up to 7 points apart, and three
rounds of nearly the same final recipe span 64.76 to 65.67. Half an index point between two training
rounds is therefore not evidence of a cause.

\subsection{Per-benchmark results}\label{sec:E.2}

Table~\ref{tab:E.1} gives every benchmark of the index for the released 27B and 9B, the hosted
reference, and the 27B after the data rounds in one pass and with reasoning.

\begingroup
\renewcommand{\thetable}{E.1}
\footnotesize\setlength{\tabcolsep}{4pt}\renewcommand{\arraystretch}{1.1}
\begin{longtable}{lrlrrrrr}
\caption{The released 27B is above the hosted reference on 31 of the 38 benchmarks and below it in knowledge and reasoning. The 38 benchmarks of Decision Index 0.2.1: weight (\%), training data aimed at the benchmark in the released weights and after the data rounds (T official training split or training set of its source, G our generator or written data in its layout with nothing of the benchmark in it, R related public data in its layout, a hyphen for nothing), and scores in the benchmark's own metric (\%). Released 27B and 9B: own runs, 2026-09-27 to 2026-10-01. Jev 1.13, the hosted reference: public board, 2026-09-28. 27B after the data rounds: own runs on the corrected serving path, one pass (2026-10-06) and reasoning (2026-10-07) (a thought when the one-pass top probability is below 0.9), after thinking replay, which trains the model to write and close thoughts, and the reader round, which trains the answer read after a thought (Section~\ref{sec:5.3}).}\label{tab:E.1}\\
\toprule
\textbf{benchmark} & {\begin{tabular}[b]{@{}r@{}}\textbf{weight,}\\\textbf{\%}\end{tabular}} & {\begin{tabular}[b]{@{}l@{}}\textbf{aimed-at}\\\textbf{data: released}\\\textbf{/ after rounds}\end{tabular}} & {\begin{tabular}[b]{@{}r@{}}\textbf{27B}\\\textbf{released}\end{tabular}} & {\begin{tabular}[b]{@{}r@{}}\textbf{Jev}\\\textbf{1.13}\end{tabular}} & {\begin{tabular}[b]{@{}r@{}}\textbf{9B}\\\textbf{released}\end{tabular}} & {\begin{tabular}[b]{@{}r@{}}\textbf{27B after}\\\textbf{rounds,}\\\textbf{one pass}\end{tabular}} & {\begin{tabular}[b]{@{}r@{}}\textbf{27B after}\\\textbf{rounds,}\\\textbf{reasoning}\end{tabular}} \\
\midrule
\endfirsthead
\multicolumn{8}{l}{\textit{Table~\thetable{} (continued)}}\\
\toprule
\textbf{benchmark} & {\begin{tabular}[b]{@{}r@{}}\textbf{weight,}\\\textbf{\%}\end{tabular}} & {\begin{tabular}[b]{@{}l@{}}\textbf{aimed-at}\\\textbf{data: released}\\\textbf{/ after rounds}\end{tabular}} & {\begin{tabular}[b]{@{}r@{}}\textbf{27B}\\\textbf{released}\end{tabular}} & {\begin{tabular}[b]{@{}r@{}}\textbf{Jev}\\\textbf{1.13}\end{tabular}} & {\begin{tabular}[b]{@{}r@{}}\textbf{9B}\\\textbf{released}\end{tabular}} & {\begin{tabular}[b]{@{}r@{}}\textbf{27B after}\\\textbf{rounds,}\\\textbf{one pass}\end{tabular}} & {\begin{tabular}[b]{@{}r@{}}\textbf{27B after}\\\textbf{rounds,}\\\textbf{reasoning}\end{tabular}} \\
\midrule
\endhead
\bottomrule
\endfoot
\multicolumn{8}{l}{\textbf{Knowledge and reasoning, area weight 25.8\%}} \\
GSM8K \textsuperscript{a} & 2.39 & T / T & 96.4 & 79.9 & 95.7 & 96.13 & 99.62 \\
ChessBench & 2.39 & - / G & 18.0 & 17.2 & 13.0 & 25.32 & 26.44 \\
MuSR & 2.39 & - / G & 67.8 & 66.1 & 59.0 & 72.47 & 68.88 \\
SATA-Bench & 2.39 & - / G, T & 10.5 & 26.4 & 26.3 & 58.97 & 55.03 \\
GPQA Diamond $\bigstar$ & 2.87 & - / - & 50.5 & 78.6 & 50.0 & 50.00 & 69.39 \\
CRUXEval & 2.39 & - / - & 75.8 & 73.0 & 60.0 & 76.49 & 96.14 \\
CLadder & 2.39 & - / G & 73.7 & 72.6 & 68.1 & 90.96 & 93.66 \\
HLE $\bigstar$ & 2.87 & - / - & 12.4 & 20.4 & 10.2 & 13.17 & 13.17 \\
MMLU-Pro $\bigstar$ & 2.87 & - / - & 69.8 & 82.7 & 61.3 & 69.47 & 82.28 \\
BBH $\bigstar$ & 2.87 & - / G & 80.2 & 92.9 & 71.2 & 90.34 & 92.52 \\
\midrule
\multicolumn{8}{l}{\textbf{Language, area weight 25.8\%}} \\
ContractNLI & 2.43 & T / T & 86.4 & 71.7 & 86.6 & 85.62 & 85.80 \\
ANLI $\bigstar$ & 2.92 & T / T & 77.9 & 74.8 & 76.4 & 78.97 & 79.47 \\
WinoGrande $\bigstar$ & 2.92 & T \textsuperscript{b} / T & 93.5 & 92.0 & 91.5 & 93.76 & 93.69 \\
HellaSwag $\bigstar$ & 2.92 & T \textsuperscript{b} / T & 97.6 & 94.5 & 96.8 & 97.54 & 97.49 \\
ACOS & 2.43 & T / T & 52.0 & 29.5 & 47.8 & 65.46 & 63.53 \\
FinEntity & 2.43 & - / R & 92.7 & 87.0 & 88.2 & 95.24 & 94.79 \\
iSarcasmEval & 2.43 & T / T & 63.0 & 50.5 & 62.6 & - \textsuperscript{c} & - \textsuperscript{c} \\
VAST & 2.43 & T / T & 82.3 & 64.6 & 79.1 & 80.78 & 81.01 \\
NLI4CT & 2.43 & T / T & 85.8 & 84.1 & 82.6 & 85.60 & 86.44 \\
RAGTruth & 2.43 & T / T & 85.6 & 76.5 & 84.3 & 86.14 & 85.71 \\
\midrule
\multicolumn{8}{l}{\textbf{Retrieval and classification, area weight 20.0\%}} \\
BANKING77 $\bigstar$ & 3.64 & T / T & 91.0 & 79.7 & 91.4 & 91.14 & 90.88 \\
CLINC150 $\bigstar$ & 3.64 & T / T & 93.0 & 89.3 & 93.2 & 93.63 & 94.24 \\
BRIGHT $\bigstar$ & 3.64 & - / G & 50.0 & 47.5 & 48.1 & 47.86 & 49.52 \\
Amazon ESCI & 3.03 & T / T & 58.5 & 55.2 & 58.1 & 64.34 & 64.60 \\
PhishNChips & 3.03 & - / G & 70.5 & 62.5 & 64.2 & 92.50 & 92.70 \\
HoVer & 3.03 & T / T & 89.6 & 72.9 & 88.2 & 89.60 & 89.05 \\
\midrule
\multicolumn{8}{l}{\textbf{Tools and automation, area weight 18.3\%}} \\
BFCL $\bigstar$ & 4.07 & R / R & 97.6 & 95.8 & 97.8 & 98.29 & 98.05 \\
ToolRet & 3.39 & - / - \textsuperscript{d} & 69.1 & 65.3 & 66.6 & 69.30 & 68.40 \\
API-Bank $\bigstar$ & 4.07 & T \textsuperscript{b} / R & 84.1 & 88.2 & 78.3 & 81.50 & 88.19 \\
Home appliance simulator & 3.39 & - / G & 77.3 & 52.3 & 38.6 & 100.00 & 94.32 \\
When2Call & 3.39 & T / T & 89.2 & 81.0 & 88.9 & 92.96 & 91.73 \\
\midrule
\multicolumn{8}{l}{\textbf{Arts and human taste, area weight 10\%}} \\
BPoMP & 1.39 & - / G & 95.3 & 90.9 & 91.0 & 96.78 & 96.82 \\
Humicroedit & 1.39 & - \textsuperscript{b} / T & 62.9 & 61.9 & 62.2 & 66.70 & 66.32 \\
POP909-CL & 1.39 & - / G & 51.0 & 16.6 & 26.1 & 83.35 & 83.55 \\
cfcolor & 1.39 & T \textsuperscript{b} / T & 71.8 & 64.4 & 71.2 & 71.12 & 70.68 \\
ForecastBench $\bigstar$ & 1.67 & - / T & 34.3 & 30.6 & 26.6 & 17.02 & 17.41 \\
Habermas & 1.39 & - / T & 43.8 & 45.9 & 46.6 & 63.66 & 60.32 \\
New Yorker & 1.39 & T / T & 79.4 & 70.1 & 77.6 & 80.49 & 81.06 \\
\end{longtable}
\endgroup
\par\smallskip
{\footnotesize\raggedright\noindent \textsuperscript{a} Rows of edition 0.2.1, whose wrong options give the answer away. On the rows
rebuilt for edition 0.3 our runs of 7 October 2026 give a one-pass skill of 60.5 for the released
27B, 30.8 for the released 9B and 53.7 for the 27B after the data rounds, against 95.3, 94.3 and
94.9 on the old rows (Table~\ref{tab:E.7}). The hosted reference has 66 in the board data.\par}
\par\smallskip
{\footnotesize\raggedright\noindent \textsuperscript{b} For the released weights, the full-fine-tuning mixes of every size hold the
official splits of API-Bank (6,379 rows) and cfcolor (3,396), HellaSwag has 20,130 rows at 0.8B to
9B and 24,522 at 27B, and Humicroedit has one row.\par}
\par\smallskip
{\footnotesize\raggedright\noindent \textsuperscript{c} Not listed in the table of the run.\par}
\par\smallskip
{\footnotesize\raggedright\noindent \textsuperscript{d} Rounds before the final recipe held its official training rows, which cost the
benchmark 26 points. The final recipe holds none of them (its file list, 5 October 2026).\par}

The released 27B is below the hosted reference on seven benchmarks (GPQA Diamond, MMLU-Pro, BBH,
HLE, SATA-Bench, API-Bank and Habermas) and above it on the other 31 in the board's skill values,
GSM8K among them on the old rows. HLE is below its 16.4\% chance level for every model of ours and
adds zero to the index. The data rounds act where data was aimed (for the 27B +49.1 skill points on
SATA-Bench, +44.1 on PhishNChips and +34.6 on CLadder), and ForecastBench is the one benchmark that
they lower clearly (34.3 to 17.02 at 27B, 26.6 to 16.88 at 9B), for a reason we have not traced.

Reasoning pays where a thought can compute or check: at the 27B, CRUXEval goes from 76.49 to 96.14,
MMLU-Pro from 69.47 to 82.28 and GPQA Diamond from 50.00 to 69.39 (at the 9B 60.35 to 88.42, 60.71
to 73.65 and 51.53 to 62.24). The home appliance simulator (100 to 94.32), SATA-Bench (58.97 to
55.03), MuSR (72.47 to 68.88) and Habermas (63.66 to 60.32) lose most.

\subsection{Other evaluations}\label{sec:E.3}

All sets in this section are for evaluation only, except that the training split of Typed Decisions,
a suite of the JevBench bundle, is in every mix (Table~\ref{tab:E.2} gives the results by size).

\begin{table}[!htbp]
\renewcommand{\thetable}{E.2}
\centering
\caption{Retrieval of a planted fact is saturated from 4B on, and long-document reasoning is where the family trails. Released models on public evaluations (own runs of 2026-09-27 to 2026-10-05, one pass). JevBench: correct answers on the 231 public items (hard tier of 111 in brackets) and average over the seven suites of the Intern-Decision bundle. Needle items: correct of 180 in the runtime check at 256K tokens. LongBench v2: accuracy on 297 items. Images: mean accuracy over eight public benchmarks, with the starting model of that size (the model it was trained from) in brackets. CJ-Bench, general domain: accuracy / calibration error in percent. Jev 1.13: bundle README and benchmark authors. A hyphen means not run.}\label{tab:E.2}
{\scriptsize\setlength{\tabcolsep}{4pt}\renewcommand{\arraystretch}{1.1}
\noindent\begin{adjustbox}{max width=\linewidth}
\begin{tabular}{lrrrrrr}
\toprule
\textbf{model} & {\begin{tabular}[b]{@{}r@{}}\textbf{JevBench:}\\\textbf{correct of 231}\\\textbf{(hard tier of 111)}\end{tabular}} & {\begin{tabular}[b]{@{}r@{}}\textbf{JevBench:}\\\textbf{seven-suite}\\\textbf{average}\end{tabular}} & {\begin{tabular}[b]{@{}r@{}}\textbf{needle items,}\\\textbf{correct of 180}\end{tabular}} & {\begin{tabular}[b]{@{}r@{}}\textbf{LongBench}\\\textbf{v2}\end{tabular}} & {\begin{tabular}[b]{@{}r@{}}\textbf{images: mean}\\\textbf{accuracy}\\\textbf{(starting model)}\end{tabular}} & {\begin{tabular}[b]{@{}r@{}}\textbf{CJ-Bench}\\\textbf{general:}\\\textbf{accuracy / error}\end{tabular}} \\
\midrule
\mdourrow StartLux-Decision-0.8B & 179 (66) & 85.03 & 168 & - & - & 57.30 / 7.37 \\
\mdourrow StartLux-Decision-2B & 196 (80) & 88.46 & 175 & - & - & 61.62 / 3.06 \\
\mdourrow StartLux-Decision-4B & 204 (84) & 91.17 & 180 & 45.1 & 81.2 (76.8) & 65.16 / 6.01 \\
\mdourrow StartLux-Decision-9B & 201 (83) & 91.08 & 180 & 50.5 & 82.7 (80.3) & 67.01 / 3.83 \\
\mdourrow StartLux-Decision-27B & 208 (88) & 91.82 & 180 & 60.9 & 84.1 (80.5) & 69.39 / 5.62 \\
\mdourrow StartLux-Decision-35B-A3B & 210 (91) & 92.29 & 180 & - & 84.9 (81.3) & - \\
Jev 1.13, hosted reference & 199 (80) & 88.74 & - & - & - & 68.35 / 11.45 \\
\bottomrule
\end{tabular}
\end{adjustbox}\par}
\end{table}

\textbf{Public JevBench items.} The bundle's own scorer is used, so the values are not the official
JevBench score. A thought before every answer takes the released 27B to 229 of 231 items. The
seven-suite average is not zero-shot: the training split of Typed Decisions is in every mix, ToolACE
comes from a public training set without a held-out split, and we watched the average while choosing
checkpoints.

\textbf{Long context.} Retrieval of a planted fact is saturated from 4B up to 248K tokens (accuracy
100 at 160K--248K tokens for the 4B, 9B, 27B and 35B-A3B). Reasoning over long documents is the open
part: on the long bucket of LongBench v2 (32K--128K tokens) the 27B reaches 59 with the whole
document and 43 with its first 8K tokens only.

\textbf{Reranking.} On BEIR SciFact and NFCorpus (nDCG@10, 100 test queries each) the 27B after the
data rounds scores 0.836 and 0.436 against 0.824 and 0.425 for Jev 1.13 as reported by the test's
authors (2026-10-05), a paired difference of +0.012 {[}$-$0.010, +0.034{]} and +0.011 {[}$-$0.008,
+0.029{]}. The released 27B and the 9B are level too, and the 4B is behind on SciFact by 0.04 to
0.05. None of the test's 126 queries of five or more words occurs in 1,546,178 training records.

\textbf{Images.} No image was in the training data, so every image result is zero-shot. Decision
training on text raised the mean over eight public benchmarks by 2.4 to 4.4 points at every size
measured and lowered one benchmark, POPE at 9B, by 1.7.

\textbf{Chinese decisions.} CJ-Bench is a third-party set of 307,900 Chinese decisions in four
domains. With no Chinese decision data in training, the released 27B is above the hosted model in
all four domains in accuracy (medical 84.88 against 84.29, legal 73.12 against 68.35, finance 80.22
against 78.39, and the general domain of Table~\ref{tab:E.2}) and in calibration error. The weak
spot is the score question: 46.6\% correct on general decisions against 75.1\% of choice and 84.3\%
of yes/no questions.

\textbf{Held-out and outside sets.} On the held-out pool (8,598 items outside the final mix)
reasoning adds 0.6 points at the 4B after the data rounds and the reader round (90.02 to 90.64). On
CITY-Jev (2,000 agent-workflow decisions, strict score = the worst of six input versions, and mean)
the released 4B scores 64.95 and 72.95 and the 27B after the rounds 79.60 and 83.24 (own runs of
2026-10-05 and 10-06), against 74.52 and 78.92 on the card of Jev 1.13.0. The data rounds, which add
12 and 9 index points at 4B and 9B, do not move it ($-$1.0 and $-$0.9 strict, $-$0.2 and $-$0.3
mean). \todo[TODO(city\_rel27d)]{CITY-Jev run of the released 27B, overlap check against the
training mix}

\textbf{Option order.} A public set of 83,183 safety requests is read in the original order,
reversed (keys and order swapped) and with an order-only control. In our runs of 2026-10-07 reversal
changes 1 to 5 of the 450 XSTest answers at every size, as for the hosted reference (5 of 450),
where the least stable of four open models tested by the authors changes 150. On 4,570 index items
the top answer of the released 4B and 9B changes with the order for 15.1\% and 11.7\% of the items
at unchanged accuracy, against 37.4\% for the 4B starting model. Order sensitivity falls with size
and training but is not zero.

\subsection{Calibration of the one-pass outputs}\label{sec:E.4}

Probabilities are taken as the model returns them, after the per-type temperature of the checkpoint
and with no fitting on the evaluation set (Table~\ref{tab:E.3}).

\begin{table}[!htbp]
\renewcommand{\thetable}{E.3}
\centering
\caption{On the hard public items the 27B has the lowest Brier score of the listed systems and the 35B-A3B the lowest calibration error. Calibration of one-pass answers, released weights, own runs (2026-09-27 to 2026-10-04), lower is better. JevBench hard: Brier score / top-label calibration error in 10 bins on 111 items. Pilot: expected Brier score / error on 96 questions whose correct answer is a known distribution. Typed Decisions: KL / Brier score against soft labels. CJ-Bench: error in 15 bins, general domain. Reference rows: bundle README, dataset card and benchmark authors.}\label{tab:E.3}
{\small\setlength{\tabcolsep}{6pt}\renewcommand{\arraystretch}{1.1}
\noindent\begin{adjustbox}{max width=\linewidth}
\begin{tabular}{lrrrr}
\toprule
\textbf{model} & {\begin{tabular}[b]{@{}r@{}}\textbf{JevBench}\\\textbf{hard: Brier}\\\textbf{/ error}\end{tabular}} & {\begin{tabular}[b]{@{}r@{}}\textbf{pilot:}\\\textbf{expected}\\\textbf{Brier / error}\end{tabular}} & {\begin{tabular}[b]{@{}r@{}}\textbf{Typed}\\\textbf{Decisions:}\\\textbf{KL / Brier}\end{tabular}} & {\begin{tabular}[b]{@{}r@{}}\textbf{CJ-Bench}\\\textbf{general:}\\\textbf{error}\end{tabular}} \\
\midrule
\mdourrow StartLux-Decision-0.8B & 0.524 / 0.124 & 0.519 / 0.051 & 0.148 / 0.079 & 0.074 \\
\mdourrow StartLux-Decision-2B & 0.394 / 0.081 & 0.515 / 0.060 & 0.102 / 0.055 & 0.031 \\
\mdourrow StartLux-Decision-4B & 0.375 / 0.104 & 0.499 / 0.059 & 0.080 / 0.044 & 0.060 \\
\mdourrow StartLux-Decision-9B & 0.355 / 0.056 & 0.477 / 0.038 & 0.080 / 0.044 & 0.038 \\
\mdourrow StartLux-Decision-27B & 0.265 / 0.054 & 0.478 / 0.064 & 0.079 / 0.042 & 0.056 \\
\mdourrow StartLux-Decision-35B-A3B & 0.280 / 0.039 & 0.502 / 0.061 & 0.075 / 0.040 & - \\
Jev 1.13 & 0.358 / 0.095 & 0.595 / 0.130 & 1.442 / 0.148 & 0.115 \\
Intern-Decision-4B & 0.347 / 0.065 & 0.550 / 0.089 & - & - \\
JevK5 & 0.366 / 0.047 & - & - & - \\
\bottomrule
\end{tabular}
\end{adjustbox}\par}
\end{table}

On the hard tier the 27B has the lowest Brier score of the listed systems and the 35B-A3B the lowest
calibration error. On the pilot all six sizes have a lower error than both reference systems. The
small sizes are less well calibrated on hard items (0.08 to 0.12 at 0.8B to 4B). On long lists the
reported probability of the chosen option exceeds the accuracy by 0.6 to 2.1 points for 50 to 228
options (3.8 for the 27B at 228). Once a policy selects or routes on the probability, these numbers
are biased on the selected answers (Chapter~\ref{sec:7}).

\subsection{Reused test sets and twin test sets in detail}\label{sec:E.5}

The reused half of DecisionPivot (Section~\ref{sec:6.4}) has 35 tasks from public evaluation data in
seven layers of a decision-making system (Table~\ref{tab:E.4}). The twin test sets
(Section~\ref{sec:6.3}) measure the skill of one index benchmark on a different public data set
(Table~\ref{tab:E.5}).

\begin{table}[!htbp]
\renewcommand{\thetable}{E.4}
\centering
\caption{Decision training transfers to the reused test sets, and the data round does not. Reused test sets, items unseen by our training: chance-corrected score per layer (A before generation, B guards, C after generation, D agent control, E classification with reasoning, F data pipelines, G search and matching) and mean of the layers. Own runs, one pass, 7 October 2026, first scoring pass. The hosted reference was called through its public interface on 6 and 7 October 2026. The mean is for comparing our own checkpoints, not a benchmark score.}\label{tab:E.4}
{\small\setlength{\tabcolsep}{6pt}\renewcommand{\arraystretch}{1.1}
\noindent\begin{adjustbox}{max width=\linewidth}
\begin{tabular}{lrrrrrrrr}
\toprule
\textbf{system} & \textbf{A} & \textbf{B} & \textbf{C} & \textbf{D} & \textbf{E} & \textbf{F} & \textbf{G} & {\begin{tabular}[b]{@{}r@{}}\textbf{mean}\\\textbf{of the}\\\textbf{layers}\end{tabular}} \\
\midrule
\mdourrow StartLux-Decision-27B, released & 39.2 & 79.3 & 58.3 & 74.9 & 49.2 & 26.7 & 74.6 & 57.5 \\
\mdourrow StartLux-Decision-27B, after data rounds & 36.2 & 77.5 & 55.1 & 73.0 & 50.5 & 29.3 & 73.7 & 56.5 \\
Hosted reference & 36.5 & 79.6 & 59.5 & 66.7 & 50.6 & 21.3 & 72.1 & 55.2 \\
\mdourrow StartLux-Decision-9B, released & 34.7 & 72.1 & 49.9 & 71.1 & 44.2 & 29.9 & 69.5 & 53.1 \\
\mdourrow StartLux-Decision-9B, after data rounds & 35.6 & 69.7 & 50.1 & 69.8 & 44.6 & 32.9 & 68.9 & 53.1 \\
Clef 27B & 33.1 & 76.3 & 50.4 & 64.9 & 44.6 & 26.7 & 72.0 & 52.6 \\
\mdourrow StartLux-Decision-4B, after data rounds & 31.5 & 68.1 & 47.6 & 66.2 & 42.9 & 29.5 & 68.3 & 50.6 \\
\mdourrow StartLux-Decision-4B, released & 31.6 & 69.0 & 48.5 & 67.8 & 43.9 & 27.1 & 65.8 & 50.5 \\
9B starting model & 29.5 & 69.3 & 43.5 & 63.2 & 39.9 & 17.1 & 58.9 & 45.9 \\
4B starting model & 27.3 & 65.2 & 36.3 & 55.6 & 37.5 & 3.2 & 61.4 & 40.9 \\
\bottomrule
\end{tabular}
\end{adjustbox}\par}
\end{table}

Decision training transfers: the released 4B and 9B are 9.6 and 7.2 points above their starting
models. The data rounds do not: against the released weights of the same size they change the mean
by $-$1.0 at 27B (interval $-$1.6 to $-$0.4), 0.0 at 9B ($-$0.6 to +0.7) and +0.1 at 4B ($-$0.6 to
+0.7). The released 27B is 2.3 points above the hosted reference (interval +1.2 to +3.3), but
exposure to related material differs between the models. Against Perplexity Decider v1.1 the
released 27B is lower on FOLIO ($-$13.2 points of the chance-corrected score), NevIR ($-$12.8) and
LLMBar ($-$12.0), where that model's training manifest lists the training split, a sibling set or
the source of the task, and higher on jailbreak prompts (+17.3), capability-boundary records (+11.7)
and CUAD clauses (+5.7), where 11.9\%, 21.7\% and 42.3\% of the items were found in our training
files before cleaning. That model was run on inputs of up to 20,000 tokens where its shipped guard
is 8,192.

\begin{table}[!htbp]
\renewcommand{\thetable}{E.5}
\centering
\caption{The twins order our sizes, and the data round leaves every size where it was. Twin test sets by area, one pass (own runs, 7 October 2026, number of tasks in brackets, no intervals). Half blend: the released 27B blended with the final data round at half of the round. Breadth-only round: a 4B round on rows from several hundred other task families, no index-targeted file. None of these checkpoints trained on a family from which a twin is built. Board scores of edition 0.3: data of 2026-10-06.}\label{tab:E.5}
{\footnotesize\setlength{\tabcolsep}{4pt}\renewcommand{\arraystretch}{1.1}
\noindent\begin{adjustbox}{max width=\linewidth}
\begin{tabular}{lrrrrrrr}
\toprule
\textbf{system} & {\begin{tabular}[b]{@{}r@{}}\textbf{knowledge}\\\textbf{(8)}\end{tabular}} & {\begin{tabular}[b]{@{}r@{}}\textbf{language}\\\textbf{(5)}\end{tabular}} & {\begin{tabular}[b]{@{}r@{}}\textbf{retrieval}\\\textbf{(5)}\end{tabular}} & {\begin{tabular}[b]{@{}r@{}}\textbf{tools}\\\textbf{(2)}\end{tabular}} & \textbf{area-weighted} & {\begin{tabular}[b]{@{}r@{}}\textbf{board:}\\\textbf{same}\\\textbf{skills}\end{tabular}} & {\begin{tabular}[b]{@{}r@{}}\textbf{board:}\\\textbf{new}\\\textbf{domains}\end{tabular}} \\
\midrule
\mdourrow StartLux-Decision-27B, released & 74.9 & 61.8 & 66.6 & 83.9 & 71.1 & - & - \\
\mdourrow StartLux-Decision-27B, after data rounds & 74.3 & 61.8 & 67.2 & 84.9 & 71.3 & - & - \\
\mdourrow StartLux-Decision-27B, half blend & 75.2 & 61.8 & 68.5 & 85.1 & 71.9 & - & - \\
\mdourrow StartLux-Decision-9B, released & - & - & - & - & 66.4 & - & - \\
\mdourrow StartLux-Decision-9B, after data rounds & - & - & - & - & 66.9 & - & - \\
9B starting model & - & - & - & - & 57.0 & - & - \\
\mdourrow StartLux-Decision-4B, released & 62.4 & 53.0 & 63.1 & 79.3 & 63.3 & - & - \\
\mdourrow StartLux-Decision-4B, after data rounds & - & - & - & - & 62.9 & - & - \\
\mdourrow StartLux-Decision-4B, breadth-only round & 64.2 & 51.8 & 67.0 & 77.5 & 64.0 & - & - \\
4B starting model & - & - & - & - & 49.2 & - & - \\
Perplexity Decider v1.1 & 84.8 & 60.3 & 72.0 & 84.4 & 74.8 & 61.1 & 55.6 \\
Kev 27B & 76.1 & 61.6 & 69.1 & 83.0 & 71.8 & 55.5 & 55.5 \\
JEV-27B & 70.1 & 66.9 & 66.6 & 80.5 & 70.5 & 54.2 & 50.8 \\
Clef 27B & 65.1 & 54.6 & 72.5 & 78.2 & 66.4 & 53.1 & 41.9 \\
Clef-flash & 59.7 & 52.9 & 69.4 & 79.6 & 64.0 & 44.0 & 42.5 \\
\bottomrule
\end{tabular}
\end{adjustbox}\par}
\end{table}

The 20 twin tasks have 16,370 items, none from a source of our training files, and there is no twin
for the arts area or for select-all questions. The data rounds leave the twins where they were at
every size, while decision training transfers (the released 4B and 9B are 14.1 and 9.4 points above
their starting models). The breadth-only round lowers the stance and sarcasm twins (36.9 against
44.9 and 32.6 against 39.2 for the released 4B). No interval has been computed for these
differences. \todo{paired intervals between our checkpoints on the twin test sets}

The five reference models come in the same order on the twins as on the board's same-skill part.
Much of the lead of Perplexity Decider v1.1 sits on twins whose training split or a sibling set is
in its training list: on Corr2Cause it scores 96.1 against 46 to 49 for our checkpoints and on
ProofWriter at depth 5 90.0 against 65 to 67. Where it has no such exposure it is level or behind
(FiQA sentiment 43.1 against 60 to 64).

\subsection{Serving settings that changed results}\label{sec:E.6}

The read-out is deterministic, so two paths that serve the same weights must agree, and they did not
always. With prefix caching on, a third-party inference server returned different read-outs for the
same rows, and with its default chunked prefill every reasoning run of ours until 6 October
under-scored tool benchmarks, which we first read as ``reasoning pays in knowledge and costs in tool
selection''.

\begin{table}[!htbp]
\renewcommand{\thetable}{E.6}
\centering
\caption{Two server settings changed answers without an error message, and one of them cost 1.4 index points. Settings that changed results. Rows 1 to 4 concern the generation server for reasoning runs (vLLM 0.19.1). The batch runner of the released package is the reference.}\label{tab:E.6}
{\footnotesize\setlength{\tabcolsep}{5pt}\renewcommand{\arraystretch}{1.1}
\noindent\begin{adjustbox}{max width=\linewidth}
\begin{tabular}{>{\raggedright\arraybackslash}p{\mdw{0.1943}}>{\raggedright\arraybackslash}p{\mdw{0.2414}}>{\raggedright\arraybackslash}p{\mdw{0.3780}}>{\raggedright\arraybackslash}p{\mdw{0.1725}}}
\toprule
\textbf{setting} & \textbf{what went wrong} & \textbf{size of the error} & \textbf{fix} \\
\midrule
1. Prefix caching on (experimental for this architecture) & Read-outs of the same rows differ & 2.6\% of the read-outs moved by more than 0.05, 16\% of the answers on lists over 26 options flipped & Caching off everywhere \\
2. Prefill in chunks of 8,192 batched tokens (the default) & A prompt whose prefill is split between two scheduler steps is read wrongly (groups of a long list, questions of one request sent at once) & 4B after data rounds, one pass, server against batch runner: same choice in 96.0\% on a 53-tool selection benchmark (accuracy 82.8 against 85.2), 93.9\% on chords with 129 labels (76.4 against 80.3), 98.4\% on a multi-question simulator. Index with reasoning 65.01 instead of 66.38 & Prefill in one piece (65,536 batched tokens): 99.4\%, 99.3\%, 100.0\% \\
3. Checkpoint sampling defaults (top-k 20, top-p 0.95) applied to the read-out & The letter distribution is truncated & not measured & Neutral settings, processed log-probabilities of 26 tokens \\
4. New reasoning requests join a running decode batch & Thoughts degrade into loops & 43--50 of 183 thoughts, 0 of 183 when all are sent at once & Reasoning requests go out in waves per server \\
5. FP8 with padded batches & A zero padding row gets a zero scale, gives NaN and leaks into real rows & Agreement with bf16 falls to about 52\% & One question per forward pass, no padding \\
6. Thought budget of 1,024 tokens on a 4B & 15--72\% of the thoughts on reasoning benchmarks are cut & Accuracy 39\% at the limit against 89\% for finished thoughts (code execution) & 4,096 tokens \\
7. A run with unanswered requests scored as complete & Unanswered requests count as wrong & 61.31 at coverage 0.960, 66.36 once the missing 5,606 requests were answered & Coverage of at least 0.999, retry passes \\
\bottomrule
\end{tabular}
\end{adjustbox}\par}
\end{table}

Row 2 hardly touches single questions (the batch runner and the server agree on 97.8 to 99.9\% of
ordinary questions whatever their length). The damage sits in requests that put several long prompts
with a common beginning into the server at once, where long lists in requests of 2,000 to 8,192
tokens agree in only 84 to 90\%. On the corrected servers the tools area is at its one-pass level
(86.1 against 86.0) and no benchmark loses more than 1.4 points to reasoning.

Two lessons generalise. Compare a serving path with a batch runner on the longest lists and on
multi-question requests, not on an average benchmark, and distrust a loss that appears where the
model does the least reasoning. Separately, a run enters a table only with a coverage of at least
0.999 (row 7), so requests that failed are sent again in up to three passes.

\subsection{Index values with the rebuilt GSM8K rows}\label{sec:E.7}

GSM8K is one of the ten benchmarks of the knowledge area, and the five areas weigh equally, so a
change of one skill point on GSM8K moves the index by 0.02 points. We ran every checkpoint on the
old rows of edition 0.2.1 and on the rows rebuilt for edition 0.3 (the same 1,319 problems with
wrong options taken from the answers of other problems, built with the maintainers' own script) and
replaced the GSM8K term of the index.

\begin{table}[!htbp]
\renewcommand{\thetable}{E.7}
\centering
\caption{The old rows lift every trained checkpoint by 0.7 to 1.8 index points and leave the order of our checkpoints unchanged. GSM8K skill in percent, chance-corrected per track and averaged over the ten-option and four-option tracks, one pass (own runs, 8 October 2026). Index: Decision Index 0.2.1 as reported in this report and with the rebuilt rows in place of the old ones. The starting models have no index run of their own in one pass, and the -Rounds checkpoints of 0.8B and 2B were not run.}\label{tab:E.7}
{\small\setlength{\tabcolsep}{6pt}\renewcommand{\arraystretch}{1.1}
\noindent\begin{adjustbox}{max width=\linewidth}
\begin{tabular}{lrrrr}
\toprule
\textbf{checkpoint} & {\begin{tabular}[b]{@{}r@{}}\textbf{skill, old rows}\\\textbf{(10 / 4 options)}\end{tabular}} & {\begin{tabular}[b]{@{}r@{}}\textbf{skill, rebuilt}\\\textbf{rows (10 / 4}\\\textbf{options)}\end{tabular}} & {\begin{tabular}[b]{@{}r@{}}\textbf{index}\\\textbf{0.2.1}\end{tabular}} & {\begin{tabular}[b]{@{}r@{}}\textbf{with rebuilt}\\\textbf{rows}\end{tabular}} \\
\midrule
4B starting model & 17.3 (10.8 / 23.8) & 11.0 (5.2 / 16.8) & -- & change $-$0.13 \\
9B starting model & 37.2 (32.4 / 42.1) & 18.0 (12.6 / 23.4) & -- & change $-$0.38 \\
\mdourrow StartLux-Decision-0.8B & 89.4 (98.0 / 80.9) & 2.0 (1.3 / 2.8) & 38.88 & 37.13 \\
\mdourrow StartLux-Decision-2B & 83.6 (96.1 / 71.0) & 7.1 (3.9 / 10.3) & 44.19 & 42.66 \\
\mdourrow StartLux-Decision-4B & 87.9 (93.8 / 81.9) & 37.2 (27.8 / 46.6) & 52.76 & 51.75 \\
\mdourrow StartLux-Decision-9B & 94.3 (99.5 / 89.1) & 30.8 (17.9 / 43.8) & 58.64 & 57.37 \\
\mdourrow StartLux-Decision-27B & 95.3 (99.0 / 91.7) & 60.5 (51.6 / 69.3) & 63.88 & 63.18 \\
\mdourrow StartLux-Decision-4B-Rounds & 91.8 (97.9 / 85.8) & 23.0 (13.9 / 32.2) & 64.78 & 63.40 \\
\mdourrow StartLux-Decision-9B-Rounds & 94.7 (99.6 / 89.9) & 26.1 (15.1 / 37.1) & 67.75 & 66.38 \\
\mdourrow StartLux-Decision-27B-Rounds & 94.9 (99.1 / 90.7) & 53.7 (42.0 / 65.4) & 70.43 & 69.61 \\
\bottomrule
\end{tabular}
\end{adjustbox}\par}
\end{table}

The released 0.8B and 2B answer the old ten-option rows almost perfectly and the rebuilt ones at
chance, so at these sizes the old score measures the layout and not the arithmetic. The 27B keeps
most of its skill, and the data round costs every size skill on the rebuilt rows, most at 4B (37.2
$\rightarrow$ 23.0). Rounds that remove the old rows and add clean problems in the rebuilt layout
are among the hygiene repairs of Section~\ref{sec:4.7}.
