# Supplementary material for: StartLux-Decision: AutoThink Decision Models with Reinforcement Learning for Calibrated Deliberative Decisions
Source: arXiv:2610.17309 source file (2026-10-20)
Supplement: Supplementary file 11 [file appendix_E_value_gate.tex]

\clearpage
\section{The value gate: details}\label{sec:E}

This appendix holds the details behind Section~\ref{sec:7.6}: why a gate that asks for the value of
reasoning follows from the objective of a gated system, how its labels are built and how it is
trained, what it does at three model sizes, the certificates per route, the route effect under it,
its use as the escalation rule of a cascade, the comparison with a difficulty question, and an
experiment on which training items set the confidence after reasoning.

\textbf{Status.} The value gate is a research result. It was evaluated on the diagnostic decisions
only. The index runs of this report route with the rule on the top probability, and an index run
with the learned gate is future work. \todo{say whether a checkpoint that answers the value question
is released; v4 says only that the gate was trained from the released 4B (part3b.md:651-654) and
that an index run with it is future work (part3b.md:810-811).}

\subsection{The gate as the solution of a policy-level objective}\label{sec:E.1}

The route effect of Section~\ref{sec:7.3} exists because the gate routes on a score that still knows
something about the answer the system reports. A gate can ask another question: is reasoning worth
its cost on this item? We trained that question as a typed yes/no question of the same model. Its
labels are exact, not estimated: for every training item both readouts exist, so the gain in the
probability of the correct option that reasoning brings is known, and the question takes a cost
level as input. It is read in the same pass as the fast answer.

Reinforcement learning from calibrated decisions rewards a proper score of each decision. A system
that reasons only sometimes is scored on what it reports: with probability g(x) the thought
distribution p1, at a cost c, and otherwise the fast distribution p0. For a proper score S its
objective is

J = E{[} (1 $-$ g(x)) \textperiodcentered{} S(p0(x), y) + g(x) \textperiodcentered{} (S(p1(x,
$\tau$), y) $-$ c($\tau$)) {]}.

Three facts follow (Proposition 5, A.6). First, J is linear in the gate, and its derivative at an
item is the value of computation, v(x) = E{[}S(p1, y) $-$ c \textbar{} x{]} $-$ E{[}S(p0, y)
\textbar{} x{]}. The optimal gate reasons exactly where v is positive. Both terms can be computed
for every training item, so the gate is learned from exact labels, without sampling its own
decisions. Our training target is the share of the positive part of v, which makes the threshold one
half optimal at every cost level. Second, the best confidence for the thought answer is the
posterior on the items the gate routes, not on all items: the population on which
Sections~\ref{sec:7.4} and \ref{sec:7.5} certify and calibrate. Third, only the reasoning itself has
a sampled gradient. For that third part our experiments with reinforcement learning give a mixed
answer (Section~\ref{sec:5.9}). No arm has made the answers more accurate than those of the
supervised stages: the one arm that gained over its own starting model (+1.95 points after the
thought) did so by learning where to skip the thought, and is level with the supervised sequence.
What a policy gradient with a bounded proper score does change, started from a model that reasons
and with rollouts sampled as at inference, is the end of the thought and the calibration of the
answer after it: 99.7\% (4B) and 99.8\% (9B) of the thoughts end, and before any temperature is
fitted the calibration error of that answer is 32\% and 43\% lower, at an accuracy within a third of
a point of the start on held-out items and without a better ranking of right and wrong answers. The
first two parts carry the gains of this appendix. In this sense the gate and the policy-aware map
are the solution of calibrated-decision training at the level of the system, obtained without
reinforcement learning where the objective allows it.

\subsection{Labels and training}\label{sec:E.2}

\textbf{Rollouts.} For a training item the released 4B's fast distribution p0 was read once, and K =
4 reasoning samples were drawn from the base model it was tuned from (budget 4,096 tokens,
temperature 0.6). The decision model read each sample, which gives a thought distribution p1,k and a
token count Tk. The thought distributions pass through one temperature per question type (1.6 for
choice, 1.0 for yes/no and 0.8 for score questions, fitted on earlier rollouts of the same kind).
The labels thus come from a two-model system. In Table~\ref{tab:E.1} the gate routes systems in
which each model reads its own reasoning, so its use there is a transfer across writers as well as
across sizes.

\textbf{Label.} With the negative Brier score S and the item's target t, the value of sample k at
cost $\lambda$ per token is dk = S(p1,k, t) $-$ S(p0, t) $-$ $\lambda$\textperiodcentered{}Tk. Let A
be the mean of the positive parts of the dk and B the mean of the negative parts. The gate's target
is P(yes) = A / (A + B) and the row's weight is A + B divided by its mean over the rows. Under the
weighted log loss the fitted probability exceeds one half exactly where the expected value of
reasoning is positive, so one threshold serves every cost level, and items on which reasoning
changes little weigh little.

\textbf{Question.} The item's own instructions and options, followed by: ``Before answering: would
careful step-by-step reasoning improve the decision on this question enough to be worth its cost?
Reasoning cost: \ldots{}'', with the level in a word: free, cheap, moderate, expensive for $\lambda$
= 0, 1\textperiodcentered{}10\textsuperscript{$-$5}, 3\textperiodcentered{}10\textsuperscript{$-$5}
and 1\textperiodcentered{}10\textsuperscript{$-$4} per reasoning token. It is a yes/no question of
the ordinary kind and is read at the same position as the item's answer.

\textbf{Round.} Each item enters once per cost level. Each item also enters once as its original
question with the model's own p0 as a soft target, so that the round does not move the fast answer.
The gate of Tables~\ref{tab:E.1} and \ref{tab:E.2} was trained on 44,434 training items of the first
training file and the early data rounds (217,424 rows after de-duplication, with a mean target of
0.46), one epoch of 1,181 steps at 184 rows per step, starting from the released 4B. The diagnostic
decisions on which it is evaluated are benchmark items and are not among them.

\subsection{Policies at three sizes}\label{sec:E.3}

At an equal think rate, the thought answers on the items the value gate routes are 75\% accurate
where those routed by uncertainty are 30\% accurate, and they become certifiable (E.4). A gate
trained on the 4B's labels transfers to the 27B.

\begin{table}[!htbp]
\renewcommand{\thetable}{E.1}
\centering
\caption{Policies on the diagnostic decisions (5,710 items for the 4B and 9B, 1,428 for the 27B). Every model reads its own reasoning. The gate is the one trained on the 4B's labels at all three sizes. Thought distributions are taken after one temperature. ``Confidence, same rate'' routes the least confident answers at the think rate of the value gate in the row above. Overconfidence is mean confidence minus accuracy. Own runs.}\label{tab:E.1}
{\small\setlength{\tabcolsep}{6pt}\renewcommand{\arraystretch}{1.1}
\noindent\begin{adjustbox}{max width=\linewidth}
\begin{tabular}{llrrrrrr}
\toprule
\textbf{model} & \textbf{policy} & {\begin{tabular}[b]{@{}r@{}}\textbf{think}\\\textbf{rate}\end{tabular}} & {\begin{tabular}[b]{@{}r@{}}\textbf{reasoning}\\\textbf{tokens}\\\textbf{per item}\end{tabular}} & \textbf{accuracy} & {\begin{tabular}[b]{@{}r@{}}\textbf{log}\\\textbf{score}\end{tabular}} & {\begin{tabular}[b]{@{}r@{}}\textbf{thought}\\\textbf{answers:}\\\textbf{accuracy}\end{tabular}} & {\begin{tabular}[b]{@{}r@{}}\textbf{thought}\\\textbf{answers:}\\\textbf{overconfidence}\end{tabular}} \\
\midrule
4B & never & 0 & 0 & 70.61 & $-$.754 & -- & -- \\
4B & always & 100\% & 624 & 73.46 & $-$.709 & 73.5 & +.035 \\
4B & plain confidence below 0.7 & 50.1\% & 464 & 73.26 & $-$.721 & 54.8 & +.062 \\
4B & value gate, moderate cost & 45.0\% & 349 & 73.43 & $-$.715 & 69.9 & +.048 \\
4B & confidence, same rate & 45.0\% & 436 & 73.08 & $-$.724 & 52.0 & +.070 \\
4B & value gate, expensive cost & 15.9\% & 128 & 72.80 & $-$.712 & 75.2 & +.021 \\
4B & confidence, same rate & 15.9\% & 231 & 71.54 & $-$.738 & 29.8 & +.130 \\
9B & never & 0 & 0 & 72.71 & $-$.706 & -- & -- \\
9B & always & 100\% & 2,934 & 74.01 & $-$.733 & 74.0 & +.054 \\
9B & plain confidence below 0.7 & 46.6\% & 1,422 & 73.91 & $-$.733 & 51.3 & +.095 \\
9B & value gate, moderate cost & 45.0\% & 1,235 & 73.70 & $-$.712 & 70.1 & +.064 \\
9B & confidence, same rate & 45.0\% & 1,376 & 73.90 & $-$.733 & 50.5 & +.097 \\
9B & value gate, expensive cost & 15.9\% & 408 & 73.72 & $-$.696 & 73.1 & +.049 \\
9B & confidence, same rate & 15.9\% & 558 & 73.52 & $-$.728 & 29.1 & +.159 \\
27B & never & 0 & 0 & 76.89 & $-$.648 & -- & -- \\
27B & always & 100\% & 540 & 79.27 & $-$.636 & 79.3 & +.046 \\
27B & plain confidence below 0.7 & 29.8\% & 327 & 78.85 & $-$.658 & 51.2 & +.111 \\
27B & value gate, moderate cost & 44.5\% & 299 & 78.61 & $-$.614 & 80.7 & +.021 \\
27B & confidence, same rate & 44.5\% & 400 & 79.06 & $-$.650 & 59.7 & +.088 \\
27B & value gate, expensive cost & 16.3\% & 90 & 78.26 & $-$.618 & 82.2 & +.033 \\
27B & confidence, same rate & 16.3\% & 217 & 77.87 & $-$.672 & 43.8 & +.127 \\
\bottomrule
\end{tabular}
\end{adjustbox}\par}
\end{table}

What the gate buys is not the accuracy of the whole system at a middling think rate: at 45\% it is
within half a point of routing by confidence at all three sizes (+0.35, $-$0.20, $-$0.45). It buys
three other things.

\begin{itemize}
\item \emph{Shorter reasoning at the same think rate} (349 against 436 tokens per item at 4B, 299 against
400 at 27B): its labels charge for tokens.
\item \emph{A better log score of the system in every pair} (by .009 to .054), because the thought answers
it reports are right far more often (70 to 82\% against 29 to 60\%) and less overconfident.
\item \emph{Accuracy at a low think rate,} where a budget forces a choice: it is ahead at 4B (+1.26 points
at a sixteen per cent think rate) and level at 9B and 27B (+0.20, +0.39), with 55\%, 73\% and 41\%
of the tokens.
\end{itemize}

A gate trained on the 9B's own labels routes 38.8\% and 14.7\% of the 9B's items and reaches 73.89
and 74.02, no clear difference from the 4B's gate. The 27B was run with the 4B's gate only.

\subsection{Certificates per route}\label{sec:E.4}

On the 4B (20 splits of the 5,710 items, target error 10\%, calibration per route as in
Section~\ref{sec:7.4}) the thought answers of the value gate at the expensive level are accepted at
a rate of 192 per split with 5.5\% error and no violation. Under the rule ``plain confidence below
0.7'' and under the confidence gate at the same think rate, no thought answer is accepted per route
in any split: the routed answers are too often wrong for a threshold to exist. With one threshold
for all answers, thought answers are accepted at 16.7\% error for the uncertainty rule (violations
in every split), 11.3\% for the confidence gate and 10.3\% for the value gate (violations in 70\%
and 65\% of the splits). The single threshold fails for every gate, as in Appendix~\ref{sec:D.4},
and fails least where the route effect is smallest. At a target of 5\% no gate has certified thought
answers. On the 27B the diagnostic set is too small for a per-route certificate of the thought
answers at a sixteen per cent think rate (about 115 routed items per calibration half). With one
threshold the value gate's accepted thought answers have 3.2 to 7.8\% error and those of the two
confidence rules 7.8 to 45.8\%.

\subsection{The route effect under the value gate}\label{sec:E.5}

In the terms of Appendix~\ref{sec:C}: at one and the same think rate, routing on the plain
confidence leaves a residual AUROC of .69 (4B) and .71 (9B) and a matched difference of $-$.23 to
$-$.27. The score of the value gate has a residual AUROC of .48--.51 (4B) and .53--.58 (9B): it says
where thinking pays, not where the thought answer will be wrong. The matched difference shrinks to
$-$.05 \ldots{} +.07 (4B, and $-$.02 at the moderate cost level, a 45\% think rate) and $-$.11
\ldots{} +.01 (9B), and the thought answers on routed items are 71\% accurate instead of 53\% (4B,
45\%). The rollouts of Table~\ref{tab:E.2} use a separate reasoner read by the decision model, a
two-model control.

\begin{table}[!htbp]
\renewcommand{\thetable}{E.2}
\centering
\caption{Routing by value against routing by confidence at the same think rate (two-model control: a separate reasoner read by the decision model, 4,997 items for the 4B reader, 5,710 for the 9B). ``Matched'' is the accuracy of the reported answer at matched reported confidence, routed minus kept. The residual AUROC is that of the routing score for the correctness of the thought answer given the thought confidence (0.5 = the score knows nothing more). Own runs.}\label{tab:E.2}
{\small\setlength{\tabcolsep}{6pt}\renewcommand{\arraystretch}{1.1}
\noindent\begin{adjustbox}{max width=\linewidth}
\begin{tabular}{llrrrrr}
\toprule
\textbf{reader} & \textbf{routing} & {\begin{tabular}[b]{@{}r@{}}\textbf{think}\\\textbf{rate}\end{tabular}} & {\begin{tabular}[b]{@{}r@{}}\textbf{thought}\\\textbf{answers right:}\\\textbf{routed / kept}\end{tabular}} & {\begin{tabular}[b]{@{}r@{}}\textbf{system}\\\textbf{accuracy}\end{tabular}} & \textbf{matched} & {\begin{tabular}[b]{@{}r@{}}\textbf{residual}\\\textbf{AUROC}\end{tabular}} \\
\midrule
4B & value gate, free & 66\% & 69.3 / 80.6 & 73.62 & $-$.052 & .478 \\
4B & confidence, same rate & 66\% & 61.9 / 95.1 & 73.28 & $-$.252 & .692 \\
4B & value gate, cheap & 56\% & 71.0 / 75.9 & 73.90 & $-$.034 & .486 \\
4B & confidence, same rate & 56\% & 58.0 / 92.4 & 73.44 & $-$.265 & .692 \\
4B & value gate, moderate & 45\% & 71.4 / 74.6 & 73.92 & $-$.021 & .494 \\
4B & confidence, same rate & 44\% & 53.0 / 89.3 & 73.16 & $-$.273 & .692 \\
4B & value gate, expensive & 16\% & 78.7 / 72.1 & 72.98 & +.069 & .513 \\
4B & confidence, same rate & 15\% & 37.6 / 79.6 & 71.80 & $-$.249 & .692 \\
9B & value gate, free & 71\% & 70.1 / 85.2 & 74.76 & $-$.105 & .533 \\
9B & confidence, same rate & 71\% & 65.2 / 97.3 & 74.85 & $-$.240 & .712 \\
9B & value gate, cheap & 60\% & 68.9 / 83.0 & 75.06 & $-$.108 & .550 \\
9B & confidence, same rate & 60\% & 61.2 / 94.7 & 75.27 & $-$.248 & .712 \\
9B & value gate, moderate & 46\% & 68.0 / 80.2 & 75.31 & $-$.088 & .563 \\
9B & confidence, same rate & 46\% & 55.9 / 90.6 & 75.64 & $-$.251 & .712 \\
9B & value gate, expensive & 18\% & 72.4 / 75.0 & 75.17 & +.007 & .583 \\
9B & confidence, same rate & 18\% & 39.7 / 82.0 & 73.91 & $-$.225 & .712 \\
\bottomrule
\end{tabular}
\end{adjustbox}\par}
\end{table}

The confidence rule sends the items on which the thought answer will be wrong and keeps those on
which it would have been right (95\% at the free level): its score predicts the thought answer's
correctness beyond what the thought confidence says. The value gate's score does not (residual AUROC
.48 to .51 at 4B), and the accuracy of the thought answer is then nearly the same on both sides of
the gate. The 9B gate of this table, the first one trained on the 9B's labels, keeps a little of the
confidence (.53 to .58), and the matched difference with it.

\begin{figure}[!htbp]
\renewcommand{\thefigure}{E.1}
\centering
\adjincludegraphics[max width=\linewidth,max height=0.5\textheight]{figures/fig1_reliability.pdf}
\caption{Reliability of the reported answer by route, one model at three sizes on the decision suite: plain answers of items that are not routed, thought answers of items routed by uncertainty, and thought answers of items routed by the value-of-computation gate. Ten equal-width confidence bins (bins with at least 30 items), 95\% Wilson intervals. \todo{the caption of v4 Figure 2 (part1.md:100) does not give the routing threshold or the cost level of the gate; the figure script uses ``plain confidence below 0.7'' and the expensive level. Add them after confirming that the figure was not regenerated since 4 October.}}\label{fig:E.1}
\end{figure}

\subsection{As the escalation rule of a cascade}\label{sec:E.6}

The same score can decide which items a small model hands to a larger one. Table~\ref{tab:E.3} gives
the gain in accuracy from escalation when the items are chosen by the small model's uncertainty and
when they are chosen by the value gate.

\begin{table}[!htbp]
\renewcommand{\thetable}{E.3}
\centering
\caption{Gain in accuracy from escalation (points) with 16\% of the items escalated, for routing by the small model's uncertainty and by the value gate. The gate's score comes from the 4B in all rows. Own runs.}\label{tab:E.3}
{\small\setlength{\tabcolsep}{6pt}\renewcommand{\arraystretch}{1.1}
\noindent\begin{adjustbox}{max width=\linewidth}
\begin{tabular}{lrr}
\toprule
{\begin{tabular}[b]{@{}l@{}}\textbf{small}\\\textbf{$\rightarrow$ large}\end{tabular}} & {\begin{tabular}[b]{@{}r@{}}\textbf{by the small}\\\textbf{model's}\\\textbf{uncertainty}\end{tabular}} & {\begin{tabular}[b]{@{}r@{}}\textbf{by the}\\\textbf{value}\\\textbf{gate}\end{tabular}} \\
\midrule
0.8B $\rightarrow$ 27B & +11.5 & +19.2 \\
2B $\rightarrow$ 27B & +10.7 & +20.8 \\
0.8B $\rightarrow$ 9B & +6.6 & +13.2 \\
0.8B $\rightarrow$ 4B & +4.5 & +7.3 \\
4B $\rightarrow$ 27B & +11.4 & +12.0 \\
9B $\rightarrow$ 27B & +5.2 & +6.0 \\
4B $\rightarrow$ 9B & +6.4 & +5.9 \\
\bottomrule
\end{tabular}
\end{adjustbox}\par}
\end{table}

The 27B is right on 73\% of the items the gate sends and on 31 to 39\% of those a small model's
uncertainty sends, and overconfident by 5 points instead of 13 to 25. The gain is 1.6 to 2.0 times
larger when the first stage is the 0.8B or the 2B, and about equal when it is the 4B or the 9B,
whose uncertainty already finds the items a larger model can repair. We have not trained the gate
question at the smaller sizes, which a deployed first stage of that size would need. \todo{the
factor is ``1.6 to 2.0 times'' in v4 Appendix E.5 (part3b.md:749-750) and ``1.7 to 1.9 times'' in v4
\S{}6 (part2.md:531-532); keep one.}

\subsection{Difficulty against value}\label{sec:E.7}

A public system (TypeLLM, \texttt{\textquotedbl{}thinking\textquotedbl{}:
\textquotedbl{}auto\textquotedbl{}}, 1--2 October 2026) routes with a typed question of the same
form as ours and another content: the model is asked, without thinking, how much step-by-step
reasoning the question needs (none, low, medium or high), and the level sets the reasoning budget.
We re-implemented its prompt format and protocol and replayed both questions on the same answers.

\textbf{Protocol.} The public system's question was rendered in its documented prompt format and
answered without reasoning by the model under test. The level sets the budget (512, 2,048 and 4,096
tokens for low, medium and high in our replication). 5,682 of the 5,710 diagnostic items were used
(28 have more options than that format admits or returned no parsable level). Every rule was
replayed on the same recorded answers, one reasoning sample per item, so that two rules differ only
in which items they send.

\textbf{On its own ground the two questions are level.} For an untrained base model, always thinking
raises accuracy from 58.7 to 72.6 (4B) and from 63.3 to 73.9 (9B). The difficulty rule reaches 69.50
/ 71.45 at 681 / 647 reasoning tokens per item. Our gate, trained for another reader and used here
only as a router, reaches 68.59 / 71.91 at 762 / 722 (differences $-$0.92 {[}$-$1.78, $-$0.09{]} and
+0.46 {[}$-$0.26, +1.16{]}). When nearly every item gains from reasoning, any question that says
``think'' does well. On the untrained 4B base the levels are informative: 21\% of the items are
``none'' (reasoning adds 3.2 points), 55\% ``low'' (+15.3), 23\% ``medium'' (+20.5), and the rule
reasons on 78.8\% of the items for 69.50\% accuracy at 681 tokens per item, against 72.60\% for
always reasoning with the largest budget at 2,527 tokens.

\textbf{On a trained decision model the content of the question matters.} There thinking improves
5.6\% / 3.0\% of the answers and damages 3.2\% / 1.4\%. With the top 20\% of the items sent to
thinking, the value gate is +1.23 {[}+0.76, +1.71{]} (4B) and +0.76 {[}+0.42, +1.11{]} (9B) points
above the difficulty question answered by the base model, and +1.72 {[}+1.21, +2.24{]} and +1.07
{[}+0.70, +1.46{]} above the difficulty question answered by the trained decision model itself. With
40\% the differences are +0.97 to +0.99 and +0.49 to +0.79. The gap is +0.4 to +0.5 at 60\% and
closes by 80\%. With 10\% of the items the gate takes 72\% of everything thinking can give on the
4B, the difficulty question 34\%, the plain confidence 32\%. As shipped, the rule ``difficulty above
none'' thinks about 77--91\% of the items for the accuracy the gate reaches with 45\% (reasoning
tokens $-$36\% on the 4B, $-$44\% on the 9B).

On the trained 4B the levels given by the base model carry gains of +0.6, +2.2 and +4.5 points: the
order is still right, the amounts are small, and a rule that reasons on everything above ``none''
spends 539 tokens per item for 74.15\%, the accuracy the value gate reaches with 346. The trained
4B's own ``none'' items are right 87\% of the time and gain +0.2 from thinking, its ``medium'' items
gain +3.3, its ``high'' items +0.6: the question orders items by how hard they look, and thinking
pays where the plain answer is wrong for a reason that reasoning can remove.

Cut to the same think rate on the trained 4B, the value gate is ahead of the difficulty question by
+1.23 {[}+0.76, +1.71{]} points at 20\% and +0.99 {[}+0.48, +1.51{]} at 40\%, and level with it from
60\% on. \todo{``level with it from 60\% on'' (part3b.md:768) against ``the gap is +0.4 to +0.5 at
60\% and closes by 80\%'' (part2.md:560); give the interval at 60\%.}

\textbf{Against the plain confidence the gate is ahead only at the low end.} At the same think rate:
+0.58 {[}+0.09, +1.11{]} at 20\%, $-$0.09 {[}$-$0.51, +0.33{]} at 40\%. On accuracy alone, then, a
confidence rule is a strong baseline for a trained decision model once a third of the items may be
reasoned about. The gate's advantage over it is the one of Tables~\ref{tab:E.1} and \ref{tab:E.2}:
fewer tokens, and thought answers whose confidence can be used.

\textbf{Caveats.} These are diagnostic items (150 per family, of benchmark type, not held-out
families). The gate's cost level was fixed before the run, and the budget ladder of the difficulty
rule is not used on the trained system, which has one budget of 4,096 tokens. \todo{the value gate
at the moderate level reaches 73.43\% with 349 tokens per item in Table E.1 (part3b.md:668) and
``74.15\% \ldots{} with 346'' in this comparison (part3b.md:766); the protocols may differ (5,710
against 5,682 items; Table E.1 reads each model's own reasoning, the comparison replays one recorded
reasoning sample per item). Say so, or give one figure.}

\subsection{Which training items set the confidence after reasoning}\label{sec:E.8}

Proposition 5(b) says that the best confidence for the thought answer is the posterior on the items
the gate routes. This can be tested directly. In the round that teaches a model to read its own
reasoning (the reader round) we chose which training items carry a reasoning trace and kept
everything else fixed: the base model, its traces, and the plain rows that hold the fast path in
place. The 5,710 diagnostic decisions were re-read by each reader with the same traces.

\begin{table}[!htbp]
\renewcommand{\thetable}{E.4}
\centering
\caption{Reader rounds that differ in which training items carry a trace (4B, first base). Thought answers on routed items: accuracy (\%), accuracy at matched confidence routed minus kept, and negative log-likelihood after one temperature. Own runs.}\label{tab:E.4}
{\footnotesize\setlength{\tabcolsep}{6pt}\renewcommand{\arraystretch}{1.1}
\noindent\begin{adjustbox}{max width=\linewidth}
\begin{tabular}{lrrrr}
\toprule
\textbf{training items that carry a trace} & {\begin{tabular}[b]{@{}r@{}}\textbf{trace rows:}\\\textbf{routed +}\\\textbf{kept items}\end{tabular}} & {\begin{tabular}[b]{@{}r@{}}\textbf{thought answers}\\\textbf{on routed items:}\\\textbf{accuracy}\end{tabular}} & {\begin{tabular}[b]{@{}r@{}}\textbf{routed minus}\\\textbf{kept at matched}\\\textbf{confidence}\end{tabular}} & {\begin{tabular}[b]{@{}r@{}}\textbf{negative}\\\textbf{log-likelihood after}\\\textbf{one temperature}\end{tabular}} \\
\midrule
none (the readout is not trained) & 0 & 58.4 & $-$.274 & 1.094 \\
the items the gate keeps & 0 + 25,244 & 58.5 & $-$.212 & 1.083 \\
2\% of all items & 399 + 516 & 58.2 & $-$.144 & 1.064 \\
10\% of all items & 1,987 + 2,506 & 58.0 & $-$.140 & 1.049 \\
the items the gate routes & 19,489 + 0 & 58.8 & $-$.136 & 1.046 \\
all items (the default round) & 19,489 + 25,244 & 58.8 & $-$.141 & 1.044 \\
the items the gate routes, two traces each & 38,978 + 0 & 58.2 & $-$.193 & 1.062 \\
\bottomrule
\end{tabular}
\end{adjustbox}\par}
\end{table}

\textbf{The confidence on the route is set by the presence of routed items in the round, not by the
amount of data.} With traces for the routed items alone, the thought answers on routed items are
where the full round puts them. With traces for the kept items alone they stay near the untrained
readout, and the difference from the full round is far outside the bootstrap interval ($-$.071
{[}$-$.083, $-$.059{]}). Four hundred routed items, with five hundred kept ones, already bring the
difference at matched confidence to the level of the full round. Twenty-five thousand kept items
alone do not. The accuracy of the thought answer is within 0.8 points in every row. The round trains
the confidence, not the answer.

\begin{table}[!htbp]
\renewcommand{\thetable}{E.5}
\centering
\caption{The same four rounds on other bases: accuracy at matched confidence, routed minus kept. Own runs.}\label{tab:E.5}
{\small\setlength{\tabcolsep}{6pt}\renewcommand{\arraystretch}{1.1}
\noindent\begin{adjustbox}{max width=\linewidth}
\begin{tabular}{lrrrr}
\toprule
\textbf{base} & {\begin{tabular}[b]{@{}r@{}}\textbf{no}\\\textbf{traces}\end{tabular}} & {\begin{tabular}[b]{@{}r@{}}\textbf{kept}\\\textbf{items}\end{tabular}} & {\begin{tabular}[b]{@{}r@{}}\textbf{routed}\\\textbf{items}\end{tabular}} & {\begin{tabular}[b]{@{}r@{}}\textbf{all}\\\textbf{items}\end{tabular}} \\
\midrule
4B, first base & $-$.274 & $-$.212 & $-$.136 & $-$.141 \\
4B, second base & $-$.247 & $-$.223 & $-$.162 & $-$.159 \\
4B, final recipe & $-$.260 & -- & $-$.141 & $-$.141 \\
9B, first base & $-$.196 & $-$.224 & $-$.157 & $-$.190 \\
9B, second base & $-$.230 & -- & $-$.192 & $-$.208 \\
\bottomrule
\end{tabular}
\end{adjustbox}\par}
\end{table}

At 4B the round on the routed items alone equals the default round on all three bases. At 9B it is
ahead of the default round at matched confidence on both bases, by .034 {[}.021, .047{]} and .016
{[}.005, .027{]}, with 2.1 and 1.3 points less raw overconfidence at the same accuracy. In negative
log-likelihood after one temperature it is ahead on the first base (1.121 against 1.137) and behind
on the second (1.202 against 1.186), so the gain is in where the confidence sits on the route, not
in the likelihood. The control on the first 9B base shows why the default round can fall short.
There the traces of the kept items make the readout for the route worse than no training ($-$.224
against $-$.196), the routed items make it better, and the default round is the sum of the two,
which is nearly nothing. Two thirds of that round's traces come from items the gate keeps.

On the full index the two rounds are level on the second 9B base: 68.44 with the routed items alone,
68.39 with all items and 67.53 in one pass (both runs predate the serving correction of
Section~\ref{sec:8.4} and the pair has not been repeated on corrected servers). The first spends
fewer reasoning tokens at inference (378 against 537 per answer, one run each).

\textbf{The round also changes what the model writes.} The comparison above holds the reasoning
fixed: every reader is given the same traces, written before the round. In deployment the model that
has been through the round writes the trace as well, and the two rounds do not leave the same
writer. After the round on routed items the thoughts are shorter at both sizes (9B: 1,312 against
1,870 tokens, 4B: 329 against 388 with the loop detector and 1,098 against 1,240 without). At 9B the
index is the same. At 4B it is not: on corrected servers the round on routed items gives 65.12 and
the default round 66.38 (64.78 in one pass), and an earlier pair without the loop detector, measured
before the correction, shows the same gap (63.65 against 64.65). The loss is in the knowledge area:
the gain on MMLU-Pro falls from 13.8 to 7.9 points, on a graduate-level science set from 8.2 to 1.4,
and code execution turns from +8.4 to $-$5.3, while the tool benchmarks are the same under both
rounds (86.2 and 86.1 points of the area). The readout experiment could not see this, and neither
could the diagnostic items, on which the two readers are level (55.5\% and 55.6\% correct on the
routed items). The saving in traces is therefore established for the confidence of the readout and
for the 9B system. At 4B it costs 1.3 points of the index, and at 27B 1.2: on one base the round on
routed items gives 70.34 and the default round 71.50 (70.08 in one pass), with 87 against 458 tokens
per thought and code execution at +0.3 instead of +20.0 skill points. After the round on routed
items the 27B hardly writes at all. \todo{``At 9B the index is the same'' rests on the pair 68.44 /
68.39, which v4 marks as measured before the serving correction and not repeated (part2.md:494-497,
part2.md:503); repeat it or keep the mark next to this sentence too.}

\textbf{Three consequences for the readout are practical.} The default round is at this optimum only
where the routed items carry enough of it, and for the confidence on the route it is never better
than the round on the routed items alone. Training harder on them does not help: a second trace of
the same item makes the readout worse, as it learns the item instead of the reading. For the
readout, reasoning traces are needed only for the items the gate routes, 44\% of the training items
here, one trace each. Whether the whole system can do without the others depends on the writer (see
the paragraph above). And where traces are expensive a tenth of the items gives the same confidence
at 0.8 points less accuracy on the routed answers.

\textbf{What this training does not remove is the top of the confidence scale.} After the round and
one temperature for the thought path, the mean overconfidence of the two routes differs by 2 to 4
points instead of 12 to 14, on six bases of two sizes. At matched confidence the routed answers are
still less accurate than the kept ones ($-$.14 to $-$.19), and one threshold for all answers still
fails (Appendix~\ref{sec:D.4}). That remainder is what the route-aware map and certification per
route are for.

\subsection{Calibrating the thought path}\label{sec:E.9}

One temperature fitted on 3,700 unseen real-task traces transfers to 32 unseen task families. Every
correction fitted on synthetic data fails (Appendix~\ref{sec:D.8}).
