# Supplementary material for: StartLux-Decision: AutoThink Decision Models with Reinforcement Learning for Calibrated Deliberative Decisions
Source: arXiv:2610.17309 source file (2026-10-20)
Supplement: Supplementary file 12 [file appendix_F_reasoning.tex]

\section{Reasoning stages: extended results}\label{sec:F}

This appendix holds the measurements behind Chapter~\ref{sec:5}: the closing probability per stage,
the thoughts each 4B stage writes, what else we tried against thoughts that do not end, every
reasoning design on the index, the token limit, loop check and gate, the joint variant, and the
calibration of the answer after a thought under reinforcement learning.

\subsection{The closing probability per stage}\label{sec:F.1}

For a stored thought we feed the item's prompt and the thought to a model and read the probability
that the closing tag follows within two tokens (directly, or after a line break). The points are the
natural ends of thoughts that their writer closed. Control points at 25\%, 50\% and 75\% of a
thought, where no model should close, have a median of 0.00 for every model, and every stage of a
size reads the same thoughts (Table~\ref{tab:F.1}).

\begin{table}[!htbp]
\renewcommand{\thetable}{F.1}
\centering
\caption{The closing probability falls in stages with a loss on the answer alone and returns after thinking replay at every size. Median probability of closing a thought at its natural end, by training stage (95\% bootstrap interval over thoughts in brackets, based on 400, 300 and 200 thoughts for 4B, 9B and 27B). First line of each size: thoughts written by the base model. Second line: thoughts written by the replayed model. The base 27B could not be loaded for this probe.}\label{tab:F.1}
{\small\setlength{\tabcolsep}{6pt}\renewcommand{\arraystretch}{1.1}
\noindent\begin{adjustbox}{max width=\linewidth}
\begin{tabular}{lrrrrr}
\toprule
{\begin{tabular}[b]{@{}l@{}}\textbf{size, writer of}\\\textbf{the thoughts}\end{tabular}} & \textbf{base model} & \textbf{-Rounds} & {\begin{tabular}[b]{@{}r@{}}\textbf{-Rounds +}\\\textbf{reader round}\end{tabular}} & {\begin{tabular}[b]{@{}r@{}}\textbf{-Rounds +}\\\textbf{thinking replay}\end{tabular}} & {\begin{tabular}[b]{@{}r@{}}\textbf{-Think}\\\textbf{(replay +}\\\textbf{reader round)}\end{tabular}} \\
\midrule
4B, base & 0.52 {[}0.50, 0.54{]} & 0.52 {[}0.49, 0.54{]} & 0.47 {[}0.43, 0.50{]} & 0.73 {[}0.68, 0.76{]} & 0.26 {[}0.20, 0.30{]} \\
4B, replayed & 0.72 {[}0.68, 0.74{]} & 0.59 {[}0.56, 0.61{]} & 0.64 {[}0.60, 0.66{]} & 0.89 {[}0.87, 0.91{]} & 0.39 {[}0.32, 0.45{]} \\
9B, base & 0.54 {[}0.52, 0.58{]} & 0.06 {[}0.05, 0.06{]} & 0.02 {[}0.01, 0.02{]} & 0.81 {[}0.76, 0.85{]} & 0.18 {[}0.13, 0.21{]} \\
9B, replayed & 0.65 {[}0.61, 0.70{]} & 0.05 {[}0.04, 0.05{]} & 0.02 {[}0.02, 0.02{]} & 0.93 {[}0.90, 0.95{]} & 0.27 {[}0.18, 0.38{]} \\
27B, base & -- & 0.84 {[}0.82, 0.86{]} & -- & 0.97 {[}0.93, 0.98{]} & 0.54 {[}0.50, 0.61{]} \\
27B, replayed & -- & 0.86 {[}0.83, 0.88{]} & -- & 0.98 {[}0.97, 0.99{]} & 0.87 {[}0.83, 0.91{]} \\
\bottomrule
\end{tabular}
\end{adjustbox}\par}
\end{table}

\subsection{The thoughts each 4B stage writes}\label{sec:F.2}

Table~\ref{tab:F.2} lets every 4B stage write its own thoughts on the same items. The base model
ends 91.1\% of them. After thinking replay 74.6\% end and 2.5\% loop, after the reader round that
follows 11.4\% end and 63.6\% loop, and without replay the reader round does no such harm (96.5\%
end), but those thoughts are a few lines long.

\begin{table}[!htbp]
\renewcommand{\thetable}{F.2}
\centering
\caption{Replay makes the 4B's thoughts long, and the reader round after it leaves only 11.4\% of them ending. Thoughts of each 4B stage on the 3,021 held-out items that StartLux-Decision-4B-Think routes to reasoning (own thoughts, 4,096-token limit, no loop detector).}\label{tab:F.2}
{\small\setlength{\tabcolsep}{6pt}\renewcommand{\arraystretch}{1.1}
\noindent\begin{adjustbox}{max width=\linewidth}
\begin{tabular}{lrrr}
\toprule
\textbf{4B stage} & {\begin{tabular}[b]{@{}r@{}}\textbf{thoughts}\\\textbf{that end}\end{tabular}} & {\begin{tabular}[b]{@{}r@{}}\textbf{in a loop}\\\textbf{at the}\\\textbf{limit}\end{tabular}} & {\begin{tabular}[b]{@{}r@{}}\textbf{tokens per}\\\textbf{thought, mean}\\\textbf{/ median}\end{tabular}} \\
\midrule
base model & 91.1\% & 0.4\% & 1,093 / 564 \\
-Rounds & 92.4\% & 2.8\% & 639 / 265 \\
-Rounds + reader round & 96.5\% & 3.0\% & 336 / 163 \\
-Rounds + thinking replay & 74.6\% & 2.5\% & 2,397 / 2,435 \\
-Think (replay + reader round) & 11.4\% & 63.6\% & 3,764 / 4,096 \\
\ldots{} + stop step & 85.9\% & 10.1\% & 1,413 / 768 \\
\bottomrule
\end{tabular}
\end{adjustbox}\par}
\end{table}

A loop sustains itself. Inside a loop no model closes the thought, the base model included: at the
start of the loop and at its end the median closing probability is 0.00 for all five stages (311
looping thoughts), and so it is at the point just before the looping line is written for the first
time (497 thoughts). Once a text repeats, repetition is what every model of the family predicts
next. What differs between stages is whether the thought is closed at its first conclusion. After
that the stages are alike.

What the reader round changes is not the reverse of what replay changed. The weight update of the
reader round has a cosine of $-$0.0022 with the update of thinking replay (200 adapted matrices of
the 4B). A reader round trained without replay has $-$0.0002. The two updates are close to
orthogonal: the reader round does not undo the replay, it moves something else that the closing
decision depends on. We have not identified what.

\subsection{What else we tried against thoughts that do not end}\label{sec:F.3}

Table~\ref{tab:F.3} lists inference-time measures and alternatives on the held-out items of
Chapter~\ref{sec:5}. Cutting every thought at 1,024 tokens gives the reference accuracy at a quarter
of the tokens on these items, but costs 0.79 index points (Table~\ref{tab:F.4}). A repetition
penalty with a loop detector ends more thoughts and loses half a point, and the base model's
thoughts need a reader that has been trained on thoughts.

\begin{table}[!htbp]
\renewcommand{\thetable}{F.3}
\centering
\caption{Thoughts end at unchanged accuracy with the stop step or when the base model writes them, but base-written thoughts need a reader trained on thoughts. Ways to deal with thoughts that do not end, StartLux-Decision-4B-Think, 3,021 held-out items (differences to the first row with 95\% bootstrap intervals over items).}\label{tab:F.3}
{\footnotesize\setlength{\tabcolsep}{5pt}\renewcommand{\arraystretch}{1.1}
\noindent\begin{adjustbox}{max width=\linewidth}
\begin{tabular}{>{\raggedright\arraybackslash}p{\mdw{0.4060}}>{\raggedleft\arraybackslash}p{\mdw{0.1695}}>{\raggedleft\arraybackslash}p{\mdw{0.1414}}>{\raggedleft\arraybackslash}p{\mdw{0.1182}}>{\raggedleft\arraybackslash}p{\mdw{0.1515}}}
\toprule
\textbf{setting} & \textbf{thoughts that end} & \textbf{tokens per thought} & \textbf{default control} & \textbf{difference} \\
\midrule
limit 4,096 (reference) & 11.4\% & 3,764 & 75.54 & -- \\
limit 16,384 & 12.6\% & 14,512 & 75.31 \textsuperscript{c} & +0.07 {[}$-$0.56, +0.73{]} \textsuperscript{c} \\
limit 16,384 with loop detector & 12.9\% (80.6\% cut at a loop) & 4,287 & 75.60 \textsuperscript{c} & +0.36 {[}$-$0.23, +0.96{]} \textsuperscript{c} \\
thought cut at 1,024 tokens & -- & 992 & 75.54 & +0.00 {[}$-$0.60, +0.63{]} \\
thought cut at 512 tokens & -- & 508 & 75.21 & $-$0.33 {[}$-$1.06, +0.36{]} \\
repetition penalty 1.1 with loop detector & 27.6\% (29.0\% cut at a loop) & 3,360 & 75.01 & $-$0.53 {[}$-$1.16, +0.10{]} \\
stop step (trained) & 85.9\% & 1,413 & 75.31 & $-$0.23 {[}$-$0.96, +0.50{]} \\
base model writes the thought, a model with the reader round (no replay) reads it & 91.1\% & 1,093 & 75.47 & $-$0.07 {[}$-$1.19, +1.06{]} \\
base model writes the thought, the model of the first row reads it & 91.1\% & 1,093 & 74.98 & $-$0.56 {[}$-$1.42, +0.30{]} \\
base model writes the thought, StartLux-Decision-4B-Rounds reads it (no reader round) & 91.1\% & 1,093 & 67.06 & $-$8.47 {[}$-$9.96, $-$6.95{]} \\
\bottomrule
\end{tabular}
\end{adjustbox}\par}
\par\smallskip
{\footnotesize\raggedright\noindent \textsuperscript{c} measured in a separate run with its own reference with the loop detector
(75.24). The difference is to that reference.\par}
\end{table}

\subsection{Every reasoning design on the index}\label{sec:F.4}

\clearpage
\begin{table}[!htbp]
\renewcommand{\thetable}{F.4}
\centering
\caption{Replay followed by the reader round scores highest on the index, at 1,144 reasoning tokens per answer. Every reasoning design on the full index, 4B (Decision Index 0.2.1, default control, 4,096-token limit, one run each). ``Reasoning tokens per answer'' is the mean over all answers, including those that are not thought about. One pass: 64.78 (knowledge 45.4, tools 86.0).}\label{tab:F.4}
{\footnotesize\setlength{\tabcolsep}{5pt}\renewcommand{\arraystretch}{1.1}
\noindent\begin{adjustbox}{max width=\linewidth}
\begin{tabular}{>{\raggedright\arraybackslash}p{\mdw{0.2360}}>{\raggedleft\arraybackslash}p{\mdw{0.0701}}>{\raggedleft\arraybackslash}p{\mdw{0.1148}}>{\raggedleft\arraybackslash}p{\mdw{0.0639}}>{\raggedleft\arraybackslash}p{\mdw{0.1216}}>{\raggedleft\arraybackslash}p{\mdw{0.1140}}>{\raggedleft\arraybackslash}p{\mdw{0.1242}}>{\raggedleft\arraybackslash}p{\mdw{0.1428}}}
\toprule
\textbf{design (4B)} & \textbf{index} & \textbf{knowledge} & \textbf{tools} & \textbf{answers thought about} & \textbf{tokens per thought} & \textbf{thoughts at the limit} & \textbf{reasoning tokens per answer} \\
\midrule
reader round only (no replay) & 66.38 & 50.0 & 86.1 & 32.2\% & 388 & 0.6\% & 125 \\
-Think (replay, then reader round) & \textbf{67.72} & 57.0 & 85.3 & 33.3\% & 3,439 & 57.5\% & 1,144 \\
\ldots{} thought cut at 1,024 tokens & 66.93 & 53.8 & 85.2 & 33.2\% & 1,003 & -- & 333 \\
\ldots{} + stop step & 67.37 & 55.7 & 85.2 & 31.3\% & 1,585 & 10.4\% & 497 \\
\ldots{} + stop step + reinforcement learning, rollouts sampled at temperature 1 \textsuperscript{f} & 67.23 & 55.1 & 84.8 & 31.4\% & 1,053 & 3.2\% & 330 \\
\ldots{} + stop step + reinforcement learning, rollouts sampled as at inference & 66.80 & 53.5 & 85.0 & 32.5\% & 617 & 0.4\% & 200 \\
\ldots{} + stop step + readout trained on thoughts sampled by the current model & 67.43 & 55.6 & 85.4 & 31.1\% & 1,845 & 13.9\% & 574 \\
base model writes the thought, the model of row 2 reads it & 67.62 & 57.7 & 84.3 & 33.2\% & 1,316 & 8.7\% & 438 \\
joint stage from the -Rounds model (F.6) & 67.11 & 57.0 & 84.0 & 47.0\% & 2,666 & 39.9\% & 1,254 \\
\ldots{} + stop step & 66.42 & 55.7 & 83.0 & 44.3\% & 1,631 & 13.6\% & 723 \\
reinforcement learning from the -Rounds model \textsuperscript{e} & 67.18 & 53.5 & 86.2 & 31.1\% & 184 & 0.7\% & 57 \\
\bottomrule
\end{tabular}
\end{adjustbox}\par}
\par\smallskip
{\footnotesize\raggedright\noindent \textsuperscript{e} 78.5\% of this model's thoughts on the index have fewer than 16 tokens: it skips
most of the questions it is asked to reason about, and its row is the score of a system that mostly
does not reason. \textsuperscript{f} 2.1\% of the thoughts have fewer than 16 tokens (0.9\% after
the stop step alone, none before it), and 57\% have 128 to 1,023 tokens.\par}
\end{table}

\subsection{Token limit, loop check and gate}\label{sec:F.5}

\begin{table}[!htbp]
\renewcommand{\thetable}{F.5}
\centering
\caption{A longer limit adds nothing, a loop check removes most open thoughts at no cost, and a gate of 0.7 costs half an index point while one of 0.98 adds nothing. Token limit, loop check and gate (4B, accuracy in percent). \emph{Block A:} 3,021 routed held-out items of the training distribution, one thought per item. The loop check looks for repetition every 256 tokens and ends a thought that has begun to repeat. In brackets: paired difference of the default answer to the 4,096-token row of the same model without a check, with its 95\% bootstrap interval over items. Index: Decision Index 0.2.1 with the gate at 0.9, one run per row, and ``--'' means not measured. \emph{Block B:} the gate, for StartLux-Decision-4B-Think with a limit of 4,096 tokens. Held-out columns: the 8,598 held-out items of the training distribution, stored thoughts replayed at each threshold. Index: one run per threshold.}\label{tab:F.5}
{\footnotesize\setlength{\tabcolsep}{6pt}\renewcommand{\arraystretch}{1.1}
\noindent\begin{adjustbox}{max width=\linewidth}
\begin{tabular}{lrlrrrrrr}
\toprule
\textbf{4B model} & \textbf{limit} & {\begin{tabular}[b]{@{}l@{}}\textbf{loop}\\\textbf{check}\end{tabular}} & {\begin{tabular}[b]{@{}r@{}}\textbf{after the}\\\textbf{thought}\end{tabular}} & \textbf{default answer} & {\begin{tabular}[b]{@{}r@{}}\textbf{open}\\\textbf{at the}\\\textbf{limit}\end{tabular}} & {\begin{tabular}[b]{@{}r@{}}\textbf{cut}\\\textbf{at a}\\\textbf{loop}\end{tabular}} & {\begin{tabular}[b]{@{}r@{}}\textbf{tokens}\\\textbf{per}\\\textbf{thought}\end{tabular}} & \textbf{index} \\
\midrule
-Think & cut at 1,024 & no & -- & 75.54 (+0.00 {[}$-$0.60, +0.63{]}) & -- & -- & 992 & 66.93 \\
 & 4,096 & no & 75.04 & 75.54 & 88.6\% & -- & 3,764 & 67.72 \\
 & 4,096 & yes & 74.91 & 75.54 & 24.1\% & 63.9\% & 2,916 & -- \\
 & 8,192 & yes & 74.61 & 75.11 ($-$0.43 {[}$-$1.09, +0.20{]}) & 6.9\% & 80.2\% & 3,367 & 67.52 \textsuperscript{c} \\
 & 16,384 & no & 74.54 & 75.31 \textsuperscript{a} & 87.4\% & -- & 14,512 & -- \\
 & 16,384 & yes \textsuperscript{b} & 75.14 & 75.60 \textsuperscript{a} & -- & 80.6\% & 4,287 & -- \\
\ldots{} and stop step & 4,096 & no & 74.38 & 75.31 & 14.1\% & -- & 1,413 & 67.37 \\
 & 4,096 & yes & 74.54 & 75.60 (+0.30 {[}$-$0.40, +0.99{]}) & 3.5\% & 12.6\% & 1,186 & -- \\
 & 8,192 & yes & 74.61 & 75.37 & 0.7\% & -- & 1,251 & -- \\
\bottomrule
\end{tabular}
\end{adjustbox}\par}
\par\smallskip
{\footnotesize\raggedright\noindent \textsuperscript{a} measured in a separate run against its own 4,096-token reference with the loop
detector (75.24): differences +0.07 {[}$-$0.56, +0.73{]} and +0.36 {[}$-$0.23, +0.96{]}.
\textsuperscript{b} the loop detector of Table~\ref{tab:F.3}, the guard of the reasoning server.
\textsuperscript{c} index run with a limit of 8,192 tokens. The loop check of the reasoning server
(checked every 1,024 tokens) was on in this run as in every index run of the table, so the index
column compares limits and gates, not checks.\par}
\par\medskip
{\small\setlength{\tabcolsep}{6pt}\renewcommand{\arraystretch}{1.1}
\noindent\begin{adjustbox}{max width=\linewidth}
\begin{tabular}{lrrr}
\toprule
{\begin{tabular}[b]{@{}l@{}}\textbf{B. gate: a thought is}\\\textbf{written when the one-pass}\\\textbf{top probability is below}\end{tabular}} & {\begin{tabular}[b]{@{}r@{}}\textbf{held-out items:}\\\textbf{questions}\\\textbf{thought about}\end{tabular}} & {\begin{tabular}[b]{@{}r@{}}\textbf{held-out items:}\\\textbf{default answer}\end{tabular}} & \textbf{index} \\
\midrule
never (one pass) & 0.0\% & 89.33 & -- \\
0.5 & 6.3\% & 90.20 & -- \\
0.7 & 18.9\% & 90.71 & 67.20 \\
0.9 (default) & 35.1\% & 90.71 & 67.72 \\
0.98 & -- & -- & 67.51 \\
always & 100.0\% & 90.72 & -- \\
\bottomrule
\end{tabular}
\end{adjustbox}\par}
\end{table}

\subsection{The joint variant}\label{sec:F.6}

The three repair stages are steps in sequence, each of which moves what the previous one fixed. The
joint variant replaces them by one stage in which every step holds thinking targets and read-out
targets (15,870 thinking targets, 16,000 read-outs after a thought and 16,000 one-pass read-outs
with soft targets, 747 steps), from the -Rounds model and from the replayed model
(Table~\ref{tab:F.6}). It gives the best default answer on the diagnostic items and is below the
sequence on held-out items, and on the index the first arm scores 67.11 with the gate firing on 47\%
of the answers instead of 33\%.

\begin{table}[!htbp]
\renewcommand{\thetable}{F.6}
\centering
\caption{The joint stage gives the best default answer on diagnostic items and trails the sequence on held-out items. Joint stage against the sequence (4B).}\label{tab:F.6}
{\footnotesize\setlength{\tabcolsep}{6pt}\renewcommand{\arraystretch}{1.1}
\noindent\begin{adjustbox}{max width=\linewidth}
\begin{tabular}{lrrrrrr}
\toprule
\textbf{4B model} & {\begin{tabular}[b]{@{}r@{}}\textbf{diagnostic}\\\textbf{items: thoughts}\\\textbf{that end}\end{tabular}} & {\begin{tabular}[b]{@{}r@{}}\textbf{one}\\\textbf{pass}\end{tabular}} & {\begin{tabular}[b]{@{}r@{}}\textbf{default}\\\textbf{control}\end{tabular}} & {\begin{tabular}[b]{@{}r@{}}\textbf{held-out items:}\\\textbf{thoughts that}\\\textbf{end}\end{tabular}} & {\begin{tabular}[b]{@{}r@{}}\textbf{tokens}\\\textbf{per}\\\textbf{thought}\end{tabular}} & {\begin{tabular}[b]{@{}r@{}}\textbf{default}\\\textbf{control}\end{tabular}} \\
\midrule
-Think (replay, then reader round) & -- \textsuperscript{d} & 72.7 & 75.9 & 11.4\% & 3,764 & 75.54 \\
replay, reader round, stop step & 88.2\% & 72.9 & 75.2 & 85.9\% & 1,413 & 75.31 \\
joint stage from the -Rounds model & 67.8\% & 72.0 & 75.6 & 57.3\% & 2,740 & 73.58 \\
joint stage from the replayed model & 72.7\% & 73.2 & 76.5 & 64.3\% & 2,613 & 74.91 \\
\bottomrule
\end{tabular}
\end{adjustbox}\par}
\par\smallskip
{\footnotesize\raggedright\noindent \textsuperscript{d} the diagnostic thoughts of this row were written by the replayed model before
its reader round (78.4\% end).\par}
\end{table}

\subsection{Reinforcement learning: calibration of the answer after the thought}\label{sec:F.7}

Table~\ref{tab:F.7} reads the answer after the thought of the stop-trained checkpoints before any
temperature is fitted, on the 3,021 routed held-out items, and the ranking measures after a
temperature has been fitted, on the test part of the items.

\begin{table}[!htbp]
\renewcommand{\thetable}{F.7}
\centering
\caption{With the proper score, reinforcement learning lowers the calibration error after a thought at both sizes without improving the ranking of answers. Calibration of the answer after the thought for the stop-trained 4B and 9B and the arms with the bounded proper score. Stated confidence, overconfidence (stated confidence minus accuracy), calibration error, Brier score and log score are read before any temperature is fitted. ``Fitted temperature'' is the temperature that calibrates this read-out. The area under the risk--coverage curve (lower is better) and the share of answers that can be accepted at an error of 5\% are read after the temperature has been fitted.}\label{tab:F.7}
{\scriptsize\setlength{\tabcolsep}{3pt}\renewcommand{\arraystretch}{1.1}
\noindent\begin{adjustbox}{max width=\linewidth}
\begin{tabular}{>{\raggedright\arraybackslash}p{\mdw{0.0790}}>{\raggedright\arraybackslash}p{\mdw{0.0970}}>{\raggedleft\arraybackslash}p{\mdw{0.0816}}>{\raggedleft\arraybackslash}p{\mdw{0.0959}}>{\raggedleft\arraybackslash}p{\mdw{0.1283}}>{\raggedleft\arraybackslash}p{\mdw{0.0982}}>{\raggedleft\arraybackslash}p{\mdw{0.0575}}>{\raggedleft\arraybackslash}p{\mdw{0.0690}}>{\raggedleft\arraybackslash}p{\mdw{0.1104}}>{\raggedleft\arraybackslash}p{\mdw{0.0857}}>{\raggedleft\arraybackslash}p{\mdw{0.0845}}}
\toprule
\textbf{answer after the thought} & \textbf{rollouts} & \textbf{accuracy} & \textbf{stated confidence} & \textbf{overconfidence} & \textbf{calibration error} & \textbf{Brier score} & \textbf{log score} & \textbf{fitted temperature} & \textbf{area under the risk--coverage curve} & \textbf{accepted at an error of 5\%} \\
\midrule
4B after the stop step (start) & -- & 74.38 & 83.70 & +9.32 & 9.43 & 0.3713 & $-$0.7302 & 1.55 & 0.1172 & 20.5\% \\
\ldots{} trained, bounded proper score & as at inference & 74.11 & 80.27 & +6.15 & 6.38 & 0.3642 & $-$0.6918 & 1.35 & 0.1201 & 18.0\% \\
9B after the stop step (start) & -- & 81.20 & 84.27 & +3.07 & 3.77 & -- & -- & 1.23 & 0.0528 & 63.1\% \\
\ldots{} trained, bounded proper score & temperature 1 & 80.97 & -- & -- & 3.76 & -- & -- & -- & -- & -- \\
\ldots{} trained, bounded proper score & as at inference & 80.87 & 81.91 & +1.04 & 2.14 & 0.2577 & $-$0.4848 & 1.05 & 0.0527 & 60.2\% \\
\bottomrule
\end{tabular}
\end{adjustbox}\par}
\end{table}

``--'' in block B: not given in our record of the run.
