# Supplementary material for: StartLux-Decision: AutoThink Decision Models with Reinforcement Learning for Calibrated Deliberative Decisions
Source: arXiv:2610.17309 source file (2026-10-20)
Supplement: Supplementary file 13 [file appendix_F_training_settings.tex]

\clearpage
\section{Training settings}\label{sec:F}

All training ran on one cluster of eight nodes with eight H200 GPUs each (141 GiB per GPU). One
trainer serves every stage. It reads a packed, pre-tokenised mix and a batch plan.
Table~\ref{tab:F.1} gives the settings that hold for a stage at every size, Tables~\ref{tab:F.2} to
\ref{tab:F.4} the values per size.

\subsection{Settings by stage}\label{sec:F.1}

\begingroup
\renewcommand{\thetable}{F.1}
\footnotesize\setlength{\tabcolsep}{5pt}\renewcommand{\arraystretch}{1.1}
\begin{longtable}{>{\raggedright\arraybackslash}p{\mdw{0.1363}}>{\raggedright\arraybackslash}p{\mdw{0.2870}}>{\raggedright\arraybackslash}p{\mdw{0.2701}}>{\raggedright\arraybackslash}p{\mdw{0.1410}}>{\raggedright\arraybackslash}p{\mdw{0.1523}}}
\caption{Settings that are the same at every size, stages as columns.}\label{tab:F.1}\\
\toprule
\textbf{setting} & \textbf{full fine-tuning (release, step 1)} & \textbf{adapter fine-tuning (release, step 2)} & \textbf{averaging (release, step 3)} & \textbf{decision data round} \\
\midrule
\endfirsthead
\multicolumn{5}{l}{\textit{Table~\thetable{} (continued)}}\\
\toprule
\textbf{setting} & \textbf{full fine-tuning (release, step 1)} & \textbf{adapter fine-tuning (release, step 2)} & \textbf{averaging (release, step 3)} & \textbf{decision data round} \\
\midrule
\endhead
\bottomrule
\endfoot
starting weights & public starting model (Table~\ref{tab:F.2}) & the same starting model & merged adapter model and fully fine-tuned checkpoint & released weights of the size \\
trained parameters & all parameters of the text layers and the output layer. The vision tower is not trained & low-rank adapter. Everything else frozen & none & low-rank adapter. Everything else frozen \\
adapter & -- & rank 64, $\alpha$ 128, no dropout, on the query, key, value and output projections of the attention layers, the three projections of the linear-attention layers and the three projections of the feed-forward blocks & -- & the same \\
loss & soft cross-entropy between the row's target and the softmax over its listed options, on the 26 letter rows of the output layer at the last prompt position, computed in FP32. Row weight divided by the mean weight of the mix & the same & -- & the same \\
read-out position & last token of the prompt. Letters not listed are masked & the same & -- & the same \\
data & broad mix (Table~\ref{tab:4.2}) & curated mix (Table~\ref{tab:4.2}) & -- & final recipe (Table~\ref{tab:4.2}) \\
epochs & 1 & 2 & -- & 1 \\
optimiser & AdamW, $\beta$1 0.9, $\beta$2 0.95, $\epsilon$ 1e-8 & AdamW, $\beta$1 0.9, $\beta$2 0.999, $\epsilon$ 1e-8 & -- & AdamW, $\beta$1 0.9, $\beta$2 0.999, $\epsilon$ 1e-8 \\
weight decay & 0 & 0 & -- & 0 \\
gradient clipping & norm 1.0 & norm 1.0 & -- & norm 1.0 \\
schedule & linear warm-up over 3\% of the steps, cosine decay to zero (27B: to 10\% of the peak) & cosine decay \todo{warm-up share of the release adapter runs, 3\% or 5\%} & -- & linear warm-up over 5\% of the steps, cosine decay to zero \\
precision & bf16 computation. 0.8B--4B: bf16 parameters updated directly. 9B and 27B: FP32 master weights (ZeRO stage 2) & bf16 computation, frozen weights in bf16, adapter weights in FP32 & sum in FP32, stored in bf16 & as adapter fine-tuning \\
gradient checkpointing & on & on & -- & on \\
longest input & 12,288 tokens. Longer rows are dropped when the mix is packed & the same & -- & the same \\
padding & to the right, to one of 36 fixed widths (multiples of 64 up to 512, of 128 up to 2,048, of 512 up to 8,192, of 1,024 above) & the same & -- & the same \\
batch plan & first step is the longest batch of the mix. Then shuffled pools of 32 batches sorted by length. Within a step the longest rows go to the GPU with the fewest tokens, and each GPU runs length groups at their own width & the same & -- & the same (length-group setting: minimum 16,384 tokens, waste 0.25) \\
option order & permuted per row by a hash of the row (score levels keep their order) & the same & -- & the same \\
after training & checkpoint as is & adapter merged into the starting weights & $\alpha$\textperiodcentered{}A + (1 $-$ $\alpha$)\textperiodcentered{}B per tensor, $\alpha$ = 0.5 & adapter merged into the released weights \\
seeds & \todo{} & \todo{} & -- & trainer 20261001, mixer shuffle seeded by the name of the mix \\
\end{longtable}
\endgroup

The trainer does not use the full-vocabulary language-model loss: the model is trained on the
restricted softmax that the server returns. Replay rows that hold a model to an earlier state are
not a separate loss term. They are ordinary rows whose target is that model's own distribution. The
0.8B, 2B and 4B tie the output layer to the input embedding, so training the 26 letter rows also
moves the input embeddings of the letters. The 9B and 27B do not tie them.

\subsection{Release recipe per size}\label{sec:F.2}

\begin{table}[!htbp]
\renewcommand{\thetable}{F.2}
\centering
\caption{Release recipe, values per size. ``Rows per step'' is GPUs $\times$ rows per GPU $\times$ accumulation steps. Hours are those the trainer reports. Losses are the smoothed training loss at the end of the run.}\label{tab:F.2}
{\footnotesize\setlength{\tabcolsep}{5pt}\renewcommand{\arraystretch}{1.1}
\noindent\begin{adjustbox}{max width=\linewidth}
\begin{tabular}{>{\raggedright\arraybackslash}p{\mdw{0.1847}}>{\raggedleft\arraybackslash}p{\mdw{0.1106}}>{\raggedleft\arraybackslash}p{\mdw{0.1410}}>{\raggedleft\arraybackslash}p{\mdw{0.1410}}>{\raggedleft\arraybackslash}p{\mdw{0.1194}}>{\raggedleft\arraybackslash}p{\mdw{0.1106}}>{\raggedright\arraybackslash}p{\mdw{0.1801}}}
\toprule
 & \textbf{0.8B} & \textbf{2B} & \textbf{4B} & \textbf{9B} & \textbf{27B} & \textbf{35B-A3B} \\
\midrule
starting model & Qwen3.5-0.8B-Base & Qwen3.5-2B, instruction-tuned & Qwen3.5-4B, instruction-tuned & Qwen3.5-9B, post-trained & Qwen3.8-27B & \todo{verify starting model} (project notes: Qwen3.6-35B-A3B) \\
\midrule
\multicolumn{7}{l}{\textbf{Full fine-tuning}} \\
mix (rows) & 2,726,203 & 2,726,203 & 2,726,203 & 2,726,203 & 791,992 & \todo{} \\
peak learning rate & 2e-5 & 1e-5 & 1e-5 & 5e-6 & 2e-6 & \todo{} \\
rows per step & 384 = 8 $\times$ 48 & 192 = 8 $\times$ 24 & 256 = 16 $\times$ 16 & 256 = 16 $\times$ 8 $\times$ 2 & 224 = 56 $\times$ 4 & \todo{} \\
steps & 7,099 & 14,198 & 10,649 & 10,649 & 3,535 & \todo{} \\
engine & DDP & DDP & DDP & ZeRO stage 2 & ZeRO stage 2 & \todo{} \\
hours & 1.03 & 1.75 & 2.10 & 4.41 & 3.19 & \todo{} \\
final training loss & 0.453 & 0.432 & 0.382 & 0.344 & 0.294 & \todo{} \\
tokens per second and GPU & 35.8 K & 18.6 K & 7.5 K & 3.5 K & 0.49 K \textsuperscript{a} & \todo{} \\
\midrule
\multicolumn{7}{l}{\textbf{Adapter fine-tuning}} \\
mix (rows) & -- & 190,418 & 92,228 & 190,418 & 190,418 & \todo{} \\
peak learning rate & -- & 1e-4 & 1e-4 & 1e-4 & 5e-5 & \todo{} \\
rows per step & -- & 256 = 8 $\times$ 32 & 184 = 8 $\times$ 23 & 96 = 8 $\times$ 12 & 128 = 16 $\times$ 4 $\times$ 2 & \todo{} \\
steps (2 epochs) & -- & 1,486 & 1,002 & 3,966 & 2,974 & \todo{} \\
hours & -- & 0.56 & 0.50 & 1.39 & 2.42 & \todo{} \\
final training loss & -- & 0.354 & 0.307 & 0.280 & 0.294 & \todo{} \\
\midrule
\multicolumn{7}{l}{\textbf{Averaging}} \\
weight of the adapter model & -- (step 1 alone) & 0.5 & 0.5 & 0.5 & 0.5 & 0.5 by project notes \todo{verify} \\
tensors averaged & -- & 321 & 427 & 427 & 851 & \todo{} \\
\textbf{Temperatures} (yes/no / choice / score) & 3.29 / 1.756 / 1.893 & 2.291 / 1.532 / 1.616 & 1.591 / 1.387 / 1.417 & 1.724 / 1.229 / 1.294 & 1.421 / 1.21 / 1.229 & \todo{} \\
\bottomrule
\end{tabular}
\end{adjustbox}\par}
\par\smallskip
{\footnotesize\raggedright\noindent \textsuperscript{a} Measured before the two throughput fixes (fixed padding widths, balanced
placement of long rows), which raised the 4B from 1.0 K to 2.2 K and from 4.7 K to 7.3 K tokens per
second and GPU.\par}
\end{table}

The 27B was fine-tuned on seven nodes with the eighth evaluating every checkpoint (707 steps apart)
on a 15\% sample of the index: 43.06 before training, 57.67 after 707 steps, 59.10 at the end
(edition 0.2). The first step of every run, the longest batch, peaked at 86 to 116 GiB on its GPU.

\begin{table}[!htbp]
\renewcommand{\thetable}{F.3}
\centering
\caption{Trainable parameters of the rank-64 adapter.}\label{tab:F.3}
{\small\setlength{\tabcolsep}{6pt}\renewcommand{\arraystretch}{1.1}
\noindent\begin{adjustbox}{max width=\linewidth}
\begin{tabular}{lrlrlr}
\toprule
 & \textbf{0.8B} & \textbf{2B} & \textbf{4B} & \textbf{9B} & \textbf{27B} \\
\midrule
trainable parameters & 40.89 M & \todo{} & 122 M & \todo{} & 435 M \\
share of all parameters & 5.4\% & \todo{} & 2.9\% & \todo{} & 1.6\% \\
\bottomrule
\end{tabular}
\end{adjustbox}\par}
\end{table}

\subsection{Decision data rounds per size}\label{sec:F.3}

\begin{table}[!htbp]
\renewcommand{\thetable}{F.4}
\centering
\caption{Final recipe of the decision data rounds. One adapter round per size on the released weights. Settings of Table~\ref{tab:F.1}.}\label{tab:F.4}
{\footnotesize\setlength{\tabcolsep}{5pt}\renewcommand{\arraystretch}{1.1}
\noindent\begin{adjustbox}{max width=\linewidth}
\begin{tabular}{>{\raggedright\arraybackslash}p{\mdw{0.1795}}>{\raggedright\arraybackslash}p{\mdw{0.1967}}>{\raggedright\arraybackslash}p{\mdw{0.1405}}>{\raggedright\arraybackslash}p{\mdw{0.1660}}>{\raggedright\arraybackslash}p{\mdw{0.1405}}>{\raggedright\arraybackslash}p{\mdw{0.1637}}}
\toprule
 & \textbf{0.8B} & \textbf{2B} & \textbf{4B} & \textbf{9B} & \textbf{27B} \\
\midrule
starting weights & released (first-stage checkpoint) & released & released & released & released \\
rows after packing & 1,078,668 & 1,078,710 & 1,078,729 & 1,078,578 & \todo{} \\
sample of the release mix & 4B adapter mix, 30,000 & 4B adapter mix, 30,000 & 4B adapter mix, 30,000 & 4B adapter mix, 30,000 & 27B full-fine-tuning mix, 30,000 \\
anchor rows (weight 3) & own distribution of the released 0.8B & of the released 2B & of the released 4B, 25,191 rows & of the released 9B & of the released 27B \\
learning rate & 5e-5 & 5e-5 & 5e-5 & 5e-5 & 5e-5 \\
rows per step & 184 & 184 & 184 = 8 $\times$ 23 & 96 = 8 $\times$ 12 & 128 = 8 $\times$ 4 $\times$ 4 \\
steps & 5,862 & 5,862 & 5,862 & 11,235 & 8,408 \\
GPUs & 8 & 8 & 8 & 8 & 8 \\
training time & about 45 min & 63 min & \todo{} \textsuperscript{b} & \todo{} \textsuperscript{c} & \todo{} \textsuperscript{d} \\
temperatures after the round & \todo{} & \todo{} & \todo{} & \todo{} & \todo{} \\
Decision Index 0.2.1, one pass & 51.60 & 57.66 & 64.78 & 67.75 & 70.43 \\
\bottomrule
\end{tabular}
\end{adjustbox}\par}
\par\smallskip
{\footnotesize\raggedright\noindent \textsuperscript{b} The preceding full-recipe round of 1.08 M rows trained at 0.73 s per step.
\textsuperscript{c} An earlier 9B round took 62 minutes for 2,443 steps. \textsuperscript{d} About
4.7 s per step were logged at the start of the run, and 73\% of the steps were done after 7 h 53
min. The manuscript gives ``about two hours (4B), three hours (9B) and eight to nine hours (27B)''
for the rounds \todo{replace by the trainer-reported hours of the five runs}.\par}
\end{table}

\begin{table}[!htbp]
\renewcommand{\thetable}{F.5}
\centering
\caption{Earlier rounds of the same line (one pass, own runs). Every round starts from the released weights.}\label{tab:F.5}
{\footnotesize\setlength{\tabcolsep}{5pt}\renewcommand{\arraystretch}{1.1}
\noindent\begin{adjustbox}{max width=\linewidth}
\begin{tabular}{>{\raggedright\arraybackslash}p{\mdw{0.0536}}>{\raggedright\arraybackslash}p{\mdw{0.2035}}>{\raggedleft\arraybackslash}p{\mdw{0.0981}}>{\raggedleft\arraybackslash}p{\mdw{0.0936}}>{\raggedright\arraybackslash}p{\mdw{0.1122}}>{\raggedleft\arraybackslash}p{\mdw{0.0701}}>{\raggedright\arraybackslash}p{\mdw{0.3561}}}
\toprule
\textbf{size} & \textbf{round} & \textbf{rows} & \textbf{steps} & \textbf{learning rate} & \textbf{index} & \textbf{what changed} \\
\midrule
4B & 4 & \todo{} & \todo{} & 1e-4 & 55.06 & teacher rows, sample of the release mix, anchor, four generators \\
4B & 5 & as round 4 & as round 4 & 5e-5 & 56.11 & learning rate \\
4B & 7 & 311,560 & 1,693 & 5e-5 & 58.31 & + replay of train splits, group-statement preference, forecasting \\
4B & 8 & \todo{} & 1,758 & 5e-5 & 58.91 & + chords \\
4B & 10 & \todo{} & 3,391 & 5e-5 & 59.45 & aspect sentiment and shopping relevance resampled \\
4B & 11 & 665,896 & 3,619 & 5e-5 & 60.69 & + phishing generator \\
4B & 11, repeated under another seed & 670,291 & 3,641 & 5e-5 & 60.87 & mixer seed, rows restored by the duplicate fix \\
4B & 12 & \todo{} & \todo{} & 5e-5 & 60.94 & + chess \\
4B & 14 & 838,446 & \todo{} & 5e-5 & 60.03 & + official tool-retrieval rows, select-all from two upstream sources \\
4B & 18 & 1,081,189 & \todo{} & 5e-5 & 63.32 & full recipe \\
4B & 18 without the tool-retrieval rows & \todo{} & \todo{} & 5e-5 & 64.29 &  \\
4B & 19 & 1,111,709 & 6,040 & 5e-5 & 63.94 & 18 + four select-all sources \\
4B & 20, final & 1,078,729 & 5,862 & 5e-5 & 64.78 & 18 without those rows, four select-all sources, anchor $\times$ 3, general multiple choice \\
9B & first round & \todo{} & 2,443 & 5e-5 & 61.24 & as 4B round 5 \\
9B & round 7 recipe & \todo{} & 3,246 & 5e-5 & 62.25 &  \\
9B & full recipe without the tool-retrieval rows & \todo{} & \todo{} & 5e-5 & 67.53 &  \\
27B & first round & \todo{} & \todo{} & 5e-5 & 65.62 &  \\
27B & round 7 recipe & 313,103 & 2,446 & 5e-5 & 66.63 &  \\
27B & recipe of the eleventh 4B round & \todo{} & \todo{} & 5e-5 & 68.78 &  \\
27B & full recipe without the tool-retrieval rows & \todo{} & 8,119 & 5e-5 & 70.08 &  \\
\bottomrule
\end{tabular}
\end{adjustbox}\par}
\end{table}

\subsection{Calibration}\label{sec:F.4}

One temperature per question type is fitted after every merge or average by the same script. Fit
rows are the development splits of three sets of an open decision-model project (2,069 choice, 973
yes/no, 35 score rows). The script reads the raw letter scores of the checkpoint on these rows,
rendered as in training, and for each type searches 1,201 logarithmically spaced values between 0.2
and 5 for the temperature with the lowest mean cross-entropy to the targets. A type with fewer than
200 fit rows takes the temperature fitted on all fit rows combined. The script reports the negative
log-likelihood and the calibration error (top label, ten bins) before and after the fit on every
other development set: the test splits of the same three sets (3,097 rows), a held-out set of hard
rows split off by parent group (11,505 rows), human-labelled rows of twelve public sets (1,800 rows)
and 1,000 questions of a multiple-choice knowledge set. It also writes the three temperatures into
the configuration file of the checkpoint.

\begin{table}[!htbp]
\renewcommand{\thetable}{F.6}
\centering
\caption{Effect of the fitted temperatures over the 47 checkpoints of the release campaign.}\label{tab:F.6}
{\footnotesize\setlength{\tabcolsep}{6pt}\renewcommand{\arraystretch}{1.1}
\noindent\begin{adjustbox}{max width=\linewidth}
\begin{tabular}{lrrr}
\toprule
\textbf{evaluation set} & {\begin{tabular}[b]{@{}r@{}}\textbf{mean at}\\\textbf{temperature}\\\textbf{1}\end{tabular}} & {\begin{tabular}[b]{@{}r@{}}\textbf{mean with}\\\textbf{fitted}\\\textbf{temperatures}\end{tabular}} & {\begin{tabular}[b]{@{}r@{}}\textbf{checkpoints}\\\textbf{better /}\\\textbf{worse}\end{tabular}} \\
\midrule
test splits of the fit source (3,097 rows), calibration error & 0.0956 & 0.0246 & 47 / 0 \\
hard public JevBench items (111), calibration error & 0.1219 & 0.0924 & 37 / 10 \\
ten probability items of the same benchmark, total variation & 0.1354 & 0.1386 & 19 / 28 \\
check set close to the training distribution (17,402 rows), calibration error & 0.0285 & 0.0491 & 11 / 36 \\
\bottomrule
\end{tabular}
\end{adjustbox}\par}
\end{table}

\subsection{Settings that were tried and not adopted}\label{sec:F.5}

\textbf{Second-stage adapter on the fully fine-tuned weights} (release campaign). Rank 64, $\alpha$
128, learning rate 1e-4 (5e-5 at 27B), 5\% warm-up, cosine decay, two epochs, merged. Data: 11,909
new rows from the training files of an open decision-model project. Mined rows: 19,000 to 23,000
from eight pools of rows unseen in step 1, 80\% of them rows that the first-stage model gets wrong
or holds below 0.6 on the gold label (total variation above 0.25 for soft targets) and 20\% easy
rows, one source at most a quarter of a pool's quota. Human-labelled rows: 3,000 of twelve public
sets. Replay rows whose target is the first-stage distribution (about 10,000 at first, 26,600 to
30,000 later). From the second day also 38,096 teacher-written rows and 15,000 exact-probability
rows. A check before training confirmed that the frozen first-stage model reproduces the replay
targets from the packed rows (mean divergence 0.0, same top option in 100\% of 2,048 rows).

\begin{table}[!htbp]
\renewcommand{\thetable}{F.7}
\centering
\caption{Second-stage adapter: change of the Decision Index against the parent checkpoint (edition 0.2.1 unless noted).}\label{tab:F.7}
{\footnotesize\setlength{\tabcolsep}{5pt}\renewcommand{\arraystretch}{1.1}
\noindent\begin{adjustbox}{max width=\linewidth}
\begin{tabular}{>{\raggedright\arraybackslash}p{\mdw{0.6103}}>{\raggedleft\arraybackslash}p{\mdw{0.1716}}>{\raggedleft\arraybackslash}p{\mdw{0.2041}}}
\toprule
\textbf{run} & \textbf{steps} & \textbf{change} \\
\midrule
day 1, 4B, first recipe (edition 0.2) & 512 & $-$1.34 \\
day 1, 4B, recipe without mining in benchmark splits, larger replay & 662 & +0.07 \\
day 2: 0.8B / 2B / 4B from Base / 4B instruction-tuned / 9B / 27B & 604 / 896 / 1,232 / 1,234 / 2,360 / 1,348 & $-$1.25 / $-$0.85 / $-$0.92 / $-$1.21 / $-$1.48 / $-$2.10 \\
day 3, 4B: day-1 recipe without teacher-written and exact-probability rows / 4B adapter mix, no replay / adapter mix of the other sizes, no replay / 4B adapter mix with replay & 656 / 1,002 / 2,068 / 1,244 & $-$0.50 / $-$1.11 / $-$2.86 / $-$0.84 \\
day 3, 27B: day-1 recipe without teacher-written and exact-probability rows & 1,034 & $-$2.08 \\
\bottomrule
\end{tabular}
\end{adjustbox}\par}
\end{table}

\clearpage
\begin{table}[!htbp]
\renewcommand{\thetable}{F.8}
\centering
\caption{Averaging ratio (release campaign): Decision Index 0.2.1 and correct public JevBench items of 231, by the weight of the adapter model. The released models use 0.5. The released 0.8B is a fully fine-tuned model from the Base checkpoint (38.86), not on this line.}\label{tab:F.8}
{\small\setlength{\tabcolsep}{6pt}\renewcommand{\arraystretch}{1.1}
\noindent\begin{adjustbox}{max width=\linewidth}
\begin{tabular}{lrrrrr}
\toprule
\textbf{size} & \textbf{0} & \textbf{0.25} & \textbf{0.5} & \textbf{0.75} & \textbf{1} \\
\midrule
0.8B, instruction-tuned start & 36.76 \textperiodcentered{} 173 & 37.26 \textperiodcentered{} 179 & 36.34 \textperiodcentered{} 181 & 34.68 \textperiodcentered{} 179 & 32.55 \textperiodcentered{} 180 \\
2B & 44.64 \textperiodcentered{} 194 & 44.89 \textperiodcentered{} 194 & 44.19 \textperiodcentered{} 196 & 42.23 \textperiodcentered{} 192 & 39.58 \textperiodcentered{} 189 \\
4B & 54.70 \textperiodcentered{} 198 & 54.39 \textperiodcentered{} 200 & 52.75 \textperiodcentered{} 204 & 49.13 \textperiodcentered{} 204 & 44.13 \textperiodcentered{} 205 \\
9B & 58.78 \textperiodcentered{} 196 & 59.20 \textperiodcentered{} 200 & 58.63 \textperiodcentered{} 201 & 56.66 \textperiodcentered{} 200 & 53.76 \textperiodcentered{} 197 \\
27B & 64.02 \textperiodcentered{} 207 & 64.25 \textperiodcentered{} 207 & 63.88 \textperiodcentered{} 208 & 63.04 \textperiodcentered{} 205 & 61.39 \textperiodcentered{} 205 \\
\bottomrule
\end{tabular}
\end{adjustbox}\par}
\end{table}

\textbf{Other release settings.} Learning rate of full fine-tuning at 9B: 2e-5 from the Base
checkpoint 51.68, 1e-5 56.07, 5e-6 from the post-trained checkpoint 58.78. At 4B from the
instruction-tuned checkpoint: 1e-5 54.70, 5e-6 51.79. Adapter on the 4B: rank 64 at 1e-4 answered
205 of the 231 public items, rank 64 at 5e-5 201, rank 16 199. An adapter that leaves the lowest
third of the layers untouched lost more than three points on a broad development set.

\textbf{Data-round settings.} Learning rate 1e-4 against 5e-5: 55.06 against 56.11 (4B), 61.04
against 61.24 (9B), and 7e-5 with another seed 61.16 (9B). Interpolation of a 9B round towards its
starting weights: 61.24 at weight 1, 61.14 at 0.7, 60.85 at 0.5. Average of two rounds: 61.70 from
61.24 and 61.04 (9B), 56.09 from 56.11 and 55.06 (4B), and of two seeds 56.28 from 56.11 and 56.10.
A second adapter round for one source on a merged round: 195 steps at 4B (12,000 chord rows and
24,000 rows resampled from the round's mix) and 375 steps at 9B.

\subsection{Generation settings for written data}\label{sec:F.6}

\begin{table}[!htbp]
\renewcommand{\thetable}{F.9}
\centering
\caption{Sampling settings of the models that wrote or verified training data.}\label{tab:F.9}
{\footnotesize\setlength{\tabcolsep}{5pt}\renewcommand{\arraystretch}{1.1}
\noindent\begin{adjustbox}{max width=\linewidth}
\begin{tabular}{>{\raggedright\arraybackslash}p{\mdw{0.1331}}>{\raggedright\arraybackslash}p{\mdw{0.2460}}>{\raggedright\arraybackslash}p{\mdw{0.1734}}>{\raggedright\arraybackslash}p{\mdw{0.2838}}>{\raggedright\arraybackslash}p{\mdw{0.1503}}}
\toprule
 & \textbf{writer of teacher items} & \textbf{verifiers} & \textbf{writers of API-written items} & \textbf{blind verifier of API-written items} \\
\midrule
model & Qwen3.8-27B (release batch: half of the second 40,000 seeds by Qwen3.6-35B-A3B) & Qwen3.8-27B and Qwen3.6-35B-A3B & GLM-5.3, DeepSeek-V4-Pro & the model of the other family \\
served by & vLLM on our GPUs, one process per GPU, prefix caching off & the same & an OpenAI-compatible third-party endpoint \todo{provider, model versions, dates, terms} & the same \\
temperature / top-p & 0.9 / 0.95 & 0.9 / 0.95 \todo{confirm for the verifier runs} & 0.8 by default \todo{value used} & \todo{} \\
new tokens & at most 16,000 (release scale-up: 10,000) & at most 16,000 & 6,000 by default, about 1,650 output tokens per retrieval call & \todo{} \\
reasoning & on in the pilot and in the data-round batch, off in the release scale-up & on & off, except for the mathematics family & on \\
context limit & 32,768 tokens & 32,768 tokens & -- & -- \\
seed & shard index & shard index & -- & -- \\
\bottomrule
\end{tabular}
\end{adjustbox}\par}
\end{table}
