# Supplementary material for: StartLux-Decision: AutoThink Decision Models with Reinforcement Learning for Calibrated Deliberative Decisions
Source: arXiv:2610.17309 source file (2026-10-20)
Supplement: Supplementary file 14 [file appendix_G_data.tex]

\clearpage
\section{Data details}\label{sec:G}

\subsection{Record format}\label{sec:G.1}

A canonical record has an identifier, a parent group, a source, a family, a type (choice with 2 to
26 options, yes/no, score with 2 to 10 ordered levels), a state, instructions, options (identifier
and criterion), a target that sums to one, a target kind and an optional weight. Converters apply
the following rules.

\begin{itemize}
\item A probability dictionary of the source is mapped to the options. A single label becomes a one-hot
target. Targets are normalised, rounded to six decimals, and the rounding error is added to the
largest entry.
\item A choice with more than 26 options keeps every option with positive probability and is filled to 26
at random. A score with more than ten levels becomes a choice.
\item A uniform target is dropped, except for program labels and for questions that are undecidable by
design.
\item An option whose identifier is a single letter has its identifier hidden, so that a prompt never
shows two letters for one option.
\item A record is rejected when its type is not one of the three, when it has fewer than 2 or more than 26
options or a repeated option, or when its target does not cover the options.
\end{itemize}

\begin{table}[!htbp]
\renewcommand{\thetable}{G.1}
\centering
\caption{Question types and target kinds, release pool and release mixes (rows).}\label{tab:G.1}
{\scriptsize\setlength{\tabcolsep}{4pt}\renewcommand{\arraystretch}{1.1}
\noindent\begin{adjustbox}{max width=\linewidth}
\begin{tabular}{>{\raggedright\arraybackslash}p{\mdw{0.1441}}>{\raggedleft\arraybackslash}p{\mdw{0.1045}}>{\raggedleft\arraybackslash}p{\mdw{0.1045}}>{\raggedleft\arraybackslash}p{\mdw{0.1045}}>{\raggedleft\arraybackslash}p{\mdw{0.1063}}>{\raggedleft\arraybackslash}p{\mdw{0.1060}}>{\raggedleft\arraybackslash}p{\mdw{0.1548}}>{\raggedleft\arraybackslash}p{\mdw{0.1623}}}
\toprule
 & \textbf{choice} & \textbf{yes/no} & \textbf{score} & \textbf{single gold label} & \textbf{program label} & \textbf{distribution from a model} & \textbf{distribution from the source} \\
\midrule
candidate pool (6,397,500) & 3,569,820 (55.8\%) & 1,683,991 (26.3\%) & 1,143,689 (17.9\%) & 4,760,575 (74.4\%) & 1,082,361 (16.9\%) & 465,226 (7.3\%) & 89,338 (1.4\%) \\
full fine-tuning mix, 0.8B--9B & 1,767,949 & 643,719 & 314,535 &  &  &  &  \\
full fine-tuning mix, 27B & 608,907 & 130,193 & 52,892 &  &  &  &  \\
adapter mix, 2B / 9B / 27B & 112,090 & 59,649 & 18,679 &  &  &  &  \\
adapter mix, 4B & 42,650 & 38,096 & 11,482 &  &  &  &  \\
\bottomrule
\end{tabular}
\end{adjustbox}\par}
\end{table}

Two labels in this table are loose: 10,447 rows counted as ``distribution from a model'' are
dialogue-intent distributions derived from human labels, and the 5,978 rows of the typed-decisions
set counted as ``distribution from the source'' are means of three samples of a teacher model.
Prompt lengths in tokens (median / 90th / 99th percentile, rows dropped above 12,288 tokens): 164 /
654 / 2,405 (1,131 dropped) for the full-fine-tuning mix of the 0.8B to 9B models, 191 / 805 / 3,962
(370) for that of the 27B, 305 / 1,202 / 3,443 (661) for the adapter mix of the 2B, 9B and 27B, and
260 / 985 / 2,974 (642) for that of the 4B. In the largest mix 40.2\% of the rows have two options,
18.0\% four and 2.3\% the maximum of 26.

\subsection{Sources of the release pool}\label{sec:G.2}

\begingroup
\renewcommand{\thetable}{G.2}
\footnotesize\setlength{\tabcolsep}{5pt}\renewcommand{\arraystretch}{1.1}
\begin{longtable}{>{\raggedright\arraybackslash}p{\mdw{0.1439}}>{\raggedright\arraybackslash}p{\mdw{0.2413}}>{\raggedright\arraybackslash}p{\mdw{0.2092}}>{\raggedleft\arraybackslash}p{\mdw{0.0987}}>{\raggedright\arraybackslash}p{\mdw{0.1632}}>{\raggedright\arraybackslash}p{\mdw{0.1306}}}
\caption{The 25 source files of the release pool (6,397,500 candidate rows). A 26th file with 6,174 rows of development and test splits is used for evaluation and calibration only, and two superseded teacher files are not counted. Licences per data set: Tables~\ref{tab:G.4} to \ref{tab:G.6}.}\label{tab:G.2}\\
\toprule
\textbf{internal file} & \textbf{what it is} & \textbf{official source} & \textbf{rows in the pool} & \textbf{target} & \textbf{licence as stated} \\
\midrule
\endfirsthead
\multicolumn{6}{l}{\textit{Table~\thetable{} (continued)}}\\
\toprule
\textbf{internal file} & \textbf{what it is} & \textbf{official source} & \textbf{rows in the pool} & \textbf{target} & \textbf{licence as stated} \\
\midrule
\endhead
\bottomrule
\endfoot
\texttt{jevembed} & community corpus of typed decisions with many sub-sources, 448,383 rows that it copies from other corpora of this table were dropped at conversion & \texttt{HIT-\allowbreak{}TMG/\allowbreak{}JevEmbed-\allowbreak{}Data} & 1,151,741 & gold labels and source distributions & apache-2.0, cc0-1.0, cc-by-4.0, ``mixed licences'', recorded per row \\
\texttt{distill} & community corpus with teacher distributions and program labels, 137,203 rows with uniform placeholder targets dropped & \texttt{SargeDev/\allowbreak{}jev-\allowbreak{}distill-\allowbreak{}corpus-\allowbreak{}v3} & 516,057 & teacher distributions (about 440,000 rows), program labels & apache-2.0 \\
\texttt{bev} & community corpus: hard decisions, skills, numeric and temporal questions & \texttt{avbiswas/\allowbreak{}bev-\allowbreak{}decision-\allowbreak{}150K} & 409,937 & gold labels & unknown, the card asserts no single licence for the mixed-source release \\
\texttt{openjev} & community corpus & \texttt{ZefanCai/\allowbreak{}Open-\allowbreak{}Jev-\allowbreak{}v1.1} & 147,139 & program labels & other: CC0-1.0 for generated content, CC BY 4.0 for one included set \\
\texttt{decider} & general public mixture: output of the public data builder of an open decision-model project, run by us & builder \texttt{Mapika/\allowbreak{}decider} (repository Apache-2.0) over the data sets of Table~\ref{tab:G.4} & 1,976,644 & gold labels, program labels for rule tasks, that project's teacher-written tasks (about 110,000 rows) & per data set, Table~\ref{tab:G.4} \\
\texttt{procedural} & procedural corpus: arithmetic, table look-up, evidence sufficiency, policy applicability & \texttt{tasksource/\allowbreak{}procedural-\allowbreak{}jev} & 729,910 & program labels & apache-2.0 \\
\texttt{probgen} & exact-probability questions, own generator (G.6) & -- & 39,995 & exact distributions & own \\
\texttt{ditrain} & train and development splits of 15 index benchmarks rebuilt in the suite's layout & Table~\ref{tab:G.5} & 425,112 & gold labels & per data set, Table~\ref{tab:G.5} \\
\texttt{ditrain\_sgd} & dialogue-intent rows rebuilt in the layout the suite actually stores (whole dialogue, target = distribution of the active intent over the user turns) & schema-guided dialogue set, train and dev & 16,345 & distribution derived from gold labels & CC BY-SA 4.0 \\
\texttt{tools} & call-or-not per candidate tool, and which tool from a list, from three function-calling corpora & \texttt{Team-\allowbreak{}ACE/\allowbreak{}ToolACE}, \texttt{NousResearch/\allowbreak{}hermes-\allowbreak{}function-\allowbreak{}calling-\allowbreak{}v1}, \texttt{Salesforce/\allowbreak{}xlam-\allowbreak{}function-\allowbreak{}calling-\allowbreak{}60k} & 54,163 & gold labels of the corpora & apache-2.0, apache-2.0, cc-by-4.0 (gated) \\
\texttt{tools\_xlam} & the same two layouts from the third corpus alone & \texttt{Salesforce/\allowbreak{}xlam-\allowbreak{}function-\allowbreak{}calling-\allowbreak{}60k} & 191,695 & gold labels & cc-by-4.0 (gated) \\
\texttt{tools\_\allowbreak{}jevdec} & next-tool choice in agent traces & \texttt{samatv256/\allowbreak{}jev-\allowbreak{}decisions-\allowbreak{}v1}, rows of four agent-trace sets & 88,658 & gold labels & cc-by-4.0 \\
\texttt{apibank\_\allowbreak{}train} & API-Bank training dialogues (levels 1 and 2) as selection of one tool & \texttt{liminghao1630/\allowbreak{}API-\allowbreak{}Bank} & 6,383 & gold labels & mit \\
\texttt{kmc} & knowledge and commonsense multiple choice in two layouts: ARC, OpenBookQA, QASC, CommonsenseQA, MedQA, a 20\% sample of MedMCQA, a 35\% sample of RACE & Table~\ref{tab:G.6} & 91,456 & gold labels & per data set \\
\texttt{std} & SciQ, AQuA-RAT and QuALITY train, When2Call preference pairs (9,000) & Table~\ref{tab:G.6} & 120,669 & gold labels & per data set \\
\texttt{winogrande} & WinoGrande XL train & \texttt{allenai/\allowbreak{}winogrande} & 40,398 & gold labels & none on the card, repository Apache-2.0 \\
\texttt{hellaswag} & HellaSwag train & \texttt{Rowan/\allowbreak{}hellaswag} & 39,905 & gold labels & none in the card metadata, card text says MIT \\
\texttt{codex\_ab} & public train splits converted and filtered in an earlier project of ours & Table~\ref{tab:G.6} & 238,469 & gold labels, some weighted & per data set \\
\texttt{eikos} & English rows of two training files written by a program or by Qwen3.8-27B, rows by another writer model and translated rows dropped & \texttt{caiovicentino1/\allowbreak{}eikos-\allowbreak{}decisions} & 16,311 & program labels, teacher distributions (6,343 rows) & cc-by-4.0 \\
\texttt{kev\_new} & training files of an open decision-model project: developer tools, dates, unknowable questions, assertions, ambiguity & public code repository of the Kev project (\texttt{kev}), commit 3e1cd3bb & 11,978 & gold labels, 50/50 targets where the answer is unknowable & repository Apache-2.0 \\
\texttt{plumb} & hard decisions with teacher probabilities & \texttt{crh225/\allowbreak{}plumb-\allowbreak{}decisions} & 5,014 & teacher distributions & apache-2.0 \\
\texttt{typed} & typed-decisions set, train split: 1,200 cases of four workflows & \texttt{LocalLLaMA/\allowbreak{}typed-\allowbreak{}decisions} & 5,978 & mean of three teacher samples & apache-2.0 \\
\texttt{teacher\_v12} & teacher-written hard decisions, release batch (Section~\ref{sec:4.2}) & -- & 38,150 & writer's gold label, confirmed by two verifiers & own \\
\texttt{wildjailbreak} & harmful or benign: 8,000 prompts of each of four data types, 70\% as a two-option choice, 30\% as yes/no & \texttt{allenai/\allowbreak{}wildjailbreak}, train & 31,997 & data type of the source & odc-by, gated, terms accepted for the account that fetched it \\
\texttt{cfcolor\_\allowbreak{}train} & pairs of five-colour palettes, ``which would this user rate higher'', built from the train ratings only & original release of the palette ratings & 3,396 & human ratings & not confirmed \todo{source page and terms} \\
\end{longtable}
\endgroup

\subsection{Sources of the decision data rounds}\label{sec:G.3}

\begingroup
\renewcommand{\thetable}{G.3a}
\footnotesize\setlength{\tabcolsep}{5pt}\renewcommand{\arraystretch}{1.1}
\begin{longtable}{>{\raggedright\arraybackslash}p{\mdw{0.1347}}>{\raggedright\arraybackslash}p{\mdw{0.3007}}>{\raggedright\arraybackslash}p{\mdw{0.2484}}>{\raggedleft\arraybackslash}p{\mdw{0.1065}}>{\raggedleft\arraybackslash}p{\mdw{0.1058}}>{\raggedleft\arraybackslash}p{\mdw{0.0909}}}
\caption{The 30 source files of the final data round (4B build). ``Built'' is the number of rows the builder wrote, and ``in the mix'' is after the scan, de-duplication and caps.}\label{tab:G.3a}\\
\toprule
\textbf{internal file} & \textbf{what it contains} & \textbf{built from} & \textbf{built} & \textbf{in the mix} & \textbf{row weight} \\
\midrule
\endfirsthead
\multicolumn{6}{l}{\textit{Table~\thetable{} (continued)}}\\
\toprule
\textbf{internal file} & \textbf{what it contains} & \textbf{built from} & \textbf{built} & \textbf{in the mix} & \textbf{row weight} \\
\midrule
\endhead
\bottomrule
\endfoot
\texttt{teacher\_v3a} & teacher-labelled decisions, first batch (48,000 seeds) & Section~\ref{sec:4.2} & 27,939 & 27,865 & 1 \\
\texttt{teacher\_v3b} & second batch (12,000 seeds) &  & 6,908 & 6,883 & 1 \\
\texttt{teacher\_v3c} & third batch &  & 6,953 & 6,939 & 1 \\
\texttt{final/\allowbreak{}4bi\_\allowbreak{}r1} (cap 30,000) & sample of the 4B adapter mix of the release & Table~\ref{tab:G.2} & 92,228 & 29,993 & as in the source \\
\texttt{r4\_\allowbreak{}replay\_\allowbreak{}kl\_\allowbreak{}soup50\_\allowbreak{}w3} & anchor: replay rows of the release mixes whose target is the released 4B's own distribution & prediction pass of the released model & 26,635 & 25,191 & 3 \\
\texttt{kmc} (cap 30,000) & knowledge and commonsense multiple choice & Table~\ref{tab:G.2} & 91,456 & 29,296 & 1 \\
\texttt{kr\_\allowbreak{}causal\_\allowbreak{}v1} & causal-reasoning questions, generated & own generator \todo{description} & \todo{} & 31,363 & \todo{} \\
\texttt{kr\_sata\_v1} & select-all questions on synthetic paragraphs about people and topics & own generator & \todo{} & 48,019 & \todo{} \\
\texttt{kr\_musr\_v1} & narrative-reasoning stories & 12,000 plans, stories written by Qwen3.8-27B, verified & \todo{} & 6,152 & \todo{} \\
\texttt{kr\_musr\_pl2} & object-placement stories & 4,000 plans, 3,617 verified & 3,617 & 3,395 & \todo{} \\
\texttt{kr\_home\_v1s} & appliance-simulator questions with state and options in sorted order & own generator \todo{description} & 52,941 & 52,401 & \todo{} \\
\texttt{ditrain4\_\allowbreak{}replay\_\allowbreak{}big} & replay of train splits: ANLI 30,000, HoVer 12,000, CLINC150 6,000, BANKING77 5,000, Humicroedit 4,000, dialogue intent 3,000, and all rows of VAST, RAGTruth, ContractNLI, NLI4CT, sarcasm tasks A and C, GSM8K, caption matching (caps before the scan) & the train-split rebuilds of Table~\ref{tab:G.2} & 110,187 & 100,679 & 1 \\
\texttt{ditrain4\_\allowbreak{}isarc\_\allowbreak{}nat} & six sarcasm-category questions for every English training text & iSarcasmEval train & 20,802 & 20,736 & 0.5 \\
\texttt{ditrain4\_\allowbreak{}w2cq} & When2Call official training set in the benchmark's layout, four response kinds as options, after the question-level check & \texttt{nvidia/\allowbreak{}When2Call}, train & 8,918 & 8,798 & 1 \\
\texttt{winogrande} (cap 20,000) & WinoGrande XL train & Table~\ref{tab:G.2} & 40,398 & 20,000 & 1 \\
\texttt{cfcolor\_\allowbreak{}train} & palette preference pairs & Table~\ref{tab:G.2} & 3,396 & 3,396 & 1 \\
\texttt{ditrain4\_\allowbreak{}sentfin} & entity-level sentiment of financial headlines in the layout of the entity-sentiment benchmark & SEntFiN 1.0 (10,753 headlines, 14,371 entity--sentiment pairs) & \todo{} & 13,975 & 1 \\
\texttt{ditrain4\_\allowbreak{}longmid} & long-document rows of 20,000 to 46,000 characters, at most 400 per source & two long-context files built on 1--2 October \todo{which sources contributed} & \todo{} & 491 & 1 \\
\texttt{ditrain3\_\allowbreak{}acos\_\allowbreak{}nat} & aspect-category sentiment: all 39 pairs for restaurant reviews, for laptop reviews the gold pairs, the other sentiments of the gold categories and 48 random pairs & official train files & 234,828 & 234,504 & 0.2 \\
\texttt{ditrain3\_\allowbreak{}esci\_\allowbreak{}sqrt} & shopping-query relevance: locales in natural shares, labels within a locale in proportion to the square root of their natural share & official train split & 89,999 & 89,904 & 1 \\
\texttt{kr\_phish\_v2} & phishing decisions: 9,000 generated e-mails with seven questions each & own generator, second version & 63,000 & 63,000 & 0.5 \\
\texttt{kr\_chess\_v1} (cap 40,000) & chess positions with engine analysis of every legal move & own builder, Stockfish & 65,555 & 40,000 & \todo{} \\
\texttt{kr\_sata\_v2} & select-all from two upstream sources: 3,000 PubMed articles with 14 root categories, 5,126 MultiRC train questions with all candidate answers & public PubMed multi-label set, MultiRC train & \todo{} (15,844 dropped by the scan) & 63,534 & \todo{} \\
\texttt{kr\_sata\_v3x} & select-all from four upstream sources: toxicity attributes (2,000 sentences, 16,000 rows), news topics (840 documents, 5,040 rows), EU-law descriptors (3,200 documents before the scan, 6 of 15 questions each), company events (1,126 documents, 6,756 rows) & RealToxicityPrompts, Reuters-21578 ModApte train, EURLEX57K train, a biotech events set, train & \todo{} & 37,061 & \todo{} \\
\texttt{ditrain2\_\allowbreak{}habermas} & group-statement preference: official training questions, both iterations of a round & Habermas Machine data, training cohorts & 2,286 & 2,236 & 1 \\
\texttt{ditrain2\_\allowbreak{}forecast} & forecasting questions resolved before 2026-07-01, at most 1,500 per source and outcome & ForecastBench question and resolution sets & 18,496 & 7,825 & 1 \\
\texttt{kr\_chord\_v1} & chord recognition: 1,500 generated songs, 8 target beats each & own generator & 12,000 & 12,000 & 1 \\
\texttt{kr\_rr\_v1} & retrieval items written by API models: per query 1.38 useful and 3.66 tempting documents and two documents of other queries & 5,162 written items & 36,324 & 35,567 & 1 \\
\texttt{kr\_lim\_v1} & limerick against a minimally corrupted copy & 6,167 written limericks & 17,920 & 17,855 & 1 \\
\texttt{kr\_bbh\_v1} & state tracking and deduction, ten families & own generator & 52,000 & 39,730 & 1 \\
\textbf{total} &  &  &  & \textbf{1,078,788} &  \\
\end{longtable}
\endgroup

\begin{table}[!htbp]
\renewcommand{\thetable}{G.3b}
\centering
\caption{What each round of the 4B line added (Table~\ref{tab:F.5} has rows, steps and scores).}\label{tab:G.3b}
{\footnotesize\setlength{\tabcolsep}{5pt}\renewcommand{\arraystretch}{1.1}
\noindent\begin{adjustbox}{max width=\linewidth}
\begin{tabular}{>{\raggedright\arraybackslash}p{\mdw{0.1544}}>{\raggedright\arraybackslash}p{\mdw{0.8313}}}
\toprule
\textbf{round} & \textbf{sources} \\
\midrule
1--5 & teacher-labelled decisions, 30,000-row sample of the release adapter mix, anchor rows, generators for causal reasoning (1), code execution (2 and 3, removed), select-all and narrative reasoning (3), the appliance simulator (4), chess (3 only) \\
7 & + replay of train splits (71,939 rows), group-statement preference (2,236), forecasting (8,227) \\
8 & + chords (12,000) \\
9 & + chords from human lead sheets (21,479) and 4,000 rows of the API-Bank training rebuild, both removed again \\
10 & aspect sentiment and shopping relevance rebuilt with the benchmark's label priors, the old rows of both removed from the replay \\
11 & + phishing generator, first version (6,000 e-mails) \\
12 & + chess (40,000) \\
14 & + official tool-retrieval training rows (68,661, removed in the final recipe) and select-all from two upstream sources \\
18 & + When2Call training set, sarcasm categories for all texts, larger replay, WinoGrande 20,000, palette pairs, entity sentiment, long-document rows, second batch of narrative stories, state tracking, written retrieval items, limerick pairs, phishing generator, second version \\
19 & + select-all from four further upstream sources \\
20 (final) & 18 without the tool-retrieval rows, the four select-all sources with more EU-law documents, anchor at weight 3, 30,000 general multiple-choice rows \\
21, 22 (experimental) & 20 + 6,201 evidence-removal rows from a claim-verification train split, 20 + 40,000 rows of a search-relevance source \\
\bottomrule
\end{tabular}
\end{adjustbox}\par}
\end{table}

By weight, round 14 (838,446 rows, weight mass 629,843, 1.29 billion characters) was 41.7\%
generators for single benchmarks, 32.6\% rebuilt train splits, 10.3\% replay of other train splits,
6.6\% teacher-labelled decisions and 8.4\% sample of the release mix with the anchor. The select-all
sources took 17.7\% of the weight for a benchmark that weighs 2.58\% in the index, and the simulator
rows 15.5\% of all text.

\subsection{Licences of the public data sets}\label{sec:G.4}

\begingroup
\renewcommand{\thetable}{G.4}
\footnotesize\setlength{\tabcolsep}{5pt}\renewcommand{\arraystretch}{1.1}
\begin{longtable}{>{\raggedright\arraybackslash}p{\mdw{0.1663}}>{\raggedright\arraybackslash}p{\mdw{0.2881}}>{\raggedright\arraybackslash}p{\mdw{0.2467}}>{\raggedright\arraybackslash}p{\mdw{0.1569}}>{\raggedright\arraybackslash}p{\mdw{0.1286}}}
\caption{Data sets of the general public mixture : the tasks that the local copy of the builder registers for training. The first-day 4B mix and the full-fine-tuning mix of the 0.8B to 9B models take every task (at most 25,000 rows per task). ``27B'' marks the tasks whose plain form is also in the 27B mixes (format variants of all tasks are). ``4B-a'' marks the tasks in the 4B adapter mix and therefore in the 30,000-row sample of the data rounds. The builder's own teacher-written and rule-based tasks (repository Apache-2.0) are in all of them. \todo{the internal record speaks of about 95 public sets; the local copy of the builder registers 71 training tasks on 58 data sets. Check the copy that was run.}}\label{tab:G.4}\\
\toprule
\textbf{task} & \textbf{data set (split)} & \textbf{licence as stated} & \textbf{27B} & \textbf{4B-a} \\
\midrule
\endfirsthead
\multicolumn{5}{l}{\textit{Table~\thetable{} (continued)}}\\
\toprule
\textbf{task} & \textbf{data set (split)} & \textbf{licence as stated} & \textbf{27B} & \textbf{4B-a} \\
\midrule
\endhead
\bottomrule
\endfoot
intent, out of scope & \texttt{clinc/\allowbreak{}clinc\_\allowbreak{}oos} plus (train) & cc-by-3.0 &  &  \\
banking intent & \texttt{mteb/\allowbreak{}banking77} (train) & mit on this mirror, original \texttt{PolyAI/\allowbreak{}banking77} cc-by-4.0 &  &  \\
assistant intent & \texttt{SetFit/\allowbreak{}amazon\_\allowbreak{}massive\_\allowbreak{}intent\_\allowbreak{}en-\allowbreak{}US} (train) & none stated on this mirror, original \texttt{AmazonScience/\allowbreak{}massive} cc-by-4.0 &  &  \\
support intent & \texttt{bitext/\allowbreak{}Bitext-\allowbreak{}customer-\allowbreak{}support-\allowbreak{}llm-\allowbreak{}chatbot-\allowbreak{}training-\allowbreak{}dataset} & cdla-sharing-1.0 &  & $\checkmark$ \\
support tickets & \texttt{Tobi-\allowbreak{}Bueck/\allowbreak{}customer-\allowbreak{}support-\allowbreak{}tickets} & cc-by-nc-4.0 &  & $\checkmark$ \\
news topic & \texttt{fancyzhx/\allowbreak{}ag\_\allowbreak{}news} (train) & unknown, the card quotes the source's permission for non-commercial use &  &  \\
encyclopedia class & \texttt{fancyzhx/\allowbreak{}dbpedia\_\allowbreak{}14} (train) & cc-by-sa-3.0 &  &  \\
question topic & \texttt{community-\allowbreak{}datasets/\allowbreak{}yahoo\_\allowbreak{}answers\_\allowbreak{}topics} (train) & unknown &  &  \\
newsgroup & \texttt{SetFit/\allowbreak{}20\_\allowbreak{}newsgroups} (train) & none stated &  &  \\
review sentiment & \texttt{stanfordnlp/\allowbreak{}imdb}, \texttt{stanfordnlp/\allowbreak{}sst2}, \texttt{SetFit/sst5}, \texttt{Yelp/\allowbreak{}yelp\_\allowbreak{}review\_\allowbreak{}full}, \texttt{SetFit/\allowbreak{}amazon\_\allowbreak{}reviews\_\allowbreak{}multi\_\allowbreak{}en} (train) & other, unknown, none stated, other (the publisher's own licence), apache-2.0 &  &  \\
emotion & \texttt{dair-\allowbreak{}ai/\allowbreak{}emotion}, \texttt{google-\allowbreak{}research-\allowbreak{}datasets/\allowbreak{}go\_\allowbreak{}emotions} (train) & other (``educational and research purposes only''), apache-2.0 &  &  \\
tweets: sentiment, emotion, offensive, hate & \texttt{cardiffnlp/\allowbreak{}tweet\_\allowbreak{}eval} (train) & unknown, the card says every subset has its own licence &  &  \\
counterfactual, subjectivity & \texttt{SetFit/\allowbreak{}amazon\_\allowbreak{}counterfactual\_\allowbreak{}en}, \texttt{SetFit/subj} (train) & none stated &  &  \\
hate and offence & \texttt{SetFit/\allowbreak{}hate\_\allowbreak{}speech\_\allowbreak{}offensive} (train), \texttt{ucberkeley-\allowbreak{}dlab/\allowbreak{}measuring-\allowbreak{}hate-\allowbreak{}speech} & none stated, cc-by-4.0 &  &  \\
toxicity & \texttt{google/\allowbreak{}civil\_\allowbreak{}comments} (first 400,000 train rows), \texttt{lmsys/\allowbreak{}toxic-\allowbreak{}chat} (train) & cc0-1.0, cc-by-nc-4.0 &  &  \\
spam, insincere questions & \texttt{ucirvine/\allowbreak{}sms\_\allowbreak{}spam}, \texttt{SetFit/\allowbreak{}enron\_\allowbreak{}spam}, \texttt{SetFit/\allowbreak{}insincere-\allowbreak{}questions} & unknown, none stated, none stated &  &  \\
inference & \texttt{stanfordnlp/\allowbreak{}snli}, \texttt{nyu-\allowbreak{}mll/\allowbreak{}multi\_\allowbreak{}nli} (train) & cc-by-sa-4.0, cc-by-3.0, cc-by-sa-3.0, mit, other &  & $\checkmark$ \\
GLUE tasks: RTE, QNLI, QQP, MRPC, CoLA & \texttt{nyu-\allowbreak{}mll/\allowbreak{}glue} (train) & other: the original licences of each task &  & $\checkmark$ (QNLI) \\
yes/no reading & \texttt{google/\allowbreak{}boolq} (train) & cc-by-sa-3.0 & $\checkmark$ & $\checkmark$ \\
science questions & \texttt{allenai/\allowbreak{}ai2\_\allowbreak{}arc} Challenge and Easy (train), \texttt{allenai/\allowbreak{}qasc}, \texttt{allenai/\allowbreak{}openbookqa} (train) & cc-by-sa-4.0, cc-by-4.0, unknown & $\checkmark$ & $\checkmark$ \\
commonsense & \texttt{tau/\allowbreak{}commonsense\_\allowbreak{}qa}, \texttt{Rowan/\allowbreak{}hellaswag}, \texttt{ybisk/piqa}, \texttt{allenai/\allowbreak{}winogrande} XL (train) & mit, none in metadata (card text: MIT), unknown, none on the card (repository Apache-2.0) & $\checkmark$ & $\checkmark$ (not PIQA) \\
reading comprehension & \texttt{ehovy/race} (train) & other: ``available for non-commercial research purpose only'' & $\checkmark$ & $\checkmark$ \\
general knowledge & \texttt{cais/mmlu}, auxiliary training split & mit & $\checkmark$ &  \\
medicine & \texttt{GBaker/\allowbreak{}MedQA-\allowbreak{}USMLE-\allowbreak{}4-\allowbreak{}options}, \texttt{openlifescienceai/\allowbreak{}medmcqa} (train) & cc-by-4.0, apache-2.0 & $\checkmark$ & $\checkmark$ (MedMCQA) \\
occupation from biography & \texttt{LabHC/\allowbreak{}bias\_\allowbreak{}in\_\allowbreak{}bios} (train) & mit &  &  \\
response rating and preference & \texttt{nvidia/\allowbreak{}HelpSteer2}, \texttt{nvidia/\allowbreak{}HelpSteer3}, \texttt{HuggingFaceH4/\allowbreak{}ultrafeedback\_\allowbreak{}binarized}, \texttt{stanfordnlp/\allowbreak{}shp}, \texttt{Anthropic/\allowbreak{}hh-\allowbreak{}rlhf} (train) & cc-by-4.0, cc-by-4.0, mit, none stated, mit & $\checkmark$ (HelpSteer2, UltraFeedback) & $\checkmark$ (HelpSteer2) \\
similarity, veracity, safety of dialogue & \texttt{SetFit/stsb}, \texttt{chengxuphd/\allowbreak{}liar2}, \texttt{allenai/\allowbreak{}prosocial-\allowbreak{}dialog} (train) & none stated, apache-2.0, cc-by-4.0 &  &  \\
SuperGLUE tasks: COPA, WiC, MultiRC & \texttt{aps/\allowbreak{}super\_\allowbreak{}glue} (train) & other: the original licences of each task & $\checkmark$ (COPA, MultiRC) &  \\
fact verification & \texttt{copenlu/\allowbreak{}fever\_\allowbreak{}gold\_\allowbreak{}evidence} (train) & cc-by-sa-3.0, gpl-3.0 & $\checkmark$ &  \\
answer sentence, passage relevance & \texttt{microsoft/\allowbreak{}wiki\_\allowbreak{}qa}, \texttt{microsoft/\allowbreak{}ms\_\allowbreak{}marco} v1.1 (train) & other (a research data licence agreement), none on the card, and the official site says ``non-commercial research purposes only'' &  &  \\
tool calls & \texttt{glaiveai/\allowbreak{}glaive-\allowbreak{}function-\allowbreak{}calling-\allowbreak{}v2}, \texttt{Team-\allowbreak{}ACE/\allowbreak{}ToolACE} (train) & apache-2.0, apache-2.0 & $\checkmark$ & $\checkmark$ (first) \\
agent and web traces & \texttt{AgentGym/\allowbreak{}AgentTraj-\allowbreak{}L}, \texttt{osunlp/\allowbreak{}Mind2Web} (train) & none stated, cc-by-4.0 & $\checkmark$ &  \\
\end{longtable}
\endgroup

\begingroup
\renewcommand{\thetable}{G.5}
\footnotesize\setlength{\tabcolsep}{5pt}\renewcommand{\arraystretch}{1.1}
\begin{longtable}{>{\raggedright\arraybackslash}p{\mdw{0.1944}}>{\raggedright\arraybackslash}p{\mdw{0.3115}}>{\raggedright\arraybackslash}p{\mdw{0.1780}}>{\raggedright\arraybackslash}p{\mdw{0.3023}}}
\caption{Sources of the benchmark train splits and of the upstream training sides. ``Release'' = in the release pool, ``rounds'' = in the final data round.}\label{tab:G.5}\\
\toprule
\textbf{benchmark} & \textbf{what we read} & \textbf{used in} & \textbf{licence as stated} \\
\midrule
\endfirsthead
\multicolumn{4}{l}{\textit{Table~\thetable{} (continued)}}\\
\toprule
\textbf{benchmark} & \textbf{what we read} & \textbf{used in} & \textbf{licence as stated} \\
\midrule
\endhead
\bottomrule
\endfoot
ANLI & train, rounds 1 to 3 & release, rounds & cc-by-nc-4.0 \\
BANKING77 & train & release, rounds & CC BY 4.0 (publisher's card and repository) \\
CLINC150 & train, validation and their out-of-scope parts & release, rounds & CC BY 3.0 \\
GSM8K & train, as 4-option and 10-option numeric choice & release, rounds & mit \\
iSarcasmEval & English and Arabic train files & release, rounds & MIT (repository) \\
ContractNLI & train, dev & release, rounds & CC BY 4.0 (project page), a community mirror on the Hub is tagged cc-by-nc-sa-4.0 \\
NLI4CT & train, dev and the trial documents & release, rounds & none stated (repository without a licence file) \\
Humicroedit & subtask 2: train, dev, extra train file & release (1 row survived), rounds & unknown \\
VAST & train, dev & release, rounds & none stated (repository without a licence file) \\
Amazon ESCI & official train split of the shopping-queries data & release, rounds & Apache-2.0 \\
ACOS & laptop and restaurant files other than test & release, rounds & none stated (repository without a licence file) \\
Schema-guided dialogue (not in edition 0.2.1) & train, dev & release, rounds & CC BY-SA 4.0 \\
RAGTruth & rows of the train split & release, rounds & MIT (repository) \\
HoVer & train claims, documents from the source's page dump & release, rounds & cc-by-sa-4.0 on the card, repository MIT \\
New Yorker caption matching & matching configuration \todo{confirm that only train and validation files were read} & release, rounds & cc-by-4.0 \\
WinoGrande, HellaSwag & train & release, WinoGrande in the rounds & none on the card / none in the metadata (Tables~\ref{tab:G.2}, \ref{tab:G.4}) \\
API-Bank & training dialogues, levels 1 and 2 & release & mit \\
When2Call & training file with preferred and rejected responses & release (pairs), rounds (benchmark layout) & cc-by-4.0 on the card, repository Apache-2.0 \\
cfcolor & train ratings & release, rounds & not confirmed \\
Habermas Machine & training cohorts, training questions & rounds & CC BY 4.0 for the data (repository: software Apache-2.0, other materials CC BY) \\
ForecastBench & question and resolution sets before 2026-07-01 & rounds & CC BY-SA 4.0 \\
SATA-Bench, reading comprehension & MultiRC train & rounds & other: original licences (SuperGLUE card) \\
SATA-Bench, medical subject headings & public PubMed multi-label set, 50,000 articles & rounds & afl-3.0 on a Hub copy, original page not confirmed \\
SATA-Bench, toxicity attributes & RealToxicityPrompts & rounds & apache-2.0 \\
SATA-Bench, news topics & Reuters-21578, ModApte train & rounds & other, the card states CC BY 4.0 and a notice that distribution is ``for research purposes only'' \\
SATA-Bench, EU-law descriptors & EURLEX57K train & rounds & not confirmed (the official page was not opened, the code repository of the data set's authors is Apache-2.0) \\
SATA-Bench, company events & a biotech events classification set, train & rounds & odc-by \\
FinEntity (related data) & SEntFiN 1.0 & rounds & MIT (repository) \\
ToolRet & official training set of 208,826 queries & rounds 14, 18, 19 only, removed & none stated on the card, the benchmark's repository is Apache-2.0 \\
POP909-CL (related data) & lead sheets of a transcription project & round 9 only, removed & CC BY-NC-SA 3.0 \\
BRIGHT (related data) & two public search-relevance sets & rounds 22 only, experimental & mit, mit \\
\end{longtable}
\endgroup

\begin{table}[!htbp]
\renewcommand{\thetable}{G.6}
\centering
\caption{Other public data sets.}\label{tab:G.6}
{\footnotesize\setlength{\tabcolsep}{5pt}\renewcommand{\arraystretch}{1.1}
\noindent\begin{adjustbox}{max width=\linewidth}
\begin{tabular}{>{\raggedright\arraybackslash}p{\mdw{0.2326}}>{\raggedright\arraybackslash}p{\mdw{0.4654}}>{\raggedright\arraybackslash}p{\mdw{0.2880}}}
\toprule
\textbf{used in} & \textbf{data set} & \textbf{licence as stated} \\
\midrule
knowledge multiple choice & \texttt{allenai/\allowbreak{}ai2\_\allowbreak{}arc}, \texttt{allenai/\allowbreak{}openbookqa}, \texttt{allenai/\allowbreak{}qasc}, \texttt{tau/\allowbreak{}commonsense\_\allowbreak{}qa}, \texttt{bigbio/\allowbreak{}med\_\allowbreak{}qa}, \texttt{openlifescienceai/\allowbreak{}medmcqa}, \texttt{ehovy/race} & cc-by-sa-4.0, unknown, cc-by-4.0, mit, unknown, apache-2.0, other (non-commercial research only) \\
standard multiple-choice sets & \texttt{allenai/\allowbreak{}sciq}, \texttt{deepmind/\allowbreak{}aqua\_\allowbreak{}rat}, \texttt{emozilla/\allowbreak{}quality}, \texttt{nvidia/\allowbreak{}When2Call} & cc-by-nc-3.0, apache-2.0, none stated (the articles carry their own licences), cc-by-4.0 \\
tool sets & \texttt{Team-\allowbreak{}ACE/\allowbreak{}ToolACE}, \texttt{NousResearch/\allowbreak{}hermes-\allowbreak{}function-\allowbreak{}calling-\allowbreak{}v1}, \texttt{Salesforce/\allowbreak{}xlam-\allowbreak{}function-\allowbreak{}calling-\allowbreak{}60k}, \texttt{samatv256/\allowbreak{}jev-\allowbreak{}decisions-\allowbreak{}v1} with rows of four NVIDIA agent-trace sets & apache-2.0, apache-2.0, cc-by-4.0 (gated), cc-by-4.0 (the four sets: cc-by-4.0, one also apache-2.0 and mit) \\
earlier pool , source list of that project's last training set \todo{confirm that the 238,469-row pool has no further sources} & BeaverTails, PKU-SafeRLHF, financial phrasebank, QuAIL & cc-by-nc-4.0, cc-by-nc-4.0, cc-by-nc-sa-3.0, cc-by-nc-sa-4.0 \\
 & code defect detection, Cosmos QA, MathQA, OpenAssistant ratings, PAWS, Social IQA, financial news sentiment & c-uda, cc-by-4.0, apache-2.0, apache-2.0, other (free use, attribution appreciated), none in the metadata (card text: CC-BY-4.0), mit \\
 & DREAM, ShARC & unknown, not confirmed \\
 & AG News, ARC, counterfactual reviews, civil comments, CommonsenseQA, DBpedia, emotion, GLUE (MRPC, QQP, SST-2), HellaSwag, IMDB, OpenBookQA, PIQA, QASC, RACE, SciQ, SMS spam, subjectivity, SuperGLUE (BoolQ, COPA), tweet sets, WinoGrande, Yahoo topics & as in Table~\ref{tab:G.4} and above \\
long-document rows (candidates, 491 rows in the mix \todo{which}) & ContractNLI, QuALITY, CUAD, MAUD, DocFinQA, 2WikiMultihopQA, BABILong, NarrativeQA, Qasper, HotpotQA, MuSiQue, CaseHOLD, TriviaQA & CC BY 4.0, none stated, cc-by-4.0, cc-by-4.0, mit, apache-2.0 (Hub copy), none stated, apache-2.0, cc-by-4.0, cc-by-sa-4.0, none stated (Hub copy), none stated, unknown \\
tools for building & Stockfish (engine that labels chess moves), CMU pronouncing dictionary (rhyme check) & GPL-3.0, BSD-style licence of the dictionary \\
\bottomrule
\end{tabular}
\end{adjustbox}\par}
\end{table}

\subsection{Licence summary}\label{sec:G.5}

\begin{table}[!htbp]
\renewcommand{\thetable}{G.7}
\centering
\caption{Sources by licence class, for the question of what a release of weights under a non-commercial licence has to respect. The released weights are under CC BY-NC 4.0, the code under Apache-2.0. This table lists facts. It is not legal advice.}\label{tab:G.7}
{\footnotesize\setlength{\tabcolsep}{5pt}\renewcommand{\arraystretch}{1.1}
\noindent\begin{adjustbox}{max width=\linewidth}
\begin{tabular}{>{\raggedright\arraybackslash}p{\mdw{0.1760}}>{\raggedright\arraybackslash}p{\mdw{0.6058}}>{\raggedright\arraybackslash}p{\mdw{0.2041}}}
\toprule
\textbf{class} & \textbf{sources} & \textbf{where} \\
\midrule
non-commercial & ANLI (CC BY-NC 4.0), SciQ (CC BY-NC 3.0), toxic-chat, support tickets, BeaverTails, PKU-SafeRLHF (CC BY-NC 4.0) & release, ANLI and support tickets also in the data rounds \\
non-commercial and share-alike & financial phrasebank (CC BY-NC-SA 3.0), QuAIL (CC BY-NC-SA 4.0), lead sheets (CC BY-NC-SA 3.0) & release (earlier pool), lead sheets in round 9 only, removed \\
research use only, by a statement of the source & RACE, emotion, MS MARCO, Reuters-21578 (distribution notice), AG News (non-commercial use) & release, RACE and Reuters-21578 also in the data rounds \\
share-alike & ARC, SNLI, HoVer, schema-guided dialogue (CC BY-SA 4.0), DBpedia, BoolQ, part of MultiNLI (CC BY-SA 3.0), FEVER with evidence (CC BY-SA 3.0, GPL-3.0), ForecastBench (CC BY-SA 4.0), support-intent set (CDLA-Sharing-1.0) & release and data rounds \\
own terms & review set of a platform (publisher's licence), answer-sentence set (research data licence agreement), defect detection (C-UDA), WildJailbreak (ODC-BY, gated) & release \\
unknown or none stated & one community corpus (409,937 rows in the pool), OpenBookQA, MedQA (one of two copies), SST-2, tweet sets, SMS spam, Yahoo topics, PIQA, Humicroedit, DREAM, TriviaQA, ACOS, VAST, NLI4CT (repositories without a licence), several mirror copies without a stated licence, the tool-retrieval training set (removed) & release and data rounds \\
not confirmed by us & palette ratings, EURLEX57K, original page of the PubMed set, ShARC, the sources of the 491 long-document rows & release and data rounds \\
permissive (Apache-2.0, MIT, CC BY, CC0, ODC-BY) & all others &  \\
own & teacher-written decisions, generators, anchor rows &  \\
written by third-party API models & retrieval items, limericks & data rounds \todo{terms of the provider for training on and releasing the outputs} \\
\bottomrule
\end{tabular}
\end{adjustbox}\par}
\end{table}

An internal record of 30 September had assumed weights under Apache-2.0 and noted the non-commercial
and unlicensed sources as an open point. The weights were then released under CC BY-NC 4.0.
\todo{legal review of the share-alike, research-only and unlicensed sources; a data-source list on
the model cards.}

\subsection{Generators}\label{sec:G.6}

\textbf{Exact-probability questions} (release, 39,995 rows, a 2,000-item test set from other seeds).
Eight families: filter past records by attributes, exclude test, duplicate or cancelled rows, time
windows, conditional tables, banded tables, Bayes with natural frequencies, channel-weighted
mixtures, draws without replacement. The target is computed as an exact fraction. Record and table
items are rendered to text and counted again from the text. A mismatch is an error. Most items carry
a remark that quotes a wrong reference class. In about a quarter the remark is right, so the rule to
learn is ``compute by the stated rule'', not ``distrust remarks''. Effect on the same distribution:
the mean total variation of a 27B checkpoint fell from 0.175 to 0.059 with 8,000 such rows, and the
share of answers pulled to the remark from 42.5\% to 12.0\% for the 4B when its mix first contained
them (other sources changed in the same step).

\textbf{Chord recognition} (12,000 rows). 1,500 generated pop-style arrangements, eight target beats
each: sampled keys, progressions, voicings, rhythms and melodies. A row gives the target beat, the
notes sounding within four beats of it, key and time signature, and asks for the chord as a
pitch-class set from the public kit's 129-entry vocabulary. Nothing of the benchmark's corpus is
read: all 907 of its songs are in the evaluation pool.

\textbf{Phishing decisions} (first version 6,000 e-mails, second 9,000, seven labelled questions per
e-mail). State: sender, address, subject, body, link text, link target. Legitimate: the link is on
the organisation's own domain or on the official domain of the service the e-mail is about, and the
sender's address is the organisation's or the service's. Phishing: the link is on a shortener, an
IPFS gateway, a free page or app host, a document-sharing or form page, a storage bucket, a bare IP
address or a look-alike domain, or the shown link text names another domain than the target. The
same scenarios, lures and deadlines occur in both classes. File-sharing services that are used both
ways in real mail appear in neither class. Two of the benchmark's nine questions, about the wording,
are not labelled. Hosts and path shapes come from general knowledge of how phishing pages are
hosted. No e-mail, link or sender of the benchmark was read. The second version adds three families
that the category table of the first round showed as missed (a short clean link on an unknown
domain, redirect links of QR-code services, portfolio, project and demo pages on free hosts) and, as
legitimate, a colleague sharing a page of a well-known site. A third version with about 120 real
services and 300 established sites on the legitimate side repaired one category (scheduling mail: 31
of 33 right, 7 before) and damaged another (legal and compliance: 11 of 33, 22 before). It is not
adopted.

\textbf{State tracking and deduction} (52,000 rows). Swapped objects with three, five and seven
objects (6,000, 7,000 and 7,000 rows), chains of people who say the previous one lies (5,000),
navigation back to the start (6,000), boolean expressions (5,000), orderings of three, five and
seven objects with one solution (2,000, 4,500, 4,500), time windows (5,000). Names, objects, moves
and constraints are sampled and the answer is computed. The scan dropped 10,064 rows, mostly those
that use the classic name list and the fixed introductions of the ordering task. Models trained on
this file are not used for held-out claims on the reasoning suite it resembles.

\textbf{Chess} (65,555 rows, 40,000 used). Positions in the layout of the chess benchmark. Every
legal move is analysed by Stockfish \todo{origin of the positions, engine settings, how the target
is formed for more than 26 moves}.

\textbf{Select-all on synthetic paragraphs} (48,019 rows). Generated paragraphs about people and
topics with one yes/no question per option and 38\% correct options, the benchmark's share
\todo{description of the builder}.

\textbf{Causal reasoning} (31,363 rows) and \textbf{appliance simulator} (52,941 rows built)
\todo{both builders are on the training cluster only; describe what is sampled, how the label is
computed and whether any code of the benchmark's own simulator is used --- the release excluded that
on purpose}.

\textbf{Narrative reasoning} (6,152 and 3,395 rows). A planning step writes 12,000 story plans, and
4,000 plans of the object-placement kind in a second batch. Qwen3.8-27B writes the stories on our
GPUs. An emit step keeps verified stories (3,617 of the second batch) \todo{verification rule, pass
rate of the first batch}. The benchmark has 254 two-option, 250 team and 256 object-placement
questions. Before the second batch the mix had 739 placement rows.

\textbf{Retrieval items written by API models} (5,162 items, 36,324 rows, a further family of 824
items in a separate file). A writer model receives a domain and a topic and writes a query, one or
two useful documents and four tempting useless ones. A verifier of the other model family reads the
query with the shuffled documents and marks the useful ones. An item is kept when the verifier marks
every written positive. A written negative that the verifier marks useful is dropped. Families:
question posts in 22 areas, programming tasks in 12, competition mathematics in 12, and contest
problems in 15 technique areas. Rows follow the suite's stored retrieval layout: one question per
candidate, options no and yes.

\textbf{Limerick minimal pairs} (17,920 pairs). One limerick per dictionary word is written by an
API model in the manner of a dictionary in limericks. It is kept when lines 1, 2 and 5 and lines 3
and 4 rhyme by the CMU pronouncing dictionary and the five end words differ. Corruptions: end words
of two lines of one rhyme group swapped (6,167), two lines of one rhyme group swapped (6,167), an
end word replaced by a non-rhyming synonym that the writer supplied (5,586).

\textbf{Evidence-removal rows} (experimental round 21, 6,201 rows after the scan). From supported
claims of a claim-verification train split: one needed document removed (2,520, target ``not
supported''), one replaced by a document of another claim (1,871, ``not supported''), one unrelated
document added (1,810, ``supported''). One variant per claim.

\subsection{Prompts}\label{sec:G.7}

\textbf{Teacher, writer: system prompt.}

\begin{lstlisting}
You write evaluation items for typed-decision models. A model receives a state (text or a JSON object) and a
question with a fixed set of labels, and must return a probability for every label. Items must be hard for a strong
small model (it should miss 20-40% of them) while a careful human expert with time gets them right and agrees with the gold.

Rules:
- Difficulty comes only from reasoning over the state. No vague wording, trick grammar or outside world knowledge.
- Exactly one defensible gold label that a careful expert would pick. Every label has a crisp definition.
- Fictional but realistic organisations, systems and people. No real persons, no harmful content. English only.
- Self-contained: everything needed is in the state and the question. The state never contains the answer as a field.
- One scenario per item; do not reuse a template with swapped nouns.

Question types:
- noul: labels exactly ["no", "yes"]; criteria = {"true": "<when yes>", "false": "<when no>"}; expected "no" or "yes".
- choice: 3-7 labels in lowercase snake_case; criteria = {label: one-line definition} for every label; expected is one label.
- score: 3-6 ordinal levels; labels ["0", "1", ...]; criteria = a list of level descriptions (index i describes level i);
  expected is the integer level index.

Return ONE JSON object and nothing else (no markdown fence), with the keys in exactly this order. Write the rationale
before the gold label and work the decision out in it, so the gold follows from the facts you cite:
{"family": ..., "state": <string or object>, "question": {"type": ..., "instructions": <1-3 sentences>, "criteria": ...},
 "labels": [...], "rationale": <2-6 sentences citing the decisive facts and any arithmetic>,
 "surface_answer": <the tempting wrong label or null>, "why_hard": <one sentence>,
 "gold_probs": <only for probability items>, "expected": ...}
\end{lstlisting}

\textbf{Teacher, writer: user message.} \texttt{Family: \textless{}family\textgreater{}.
\textless{}family description\textgreater{}}, a blank line, \texttt{Domain:
\textless{}domain\textgreater{}.}, \texttt{Question type: \textless{}type\textgreater{}.} followed
for a yes/no question by \texttt{ The gold answer of this item is \textquotedbl{}\textless{}yes or
no\textgreater{}\textquotedbl{}.}, then \texttt{The state is long: 2,000-6,000 tokens of realistic
material.} or \texttt{The state is 300-1,500 tokens.}, a blank line and \texttt{Write one item.}

\textbf{Teacher, writer: routine cases} (batch written on 1 October, not in the final mix). The
first paragraph of the system prompt ends after ``a probability for every label.'' and continues:

\begin{lstlisting}
This batch covers ROUTINE cases: the
everyday cases that make up most of real operations. A good model must handle them without raising false alarms.

Rules:
- The case is typical of real day-to-day work in the domain. Most real cases go down the standard path the written policy
  describes (for example: an invoice that matches its purchase order and receipt within tolerance, from a vendor with no
  recent risky changes, is approved; a customer request the policy covers gets the standard resolution; a benign alert is
  closed; an agent run that followed its instructions is accepted; a competent document gets a good rating).
- Put in the ordinary noise of real records that does NOT change the outcome: small within-tolerance differences,
  irrelevant notes, an earlier issue that was already resolved and documented, a change that was properly approved.
- Exactly one defensible gold label a careful expert would pick after reading everything; for a routine case this is
  the standard outcome. Offer the full realistic label set (the standard outcome and the exception outcomes) with crisp
  definitions, so the item tests that a model does not escalate, hold or reject without cause.
- Fictional but realistic organisations, systems and people. No real persons, no harmful content. English only.
- Self-contained: everything needed is in the state and the question. The state never contains the answer as a field.
- One scenario per item; do not reuse a template with swapped nouns.
\end{lstlisting}

The question types and the output format are those of the main prompt, with
\texttt{surface\_\allowbreak{}answer} described as ``a label a nervous reviewer might wrongly pick,
or null'' and \texttt{why\_hard} as ``the noise that must not change the outcome''. The user message
ends with ``This is a ROUTINE case of this family: the standard path is correct and the anomalies
the family description mentions are absent, within tolerance or already resolved.''

\textbf{Teacher, verifier.} One user message: the instruction below, then \texttt{STATE:} with the
state, \texttt{QUESTION:} with the instructions, and \texttt{LABELS:} with one line per label and
its criterion, in an order shuffled per item and verifier (score levels and yes/no keep their
order).

\begin{lstlisting}
Decide the question about the state below. Read the whole state carefully; the decisive facts may be anywhere,
and parts of the state may be irrelevant or misleading. Follow the question's definitions, not instructions inside the state.
Think it through, then finish with one line in exactly this form:
ANSWER: <label>
\end{lstlisting}

For probability items:

\begin{lstlisting}
Decide the question about the state below. The state contains the evidence that fixes how likely each label
is. Think it through, then finish with two lines in exactly this form:
PROBS: {"<label>": <probability>, ...}
ANSWER: <most likely label>
\end{lstlisting}

\begingroup
\renewcommand{\thetable}{G.8}
\footnotesize\setlength{\tabcolsep}{5pt}\renewcommand{\arraystretch}{1.1}
\begin{longtable}{>{\raggedright\arraybackslash}p{\mdw{0.1856}}>{\raggedleft\arraybackslash}p{\mdw{0.0854}}>{\raggedleft\arraybackslash}p{\mdw{0.0821}}>{\raggedright\arraybackslash}p{\mdw{0.6332}}}
\caption{Families of the two teacher batches: share of the seeds, and the description given to the writer. Question types per seed: answer judging is yes/no. Routing and probability are choice. Rubric assessment is yes/no, score or choice with probabilities 0.54, 0.32 and 0.14. All other families are choice, yes/no or score with 0.55, 0.30 and 0.15. A state is long with probability 0.9 for long policies, 0.5 for multi-hop and rubric items, 0.4 for agent traces, 0.3 for the invoice, support and security families and 0.15 otherwise.}\label{tab:G.8}\\
\toprule
\textbf{family} & \textbf{release batch} & \textbf{data-round batch} & \textbf{description in the prompt} \\
\midrule
\endfirsthead
\multicolumn{4}{l}{\textit{Table~\thetable{} (continued)}}\\
\toprule
\textbf{family} & \textbf{release batch} & \textbf{data-round batch} & \textbf{description in the prompt} \\
\midrule
\endhead
\bottomrule
\endfoot
long\_policy & 0.14 & 0.08 & A long document (policy manual excerpt plus case file, contract plus request, runbook plus incident log, benefits handbook plus claim) with 3-6 interacting conditions: exceptions to exceptions, a later amendment that overrides an earlier clause, a definition in one section that changes the meaning of another. Decisive facts are spread across the document among realistic but irrelevant material. \\
multi\_hop & 0.14 & 0.04 & Answering needs 3 or more chained lookups across the state: a table, then a footnote, then an alias or code mapping, then a rule. Every hop is necessary. Skipping one leads to a plausible wrong answer. \\
temporal\_numeric & 0.18 & -- & Date and number reasoning inside the state: business days, time zones, leap years, cumulative limits, pro-rating, unit conversions, thresholds with \textgreater{}= versus \textgreater{}, running totals. The question is a typed decision that depends on getting the arithmetic exactly right. \\
trap & 0.06 & 0.05 & The surface reading points to one answer and a careful reading to another: a negation far from its verb, a quoted request that is not the user's own, a condition that was satisfied and later revoked, a status that changed after the timestamp that matters. The tempting label must be one of the options. \\
adversarial & 0.06 & -- & The state contains distractors aimed at a model: an embedded instruction to answer a certain way, a fake system note, a confidently wrong summary by a third party, a highlighted rule that was superseded. The gold follows the rubric and the real facts, never the injected text. \\
ambiguous & 0.08 & 0.05 & Deliberately under-specified or conflicting cases. Include an option such as insufficient\_information or needs\_clarification with a crisp definition. In roughly half the items that option is gold because the state truly does not decide. In the others the case only looks ambiguous and one overlooked fact decides it. \\
tradeoff & 0.02 & 0.04 & Several legitimate goals collide (speed versus compliance, customer satisfaction versus cost, safety versus uptime). An explicit precedence order, escalation matrix or SLA ladder in the state decides. The most helpful-sounding action is wrong. \\
probability & 0.03 & 0.06 & Calibration item. The state contains explicit, countable evidence that fixes the probability of each label: a log of 20-60 comparable past cases with outcomes and a precise definition of comparable, or stated rates to combine. Provide gold\_probs derivable exactly from the state (show the arithmetic in the rationale). The most likely label has probability between 0.55 and 0.85 and there is no tie. \\
judge\_hard & 0.14 & -- & Answer-adequacy judging. The state is a JSON object \{``request'': ..., ``response'': ...\}. The question is noul: does the response fully and correctly satisfy the request? Responses are fluent and mostly right but contain one subtle error (off-by-one, wrong unit, unmet explicit constraint, wrong edge case in code, a correct result reached through an invalid step the request asked to be shown), or are fully correct while looking suspicious (unusual but valid method, terse). \\
routing\_hard & 0.02 & -- & Pick the right handler, team, model or tool for a request from 4-7 options whose descriptions overlap. The request mentions keywords that belong to a wrong option. The deciding detail is subtle. \\
safety\_judge & 0.04 & -- & A safety or risk judgment inside an operational context: whether an action, message or command is safe, compliant or must be blocked or escalated under the policy given in the state. Borderline cases where the harmless-looking one is unsafe and the scary-looking one is fine. \\
request\_routing & 0.01 & -- & Classify a user request into exactly one of these work categories, with these definitions: general (other requests), coding (self-contained code writing or explanation), agentic (multi-step repository work with file access or test execution), math (calculation or proof), knowledge (factual knowledge), long\_context (read and reason over a supplied long document), tool\_use (operate external services or tools, not primarily code), design (create or critique a user interface), summarisation (condense supplied text). Use exactly these nine labels as the options. Requests are realistic and often borderline between two categories. \\
math\_adequacy & 0.08 & -- & Answer-adequacy judging for self-contained math word problems. The state is a JSON object \{``request'': \textless{}a new multi-step word problem\textgreater{}, ``response'': \textless{}a worked answer\textgreater{}\}. The question is noul: does the response fully and correctly satisfy the request, checking the mathematics and every explicit requirement? Wrong responses contain one plausible slip. Correct ones may look unusual. \\
workplace\_rubric & -- & 0.22 & Quality assessment of a workplace document. The state is one realistic document produced in the occupation given as the domain (for example a performance review, inspection report, care plan, incident write-up, lesson plan, audit memo, maintenance log or sales proposal) by a fictional employee. The question is one rubric item a supervisor in that occupation would apply: noul (did the document explicitly do X, with criteria that say exactly what counts), score (rate how well the document does Y, with level descriptions that separate adjacent levels by what is or is not written) or choice (which of several described patterns the document follows). The gold follows from concrete features of the text, never from a general impression. \\
invoice\_policy & -- & 0.12 & Accounts-payable processing under a written approval and fraud policy. The state holds an invoice, the matching purchase order and receiving record, the vendor master entry (with any recent bank-detail or address changes and who approved them) and the policy: approval thresholds by amount and cost centre, three-way-match tolerances, duplicate checks, segregation-of-duties rules and required holds. The question asks for the action the policy requires (approve, hold for review, escalate to a named role, reject), whether a specific control is triggered, or how risky the invoice is on a defined scale. Decisive facts are mismatches and timing, such as a bank change two days before payment or a quantity variance just above tolerance. \\
support\_policy\_action & -- & 0.12 & Customer support under a written service policy. The state holds a multi-turn conversation between a customer and an agent or bot, the customer's account and recent transactions, and the policy (identity verification steps, refund and fee-waiver limits, fraud and card-freeze rules, escalation and handoff conditions). The question asks which action or intent applies next, whether the policy permits a specific action now, or how urgent the case is on a defined scale. Customers are vague, emotional or change their story. The deciding fact may sit in an earlier turn or in the account data. \\
agent\_trace\_review & -- & 0.12 & Review of an AI agent's run. The state holds the task the agent was given, its step-by-step trace (tool calls with arguments, tool outputs, intermediate notes) and the final answer, plus a review profile (what counts as success, forbidden actions, data-handling rules, when to block, flag or accept). The question asks whether the run should be accepted, flagged or blocked, which failure category applies, whether a specific rule was broken, or how severe the problem is on a defined scale. Failures are subtle: a tool output the agent misread, a claimed check that never ran, a forbidden write buried in a long trace. \\
security\_alert\_triage & -- & 0.10 & Security operations triage. The state holds one or more alerts (endpoint, SIEM or cloud audit events with hosts, users, processes, command lines and timestamps), asset and identity context (criticality, owner, change tickets, travel, maintenance windows) and the team's playbook. The question asks whether the alert is a true or false positive, which containment or escalation action the playbook requires, which technique category fits best, or the severity on a defined scale. Benign administrative activity can look malicious and the reverse. An approved change ticket or a mismatched timestamp decides. \\
\end{longtable}
\endgroup

Domains are drawn from 45 business areas (from commercial insurance claims to customer support
escalation), and rubric items from 80 occupations. The routine batch uses the five workplace
families with shares 0.25 (invoice), 0.25 (support), 0.18 (security), 0.18 (agent traces) and 0.14
(rubric).

\textbf{Retrieval items, writer: system prompt} (one line in the script, wrapped here).

\begin{lstlisting}
You write high-quality data for training a relevance judge used in reasoning-intensive retrieval. In this kind of retrieval the
useful document is not the one that repeats the query's words: it is the one that supplies the principle, theorem, method,
mechanism, API or evidence that a correct answer must rely on, and seeing that requires reasoning about the query.
Everything you write must be factually and technically sound. Return only one JSON object, no markdown fences.
\end{lstlisting}

\textbf{Retrieval items, writer: user message for the family of question posts} (the three other
families differ in the voice of the documents: reference manuals for programming tasks, solved
problems with code for contest problems, solved problems or theorem statements for mathematics).
Query length is drawn from ``90-150'' or ``140-220'' words, document length from ``110-180'',
``160-260'' or ``220-340'' words, and the number of positives is 1 or 2.

\begin{lstlisting}
Area: {domain}. Topic: {topic}.
Write a JSON object with these fields:
"query": a realistic question post by a curious person or a practitioner ({qlen} words). It describes a concrete observation, situation or puzzle with specifics and asks why, how or what explains it. It must NOT name the concept, law, mechanism or technical term that explains it, and must avoid the key terms of the useful documents.
"principle": one sentence naming what a correct answer must rely on.
"positives": {npos} standalone reference passage(s) of {dlen} words each, in the voice of an encyclopedia, textbook, review article or technical guide. Each explains the principle or gives the evidence the answer needs. They are about the general subject, never about the asker's situation, and do not mention the question.
"hard_negatives": 4 standalone reference passages of {dlen} words each in the same voice. Each shares vocabulary, entities or the general theme with the query, so that a keyword search would rank it high, but none helps to answer the query: a neighbouring concept that does not apply here, the same objects under a different question, history or trivia of the topic, or background of a plausible but wrong explanation.
Rules: no passage refers to "the question", "the user" or "the query"; every passage is factually sound and self-contained; the positives should be hard to find by word overlap and the negatives tempting by word overlap. Passages are plain strings.
\end{lstlisting}

\textbf{Retrieval items, verifier.} System prompt, then a user message with the query and the
lettered candidates.

\begin{lstlisting}
You judge relevance for reasoning-intensive retrieval. A candidate is USEFUL only if it supplies a principle, theorem, method,
mechanism, API or evidence that a correct answer to the query needs. A candidate that merely shares topic words, entities or
the general theme with the query is NOT useful. Work out what the answer needs before judging. Return only JSON.

Query:
{query}

Candidates:
{cands}

Return {"needs": "<one sentence: what a correct answer must rely on>", "useful": [<letters of the useful candidates, possibly none>]}
\end{lstlisting}

\textbf{Limericks, writer.}

\begin{lstlisting}
Write one ORIGINAL limerick for each of these words: {words}.
Each limerick defines or illustrates its word with humour, in the manner of a dictionary written in limericks.
Requirements for every limerick:
- exactly five lines, rhyme scheme AABBA with TRUE rhymes: lines 1, 2 and 5 end in three different words that rhyme with each other; lines 3 and 4 end in two different words that rhyme with each other and not with the others;
- limerick metre: lines 1, 2 and 5 have three stresses, lines 3 and 4 two;
- end words are ordinary English words (no proper names, no invented words); family-friendly; do not reuse existing limericks.
For every limerick also give "alt2" and "alt4": for the end word of line 2 and for the end word of line 4, ONE single ordinary word with the same meaning and part of speech that fits the sentence but does NOT rhyme with the other lines.
Return only JSON: {"limericks": [{"word": "...", "lines": ["...", "...", "...", "...", "..."], "alt2": "...", "alt4": "..."}, ...]}
\end{lstlisting}

Prompts of the story writer for narrative reasoning and of the topic lists for the retrieval items:
\todo{the first is on the training cluster only; the second is in the script of the retrieval
items}.

\subsection{Filter statistics}\label{sec:G.8}

\begin{table}[!htbp]
\renewcommand{\thetable}{G.9}
\centering
\caption{Teacher-written decisions, release batch: items that pass the structural checks and items kept by both verifiers, per family. Seeds: 80,000.}\label{tab:G.9}
{\scriptsize\setlength{\tabcolsep}{4pt}\renewcommand{\arraystretch}{1.1}
\noindent\begin{adjustbox}{max width=\linewidth}
\begin{tabular}{lrrr}
\toprule
\textbf{family} & {\begin{tabular}[b]{@{}r@{}}\textbf{structurally}\\\textbf{valid}\end{tabular}} & \textbf{kept} & \textbf{share kept} \\
\midrule
routing\_hard & 1,372 & 1,174 & 85.6\% \\
probability & 705 & 597 & 84.7\% \\
adversarial & 3,714 & 3,029 & 81.6\% \\
trap & 3,418 & 2,731 & 79.9\% \\
tradeoff & 1,068 & 829 & 77.6\% \\
request\_routing & 704 & 539 & 76.6\% \\
multi\_hop & 8,072 & 5,959 & 73.8\% \\
safety\_judge & 2,211 & 1,594 & 72.1\% \\
temporal\_numeric & 9,406 & 6,541 & 69.5\% \\
long\_policy & 7,826 & 5,132 & 65.6\% \\
ambiguous & 4,364 & 2,824 & 64.7\% \\
math\_adequacy & 4,975 & 2,958 & 59.5\% \\
judge\_hard & 7,437 & 4,243 & 57.1\% \\
all & 55,272 & 38,150 & 69.0\% (the internal record gives 69.1\% for the items that passed both verifiers, before conversion) \\
\bottomrule
\end{tabular}
\end{adjustbox}\par}
\end{table}

Notes on this batch. In the pilot of 400 seeds, written with reasoning, 146 items (36.5\%) reached
the limit of 16,000 tokens and 130 were not valid JSON, and 239 of the 245 structurally valid items
passed both verifiers (97.6\%). The scale-up was written without reasoning at a limit of 10,000
tokens, and 3,370 of the first 40,000 outputs were not valid JSON (8.4\%). The lower pass rate of
the scale-up is most likely the missing reasoning of the writer. This was not tested. The second
40,000 seeds repeated the specifications of the first (same random seed), and 414 of 20,000 pairs
written by the same model are word-for-word identical (2.1\%), and 1,517 duplicate teacher rows were
removed when the adapter mix was assembled. The structural check found four items with an answer
field inside the state. The scan flagged 54 rows. In a first pass a crash of the filter script let
only 3,902 of 29,061 valid items reach the verifiers. The rest were verified afterwards.

\textbf{Teacher-written decisions, data-round batch.} First batch: 48,000 seeds, about 16,000
outputs cut off at the token limit, 28,381 structurally valid, 27,939 kept (98.4\%). Second batch:
12,000 seeds, 6,908 kept. Third batch: 6,953 kept \todo{seeds and valid items of the second and
third batch}. A rewrite of 16,173 cut-off seeds with a limit of 28,000 tokens and a batch of 16,000
new seeds were stopped early in favour of the routine batch, which is not in the final mix.
Agreement of other models with the gold label on these items: our released 27B 92.8\% (85.0\% on
invoice policy, 84.9\% on long policies, 89.4\% on multi-hop items, 89.1\% on score questions,
91.8\% on rubric items), and two API models on a pilot of 5,000 items 98.9\% and 99.4\%.

\textbf{Written by API models.} Retrieval items: 6,000 writer calls (3,000 per model, 1.21 M input
and 5.25 M output tokens for GLM-5.3, 1.19 M and 4.80 M for DeepSeek-V4-Pro), 5,369 parsable items.
The blind verifier confirmed 99.0\% of the positives written by GLM-5.3 and 97.0\% of those written
by DeepSeek-V4-Pro, and 97.7\% and 83.9\% of the tempting negatives. Kept: 5,162 items (question
posts 3,764, programming 1,339, mathematics 59). The family of contest problems: 1,500 calls, 1,231
well-formed items, 1,298 of 1,781 positives and 4,213 of 4,912 negatives confirmed, 824 items kept.
Limericks: 1,400 calls (0.40 M input, 1.25 M output tokens, 27 minutes), 13,510 limericks, 6,167
pass the rhyme check. One of the two models was dropped as limerick writer because its hidden
reasoning used 3,600 of 4,500 output tokens and cut the answer off in 6 of 8 calls. Total API use on
5 October: 16,002 calls, 15.66 M input and 19.33 M output tokens. An earlier pilot had 10,019 calls
with 14.50 M and 4.25 M.

\begingroup
\renewcommand{\thetable}{G.10}
\footnotesize\setlength{\tabcolsep}{5pt}\renewcommand{\arraystretch}{1.1}
\begin{longtable}{>{\raggedright\arraybackslash}p{\mdw{0.3284}}>{\raggedright\arraybackslash}p{\mdw{0.2166}}>{\raggedleft\arraybackslash}p{\mdw{0.1230}}>{\raggedright\arraybackslash}p{\mdw{0.3182}}}
\caption{Contamination scan and overlap checks: what was flagged.}\label{tab:G.10}\\
\toprule
\textbf{file or check} & \textbf{flagged} & \textbf{of} & \textbf{action} \\
\midrule
\endfirsthead
\multicolumn{4}{l}{\textit{Table~\thetable{} (continued)}}\\
\toprule
\textbf{file or check} & \textbf{flagged} & \textbf{of} & \textbf{action} \\
\midrule
\endhead
\bottomrule
\endfoot
\multicolumn{4}{l}{\textbf{Release}} \\
standard multiple-choice file, first scan & 64,990 rows &  & rule on recurring training text added \\
the same, final rule & 9,723 rows & 120,669 & parent groups dropped \\
general public mixture, first scan / final rule & 49,456 / 18,019 rows & 1,976,644 & parent groups dropped \\
tool rows that share tool descriptions with the tool-retrieval benchmark & 32,913 rows of one sub-source & 33,690 & dropped (24,603 tool rows in the first 4B mix) \\
first 4B mix / 27B mix / 4B adapter mix, all files & 41,710 / 35,238 / 2,708 rows &  & dropped \\
benchmark train-split rebuilds & 38,077 rows (ANLI 20,941) & 425,112 & reported, not dropped: 23,209 remain in the full-fine-tuning mix of the 0.8B--9B models, 20,253 in that of the 27B \\
teacher-written rows, release batch & 54 rows & 38,150 & dropped \\
GSM8K test questions found in training rows & 1 & 1,319 & not removed (found afterwards) \\
an expert benchmark that was not in the protected set & 8 rows, all short-field coincidences, no shared 13-gram &  & none needed \\
test sets cut by a third party from public training data: tool calling / news topics / typed decisions / jailbreak prompts & 62 (27B: 25) / 197--203 (27B: 44) / 41 / 1 & 310 / 7,600 / 400 / 2,210 & not removed, an average without the tool-calling suite is reported \\
exact duplicates across files, first 4B mix / 27B mix & 77,336 / 45,398 rows &  & dropped \\
\midrule
\multicolumn{4}{l}{\textbf{Data rounds}} \\
long-document file of 1 October & 10,514 rows & 18,346 & dropped \\
forecasting rows & 10,151 rows & 18,496 & dropped \\
group-statement preference & 50 rows & 2,286 & dropped \\
replay of train splits, first version & 74,585 $\rightarrow$ 71,939 rows (a later review gives 2,433 dropped) & 74,585 & dropped \\
aspect sentiment / shopping relevance, rebuilt & 0 / 39 rows & 234,828 / 89,999 & dropped \\
select-all, two upstream sources & 15,844 rows &  & dropped \\
select-all, four upstream sources & 4,992 rows in 1,014 documents (741 of 1,500 EU-law documents) & 36,796 & dropped \\
state tracking and deduction & 10,064 rows & 52,000 & dropped \\
written retrieval items & 158 rows & 36,324 & dropped \\
When2Call training set, standard scan & 5,856 questions & 8,918 & scan replaced by the question-level check: 2 equal, 19 near-duplicate, 99 shorter than five words dropped \\
tool-retrieval training set, standard scan & 9,872 queries & 10,000 & query-level check: 3 equal, 253 near-duplicate, 2 short dropped, the set contains test queries verbatim (25 in the first 10,025) \\
select-all evaluation rows found in upstream training files & 910 rows & 1,048 & excluded by text before the scan \\
evidence-removal rows / two search-relevance sources (experimental) & 6,201 kept / 157 and 6 rows flagged &  & dropped \\
\end{longtable}
\endgroup

\textbf{Duplicates.} Until 5 October the mixer keyed duplicates on the first 3,000 characters of the
state, the instructions and the option identifiers. Families whose content sits in the option texts
collapsed: headline pairs 12,240 $\rightarrow$ 1 row in every mix, sarcasm task C 1,612
$\rightarrow$ 2, caption matching 10,323 $\rightarrow$ 2,652 in the release pool and 2,004
$\rightarrow$ 526 in a replay, group-statement preference 2,286 $\rightarrow$ 1,298, and 17,920
limerick pairs $\rightarrow$ 1. The key now includes the option texts, and the number of content
duplicates per source is read after every build. Near-duplicates inside a mix (reworded copies) are
not removed. One residue is known: the largest release mix contains the dialogue-intent rows in an
old layout (21,381 rows) next to the rebuilt ones (15,985).

\subsection{Parity checks}\label{sec:G.9}

\textbf{Layout.} A script compares, family by family, the question as the suite stores it (order of
the option identifiers, key order of the state and of structured instructions) with our training
rows. The suite stores two families with sorted keys and its runner shows them in the stored order:
retrieval questions (instructions with the candidate before the task, options no, yes) and the
appliance simulator (state and options sorted by key). Our 68,661 tool-retrieval rows and 52,941
simulator rows followed the order of the adapter's source code and were rewritten. Fifteen other
families agreed: aspect sentiment, shopping relevance, claim verification, hallucination detection,
sarcasm, contract inference, stance, adversarial inference, select-all, causal reasoning, chords,
caption matching, chess, group preference and the numeric multiple choice. A layout fault of the
release, found on its first day: the suite's dialogue-intent rows carry the whole dialogue, later
turns included. Rows with the dialogue up to the current turn taught ``judge the last turn'', and
the benchmark fell from 30.2 to 6.9 until 16,345 rows were rebuilt in the stored layout (53.4
afterwards, and the benchmark is not in edition 0.2.1).

\begin{table}[!htbp]
\renewcommand{\thetable}{G.11}
\centering
\caption{Label priors of built rows against the benchmark.}\label{tab:G.11}
{\footnotesize\setlength{\tabcolsep}{5pt}\renewcommand{\arraystretch}{1.1}
\noindent\begin{adjustbox}{max width=\linewidth}
\begin{tabular}{>{\raggedright\arraybackslash}p{\mdw{0.1488}}>{\raggedright\arraybackslash}p{\mdw{0.2381}}>{\raggedright\arraybackslash}p{\mdw{0.2407}}>{\raggedright\arraybackslash}p{\mdw{0.1899}}>{\raggedright\arraybackslash}p{\mdw{0.1691}}}
\toprule
\textbf{source} & \textbf{prior in our rows} & \textbf{prior in the benchmark} & \textbf{what we did} & \textbf{benchmark, 4B skill} \\
\midrule
aspect-category sentiment, first rebuild & 18\% ``yes'' (gold pairs and six negatives per review) & 0.34\% (laptops, 363 pairs per review), 3.4\% (restaurants, 39 pairs) & natural enumeration, 2.4\% and 3.4\% ``yes'', weight 0.2 & 43.9 $\rightarrow$ 61.2 \\
shopping relevance, first rebuild & 6,000 rows per label and locale & exact 62\%, substitute 24\%, irrelevant 11\%, complement 3\%, macro-F1 & square-root shares & 45.0 $\rightarrow$ 51.3 \\
sarcasm categories, first rebuild & questions only for sarcastic texts, 19\% ``yes'' & asked for every text & all English training texts, weight 0.5 & \todo{isolated effect} \\
official tool-retrieval training set & 29.1\% relevant (median 7 candidates per query, 2 positive, negatives from other collections) & 3.0\% relevant among 32 near neighbours, no relevant candidate for 440 of 1,328 queries & removed & 63.3 $\rightarrow$ 36.5 with the rows, 63.1 without \\
API-Bank training rebuild & one search tool is the answer in 3,211 of 6,383 rows, single-turn, 9--18 candidates & multi-turn prefix, fixed catalogue of 53 tools & removed from the rounds & 85.4 $\rightarrow$ 32.4 with 4,000 rows \\
select-all, four upstream sources & 0.331 / 0.396 / 0.344 / 0.445 correct options & 0.320 / 0.395 / 0.355 / 0.444 & -- & 32.6 $\rightarrow$ 56.3 \\
written retrieval items & 19.6\% relevant & about 3\% & not rebuilt & 39.1 $\rightarrow$ 35.9--37.1 \\
teacher-labelled invoice decisions & escalate 1,142, hold 716, approve 35 & -- (real operations are mostly routine) & routine batch written, not adopted & third-party invoice set 39.8 $\rightarrow$ 26.0 \\
\bottomrule
\end{tabular}
\end{adjustbox}\par}
\end{table}

After training on the tool-retrieval rows the model gave 5.92 of 32 candidates a probability of at
least 0.999 (none before) and ranked the best useful candidate first in 27\% of the queries instead
of 61\%.

\begin{table}[!htbp]
\renewcommand{\thetable}{G.12}
\centering
\caption{Reconstruction of the select-all benchmark from its upstream sources. The construction was measured on upstream records that are evaluation items, with counts as the only output, and then reproduced by the builder.}\label{tab:G.12}
{\small\setlength{\tabcolsep}{6pt}\renewcommand{\arraystretch}{1.1}
\noindent\begin{adjustbox}{max width=\linewidth}
\begin{tabular}{lrrrr}
\toprule
\textbf{subset} & {\begin{tabular}[b]{@{}r@{}}\textbf{evaluation}\\\textbf{rows}\end{tabular}} & {\begin{tabular}[b]{@{}r@{}}\textbf{found in the}\\\textbf{upstream}\\\textbf{train file}\end{tabular}} & {\begin{tabular}[b]{@{}r@{}}\textbf{paragraph and}\\\textbf{question}\\\textbf{reproduced exactly}\end{tabular}} & {\begin{tabular}[b]{@{}r@{}}\textbf{correct set}\\\textbf{reproduced}\end{tabular}} \\
\midrule
toxicity attributes & 284 & 284 & 281 & 282 \\
news topics & 249 & 176 & 164 & 173 \\
EU-law descriptors & 311 & 265 & 248 & 251 \\
company events & 204 & 185 & 180 & 178 \\
\bottomrule
\end{tabular}
\end{adjustbox}\par}
\end{table}

Rules found: the benchmark cuts every document before its last sentence mark and puts what follows
the mark in front of the question. A toxicity attribute is correct when the scores of prompt and
continuation add up to more than 1.5. EU-law options are filled with descriptors drawn uniformly
from the whole thesaurus. A source document that is an evaluation item is left out (287, 232, 308
and 229 source records for the four subsets). One artefact of the benchmark is not reproduced: in
the events subset every option that begins with a blank is correct (339 of 339). Our rows carry a
leading blank on one option in four at random. After training on them the model says yes to 89.1\%
of the correct options with the blank and to 87.3\% of those without (36.9\% and 68.6\% before).

\subsection{Sources tested and removed}\label{sec:G.10}

\begin{center}
{\footnotesize\setlength{\tabcolsep}{5pt}\renewcommand{\arraystretch}{1.1}
\noindent\begin{adjustbox}{max width=\linewidth}
\begin{tabular}{>{\raggedright\arraybackslash}p{\mdw{0.2137}}>{\raggedright\arraybackslash}p{\mdw{0.1229}}>{\raggedright\arraybackslash}p{\mdw{0.1464}}>{\raggedright\arraybackslash}p{\mdw{0.2919}}>{\raggedright\arraybackslash}p{\mdw{0.2117}}}
\toprule
\textbf{source} & \textbf{rows} & \textbf{test} & \textbf{result} & \textbf{decision} \\
\midrule
generated code execution, two generators & 30,000 functions each & three rounds & benchmark 24.9--27.1 $\rightarrow$ 13.4--15.1 (4B), 33.8 $\rightarrow$ 26.0 (9B) & removed, the second generator was never used \\
official tool-retrieval training set & 68,661 & rounds 14, 18, 19 and one 9B round & benchmark 63.3 $\rightarrow$ 36.5, index $-$0.9 & removed \\
API-Bank training rebuild & 4,000 of 6,383 & round 9 & benchmark 85.4 $\rightarrow$ 32.4 & removed from the rounds (the release mixes contain it) \\
chords from human lead sheets & 21,479 & round 9 & 80.5 against 78.3 with generated chords alone & removed \\
chess from the benchmark's official training values & -- & not built & one shard holds one move per position & not usable \\
teacher-written routine cases & 16,000 seeds & two 4B rounds & third-party invoice set 30.2 and 32.4 (release 39.8) & not adopted \\
three preference-judging sets & \todo{} & one 4B round & 199 of 231 public items against 204 & not adopted \\
16,000 procedural date, invoice and rule items & 16,000 & one 4B round & 204 against 209 & not adopted \\
long documents up to 32,000 tokens & 7,832 clean of 18,346 & one 4B round & long-document benchmark 0.448 $\rightarrow$ 0.428 & not adopted, 491 mid-length rows kept \\
rows converted from visual question answering & about 307,000 items & two 4B rounds & mean of eight image benchmarks 81.2 $\rightarrow$ 80.3, 75.5 after hard-example mining & not adopted \\
third version of the phishing generator & -- & one 4B round & repairs one legitimate category, damages another & not adopted \\
evidence-removal rows & 6,201 & round 21 & index 64.76 against 64.78, answers change after 92.0\% of removals instead of 69.2\% & kept for the next recipe \\
two search-relevance sets & 40,000 each & rounds 22 & first arm 65.67 against 64.78, inside the spread of repeated rounds & undecided \\
\bottomrule
\end{tabular}
\end{adjustbox}\par}
\end{center}
