# Supplementary material for: StartLux-Decision: AutoThink Decision Models with Reinforcement Learning for Calibrated Deliberative Decisions
Source: arXiv:2610.17309 source file (2026-10-20)
Supplement: Supplementary file 15 [file appendix_H_evaluation.tex]

\clearpage
\section{Evaluation details}\label{sec:H}

\subsection{The index suite and settings common to all benchmarks}\label{sec:H.1}

All 38 benchmarks are answered with the prompt and the letter read-out of Section~\ref{sec:3.2}.
There is no benchmark-specific prompt, instruction or temperature. Lists of more than 26 options are
answered by the knock-out. This concerns intent classification with 77 and 151 labels, chords with
129 labels, tool selection among 53 tools and legal chess moves (27 to 43 options). The retrieval
benchmarks are stored as one yes/no question per candidate, with the options in the order ``no,
yes'' and about 3\% of the candidates relevant. The ranking is by the probability of yes. The kit
uses the probabilities in three places only: a yes/no answer counts as yes from 0.5, rankings use
the probability, and the forecasting benchmark is scored by its Brier score. Two families are stored
with sorted keys. We show every question in the stored layout.

\begingroup
\renewcommand{\thetable}{H.1}
\scriptsize\setlength{\tabcolsep}{4pt}\renewcommand{\arraystretch}{1.1}
\begin{longtable}{>{\raggedright\arraybackslash}p{\mdw{0.1418}}>{\raggedright\arraybackslash}p{\mdw{0.0503}}>{\raggedright\arraybackslash}p{\mdw{0.1253}}>{\raggedleft\arraybackslash}p{\mdw{0.0781}}>{\raggedleft\arraybackslash}p{\mdw{0.0905}}>{\raggedleft\arraybackslash}p{\mdw{0.0920}}>{\raggedright\arraybackslash}p{\mdw{0.1373}}>{\raggedright\arraybackslash}p{\mdw{0.1477}}>{\raggedright\arraybackslash}p{\mdw{0.1244}}}
\caption{The 38 benchmarks of Decision Index 0.2.1. $\bigstar$: weight 1.2 inside its area. Chance: the level the kit subtracts, read from a result file written by the kit (it does not depend on the system). Weight: computed from the edition's rule, area weight $\times$ benchmark weight / sum of benchmark weights of the area. Answers per run: questions answered in one of our runs (337,742 in all, in 133,876 requests). Training data aimed at the benchmark: T = official training split or training set of the benchmark's source. G = our generator or written data in the benchmark's request layout, containing nothing of the benchmark. R = related public data in the benchmark's layout. -- = nothing. Evaluation items were never trained on.}\label{tab:H.1}\\
\toprule
\textbf{benchmark} & \textbf{area} & \textbf{metric} & \textbf{chance} & \textbf{weight in the index} & \textbf{answers per run} & \textbf{training data aimed at it: released weights} & \textbf{after data rounds} & \textbf{\dag{} in the public README} \\
\midrule
\endfirsthead
\multicolumn{9}{l}{\textit{Table~\thetable{} (continued)}}\\
\toprule
\textbf{benchmark} & \textbf{area} & \textbf{metric} & \textbf{chance} & \textbf{weight in the index} & \textbf{answers per run} & \textbf{training data aimed at it: released weights} & \textbf{after data rounds} & \textbf{\dag{} in the public README} \\
\midrule
\endhead
\bottomrule
\endfoot
GSM8K \textsuperscript{d} & K & accuracy & 25.0\% & 2.39\% & 2,638 & T & T & \dag{} \\
ChessBench & K & accuracy & 8.2\% & 2.39\% & 5,000 & -- & G (own engine labels) &  \\
MuSR & K & accuracy & 37.1\% & 2.39\% & 756 & -- & G &  \\
SATA-Bench & K & case exact accuracy & 1.3\% & 2.39\% & 15,517 & -- & G, and T of its upstream sources &  \\
GPQA Diamond $\bigstar$ & K & accuracy & 25.0\% & 2.87\% & 198 & -- & -- &  \\
CRUXEval & K & accuracy & 37.0\% & 2.39\% & 570 & -- & -- &  \\
CLadder & K & accuracy & 50.0\% & 2.39\% & 5,000 & -- & G &  \\
HLE $\bigstar$ & K & accuracy & 16.4\% & 2.87\% & 513 & -- & -- &  \\
MMLU-Pro $\bigstar$ & K & accuracy & 11.1\% & 2.87\% & 12,032 & -- & -- &  \\
BBH, fixed-option tasks $\bigstar$ & K & accuracy & 31.0\% & 2.87\% & 5,507 & -- & G (from the eighteenth round on) &  \\
ContractNLI & L & macro-F1 & 30.9\% & 2.43\% & 2,091 & T & T & \dag{} \\
ANLI $\bigstar$ & L & macro-F1 & 33.2\% & 2.92\% & 3,200 & T & T & \dag{} \\
WinoGrande $\bigstar$ & L & accuracy & 50.0\% & 2.92\% & 1,267 & T (27B: full split, smaller sizes: a small sample) & T &  \\
HellaSwag $\bigstar$ & L & accuracy & 25.0\% & 2.92\% & 10,042 & T (27B: full split, smaller sizes: a small sample) & T &  \\
ACOS & L & per-review F1 & 3.1\% & 2.43\% & 91,092 & T & T (resampled) & \dag{} \\
FinEntity & L & macro-F1 & 32.0\% & 2.43\% & 2,129 & -- & R (another entity-sentiment corpus) &  \\
iSarcasmEval & L & sarcasm F1, track A, English & 22.3\% & 2.43\% & 11,600 \textsuperscript{c} & T & T & \dag{} \\
VAST & L & macro-F1 & 33.3\% & 2.43\% & 3,006 & T & T & \dag{} \\
NLI4CT & L & macro-F1 & 48.6\% & 2.43\% & 5,500 & T & T & \dag{} \\
RAGTruth & L & F1 on the hallucinated class & 51.8\% & 2.43\% & 2,700 & T & T & \dag{} \\
BANKING77 $\bigstar$ & R & macro-F1 & 1.3\% & 3.64\% & 3,080 & T & T & \dag{} \\
CLINC150 with out-of-scope $\bigstar$ & R & macro-F1 & 0.6\% & 3.64\% & 5,500 & T & T & \dag{} \\
BRIGHT $\bigstar$ & R & nDCG@10 & 11.6\% & 3.64\% & 20,383 & -- & G (written items, none of its documents) &  \\
Amazon ESCI & R & macro-F1 & 20.3\% & 3.03\% & 5,000 & T & T (resampled) & \dag{} \\
PhishNChips & R & accuracy & 50.0\% & 3.03\% & 18,000 & -- & G &  \\
HoVer & R & accuracy & 50.0\% & 3.03\% & 4,000 & T & T & \dag{} \\
BFCL $\bigstar$ & T & case exact accuracy & 25.9\% & 4.07\% & 4,768 & R & R &  \\
ToolRet & T & nDCG@10 & 13.4\% & 3.39\% & 40,127 & -- & T \textsuperscript{a} &  \\
API-Bank $\bigstar$ & T & accuracy & 1.9\% & 4.07\% & 508 & T (27B), R & R &  \\
Home appliance simulator & T & case exact accuracy & 0.0\% & 3.39\% & 2,895 & -- & G &  \\
When2Call & T & accuracy & 25.0\% & 3.39\% & 3,652 & T (2,700 rows) & T &  \\
BPoMP & A & accuracy & 50.0\% & 1.39\% & 5,000 & -- & G (written limericks) &  \\
Humicroedit & A & accuracy & 50.0\% & 1.39\% & 2,628 & -- (1 row \textsuperscript{b}) & T & \dag{} \\
POP909-CL & A & accuracy & 0.8\% & 1.39\% & 2,000 & -- & G (no material of the corpus) &  \\
cfcolor & A & accuracy & 50.0\% & 1.39\% & 5,000 & T (27B) & T &  \\
ForecastBench $\bigstar$ & A & (0.25 $-$ Brier) / 0.25 & baseline 0.25 & 1.67\% & 10,139 & -- & T (questions resolved before the test window) &  \\
Habermas & A & accuracy & 31.1\% & 1.39\% & 1,676 & -- & T &  \\
New Yorker caption matching & A & accuracy & 20.0\% & 1.39\% & 528 & T & T & \dag{} \\
\end{longtable}
\endgroup
\par\smallskip
{\footnotesize\raggedright\noindent \textsuperscript{a} The manuscript's table lists official training rows for ToolRet in the newest
rounds, while the final recipe is described as the full recipe without those rows (they cost the
benchmark 26 points). \todo{confirm the entry for the final recipe} \textsuperscript{b} A duplicate
filter keyed on option identifiers reduced this family to one row in the release mix
(Chapter~\ref{sec:4}). \textsuperscript{c} By difference from the total. The per-benchmark table of
the run does not list this benchmark. \textsuperscript{d} In edition 0.2.1 the wrong options of the
GSM8K rows give the answer away. Edition 0.3 rebuilds them. Every GSM8K value of this appendix is a
value on the old rows. The notes under Tables~\ref{tab:H.2}, \ref{tab:H.3} and \ref{tab:H.5} give
the values on the rebuilt rows.\par}

In the released weights 16 (4B line) to 18 (27B) benchmarks have an official training split in the
mix. After the data rounds 33 have training data aimed at them. GPQA Diamond and MMLU-Pro have
layout-only rows, and tool retrieval, HLE and CRUXEval are zero-shot (Table~\ref{tab:4.3}). The
public README marks 14 benchmarks with \dag{}. It lacks the mark on When2Call, WinoGrande and
HellaSwag and carries it on Humicroedit. \todo{bring the public page and this table into agreement;
re-check the mixes of the 0.8B, 2B, 9B and 35B-A3B, which were read from the 4B and 27B mixes}

\subsection{Released weights, per benchmark}\label{sec:H.2}

\begingroup
\renewcommand{\thetable}{H.2}
\footnotesize\setlength{\tabcolsep}{5pt}\renewcommand{\arraystretch}{1.1}
\begin{longtable}{>{\raggedright\arraybackslash}p{\mdw{0.1743}}>{\raggedright\arraybackslash}p{\mdw{0.1668}}>{\raggedright\arraybackslash}p{\mdw{0.2016}}>{\raggedleft\arraybackslash}p{\mdw{0.0624}}>{\raggedleft\arraybackslash}p{\mdw{0.0533}}>{\raggedleft\arraybackslash}p{\mdw{0.0581}}>{\raggedleft\arraybackslash}p{\mdw{0.0581}}>{\raggedleft\arraybackslash}p{\mdw{0.0581}}>{\raggedleft\arraybackslash}p{\mdw{0.0811}}>{\raggedleft\arraybackslash}p{\mdw{0.0745}}}
\caption{Native metric $\times$ coverage in percent for the six released models (own runs with the 0.2.1 kit, bf16, H200 GPUs, 2026-09-27 to 2026-10-01, best value of a row in bold) and for Jev 1.13 (public board, 2026-09-28). In-domain markers are those of Table~\ref{tab:H.1}.}\label{tab:H.2}\\
\toprule
\textbf{Area} & \textbf{Benchmark} & \textbf{Metric} & \textbf{0.8B} & \textbf{2B} & \textbf{4B} & \textbf{9B} & \textbf{27B} & \textbf{35B-A3B} & \textbf{Jev 1.13} \\
\midrule
\endfirsthead
\multicolumn{10}{l}{\textit{Table~\thetable{} (continued)}}\\
\toprule
\textbf{Area} & \textbf{Benchmark} & \textbf{Metric} & \textbf{0.8B} & \textbf{2B} & \textbf{4B} & \textbf{9B} & \textbf{27B} & \textbf{35B-A3B} & \textbf{Jev 1.13} \\
\midrule
\endhead
\bottomrule
\endfoot
Knowledge \& Reasoning & GSM8K \textsuperscript{a} & accuracy & 92.0 & 87.4 & 90.4 & 95.7 & 96.4 & \textbf{96.6} & 79.9 \\
Knowledge \& Reasoning & ChessBench & accuracy & 10.7 & 11.2 & 11.9 & 13.0 & \textbf{18.0} & 16.3 & 17.2 \\
Knowledge \& Reasoning & MuSR & accuracy & 54.8 & 56.0 & 56.0 & 59.0 & \textbf{67.8} & 60.2 & 66.1 \\
Knowledge \& Reasoning & SATA-Bench & case exact accuracy & 16.5 & 25.4 & 15.2 & 26.3 & 10.5 & \textbf{28.5} & 26.4 \\
Knowledge \& Reasoning & GPQA Diamond $\bigstar$ & accuracy & 32.1 & 42.4 & 41.8 & 50.0 & 50.5 & 51.0 & \textbf{78.6} \\
Knowledge \& Reasoning & CRUXEval & accuracy & 31.9 & 37.4 & 54.4 & 60.0 & \textbf{75.8} & 71.2 & 73.0 \\
Knowledge \& Reasoning & CLadder & accuracy & 56.3 & 58.6 & 65.9 & 68.1 & \textbf{73.7} & 69.6 & 72.6 \\
Knowledge \& Reasoning & HLE $\bigstar$ & accuracy & 12.8 & 14.2 & 12.8 & 10.2 & 12.4 & 10.2 & \textbf{20.4} \\
Knowledge \& Reasoning & MMLU-Pro $\bigstar$ & accuracy & 31.5 & 41.0 & 56.9 & 61.3 & 69.8 & 67.1 & \textbf{82.7} \\
Knowledge \& Reasoning & BBH $\bigstar$ & accuracy & 50.3 & 57.4 & 66.9 & 71.2 & 80.2 & 76.1 & \textbf{92.9} \\
Language Understanding & ContractNLI & macro-F1 & 83.2 & 83.4 & 83.9 & \textbf{86.6} & 86.4 & 85.4 & 71.7 \\
Language Understanding & ANLI $\bigstar$ & macro-F1 & 55.7 & 61.5 & 69.9 & 76.4 & \textbf{77.9} & 77.8 & 74.8 \\
Language Understanding & WinoGrande $\bigstar$ & accuracy & 67.8 & 74.3 & 85.2 & 91.5 & \textbf{93.5} & 93.0 & 92.0 \\
Language Understanding & HellaSwag $\bigstar$ & accuracy & 82.4 & 89.0 & 94.3 & 96.8 & 97.6 & \textbf{97.7} & 94.5 \\
Language Understanding & ACOS & per-review F1 & 45.1 & 35.5 & 34.3 & 47.8 & \textbf{52.0} & \textbf{52.0} & 29.5 \\
Language Understanding & FinEntity & macro-F1 & 77.8 & 76.2 & 90.9 & 88.2 & \textbf{92.7} & 88.6 & 87.0 \\
Language Understanding & iSarcasmEval & Sarcasm F1 \textperiodcentered{} track A, English & 18.4 & 30.9 & 51.3 & 62.6 & 63.0 & \textbf{67.9} & 50.5 \\
Language Understanding & VAST & macro-F1 & 74.6 & 76.9 & 76.7 & 79.1 & \textbf{82.3} & 80.2 & 64.6 \\
Language Understanding & NLI4CT & macro-F1 & 66.3 & 70.3 & 79.4 & 82.6 & \textbf{85.8} & 84.6 & 84.1 \\
Language Understanding & RAGTruth & F1 on hallucinated class & 76.8 & 79.1 & 80.0 & 84.3 & \textbf{85.6} & 84.9 & 76.5 \\
Retrieval \& Classification & BANKING77 $\bigstar$ & macro-F1 & 89.9 & 86.1 & 85.9 & \textbf{91.4} & 91.0 & 91.1 & 79.7 \\
Retrieval \& Classification & CLINC150 $\bigstar$ & macro-F1 & 90.3 & 86.8 & 91.5 & 93.2 & 93.0 & \textbf{93.7} & 89.3 \\
Retrieval \& Classification & BRIGHT $\bigstar$ & nDCG@10 & 38.7 & 40.4 & 45.4 & 48.1 & \textbf{50.0} & 48.4 & 47.5 \\
Retrieval \& Classification & Amazon ESCI & macro-F1 & 51.1 & 52.0 & 54.7 & 58.1 & \textbf{58.5} & 57.2 & 55.2 \\
Retrieval \& Classification & PhishNChips & accuracy & 50.1 & 56.5 & 59.9 & 64.2 & \textbf{70.5} & 69.1 & 62.5 \\
Retrieval \& Classification & HoVer & accuracy & 77.2 & 75.0 & 76.4 & 88.2 & \textbf{89.6} & 89.0 & 72.9 \\
Retrieval \& Classification & SGD (0.2 only) & macro-F1 & 69.8 & 70.8 & 67.9 & 71.9 & \textbf{74.0} & 73.2 &  \\
Tools \& Automation & BFCL $\bigstar$ & case exact accuracy & 93.5 & 95.5 & 96.1 & \textbf{97.8} & 97.6 & 97.5 & 95.8 \\
Tools \& Automation & ToolRet & nDCG@10 & 63.2 & 64.2 & 67.5 & 66.6 & \textbf{69.1} & 68.8 & 65.3 \\
Tools \& Automation & API-Bank $\bigstar$ & accuracy & 17.9 & 50.4 & 86.2 & 78.3 & 84.1 & 79.9 & \textbf{88.2} \\
Tools \& Automation & Home appliances & case exact accuracy & 0.0 & 17.1 & 30.7 & 38.6 & \textbf{77.3} & 51.1 & 52.3 \\
Tools \& Automation & When2Call & accuracy & 79.5 & 80.3 & 85.2 & 88.9 & \textbf{89.2} & 88.5 & 81.0 \\
Tools \& Automation & RouterBench (0.2 only) & selected quality (quality objective) & 75.9 & 78.9 & \textbf{80.0} & 79.9 & 79.7 & \textbf{80.0} & 79.9 \\
Arts \& Human Taste & BPoMP & accuracy & 59.8 & 67.6 & 83.1 & 91.0 & \textbf{95.3} & 92.8 & 90.9 \\
Arts \& Human Taste & Humicroedit & accuracy & 56.7 & 61.6 & 59.8 & 62.2 & \textbf{62.9} & 62.4 & 61.9 \\
Arts \& Human Taste & POP909 & accuracy & 6.4 & 3.1 & 16.6 & 26.1 & \textbf{51.0} & 32.5 & 16.6 \\
Arts \& Human Taste & cfcolor & accuracy & 64.2 & 62.0 & 65.2 & 71.2 & \textbf{71.8} & 71.3 & 64.4 \\
Arts \& Human Taste & ForecastBench $\bigstar$ & (0.25 - Brier) / 0.25, higher is better & 0.8 & 13.8 & 24.6 & 26.6 & \textbf{34.3} & 30.6 & 30.6 \\
Arts \& Human Taste & Habermas & accuracy & 44.0 & 45.1 & 43.3 & 46.6 & 43.8 & \textbf{49.2} & 45.9 \\
Arts \& Human Taste & New Yorker & accuracy & 58.3 & 66.5 & 70.6 & 77.6 & \textbf{79.4} & \textbf{79.4} & 70.1 \\
\end{longtable}
\endgroup
\par\smallskip
{\footnotesize\raggedright\noindent \textsuperscript{a} Rows of edition 0.2.1, which could be answered from the layout of the options
(Section~\ref{sec:6.2.1}). On the rows rebuilt for edition 0.3 the one-pass skill of the released
models, in the chance-corrected units of Table~\ref{tab:H.3}, is 2.0 (0.8B), 7.1 (2B), 37.2 (4B),
30.8 (9B) and 60.5 (27B) in our own runs of 7 October 2026 (Table~\ref{tab:6.15}). The 35B-A3B has
not been run on the rebuilt rows. The board data of edition 0.3 give the hosted reference 66 on
them.\par}

\begingroup
\renewcommand{\thetable}{H.3}
\scriptsize\setlength{\tabcolsep}{4pt}\renewcommand{\arraystretch}{1.1}
\begin{longtable}{>{\raggedright\arraybackslash}p{\mdw{0.1565}}>{\raggedleft\arraybackslash}p{\mdw{0.1221}}>{\raggedleft\arraybackslash}p{\mdw{0.1334}}>{\raggedleft\arraybackslash}p{\mdw{0.1196}}>{\raggedleft\arraybackslash}p{\mdw{0.1196}}>{\raggedleft\arraybackslash}p{\mdw{0.0607}}>{\raggedleft\arraybackslash}p{\mdw{0.0798}}>{\raggedleft\arraybackslash}p{\mdw{0.0979}}>{\raggedleft\arraybackslash}p{\mdw{0.0977}}}
\caption{Chance-corrected skill, the index's own scale, for four released sizes and four other systems (their values from the public board, 2026-09-28). Rows in bold are the index and its area scores. A bold value is the best of its row.}\label{tab:H.3}\\
\toprule
 & \textbf{StartLux-Decision-27B} & \textbf{StartLux-Decision-35B-A3B} & \textbf{StartLux-Decision-9B} & \textbf{StartLux-Decision-4B} & \textbf{Jev 1.13} & \textbf{Rune 26B-A4B} & \textbf{Decider chat 31B} & \textbf{AutoJev-27B} \\
\midrule
\endfirsthead
\multicolumn{9}{l}{\textit{Table~\thetable{} (continued)}}\\
\toprule
 & \textbf{StartLux-Decision-27B} & \textbf{StartLux-Decision-35B-A3B} & \textbf{StartLux-Decision-9B} & \textbf{StartLux-Decision-4B} & \textbf{Jev 1.13} & \textbf{Rune 26B-A4B} & \textbf{Decider chat 31B} & \textbf{AutoJev-27B} \\
\midrule
\endhead
\bottomrule
\endfoot
\textbf{Decision Index 0.2.1} & \textbf{63.88} & 61.55 & 58.63 & 52.75 & 57.91 & 57.44 & 57.33 & 56.40 \\
\textbf{Knowledge \& Reasoning} & 44.3 & 42.4 & 38.0 & 32.1 & \textbf{51.4} & 43.4 & 44.3 & 40.9 \\
GSM8K \textsuperscript{a} & 95.3 & \textbf{95.6} & 94.3 & 87.8 & 75.6 & 75.7 & 78.8 & 61.1 \\
ChessBench & 10.7 & 8.8 & 5.3 & 4.0 & 9.8 & 11.5 & \textbf{15.4} & 9.8 \\
MuSR & \textbf{48.8} & 36.8 & 34.9 & 30.0 & 46.1 & 44.2 & 43.1 & 39.3 \\
SATA-Bench & 9.3 & 27.5 & 25.3 & 14.0 & 25.4 & \textbf{34.0} & 28.4 & 28.9 \\
GPQA Diamond $\bigstar$ & 34.0 & 34.7 & 33.3 & 22.4 & \textbf{71.4} & 29.2 & 32.0 & 32.6 \\
CRUXEval & 61.6 & 54.4 & 36.5 & 27.6 & 57.1 & 59.4 & \textbf{67.2} & 60.2 \\
CLadder & 47.3 & 39.1 & 36.1 & 31.8 & 45.3 & 45.5 & \textbf{49.2} & 49.0 \\
HLE $\bigstar$ & 0.0 & 0.0 & 0.0 & 0.0 & \textbf{4.7} & 0.0 & 0.0 & 0.0 \\
MMLU-Pro $\bigstar$ & 66.0 & 63.0 & 56.5 & 51.6 & \textbf{80.5} & 63.1 & 65.8 & 60.1 \\
BBH $\bigstar$ & 71.3 & 65.4 & 58.2 & 52.0 & \textbf{89.7} & 72.7 & 65.5 & 68.3 \\
\textbf{Language Understanding} & \textbf{74.5} & 73.6 & 71.3 & 63.9 & 62.0 & 63.1 & 60.4 & 63.5 \\
ContractNLI & 80.3 & 78.9 & \textbf{80.6} & 76.8 & 59.1 & 66.7 & 61.8 & 68.4 \\
ANLI $\bigstar$ & \textbf{67.0} & 66.8 & 64.6 & 54.9 & 62.2 & 60.3 & 59.8 & 56.0 \\
WinoGrande $\bigstar$ & \textbf{87.1} & 86.0 & 83.0 & 70.3 & 83.9 & 71.9 & 67.3 & 70.3 \\
HellaSwag $\bigstar$ & 96.8 & \textbf{97.0} & 95.7 & 92.4 & 92.7 & 89.9 & 89.4 & 92.0 \\
ACOS & 50.4 & \textbf{50.5} & 46.2 & 32.2 & 27.3 & 24.4 & 16.2 & 17.8 \\
FinEntity & 89.3 & 83.3 & 82.6 & 86.6 & 80.8 & 83.0 & 86.6 & \textbf{89.6} \\
iSarcasmEval & 52.4 & \textbf{58.7} & 51.9 & 37.3 & 36.3 & 49.0 & 37.0 & 49.0 \\
VAST & \textbf{73.4} & 70.3 & 68.7 & 65.0 & 46.9 & 64.9 & 59.8 & 56.2 \\
NLI4CT & \textbf{72.3} & 70.0 & 66.1 & 60.0 & 69.0 & 62.0 & 66.6 & 70.5 \\
RAGTruth & \textbf{70.1} & 68.7 & 67.5 & 58.5 & 51.3 & 51.9 & 52.2 & 59.2 \\
\textbf{Retrieval \& Classification} & \textbf{66.8} & 65.8 & 64.1 & 56.7 & 55.4 & 63.5 & 63.1 & 54.9 \\
BANKING77 $\bigstar$ & 90.9 & 91.0 & \textbf{91.3} & 85.7 & 79.5 & 83.5 & 78.8 & 78.8 \\
CLINC150 $\bigstar$ & 92.9 & \textbf{93.7} & 93.1 & 91.5 & 89.2 & 87.3 & 91.1 & 87.7 \\
BRIGHT $\bigstar$ & \textbf{43.5} & 41.7 & 41.3 & 38.2 & 40.6 & 39.3 & 36.2 & 41.9 \\
Amazon ESCI & \textbf{47.9} & 46.3 & 47.4 & 43.2 & 43.8 & 43.9 & 41.2 & 43.7 \\
PhishNChips & 40.9 & 38.2 & 28.5 & 19.8 & 25.1 & 61.8 & \textbf{75.0} & 19.9 \\
HoVer & \textbf{79.2} & 78.1 & 76.5 & 52.8 & 45.7 & 61.3 & 52.8 & 48.4 \\
\textbf{Tools \& Automation} & \textbf{82.2} & 76.2 & 73.2 & 72.3 & 75.1 & 71.2 & 75.6 & 79.3 \\
BFCL $\bigstar$ & 96.7 & 96.7 & 97.0 & 94.7 & 94.3 & 93.0 & \textbf{97.3} & 96.8 \\
ToolRet & \textbf{64.3} & 64.0 & 61.5 & 62.5 & 59.9 & 58.9 & 58.0 & 62.4 \\
API-Bank $\bigstar$ & 83.8 & 79.5 & 77.9 & 86.0 & \textbf{88.0} & 83.0 & 84.8 & 83.8 \\
Home appliances & \textbf{77.3} & 51.1 & 38.6 & 30.7 & 52.3 & 46.6 & 62.5 & 73.9 \\
When2Call & \textbf{85.7} & 84.7 & 85.2 & 80.3 & 74.6 & 68.0 & 69.2 & 75.6 \\
\textbf{Arts \& Human Taste} & \textbf{47.9} & 44.7 & 41.8 & 33.7 & 37.7 & 41.9 & 38.3 & 39.4 \\
BPoMP & \textbf{90.6} & 85.7 & 82.1 & 66.3 & 81.8 & 79.9 & 81.2 & 87.8 \\
Humicroedit & 25.8 & 24.7 & 24.3 & 19.6 & 23.7 & 24.4 & \textbf{27.6} & 24.8 \\
POP909 & 50.6 & 32.0 & 25.5 & 16.0 & 15.9 & \textbf{65.8} & 27.3 & 37.3 \\
cfcolor & \textbf{43.6} & 42.5 & 42.4 & 30.5 & 28.8 & 25.1 & 25.2 & 28.8 \\
ForecastBench $\bigstar$ & \textbf{34.3} & 30.6 & 26.6 & 24.6 & 30.6 & 18.9 & 19.2 & 22.1 \\
Habermas & 18.4 & \textbf{26.2} & 22.5 & 17.7 & 21.5 & 16.2 & 24.4 & 15.5 \\
New Yorker & \textbf{74.2} & \textbf{74.2} & 72.1 & 63.3 & 62.6 & 67.6 & 67.3 & 62.8 \\
\end{longtable}
\endgroup
\par\smallskip
{\footnotesize\raggedright\noindent \textsuperscript{a} Rows of edition 0.2.1. On the rows rebuilt for edition 0.3 our own runs of 7
October 2026 give 60.5 for the released 27B, 30.8 for the 9B and 37.2 for the 4B, where the same
runs give 95.3, 94.3 and 87.9 on the old rows. The 35B-A3B has not been run on them. The board data
of edition 0.3 give the hosted reference 66 on the rebuilt rows. This appendix has no rebuilt-row
values for the three other systems of the table.\par}

The released 27B is below Jev 1.13 on seven benchmarks: GPQA Diamond, SATA-Bench, HLE, MMLU-Pro,
BBH, API-Bank and Habermas. On the rebuilt GSM8K rows it is below the hosted reference as well (60.5
in our own run against 66 in the board data of edition 0.3).

\begin{table}[!htbp]
\renewcommand{\thetable}{H.4}
\centering
\caption{The seven suites of the Intern-Decision bundle, accuracy in percent (own runs of the released weights, other rows as reported in the bundle's README, commit 2f81580, same scorer). Easy, Original and Hard are the 48, 72 and 111 public JevBench items. Typed is the test split of Typed Decisions, whose training split is in our training mix.}\label{tab:H.4}
{\footnotesize\setlength{\tabcolsep}{4pt}\renewcommand{\arraystretch}{1.1}
\noindent\begin{adjustbox}{max width=\linewidth}
\begin{tabular}{lrrrrrrrrr}
\toprule
\textbf{Model} & \textbf{Easy} & \textbf{Original} & \textbf{Hard} & \textbf{Typed} & \textbf{ToolACE} & {\begin{tabular}[b]{@{}r@{}}\textbf{AG}\\\textbf{News}\end{tabular}} & \textbf{WildJB} & \textbf{Average} & {\begin{tabular}[b]{@{}r@{}}\textbf{Average}\\\textbf{without}\\\textbf{ToolACE}\end{tabular}} \\
\midrule
\mdourrow StartLux-Decision-0.8B & 100.00 & 90.28 & 59.46 & 75.85 & 91.94 & 90.97 & 86.70 & \textbf{85.03} & 83.88 \\
\mdourrow StartLux-Decision-2B & 100.00 & 94.44 & 72.07 & 77.95 & 93.23 & 89.43 & 92.13 & \textbf{88.46} & 87.67 \\
\mdourrow StartLux-Decision-4B & 100.00 & 100.00 & 75.68 & 79.95 & 94.19 & 90.91 & 97.47 & \textbf{91.17} & 90.67 \\
\mdourrow StartLux-Decision-9B & 100.00 & 97.22 & 74.77 & 81.45 & 94.84 & 91.97 & 97.33 & \textbf{91.08} & 90.46 \\
\mdourrow StartLux-Decision-27B & 100.00 & 100.00 & 79.28 & 80.20 & 94.52 & 90.57 & 98.19 & \textbf{91.82} & 91.37 \\
\mdourrow StartLux-Decision-35B-A3B & 100.00 & 98.61 & 81.98 & 81.30 & 95.48 & 91.00 & 97.65 & \textbf{92.29} & 91.76 \\
Jev 1.13 & 100.00 & 98.61 & 72.07 & 73.35 & 91.29 & 89.57 & 96.29 & 88.74 & 88.31 \\
Laya & 95.83 & 72.22 & 28.83 & 35.95 & 63.87 & 92.84 & 14.84 & 57.77 & 56.75 \\
SemIf & 100.00 & 98.61 & 61.26 & 62.80 & 85.16 & 89.22 & 92.53 & 84.23 & 84.07 \\
Kev (size not stated) & 100.00 & 93.06 & 45.05 & 65.60 & 87.42 & 89.82 & 75.97 & 79.56 & 78.25 \\
JevK5 & 100.00 & 97.22 & 73.87 & 64.50 & 80.97 & 89.13 & 90.45 & 85.16 & 85.86 \\
Intern-Decision-0.8B & 97.92 & 80.56 & 52.25 & 77.35 & 94.52 & 88.61 & 64.48 & 79.38 & 76.86 \\
Intern-Decision-2B & 100.00 & 84.72 & 63.96 & 79.35 & 96.45 & 89.96 & 78.33 & 84.68 & 82.72 \\
Intern-Decision-4B & 100.00 & 98.61 & 73.87 & 80.55 & 96.45 & 90.82 & 89.86 & 90.02 & 88.95 \\
\bottomrule
\end{tabular}
\end{adjustbox}\par}
\end{table}

Typed Decisions in more detail (test split, 400 cases, 2,000 decisions, against soft labels):
accuracy 0.758 (0.8B), 0.779 (2B), 0.799 (4B), 0.815 (9B), 0.802 (27B), 0.813 (35B-A3B). The dataset
card lists 0.727 for Jev 1.13.0 and 0.470 for the prior. The card gives 0.735 as the agreement of a
fresh sample of the labelling model with the gold labels and warns that a score far above it means
predicting that model's habits. No test case is in our training data (no shared identifier, no
identical state), but both splits come from one generator and 20 question schemas, and a test state
shares a median 26\% of its word 13-grams with training states. By the card's terms our number is a
specialist's.

\subsection{After data rounds, per benchmark}\label{sec:H.3}

\begingroup
\renewcommand{\thetable}{H.5}
\scriptsize\setlength{\tabcolsep}{4pt}\renewcommand{\arraystretch}{1.1}
\begin{longtable}{lrrrrrrrr}
\caption{Raw benchmark scores ($\times$ 100, while the index uses chance-corrected skill) in one pass and with reasoning at the default threshold, for the 4B after data rounds (reader round, index 64.78 $\rightarrow$ 66.38) and the 9B after data rounds with thinking replay (index 67.75 $\rightarrow$ 69.77). Own runs on the corrected serving path, 2026-10-06, 337,742 answers each.}\label{tab:H.5}\\
\toprule
\textbf{benchmark} & {\begin{tabular}[b]{@{}r@{}}\textbf{4B:}\\\textbf{one}\\\textbf{pass}\end{tabular}} & \textbf{reasoning} & {\begin{tabular}[b]{@{}r@{}}\textbf{reasoned}\\\textbf{about}\end{tabular}} & {\begin{tabular}[b]{@{}r@{}}\textbf{tokens}\\\textbf{per}\\\textbf{thought}\end{tabular}} & {\begin{tabular}[b]{@{}r@{}}\textbf{9B:}\\\textbf{one}\\\textbf{pass}\end{tabular}} & {\begin{tabular}[b]{@{}r@{}}\textbf{reasoning after}\\\textbf{thinking replay}\end{tabular}} & {\begin{tabular}[b]{@{}r@{}}\textbf{reasoned}\\\textbf{about}\end{tabular}} & {\begin{tabular}[b]{@{}r@{}}\textbf{tokens}\\\textbf{per}\\\textbf{thought}\end{tabular}} \\
\midrule
\endfirsthead
\multicolumn{9}{l}{\textit{Table~\thetable{} (continued)}}\\
\toprule
\textbf{benchmark} & {\begin{tabular}[b]{@{}r@{}}\textbf{4B:}\\\textbf{one}\\\textbf{pass}\end{tabular}} & \textbf{reasoning} & {\begin{tabular}[b]{@{}r@{}}\textbf{reasoned}\\\textbf{about}\end{tabular}} & {\begin{tabular}[b]{@{}r@{}}\textbf{tokens}\\\textbf{per}\\\textbf{thought}\end{tabular}} & {\begin{tabular}[b]{@{}r@{}}\textbf{9B:}\\\textbf{one}\\\textbf{pass}\end{tabular}} & {\begin{tabular}[b]{@{}r@{}}\textbf{reasoning after}\\\textbf{thinking replay}\end{tabular}} & {\begin{tabular}[b]{@{}r@{}}\textbf{reasoned}\\\textbf{about}\end{tabular}} & {\begin{tabular}[b]{@{}r@{}}\textbf{tokens}\\\textbf{per}\\\textbf{thought}\end{tabular}} \\
\midrule
\endhead
\bottomrule
\endfoot
GSM8K \textsuperscript{a} & 93.78 & 97.73 & 31.4\% & 267 & 96.06 & 99.32 & 17.9\% & 875 \\
ChessBench & 22.92 & 22.70 & 99.1\% & 502 & 23.32 & 23.18 & 99.2\% & 2,956 \\
MuSR & 67.95 & 68.88 & 62.0\% & 352 & 67.95 & 69.68 & 56.7\% & 3,821 \\
SATA-Bench & 57.76 & 56.73 & 23.0\% & 347 & 58.36 & 55.94 & 23.0\% & 3,555 \\
GPQA Diamond $\bigstar$ & 42.35 & 48.47 & 95.5\% & 742 & 51.53 & 62.24 & 89.4\% & 3,976 \\
CRUXEval & 55.09 & 60.35 & 90.5\% & 283 & 60.35 & 88.42 & 80.7\% & 2,664 \\
CLadder & 85.50 & 87.72 & 28.7\% & 573 & 89.10 & 91.96 & 19.5\% & 3,318 \\
HLE $\bigstar$ & 12.18 & 11.58 & 97.1\% & 506 & 11.18 & 13.57 & 92.0\% & 3,920 \\
MMLU-Pro $\bigstar$ & 55.94 & 68.17 & 77.2\% & 657 & 60.71 & 73.65 & 64.1\% & 3,594 \\
BBH, fixed-option tasks $\bigstar$ & 81.55 & 84.86 & 46.0\% & 298 & 85.29 & 88.60 & 39.2\% & 3,259 \\
ContractNLI & 84.34 & 84.93 & 32.6\% & 384 & 85.86 & 85.39 & 23.1\% & 3,696 \\
ANLI $\bigstar$ & 71.93 & 73.91 & 66.4\% & 343 & 76.19 & 76.76 & 55.6\% & 3,380 \\
WinoGrande $\bigstar$ & 87.61 & 87.69 & 27.1\% & 362 & 91.55 & 92.42 & 11.6\% & 3,211 \\
HellaSwag $\bigstar$ & 94.53 & 94.20 & 15.2\% & 309 & 96.50 & 96.43 & 6.8\% & 3,799 \\
ACOS & 60.62 & 61.25 & 2.7\% & 248 & 64.89 & 63.70 & 2.3\% & 3,590 \\
FinEntity & 95.19 & 95.33 & 40.5\% & 218 & 95.09 & 95.45 & 31.0\% & 2,944 \\
iSarcasmEval & -- & -- & -- & -- & -- & -- & -- & -- \\
VAST & 77.62 & 77.62 & 67.2\% & 263 & 78.22 & 78.81 & 57.9\% & 3,528 \\
NLI4CT & 78.27 & 80.54 & 59.4\% & 352 & 81.40 & 83.05 & 41.2\% & 3,443 \\
RAGTruth & 83.91 & 83.41 & 68.0\% & 243 & 84.27 & 83.15 & 56.8\% & 3,761 \\
BANKING77 $\bigstar$ & 89.81 & 89.55 & 31.7\% & 342 & 92.53 & 92.17 & 17.2\% & 3,700 \\
CLINC150 with out-of-scope $\bigstar$ & 91.65 & 92.99 & 25.6\% & 245 & 93.81 & 93.57 & 15.3\% & 3,469 \\
BRIGHT $\bigstar$ & 44.59 & 44.46 & 13.0\% & 235 & 47.30 & 47.88 & 14.2\% & 3,103 \\
Amazon ESCI & 61.39 & 61.99 & 80.7\% & 302 & 61.99 & 62.18 & 76.5\% & 3,173 \\
PhishNChips & 85.95 & 86.15 & 14.9\% & 266 & 90.90 & 89.20 & 16.1\% & 3,336 \\
HoVer & 87.83 & 88.52 & 41.7\% & 221 & 89.03 & 88.38 & 31.1\% & 3,090 \\
BFCL $\bigstar$ & 96.69 & 96.99 & 5.8\% & 364 & 97.99 & 97.70 & 5.1\% & 3,184 \\
ToolRet & 68.15 & 67.98 & 27.7\% & 320 & 67.65 & 67.01 & 29.2\% & 3,315 \\
API-Bank $\bigstar$ & 85.24 & 87.60 & 54.3\% & 361 & 82.68 & 82.48 & 76.6\% & 2,239 \\
Home appliance simulator & 94.32 & 93.18 & 1.9\% & 165 & 95.45 & 95.45 & 3.5\% & 2,919 \\
When2Call & 92.66 & 91.62 & 23.9\% & 223 & 92.83 & 91.07 & 27.3\% & 3,673 \\
BPoMP & 94.46 & 95.36 & 26.3\% & 324 & 95.56 & 95.94 & 17.5\% & 3,931 \\
Humicroedit & 64.80 & 64.19 & 99.4\% & 158 & 65.26 & 66.63 & 99.3\% & 2,988 \\
POP909-CL & 80.35 & 79.45 & 35.0\% & 196 & 80.80 & 80.10 & 41.9\% & 3,342 \\
cfcolor & 68.42 & 68.54 & 99.4\% & 327 & 69.42 & 69.42 & 93.0\% & 4,064 \\
ForecastBench $\bigstar$ & 17.74 & 17.47 & 72.8\% & 358 & 16.88 & 17.23 & 72.8\% & 3,502 \\
Habermas & 63.07 & 62.29 & 96.9\% & 247 & 64.02 & 64.38 & 96.3\% & 3,926 \\
New Yorker caption matching & 74.05 & 75.19 & 38.1\% & 323 & 78.60 & 78.98 & 29.9\% & 3,772 \\
RouterBench (edition 0.2 only) & 79.96 & 79.92 & 100.0\% & 551 & 79.85 & 80.05 & 100.0\% & 3,935 \\
SGD (edition 0.2 only) & 46.68 & 47.32 & 44.9\% & 240 & 69.22 & 67.59 & 68.8\% & 3,701 \\
\end{longtable}
\endgroup
\par\smallskip
{\footnotesize\raggedright\noindent \textsuperscript{a} Rows of edition 0.2.1. On the rows rebuilt for edition 0.3 the 4B and the 9B
after the data rounds have a one-pass skill of 23.0 and 26.1, against 91.8 and 94.7 on the old rows.
Neither run of this table has been repeated on the rebuilt rows. With a thought on every item, the
4B and the 9B after the stop step reach a skill of 94.4 and 96.3 on them, and 93.8 and 94.6 with the
default answer (Table~\ref{tab:5.9}).\par}

Over all answers the 4B reasons about 32.2\% with 388 tokens per thought (125 reasoning tokens per
answer), the 9B after replay about 29.8\% with 3,517 tokens per thought (1,049 per answer).
\todo{the same table for the 9B and the 27B with the reader round only, and per-benchmark skill of
the 0.8B, 2B and 27B after data rounds, from the score files of those runs}

\subsection{Spread between training rounds}\label{sec:H.4}

\begin{table}[!htbp]
\renewcommand{\thetable}{H.6}
\centering
\caption{Thirteen benchmarks over nineteen training rounds of the 4B (chance-corrected skill, one pass, own runs, the first row is the released model). The jumps are the targeted sources of Section~\ref{sec:4.6}. The columns that do not jump show the spread between rounds.}\label{tab:H.6}
{\tiny\setlength{\tabcolsep}{2pt}\renewcommand{\arraystretch}{1.1}
\noindent\begin{adjustbox}{max width=\linewidth}
\begin{tabular}{>{\raggedright\arraybackslash}p{\mdw{0.1527}}>{\raggedleft\arraybackslash}p{\mdw{0.0390}}>{\raggedleft\arraybackslash}p{\mdw{0.0452}}>{\raggedleft\arraybackslash}p{\mdw{0.0559}}>{\raggedleft\arraybackslash}p{\mdw{0.0724}}>{\raggedleft\arraybackslash}p{\mdw{0.0725}}>{\raggedleft\arraybackslash}p{\mdw{0.0373}}>{\raggedleft\arraybackslash}p{\mdw{0.0466}}>{\raggedleft\arraybackslash}p{\mdw{0.0611}}>{\raggedleft\arraybackslash}p{\mdw{0.0683}}>{\raggedleft\arraybackslash}p{\mdw{0.0430}}>{\raggedleft\arraybackslash}p{\mdw{0.0743}}>{\raggedleft\arraybackslash}p{\mdw{0.0739}}>{\raggedleft\arraybackslash}p{\mdw{0.0791}}>{\raggedleft\arraybackslash}p{\mdw{0.0656}}}
\toprule
\textbf{round} & \textbf{index} & \textbf{chords} & \textbf{phishing} & \textbf{aspect sentiment} & \textbf{shopping relevance} & \textbf{chess} & \textbf{select-all} & \textbf{tool retrieval} & \textbf{code execution} & \textbf{causal} & \textbf{appliance simulator} & \textbf{narrative reasoning} & \textbf{claim verification} & \textbf{preference} \\
\midrule
released & 52.76 & 15.9 & 19.8 & 32.2 & 43.1 & 4.1 & 14.0 & 62.5 & 27.9 & 31.7 & 30.7 & 30.2 & 53.0 & 17.4 \\
1 & 53.32 & 17.2 & 20.8 & 34.5 & 42.0 & 5.0 & 18.9 & 62.5 & 25.1 & 73.3 & 29.5 & 31.5 & 45.5 & 20.5 \\
2 & 52.04 & 3.4 & 14.6 & 29.9 & 40.7 & 3.8 & 11.5 & 61.0 & 15.1 & 73.9 & 26.1 & 30.6 & 45.0 & 23.5 \\
3 & 52.55 & 6.3 & 20.4 & 33.7 & 40.8 & 13.4 & 26.6 & 61.8 & 13.4 & 73.9 & 31.8 & 44.2 & 46.0 & 21.1 \\
4 & 55.06 & 11.6 & 22.6 & 30.8 & 39.9 & 4.9 & 28.0 & 60.4 & 24.9 & 66.2 & 94.3 & 45.9 & 48.3 & 25.3 \\
5 & 56.11 & 14.9 & 18.0 & 33.1 & 42.7 & 4.1 & 29.9 & 62.0 & 26.5 & 77.4 & 86.4 & 44.0 & 49.8 & 20.6 \\
7 & 58.31 & 9.4 & 23.6 & 42.2 & 45.0 & 4.4 & 28.3 & 62.0 & 25.7 & 76.1 & 89.8 & 41.9 & 74.3 & 43.3 \\
8 & 58.91 & 78.3 & 18.2 & 43.9 & 45.0 & 4.0 & 25.7 & 61.9 & 27.1 & 75.8 & 81.8 & 41.0 & 74.2 & 44.2 \\
10 & 59.45 & 80.0 & 14.5 & 61.2 & 51.3 & 3.8 & 27.9 & 62.6 & 28.7 & 71.6 & 89.8 & 42.5 & 74.4 & 43.0 \\
11 & 60.69 & 77.9 & 72.1 & 59.7 & 51.5 & 3.7 & 25.8 & 63.2 & 24.0 & 74.0 & 85.2 & 42.9 & 75.2 & 44.1 \\
11, option order of one source randomised & 61.32 & 81.1 & 79.1 & 60.7 & 51.3 & 3.6 & 25.7 & 62.4 & 25.4 & 76.4 & 90.9 & 44.8 & 74.8 & 45.0 \\
12 & 60.94 & 80.0 & 65.0 & 60.0 & 51.0 & 15.2 & 26.0 & 63.3 & 24.0 & 73.2 & 92.0 & 42.3 & 74.8 & 45.4 \\
12, second phishing generator & 61.22 & 79.6 & 79.2 & 61.4 & 51.1 & 15.1 & 25.9 & 62.7 & 28.5 & 72.5 & 87.5 & 43.3 & 74.7 & 46.1 \\
14 & 60.03 & 80.6 & 79.0 & 59.2 & 51.3 & 15.0 & 33.4 & 36.5 & 25.7 & 71.2 & 88.6 & 42.7 & 73.6 & 44.8 \\
18, full recipe & 63.32 & 81.0 & 82.3 & 59.4 & 51.4 & 14.9 & 32.6 & 36.4 & 28.7 & 74.7 & 88.6 & 48.2 & 75.4 & 44.5 \\
19, full recipe and four select-all sources & 63.94 & 79.0 & 82.2 & 60.9 & 52.2 & 15.6 & 56.3 & 35.1 & 29.0 & 76.3 & 93.2 & 48.4 & 76.1 & 46.2 \\
18 without the official tool-retrieval rows & 64.29 & 80.6 & 80.7 & 59.5 & 50.6 & 15.6 & 32.9 & 63.1 & 31.5 & 78.9 & 88.6 & 45.5 & 76.4 & 44.0 \\
20, final recipe: 18 without those rows, with the four select-all sources and a heavier anchor & 64.78 & 79.6 & 71.9 & 59.4 & 51.6 & 16.1 & 57.2 & 63.2 & 28.7 & 71.0 & 94.3 & 49.0 & 75.6 & 46.4 \\
21, final recipe with evidence-removal rows & 64.76 & 80.1 & 82.8 & 60.1 & 52.2 & 15.4 & 56.6 & 63.4 & 29.3 & 76.0 & 87.5 & 44.4 & 75.3 & 46.7 \\
\bottomrule
\end{tabular}
\end{adjustbox}\par}
\end{table}

Five observations set the scale for reading any difference between two rounds.

\begin{itemize}
\item The same recipe trained twice, with only the seed of the mixer changed, gives 60.69 and 60.87.
Behind the 0.18 are PhishNChips at 72.1 and 64.9, When2Call at 75.2 and 79.6, CRUXEval at 24.0 and
28.2, and the appliance simulator at 85.2 and 81.8.
\item With the same phishing data, five rounds that differ in other sources score 72.1, 65.0, 79.0, 69.6
and 79.1 on PhishNChips. At 3.0--3.4\% of the index each, such benchmarks alone move the index by
$\pm$0.3.
\item A released model can be a lucky draw: the released 4B answered 63 of 111 items of one long-document
bucket, where 48 later rounds average 58.0 with a standard deviation of 2.6. On the whole set it is
in the middle (133 right against 132.0 $\pm$ 3.7).
\item A 198-question benchmark returns to its mean: one round stood at 29.2 on GPQA Diamond where seven
others stand at 22.4--24.5.
\item Three rounds of nearly the same final recipe span 64.76 to 65.67, with PhishNChips moving by 10
points between them.
\end{itemize}

Repeated inference is a much smaller source: two runs of one reasoning system with thoughts sampled
anew differ by 0.05 on the index. Before a difference between rounds is interpreted we pair the
items and count flips, look at the spread of earlier rounds on the same benchmark, and repeat the
round under another seed.

\subsection{JevBench after the release}\label{sec:H.5}

On the 231 public items in one pass the models after data rounds answer 205 (4B), 202 (9B) and 213
(27B, round without the last four sources). An earlier 9B round answered 206. With reasoning:
released 27B 229 with a thought before every answer, 227 at the default threshold with 61 items
reasoned about, and released 4B 218 with a thought before every answer. The official board, revision
1.6.0 of 2026-10-05, has 1,500 items of which 300 are public as aggregates only. We are not listed
and have no run on it.

\subsection{Lists longer than one pass reads}\label{sec:H.6}

\begin{table}[!htbp]
\renewcommand{\thetable}{H.7}
\centering
\caption{Knock-out on long lists: 1,000 questions of two intent benchmarks (evaluation only), each list cut or extended to the given length with the other benchmark's labels beyond a benchmark's own. Released weights, one H200, 2026-10-06. Groups of at most 25 options, the best three of each group go to the final round.}\label{tab:H.7}
{\small\setlength{\tabcolsep}{6pt}\renewcommand{\arraystretch}{1.1}
\noindent\begin{adjustbox}{max width=\linewidth}
\begin{tabular}{rrrrrr}
\toprule
\textbf{options} & {\begin{tabular}[b]{@{}r@{}}\textbf{accuracy: 4B}\\\textbf{/ 9B / 27B}\end{tabular}} & {\begin{tabular}[b]{@{}r@{}}\textbf{correct option}\\\textbf{lost before the}\\\textbf{final round}\end{tabular}} & {\begin{tabular}[b]{@{}r@{}}\textbf{calibration}\\\textbf{error (\%)}\end{tabular}} & {\begin{tabular}[b]{@{}r@{}}\textbf{question}\\\textbf{rows}\\\textbf{per item}\end{tabular}} & {\begin{tabular}[b]{@{}r@{}}\textbf{prompt}\\\textbf{tokens}\\\textbf{per item}\end{tabular}} \\
\midrule
5 & 98.5 / 99.3 / 98.8 & -- & 0.43 / 0.50 / 0.50 & 1 & 104 \\
10 & 97.9 / 98.9 / 98.5 & -- & 0.75 / 0.66 / 0.45 & 1 & 134 \\
26 & 95.7 / 96.8 / 96.8 & -- & 1.52 / 1.10 / 0.98 & 1 & 229 \\
50 & 92.0 / 93.9 / 93.8 & 0.7\% / 0.3\% / 0.5\% & 0.80 / 1.08 / 1.36 & 3 & 558 \\
100 & 88.3 / 91.4 / 91.5 & 0.5\% / 0.4\% / 0.4\% & 2.28 / 1.59 / 2.32 & 5 & 1,262 \\
151 & 86.7 / 89.9 / 89.7 & 0.6\% / 0.2\% / 0.3\% & 2.85 / 1.96 / 3.04 & 8 & 1,929 \\
228 & 83.9 / 88.4 / 86.8 & 2.1\% / 1.5\% / 1.1\% & 2.65 / 2.42 / 3.80 & 13 & 3,679 \\
\bottomrule
\end{tabular}
\end{adjustbox}\par}
\end{table}

Keeping one, three or five options per group changes the accuracy by about a point at most. The
knock-out loses the correct option in the group stage in 0.2--0.7\% of the items up to 151 options
and 1.1--2.1\% at 228. What is lost beyond that is lost in the final round, among near-synonymous
labels.

\begin{table}[!htbp]
\renewcommand{\thetable}{H.8}
\centering
\caption{One position instead of a knock-out: options labelled A \ldots{} Z, AA, AB, \ldots{} (two-letter upper-case strings that are single tokens) and read at one position. Accuracy of the knock-out / of the one-position read-out on the items of Table~\ref{tab:H.7}. The last model column is a 4B after data rounds with one further low-rank round of 32 minutes on 21,000 long lists from the training splits of the two intent sources and 8,000 chord questions among 60,000 rows of the ordinary mix.}\label{tab:H.8}
{\small\setlength{\tabcolsep}{6pt}\renewcommand{\arraystretch}{1.1}
\noindent\begin{adjustbox}{max width=\linewidth}
\begin{tabular}{rrrrrr}
\toprule
\textbf{options} & {\begin{tabular}[b]{@{}r@{}}\textbf{4B released:}\\\textbf{knock-out /}\\\textbf{one position}\end{tabular}} & {\begin{tabular}[b]{@{}r@{}}\textbf{9B}\\\textbf{released}\end{tabular}} & {\begin{tabular}[b]{@{}r@{}}\textbf{4B after}\\\textbf{data}\\\textbf{rounds}\end{tabular}} & {\begin{tabular}[b]{@{}r@{}}\textbf{the same after}\\\textbf{one round on}\\\textbf{long lists}\end{tabular}} & {\begin{tabular}[b]{@{}r@{}}\textbf{prompt tokens:}\\\textbf{knock-out /}\\\textbf{one position}\end{tabular}} \\
\midrule
26 & 95.7 / 95.7 & 96.8 / 96.8 & 96.0 / 96.0 & 96.7 / 96.6 & 229 / 229 \\
50 & 92.0 / 90.9 & 93.9 / 78.5 & 93.3 / 88.9 & 94.2 / 94.1 & 558 / 372 \\
100 & 88.3 / 86.7 & 91.4 / 67.8 & 89.9 / 86.1 & 92.2 / 92.4 & 1,262 / 649 \\
151 & 86.7 / 85.1 & 89.9 / 66.4 & 88.5 / 86.1 & 90.6 / 91.4 & 1,929 / 906 \\
228 & 83.9 / 80.9 & 88.4 / 69.2 & 86.1 / 81.3 & 89.1 / 90.6 & 3,679 / 1,365 \\
\bottomrule
\end{tabular}
\end{adjustbox}\par}
\end{table}

The released 4B, which has never seen a two-letter label, is within 1.1 to 3.0 points of its
knock-out at 37--67\% of the tokens. The released 9B is not: it leaves about 40\% of the probability
on the 26 letters. After the short round the one-position read-out is within 0.1 points of the
knock-out or above it at every length.

\begin{table}[!htbp]
\renewcommand{\thetable}{H.9}
\centering
\caption{The long-list questions of the index, 4B after data rounds, before and after the round of Table~\ref{tab:H.8}.}\label{tab:H.9}
{\scriptsize\setlength{\tabcolsep}{4pt}\renewcommand{\arraystretch}{1.1}
\noindent\begin{adjustbox}{max width=\linewidth}
\begin{tabular}{lrrlrrr}
\toprule
\textbf{family of the index} & \textbf{questions} & {\begin{tabular}[b]{@{}r@{}}\textbf{options}\\\textbf{(mean)}\end{tabular}} & {\begin{tabular}[b]{@{}l@{}}\textbf{in the long-list}\\\textbf{round}\end{tabular}} & {\begin{tabular}[b]{@{}r@{}}\textbf{before the round:}\\\textbf{knock-out / one}\\\textbf{position}\end{tabular}} & {\begin{tabular}[b]{@{}r@{}}\textbf{after the round:}\\\textbf{knock-out / one}\\\textbf{position}\end{tabular}} & {\begin{tabular}[b]{@{}r@{}}\textbf{prompt tokens per}\\\textbf{question: knock-out}\\\textbf{/ one position}\end{tabular}} \\
\midrule
API-Bank, tool selection & 508 & 53.0 & no & 84.8 / 75.6 & 84.8 / 83.7 & 29,521 / 7,574 \\
BANKING77 & 1,000 & 77.0 & yes & 89.4 / 85.3 & 92.6 / 92.7 & 970 / 600 \\
CLINC150 with out-of-scope & 1,000 & 151.0 & yes & 86.8 / 84.6 & 88.8 / 90.2 & 1,480 / 839 \\
ChessBench, legal moves & 1,000 & 36.4 & no & 18.1 / 19.2 & 17.9 / 19.3 & 1,735 / 1,123 \\
POP909-CL, chords & 1,000 & 129.0 & generated chords & 78.5 / 79.5 & 79.6 / 80.8 & 22,416 / 6,714 \\
all five families & 4,508 & 93.2 &  & 70.1 / 68.1 & 71.4 / 72.2 & 9,228 / 2,911 \\
\bottomrule
\end{tabular}
\end{adjustbox}\par}
\end{table}

The alphabet carries over to lists of kinds the round has not seen (tool selection 75.6
$\rightarrow$ 83.7 at one position). The round itself behaves like any second-stage round: on the
ordinary index, read with the knock-out, the model scores 64.55 after it against 64.78 before, with
the two intent benchmarks up 3.2 and 1.6 skill points, the arts area down 2.6 and the appliance
simulator down 3.4. The longer alphabet therefore belongs in a full data round.

\subsection{Evidence-removal probes, full tables}\label{sec:H.7}

\begin{table}[!htbp]
\renewcommand{\thetable}{H.10}
\centering
\caption{First probe: 1,200 multi-hop claim-verification items of the index, 600 supported claims, one needed document removed at a time (1,814 variants). Own runs, 2026-10-06, 95\% bootstrap intervals.}\label{tab:H.10}
{\footnotesize\setlength{\tabcolsep}{5pt}\renewcommand{\arraystretch}{1.1}
\noindent\begin{adjustbox}{max width=\linewidth}
\begin{tabular}{>{\raggedright\arraybackslash}p{\mdw{0.1477}}>{\raggedleft\arraybackslash}p{\mdw{0.1326}}>{\raggedleft\arraybackslash}p{\mdw{0.2233}}>{\raggedleft\arraybackslash}p{\mdw{0.1357}}>{\raggedleft\arraybackslash}p{\mdw{0.1833}}>{\raggedleft\arraybackslash}p{\mdw{0.1644}}}
\toprule
\textbf{model} & \textbf{accuracy on the original items} & \textbf{change of P(supported) when a needed document is removed {[}95\%{]}} & \textbf{removals after which it is lower} & \textbf{removals after which the answer is ``not supported''} & \textbf{change when an unrelated document is added} \\
\midrule
4B starting model & 63.2 & $-$.166 {[}$-$.177, $-$.155{]} & 79\% & 50\% & $-$.03 \\
9B starting model & 78.5 & $-$.282 {[}$-$.299, $-$.266{]} & 86\% & 44\% & +.01 \\
27B starting model & 80.8 & $-$.434 {[}$-$.453, $-$.415{]} & 93\% & 62\% & $-$.02 \\
0.8B, released & 85.8 & $-$.313 {[}$-$.325, $-$.302{]} & 89\% & 68\% & $-$.01 \\
2B, released & 79.5 & $-$.305 {[}$-$.321, $-$.291{]} & 87\% & 63\% & $-$.01 \\
4B, released & 94.0 & $-$.460 {[}$-$.478, $-$.444{]} & 94\% & 62\% & $-$.00 \\
9B, released & 90.8 & $-$.509 {[}$-$.529, $-$.492{]} & 93\% & 70\% & +.00 \\
27B, released & 90.7 & $-$.608 {[}$-$.627, $-$.590{]} & 94\% & 80\% & +.01 \\
4B, after data rounds & 92.5 & $-$.511 {[}$-$.528, $-$.495{]} & 91\% & 69\% & $-$.01 \\
9B, after data rounds & 91.2 & $-$.509 {[}$-$.529, $-$.491{]} & 92\% & 68\% & $-$.00 \\
27B, after data rounds & 91.5 & $-$.559 {[}$-$.578, $-$.542{]} & 93\% & 74\% & +.00 \\
4B, after data rounds with evidence-removal rows & 91.2 & $-$.695 {[}$-$.713, $-$.678{]} & 99\% & 92\% & +.02 \\
\bottomrule
\end{tabular}
\end{adjustbox}\par}
\end{table}

A needed document replaced by an unrelated one has the effect of a removal ($-$.34 to $-$.64 for the
trained models). Reversing the order of the documents moves the probability by 0.02 at most. When a
claim has two documents and one is removed, the trained models from 4B on change their answer in
82--94\% of the cases, with three documents in 61--78\%, with four in 54--77\%. With the
evidence-removal rows the figures for three and four documents are 92\% and 88\%.

\begin{table}[!htbp]
\renewcommand{\thetable}{H.11}
\centering
\caption{Second probe: 1,000 questions from the validation split of a multi-hop question-answering set, with the gold answer as proposed answer and four paragraphs, two needed and two distractors, with each needed paragraph removed in turn (2,000 variants). The training split of this source is among our long-document training data in another layout.}\label{tab:H.11}
{\scriptsize\setlength{\tabcolsep}{4pt}\renewcommand{\arraystretch}{1.1}
\noindent\begin{adjustbox}{max width=\linewidth}
\begin{tabular}{>{\raggedright\arraybackslash}p{\mdw{0.1083}}>{\raggedleft\arraybackslash}p{\mdw{0.1008}}>{\raggedleft\arraybackslash}p{\mdw{0.1375}}>{\raggedleft\arraybackslash}p{\mdw{0.1048}}>{\raggedleft\arraybackslash}p{\mdw{0.0843}}>{\raggedleft\arraybackslash}p{\mdw{0.1366}}>{\raggedleft\arraybackslash}p{\mdw{0.1161}}>{\raggedleft\arraybackslash}p{\mdw{0.0840}}>{\raggedleft\arraybackslash}p{\mdw{0.1148}}}
\toprule
\textbf{model} & \textbf{accepts the complete item} & \textbf{change of P(yes) when a needed paragraph is removed {[}95\%{]}} & \textbf{removals after which it is lower} & \textbf{answer changes} & \textbf{\ldots{} when the answer is no longer mentioned in what is left} & \textbf{\ldots{} when it still is (answers other than yes / no)} & \textbf{rejects a wrong answer} & \textbf{change when a distractor is removed} \\
\midrule
4B starting model & 65.8 & $-$.230 {[}$-$.240, $-$.220{]} & 86\% & 51\% & 82\% & 38\% & 93\% & +.00 \\
9B starting model & 83.5 & $-$.405 {[}$-$.422, $-$.387{]} & 93\% & 52\% & 83\% & 40\% & 90\% & +.01 \\
27B starting model & 90.1 & $-$.601 {[}$-$.619, $-$.583{]} & 96\% & 74\% & 92\% & 64\% & 95\% & $-$.00 \\
0.8B, released & 98.7 & $-$.169 {[}$-$.175, $-$.164{]} & 92\% & 29\% & 49\% & 19\% & 49\% & +.01 \\
2B, released & 94.8 & $-$.285 {[}$-$.296, $-$.274{]} & 91\% & 42\% & 78\% & 24\% & 87\% & +.01 \\
4B, released & 94.1 & $-$.521 {[}$-$.537, $-$.506{]} & 96\% & 65\% & 87\% & 54\% & 97\% & +.00 \\
9B, released & 97.6 & $-$.527 {[}$-$.541, $-$.514{]} & 97\% & 64\% & 88\% & 52\% & 99\% & $-$.00 \\
27B, released & 95.1 & $-$.598 {[}$-$.614, $-$.583{]} & 96\% & 75\% & 95\% & 67\% & 100\% & $-$.00 \\
4B, after data rounds & 95.5 & $-$.519 {[}$-$.535, $-$.505{]} & 96\% & 64\% & 90\% & 52\% & 98\% & +.01 \\
9B, after data rounds & 97.4 & $-$.511 {[}$-$.526, $-$.497{]} & 97\% & 61\% & 87\% & 47\% & 99\% & $-$.00 \\
27B, after data rounds & 96.9 & $-$.530 {[}$-$.545, $-$.516{]} & 96\% & 68\% & 93\% & 57\% & 100\% & $-$.00 \\
4B, after data rounds with evidence-removal rows & 96.4 & $-$.626 {[}$-$.642, $-$.611{]} & 98\% & 74.5\% & 95\% & 66\% & 98\% & +.00 \\
\bottomrule
\end{tabular}
\end{adjustbox}\par}
\end{table}

\subsection{Outside sets in detail}\label{sec:H.8}

\clearpage
\begin{table}[!htbp]
\renewcommand{\thetable}{H.12}
\centering
\caption{CITY-Jev, released StartLux-Decision-4B, by task (own run, 2026-10-05, 12,000 decisions read, none failed, 87 questions with an input cut to the model's length limit of that run). Last column: the card's values for Jev 1.13.0. Abstention-aware accuracy counts an answer below confidence 0.5 as correct.}\label{tab:H.12}
{\scriptsize\setlength{\tabcolsep}{4pt}\renewcommand{\arraystretch}{1.1}
\noindent\begin{adjustbox}{max width=\linewidth}
\begin{tabular}{lrrrrrrr}
\toprule
\textbf{task} & \textbf{questions} & \textbf{excluded} & {\begin{tabular}[b]{@{}r@{}}\textbf{strict}\\\textbf{accuracy}\end{tabular}} & {\begin{tabular}[b]{@{}r@{}}\textbf{mean}\\\textbf{accuracy}\end{tabular}} & {\begin{tabular}[b]{@{}r@{}}\textbf{strict}\\\textbf{abstention-aware}\end{tabular}} & {\begin{tabular}[b]{@{}r@{}}\textbf{mean}\\\textbf{abstention-aware}\end{tabular}} & {\begin{tabular}[b]{@{}r@{}}\textbf{Jev 1.13.0 (card):}\\\textbf{strict / mean / strict}\\\textbf{AA / mean AA}\end{tabular}} \\
\midrule
Overall & 2000 & 0 & 64.95 & 72.95 & 84.65 & 89.94 & 74.52 / 78.92 / 85.31 / 88.78 \\
Safety Analysis & 450 & 0 & 67.11 & 77.30 & 89.56 & 93.70 & 84.22 / 87.78 / 90.89 / 93.15 \\
Outcome Verification & 235 & 0 & 62.98 & 70.00 & 83.40 & 86.03 & 74.24 / 78.97 / 82.10 / 85.01 \\
Action Selection & 452 & 0 & 79.42 & 83.44 & 92.26 & 95.58 & 83.14 / 85.80 / 92.38 / 95.73 \\
Evidence Assessment & 413 & 0 & 76.76 & 86.44 & 93.95 & 98.18 & 83.78 / 89.43 / 92.98 / 95.92 \\
Process Evaluation & 450 & 0 & 38.44 & 47.22 & 64.22 & 75.00 & 48.11 / 53.71 / 67.48 / 73.05 \\
\bottomrule
\end{tabular}
\end{adjustbox}\par}
\end{table}

\begin{table}[!htbp]
\renewcommand{\thetable}{H.13}
\centering
\caption{The same run by input version.}\label{tab:H.13}
{\small\setlength{\tabcolsep}{6pt}\renewcommand{\arraystretch}{1.1}
\noindent\begin{adjustbox}{max width=\linewidth}
\begin{tabular}{lrrrrrrr}
\toprule
\textbf{input version} & \textbf{accuracy} & {\begin{tabular}[b]{@{}r@{}}\textbf{decision}\\\textbf{differs from}\\\textbf{the original}\end{tabular}} & \textbf{abstained} & {\begin{tabular}[b]{@{}r@{}}\textbf{error}\\\textbf{among}\\\textbf{answered}\end{tabular}} & {\begin{tabular}[b]{@{}r@{}}\textbf{error at}\\\textbf{80\%}\\\textbf{coverage}\end{tabular}} & {\begin{tabular}[b]{@{}r@{}}\textbf{ECE}\\\textbf{of}\\\textbf{p\_max}\end{tabular}} & {\begin{tabular}[b]{@{}r@{}}\textbf{mean}\\\textbf{p\_max}\end{tabular}} \\
\midrule
v0\_original & 72.70 & 0.00\% & 38.20\% & 15.70\% & 21.75\% & 0.041 & 0.764 \\
v1\_order & 73.30 & 7.75\% & 38.60\% & 16.12\% & 20.69\% & 0.045 & 0.766 \\
v2\_label & 73.65 & 3.95\% & 36.40\% & 16.04\% & 21.25\% & 0.050 & 0.770 \\
v3\_format & 72.75 & 5.55\% & 39.90\% & 15.39\% & 21.31\% & 0.044 & 0.754 \\
v4\_context & 71.80 & 7.75\% & 35.50\% & 16.20\% & 22.81\% & 0.061 & 0.775 \\
v5\_paraphrase & 73.50 & 5.30\% & 36.80\% & 17.17\% & 21.38\% & 0.046 & 0.772 \\
\bottomrule
\end{tabular}
\end{adjustbox}\par}
\end{table}

The 4B answers below confidence 0.5 twice as often as the hosted model (37.6\% against 19.4\%), and
so comes within a point of the card's abstention-aware scores (84.65 and 89.94 against 85.31 and
88.78) while being 6 to 10 points less accurate. The metric rewards not answering.

\begin{table}[!htbp]
\renewcommand{\thetable}{H.14}
\centering
\caption{CJ-Bench by question type, accuracy in percent (number of decisions).}\label{tab:H.14}
{\small\setlength{\tabcolsep}{6pt}\renewcommand{\arraystretch}{1.1}
\noindent\begin{adjustbox}{max width=\linewidth}
\begin{tabular}{llrrr}
\toprule
\textbf{domain} & \textbf{model} & \textbf{choice} & \textbf{yes/no} & \textbf{score} \\
\midrule
general & StartLux-Decision-27B & 75.1 (33,334) & 84.3 (33,333) & 46.6 (30,255) \\
general & StartLux-Decision-9B & 70.7 (33,334) & 82.3 (33,333) & 46.0 (30,255) \\
general & StartLux-Decision-4B & 68.6 (33,334) & 82.9 (33,333) & 41.8 (30,255) \\
medical & StartLux-Decision-27B & 75.2 (98,543) & 95.9 (98,544) & 41.5 (2,913) \\
medical & StartLux-Decision-9B & 69.2 (98,543) & 95.2 (98,544) & 42.7 (2,913) \\
medical & StartLux-Decision-4B & 69.1 (98,543) & 95.2 (98,544) & 42.0 (2,913) \\
legal & StartLux-Decision-27B & 75.7 (1,500) & 79.1 (1,500) & 63.2 (1,300) \\
legal & StartLux-Decision-9B & 65.8 (1,500) & 76.3 (1,500) & 54.0 (1,300) \\
legal & StartLux-Decision-4B & 60.5 (1,500) & 74.3 (1,500) & 55.3 (1,300) \\
finance & StartLux-Decision-27B & 76.2 (1,200) & 84.2 (1,200) & 80.2 (1,200) \\
finance & StartLux-Decision-9B & 71.7 (1,200) & 80.9 (1,200) & 74.6 (1,200) \\
finance & StartLux-Decision-4B & 67.7 (1,200) & 77.3 (1,200) & 66.4 (1,200) \\
\bottomrule
\end{tabular}
\end{adjustbox}\par}
\end{table}

\begin{table}[!htbp]
\renewcommand{\thetable}{H.15}
\centering
\caption{Option-order probe on 4,570 index items (evaluation only, own runs, 2026-10-04): accuracy in the stored order, in a permuted order and with the distributions averaged over orders, and share of items whose top answer changes with the order.}\label{tab:H.15}
{\small\setlength{\tabcolsep}{6pt}\renewcommand{\arraystretch}{1.1}
\noindent\begin{adjustbox}{max width=\linewidth}
\begin{tabular}{llrrrrr}
\toprule
\textbf{model} & \textbf{items} & \textbf{n} & {\begin{tabular}[b]{@{}r@{}}\textbf{original}\\\textbf{order}\end{tabular}} & {\begin{tabular}[b]{@{}r@{}}\textbf{permuted}\\\textbf{order}\end{tabular}} & {\begin{tabular}[b]{@{}r@{}}\textbf{average}\\\textbf{over}\\\textbf{orders}\end{tabular}} & {\begin{tabular}[b]{@{}r@{}}\textbf{top answer}\\\textbf{changes with}\\\textbf{the order}\end{tabular}} \\
\midrule
\mdourrow StartLux-Decision-4B, released & all & 4,570 & 70.94 & 71.00 & 71.49 & 15.10\% \\
\mdourrow StartLux-Decision-4B, released & content options & 1,920 & 64.22 & 64.10 & 65.00 & 21.72\% \\
\mdourrow StartLux-Decision-4B, released & label options & 2,650 & 75.81 & 76.00 & 76.19 & 10.30\% \\
\mdourrow StartLux-Decision-9B, released & all & 4,570 & 73.68 & 73.33 & 73.89 & 11.68\% \\
\mdourrow StartLux-Decision-9B, released & content options & 1,920 & 69.11 & 68.75 & 69.43 & 16.04\% \\
\mdourrow StartLux-Decision-9B, released & label options & 2,650 & 76.98 & 76.65 & 77.13 & 8.53\% \\
4B starting model & all & 4,570 & 58.67 & 59.51 & 61.51 & 37.35\% \\
4B starting model & content options & 1,920 & 48.18 & 48.84 & 52.34 & 45.42\% \\
4B starting model & label options & 2,650 & 66.26 & 67.25 & 68.15 & 31.51\% \\
\bottomrule
\end{tabular}
\end{adjustbox}\par}
\end{table}

\subsection{Notes on benchmark artefacts}\label{sec:H.9}

\begin{itemize}
\item \textbf{A formatting mark that gives the answer.} In the company-events subset of SATA-Bench 339
options begin with a blank and all 339 are correct. Our models do not use the mark. Our training
rows carry a leading blank on one option in four at random.
\item \textbf{Test items inside public training splits.} For four of the six upstream sources of that
benchmark, 910 of 1,048 evaluation rows are in the upstream training files (284 of 284, 176 of 249,
265 of 311, 185 of 204). Training on those corpora without a lookup by text trains on test items.
Our rows are filtered by text.
\item \textbf{A benchmark below chance.} On HLE every model of ours answers 8.6--13.8\% correctly against
a chance level of 16.4\%, with or without reasoning. It contributes zero to every index value in
this report.
\item \textbf{A labelling model's ceiling.} Typed Decisions, Section~\ref{sec:H.2}.
\item \textbf{A prior measured as a skill.} API-Bank shows its full catalogue of 53 tools in every item,
also where a tool search is the expected first call. Three fixed patterns account for the errors of
all our models on its 508 items.
\item \textbf{Stored layouts.} Two families are stored with sorted keys. Rows written in the source's
order differ from what the model is shown at test time.
\end{itemize}

\subsection{Sets with pending rows}\label{sec:H.10}

\textbf{Reranking test.} Item file: the test queries, the 50 candidates of each query in the order
of the hybrid search, the relevance judgements, and the published ranking of every reference arm,
from which we reproduce every published number. Three request forms are run for each of our models:
the rubric request registered for decision models (three requests of 17, 17 and 16 passages, one
four-level question per passage, relevance = expected level / 3), the same rubric with one passage
per request, and our yes/no retrieval layout with relevance = P(yes). Scoring: nDCG@10 with linear
gain, ties by document identifier, paired bootstrap over queries with 10,000 resamples.

\begin{table}[!htbp]
\renewcommand{\thetable}{H.17}
\centering
\caption{Reranking test, nDCG@10 (SciFact / NFCorpus) for the three request forms. Own runs of 2026-10-07.}\label{tab:H.17}
{\small\setlength{\tabcolsep}{6pt}\renewcommand{\arraystretch}{1.1}
\noindent\begin{adjustbox}{max width=\linewidth}
\begin{tabular}{lrrr}
\toprule
\textbf{model} & {\begin{tabular}[b]{@{}r@{}}\textbf{registered}\\\textbf{request (17 / 17}\\\textbf{/ 16 passages)}\end{tabular}} & {\begin{tabular}[b]{@{}r@{}}\textbf{one passage}\\\textbf{per request,}\\\textbf{rubric}\end{tabular}} & {\begin{tabular}[b]{@{}r@{}}\textbf{one passage}\\\textbf{per request,}\\\textbf{yes/no layout}\end{tabular}} \\
\midrule
4B, released & 0.788 / 0.381 & 0.774 / 0.404 & 0.770 / 0.417 \\
4B, after data rounds & 0.785 / 0.391 & 0.783 / 0.425 & 0.771 / 0.430 \\
9B, released & 0.794 / 0.388 & 0.792 / 0.414 & 0.807 / 0.422 \\
9B, after data rounds & 0.806 / 0.409 & 0.810 / 0.414 & 0.807 / 0.424 \\
27B, released & 0.828 / 0.435 & 0.821 / 0.434 & 0.808 / 0.442 \\
27B, after data rounds & 0.836 / 0.436 & 0.825 / 0.428 & 0.809 / 0.438 \\
\bottomrule
\end{tabular}
\end{adjustbox}\par}
\end{table}

Many passages in one request cost the small models on NFCorpus (4B: 0.381 to 0.391 against 0.404 to
0.430 one passage at a time) and help the 27B on SciFact.

\textbf{Option-reversal safety set.} One choice question per request with the row's options in the
row's order, the small panels (XSTest, OR-Bench Hard and Toxic, HarmBench text) in three views, the
80K panel in two. A smoke test of 66 pairs with the 4B after data rounds changed no answer under
reversal. \todo{run pending}

\textbf{Capability-boundary pilot.} 10,976 requests that ask for the probability that a named model
answers a question correctly, built from stored answers of public chat models on arithmetic,
open-domain and reasoning questions. The hosted reference answered all requests (API run of
2026-10-06 to 10-07): its probability separates right from wrong answers with an AUROC of 0.727 from
the model card alone and 0.762 with a track record of eight questions, and as a probability it is on
average no better than quoting the base rate (mean skill $-$0.21 and $-$0.02).

\begin{table}[!htbp]
\renewcommand{\thetable}{H.18}
\centering
\caption{Capability-boundary pilot (10,976 requests, every system answered all of them, own runs of 2026-10-07, hosted reference by API). Mean over the cells (domain $\times$ answering model) of the AUROC against ``right more often than not'' and of the skill, 1 $-$ MSE / MSE of the cell's own mean success rate with the sampling noise of the label removed. Card: the state names the answering model. Record: it also lists eight other questions of the domain with that model's results.}\label{tab:H.18}
{\small\setlength{\tabcolsep}{6pt}\renewcommand{\arraystretch}{1.1}
\noindent\begin{adjustbox}{max width=\linewidth}
\begin{tabular}{lrrrr}
\toprule
\textbf{system} & {\begin{tabular}[b]{@{}r@{}}\textbf{card:}\\\textbf{AUROC}\end{tabular}} & {\begin{tabular}[b]{@{}r@{}}\textbf{card:}\\\textbf{skill}\end{tabular}} & {\begin{tabular}[b]{@{}r@{}}\textbf{record:}\\\textbf{AUROC}\end{tabular}} & {\begin{tabular}[b]{@{}r@{}}\textbf{record:}\\\textbf{skill}\end{tabular}} \\
\midrule
hosted reference (Jev 1.13) & 0.727 & $-$0.212 & 0.762 & $-$0.024 \\
4B, released & 0.716 & $-$0.368 & 0.719 & $-$0.117 \\
9B, released & 0.731 & $-$0.214 & 0.730 & $-$0.140 \\
27B, released & 0.741 & $-$0.297 & 0.788 & $-$0.046 \\
4B, after data rounds & 0.707 & $-$0.486 & 0.704 & $-$0.184 \\
9B, after data rounds & 0.728 & $-$0.262 & 0.738 & $-$0.085 \\
27B, after data rounds & 0.704 & $-$0.877 & 0.798 & +0.024 \\
\bottomrule
\end{tabular}
\end{adjustbox}\par}
\end{table}

No system's probabilities beat the base rate of the answering model by more than 0.03 in skill (one
cell is +0.024). Ranking is moderate, and only the 27B models and the hosted reference use the track
record. The data rounds do not help this decision, which no training source asks for, and make the
card-only probabilities of the 27B worse.

\subsection{Evaluation sets and their role}\label{sec:H.11}

\begin{table}[!htbp]
\renewcommand{\thetable}{H.16}
\centering
\caption{Evaluation sets of Chapter~\ref{sec:6}, their size and their role for our models. \ddag{}: training data aimed at the set is in our training mix.}\label{tab:H.16}
{\footnotesize\setlength{\tabcolsep}{5pt}\renewcommand{\arraystretch}{1.1}
\noindent\begin{adjustbox}{max width=\linewidth}
\begin{tabular}{>{\raggedright\arraybackslash}p{\mdw{0.1635}}>{\raggedright\arraybackslash}p{\mdw{0.4112}}>{\raggedright\arraybackslash}p{\mdw{0.4112}}}
\toprule
\textbf{set} & \textbf{size} & \textbf{role for our models} \\
\midrule
Decision Index 0.2.1 \ddag{} & 38 benchmarks, 133,876 requests & development set \\
JevBench public tiers & 231 items & run for release candidates, in a seven-suite average that was watched while choosing checkpoints \\
Typed Decisions, test split \ddag{} & 400 cases, 2,000 decisions & in-domain: the training split is in every mix \\
long-document sets & LongBench v2 (297 items up to 128K tokens), needle items up to 248K, 1,690 held-out questions & evaluation only \\
image sets & eight public sets & zero-shot: no image in training \\
CJ-Bench (Chinese) & 307,900 decisions, 304,822 scored & zero-shot, evaluation only \\
CITY-Jev & 2,000 decisions $\times$ 6 input versions & evaluation only \\
option-reversal safety set & 83,183 requests in up to three views & evaluation only \\
reranking test & 200 queries $\times$ 50 candidates & evaluation only \\
held-out pool & 8,598 items of sources that are not in the final mix & never trained on \\
diagnostic decisions & 5,710 items in 39 families of benchmark type & items never trained on, families not held out \\
evidence-removal probes & 1,200 claims, 1,000 questions & evaluation only \\
\bottomrule
\end{tabular}
\end{adjustbox}\par}
\end{table}
