# Supplementary material for: StartLux-Decision: AutoThink Decision Models with Reinforcement Learning for Calibrated Deliberative Decisions
Source: arXiv:2610.17309 source file (2026-10-20)
Supplement: Supplementary file 16 [file appendix_J_serving.tex]

\clearpage
\setcounter{section}{9}
\section{Serving details}\label{sec:J}

\subsection{Software}\label{sec:J.1}

\textbf{Released runtime.} The inference package is tested with PyTorch 2.11, transformers 5.8.1,
flash-linear-attention 0.5.2 and causal-conv1d 1.7.0 on H200 GPUs. The last two are the kernel
packages of the linear-attention layers and are required on CUDA. A check command reports whether
they are active for a model, and the server refuses to start without them unless a variable is set
that allows the slow path. Image input needs the image processor of the checkpoint. On Apple Silicon
the forward pass runs in MLX (mlx-lm 0.31.3 or newer). GGUF files need a llama.cpp build of b10454
or newer. \todo{driver, CUDA and cuDNN versions of the machines behind Table 8.1}

\textbf{Reasoning runs.} The thoughts of all reasoning runs are generated by vLLM 0.19.1 servers,
one per GPU, with the settings of Section~\ref{sec:J.2}. The one-pass read-outs of a reasoning run
go through the same servers. The one-pass index runs go through the batch runner, which uses the
read-out code of the released package.

\subsection{The reasoning server}\label{sec:J.2}

A reasoning run has three layers on one node of eight GPUs. There are eight generation servers, one
per GPU. In front of each server is one reasoning process, which implements the five steps of
Section~\ref{sec:3.4} for every question. In front of the eight reasoning processes is a load
balancer, to which 512 concurrent clients send the requests. Each server is started with

\begin{lstlisting}
python3 -m vllm.entrypoints.openai.api_server --model <checkpoint> --max-model-len 65536
    --gpu-memory-utilization 0.88 --logprobs-mode processed_logprobs --max-logprobs 26 --generation-config vllm
    --no-enable-prefix-caching --no-enable-chunked-prefill --max-num-batched-tokens 65536
    --limit-mm-per-prompt '{"image":0,"video":0}'
\end{lstlisting}

The first three options after the memory setting make the read-out exact: the 26 letter
log-probabilities are returned after the server's own processing and without the sampling defaults
stored in the checkpoint, which would truncate the letter distribution. The next three are the
corrections of Section~\ref{sec:8.4}. The context of these servers is 65,536 tokens because index
inputs are short. The released runtime reads 262,144.

\begin{table}[!htbp]
\renewcommand{\thetable}{J.1}
\centering
\caption{Settings of the reasoning process in the index runs of this report.}\label{tab:J.1}
{\footnotesize\setlength{\tabcolsep}{5pt}\renewcommand{\arraystretch}{1.1}
\noindent\begin{adjustbox}{max width=\linewidth}
\begin{tabular}{>{\raggedright\arraybackslash}p{\mdw{0.2080}}>{\raggedright\arraybackslash}p{\mdw{0.7777}}}
\toprule
\textbf{setting} & \textbf{value} \\
\midrule
rule & reason when the top one-pass probability is below 0.9 \\
mixture & 0.5 $\times$ one-pass distribution + 0.5 $\times$ distribution after the thought \\
thought budget & 4,096 tokens, or what is left of the context \\
opening of the thought & ``Let me work through this carefully, step by step.'' \\
sampling & temperature 0.6, top-p 0.95, top-k 20. The seed is derived from the prompt (a repeated run still differs through batch numerics: 97.0\% of the answers are the same choice) \\
stop & the closing mark of the thought \\
loop guard & on in runs ``with the detector'': the thought is generated 1,024 tokens at a time and ended when its tail is a loop (rules in Appendix~\ref{sec:J.2}) \\
read-back & the last 4,000 characters of the thought, marked as cut when longer \\
a thought that reaches the budget & the sentence ``I have to decide now with what I have worked out so far.'' and the closing mark are appended \\
temperature after the thought & 1 \\
reasoning requests & sent to a server in waves: everything queued goes out at once, and the next wave starts when the whole wave has finished \\
recorded per answer & both distributions and the thought length, so a run can be replayed at any threshold and mixture \\
\bottomrule
\end{tabular}
\end{adjustbox}\par}
\end{table}

Three details differ from the released one-pass package and matter for reproduction. For a list of
more than 26 options the reasoning process reads the groups of the first round at once, keeps the
best three of each group, and if more than 26 options reach the final it keeps the 26 with the
highest first-round probability, where the released package runs a further knock-out round. The
\texttt{confidence} field of this process is the top probability, not the formulas of
Table~\ref{tab:3.1}. The index scorer does not read it. And a request can override the rule per call
(never reason, always reason, or the rule).

\subsection{Formats and precisions}\label{sec:J.3}

\begin{table}[!htbp]
\renewcommand{\thetable}{J.2}
\centering
\caption{FP8 weights and activations (dynamic activation scales, per-row weight scales on the text layers, with the letter read-out kept in bf16) against bf16 on 2,541 decisions (JevBench public, Typed Decisions test, ToolACE test).}\label{tab:J.2}
{\small\setlength{\tabcolsep}{6pt}\renewcommand{\arraystretch}{1.1}
\noindent\begin{adjustbox}{max width=\linewidth}
\begin{tabular}{lrr}
\toprule
\textbf{model} & {\begin{tabular}[b]{@{}r@{}}\textbf{same}\\\textbf{option}\\\textbf{as bf16}\end{tabular}} & {\begin{tabular}[b]{@{}r@{}}\textbf{accuracy}\\\textbf{bf16 $\rightarrow$ FP8}\end{tabular}} \\
\midrule
StartLux-Decision-0.8B & 96.3\% & 78.00 $\rightarrow$ 77.76 \\
StartLux-Decision-2B & 96.5\% & 80.44 $\rightarrow$ 80.05 \\
StartLux-Decision-4B & 98.0\% & 82.37 $\rightarrow$ 81.98 \\
StartLux-Decision-9B & 98.2\% & 83.67 $\rightarrow$ 83.23 \\
StartLux-Decision-27B & 98.6\% & 82.96 $\rightarrow$ 82.76 \\
\bottomrule
\end{tabular}
\end{adjustbox}\par}
\end{table}

FP8 is a memory option: the weights of the 27B take 27.5 GiB on the GPU, but in this test FP8 was
about 2.7 times slower per decision than bf16, both run with one question per forward pass. With
padded batches an all-zero padding row gets a zero scale and produces NaN that leaks into real rows
through attention, and agreement with bf16 fell to about 52\%. FP8 must be run one question per
forward pass without padding.

\begin{table}[!htbp]
\renewcommand{\thetable}{J.3}
\centering
\caption{GGUF files for llama.cpp against the original weights on the 231 public JevBench items, same machine and same decision code in front of both.}\label{tab:J.3}
{\small\setlength{\tabcolsep}{6pt}\renewcommand{\arraystretch}{1.1}
\noindent\begin{adjustbox}{max width=\linewidth}
\begin{tabular}{lrrr}
\toprule
\textbf{model} & {\begin{tabular}[b]{@{}r@{}}\textbf{file size, BF16 /}\\\textbf{Q8\_0 / Q4\_K\_M}\end{tabular}} & {\begin{tabular}[b]{@{}r@{}}\textbf{same decision}\\\textbf{as the original}\end{tabular}} & {\begin{tabular}[b]{@{}r@{}}\textbf{correct of 231:}\\\textbf{original, BF16 /}\\\textbf{Q8\_0 / Q4\_K\_M}\end{tabular}} \\
\midrule
StartLux-Decision-0.8B & 1.52 / 0.81 / 0.53 GB & 99.6\% / 100.0\% / 93.1\% & 177, 178 / 177 / 172 \\
StartLux-Decision-2B & 3.78 / 2.01 / 1.27 GB & 100.0\% / 99.1\% / 94.4\% & 195, 195 / 193 / 199 \\
StartLux-Decision-4B & 8.42 / 4.48 / 2.71 GB & 100.0\% / 100.0\% / 98.3\% & 204, 204 / 204 / 201 \\
StartLux-Decision-9B & 17.92 / 9.53 / 5.63 GB & 99.6\% / 100.0\% / 98.3\% & 200, 201 / 200 / 201 \\
StartLux-Decision-27B & 53.81 / 28.60 / 16.55 GB & 100.0\% / 100.0\% / 96.5\% & 209, 209 / 209 / 208 \\
\bottomrule
\end{tabular}
\end{adjustbox}\par}
\end{table}

BF16 and Q8\_0 give the original answer on 99 to 100\% of the items. Q4\_K\_M keeps 96.5 to 98.3\%
from 4B up and changes more answers at 0.8B and 2B, where Q8\_0 is the better choice. The
``original'' counts of this table differ from Table~\ref{tab:6.3} by one or two items of rounding
between two inference paths of the same weights. The GGUF files hold the text decoder only. The
35B-A3B is not available as GGUF.

\textbf{MLX.} On Apple Silicon the forward pass runs in MLX with its own kernels for the
linear-attention layers. Prompts, read-out, temperatures and the knock-out are the package's code.
In bf16 the public JevBench counts of the 0.8B, 2B, 4B and 9B are the published ones. An int8 mode
for the large projections matches bf16 on 97.4 to 99.6\% of the public JevBench items, and an 8-bit
conversion of the 27B answers 208 of 231 where bf16 answers 209. The MLX and GGUF backends read text
only, and the MLX backend does not run the mixture-of-experts model.

\subsection{Recorded graphs and padding}\label{sec:J.4}

At start-up the released server records CUDA graphs in one shared memory pool: for a single question
one graph per padded length of 128, 192, 256, 320, 384, 512, 640, 768, 1,024, 1,536, 2,048, 3,072
and 4,096 tokens, and for two, three and four questions one per length up to 1,024 tokens, 40 graphs
in all. The experts of the 35B-A3B run as grouped matrix multiplications with no synchronisation
with the host, so they are recorded as well. A short request is padded on the right to the next
recorded length and replayed. Requests with more or longer questions, and all requests with images,
run unrecorded as one batch, padded to a fixed ladder of lengths because the linear-attention
kernels are compiled once per sequence length. One request is run through both paths at start-up,
and the graphs are dropped if a probability differs by more than 0.02. The difference is 0.0 for all
six models.

Bulk work goes through a second entry point that sorts every question of every request by length and
packs them into padded forward passes of up to 65,536 tokens. On a random 2\% of the index (2,678
requests, 6,897 questions) and one H200 the 4B took 140 s this way, against 337 s with one request
at a time through the recorded graphs and 254 s with one request at a time without them. Graphs help
single short requests and not this mix. The same option was chosen for 99.94\% of the questions, and
on 981 JevBench and Typed Decisions questions the largest difference of a probability was 0.008. A
full index run of the 4B took about 25 minutes on five H200s (about 1.9 GPU-hours with model loading
and kernel compilation).

\subsection{\texorpdfstring{Reproducing the faults of Section~\ref{sec:8.4}}{Reproducing the faults of Section 8.4}}\label{sec:J.5}

\textbf{Prefix caching.} Send the same rows twice to one server under the same load, once with the
cache shared between calls and once with a fresh cache key per call, and compare the one-pass
read-outs. With caching on we found 2.6\% of the ordinary read-outs moved by more than 0.05 (top
option the same in 97.4\%) and 16\% of the answers on lists over 26 options changed. Without any
caching two passes over the same rows still disagreed on 0.5\% of ordinary questions and 6\% of
long-list questions under the default prefill, which is consistent with the fault of the next
paragraph.

\textbf{Chunked prefill.} Run a model in one pass through the generation servers and through the
batch runner of the released package, on benchmarks with long lists and with several questions per
request, and count answers with the same choice. Table~\ref{tab:J.4} is this test for the 4B after
data rounds on seven benchmarks (12,347 to 12,455 requests per setting).

\begin{table}[!htbp]
\renewcommand{\thetable}{J.4}
\centering
\caption{One-pass answers of the same weights through the generation servers and through the batch runner (2026-10-06): share of answers with the same choice and, for the three benchmarks that showed the fault, accuracy through the servers / through the batch runner.}\label{tab:J.4}
{\scriptsize\setlength{\tabcolsep}{4pt}\renewcommand{\arraystretch}{1.1}
\noindent\begin{adjustbox}{max width=\linewidth}
\begin{tabular}{>{\raggedright\arraybackslash}p{\mdw{0.1491}}>{\raggedleft\arraybackslash}p{\mdw{0.1733}}>{\raggedleft\arraybackslash}p{\mdw{0.1047}}>{\raggedleft\arraybackslash}p{\mdw{0.1101}}>{\raggedleft\arraybackslash}p{\mdw{0.1513}}>{\raggedleft\arraybackslash}p{\mdw{0.1016}}>{\raggedleft\arraybackslash}p{\mdw{0.1064}}>{\raggedleft\arraybackslash}p{\mdw{0.0905}}}
\toprule
\textbf{server setting} & \textbf{API-Bank: same choice, accuracy server / batch runner} & \textbf{POP909-CL} & \textbf{appliance simulator} & \textbf{BANKING77: same choice} & \textbf{CLINC150} & \textbf{CRUXEval} & \textbf{BRIGHT} \\
\midrule
prefill in chunks of 8,192 batched tokens (as before) & 96.0\%, 82.83 / 85.23 & 93.9\%, 76.41 / 80.28 & 98.4\%, 98.07 / 99.65 & 99.5\% & 99.3\% & 98.2\% & 100.0\% \\
the same with a cache key per call & 93.5\%, 80.36 / 85.12 & 93.8\%, 76.45 / 80.29 & 98.5\%, 98.11 / 99.65 & 99.4\% & 99.3\% & 98.4\% & 100.0\% \\
chunked prefill with 65,536 batched tokens & 99.0\%, 84.98 / 85.18 & 98.6\%, 79.88 / 80.23 & 99.8\%, 99.48 / 99.69 & 99.5\% & 99.6\% & 98.2\% & 100.0\% \\
one sequence at a time & 99.4\%, 85.01 / 85.21 & 98.9\%, 80.30 / 80.35 & 100.0\%, 99.65 / 99.65 & 99.6\% & 99.6\% & 98.2\% & 100.0\% \\
no chunked prefill, 65,536 batched tokens & 99.4\%, 84.75 / 85.15 & 99.3\%, 80.29 / 80.34 & 100.0\%, 99.65 / 99.65 & 99.6\% & 99.6\% & 98.2\% & 100.0\% \\
corrected launcher, second run & 99.4\%, 85.04 / 85.24 & 99.1\%, 80.30 / 80.35 & 100.0\%, 99.65 / 99.65 & 99.6\% & 99.5\% & 97.7\% & 100.0\% \\
\bottomrule
\end{tabular}
\end{adjustbox}\par}
\end{table}

A cache key per call does not remove the fault, so it is not a caching fault. A larger token budget
per step, one sequence at a time and prefill in one piece all do.

\begin{table}[!htbp]
\renewcommand{\thetable}{J.5}
\centering
\caption{Where the two paths part, by kind of question and request length: one-pass path of a 4B recorded by a reasoning run on the earlier servers against the same model in the batch runner.}\label{tab:J.5}
{\small\setlength{\tabcolsep}{6pt}\renewcommand{\arraystretch}{1.1}
\noindent\begin{adjustbox}{max width=\linewidth}
\begin{tabular}{lrrrr}
\toprule
{\begin{tabular}[b]{@{}l@{}}\textbf{kind of}\\\textbf{question}\end{tabular}} & \textbf{request tokens} & \textbf{answers} & {\begin{tabular}[b]{@{}r@{}}\textbf{same}\\\textbf{top}\\\textbf{option}\end{tabular}} & {\begin{tabular}[b]{@{}r@{}}\textbf{top probability}\\\textbf{moved by}\\\textbf{more than 0.05}\end{tabular}} \\
\midrule
ordinary & 0--1,000 & 111,123 & 98.94\% & 0.40\% \\
ordinary & 1,000--2,000 & 38,620 & 97.80\% & 1.23\% \\
ordinary & 2,000--4,000 & 5,899 & 98.75\% & 1.36\% \\
ordinary & 4,000--8,192 & 113,762 & 99.92\% & 0.01\% \\
ordinary & 8,192--16,384 & 24,856 & 99.82\% & 0.00\% \\
ordinary & 16,384 and more & 14,255 & 99.81\% & 0.00\% \\
long list & 0--1,000 & 6,492 & 96.50\% & 0.00\% \\
long list & 1,000--2,000 & 5,509 & 99.36\% & 0.00\% \\
long list & 2,000--4,000 & 1,988 & 89.59\% & 0.00\% \\
long list & 4,000--8,192 & 511 & 84.34\% & 0.00\% \\
\bottomrule
\end{tabular}
\end{adjustbox}\par}
\end{table}

Ordinary questions agree in 97.8 to 99.9\% whatever their length. Long lists in requests of 2,000 to
8,192 tokens agree in 84 to 90\%.

\textbf{Stored thoughts re-read.} The offline engine that produced the diagnostic read-outs of
Chapter~\ref{sec:7} had the same default. Re-reading 5,710 stored items with prefill in one piece:
the one-pass answer has the same top option in 99.12\% (4B) and 99.40\% (9B) of the items and the
answer after the thought in 99.56\% and 99.65\%. A top probability moves by more than 0.05 in 0.02
to 0.14\% of the items. Accuracy changes by at most 0.11 points, and the difference in accuracy
between routed and kept answers at matched confidence is $-$0.093 before and $-$0.094 after at 4B,
$-$0.103 and $-$0.102 at 9B.

\textbf{The two prefill kernels.} The server has two kernels for the prefill of the linear-attention
layers. With the second one, on the seven benchmarks of Table~\ref{tab:J.4} (12,455 requests, none
failed), 99.82\% of 34,677 answers have the same choice as with the default kernel and the
probability of the chosen option differs by 0.0019 on average. Two runs with the default kernel
differ by 99.77\% and 0.0022. The run took 186 s against 162 s.

\subsection{Operations}\label{sec:J.6}

\textbf{Watchdog.} Every 30 seconds each generation server is asked for its counters. A server
counts as stopped when it has requests running and its prompt and generation token counters have not
moved for 120 seconds, or when it has answered before and does not answer for 120 seconds. The
watchdog then writes the state of the server's threads next to the server log, ends the processes
and starts the server again with the same command line, environment and log file, at most three
times per server. By default it restarts a stopped server with the second prefill kernel.

\textbf{What a stop looks like.} The main thread of the engine waits for the result of the step it
submitted. The worker thread waits for the event that marks the end of that step on the GPU,
spinning at full load of one core while the GPU shows full utilisation. The step never ends on the
device. No device error is logged. Requests in flight at the stops we recorded were ordinary
reasoning requests of different benchmarks, and all of them went through when sent again.

\textbf{Balancer.} Each request goes to the healthy reasoning process with the fewest requests in
flight. A failed request is sent to up to two other processes before the failure is passed on. A
process that fails three times in a row is left out for 30 seconds and then tried with a single
request. The limit on open files is raised to the hard limit, because every request in flight holds
two sockets.

\textbf{Retry passes.} After the first pass every request without an answer is sent again, in up to
three rounds with a pause between them. Results of later rounds replace failed rows. A run enters a
table only with a coverage of at least 0.999. One 4B run that ended at a coverage of 0.960 scored
61.31. With its 5,606 missing requests answered it scores 66.36.

\textbf{Counts.} Five stops in about 110 server-hours until 6 October 17:00, four of them on 4B
runs. One run of the 4B with three stops lost no request. One 27B run with one stop among 32 servers
had 395 failed requests, all answered in its retry pass.

\subsection{Decisions per request, all sizes}\label{sec:J.7}

\begingroup
\renewcommand{\thetable}{J.6}
\small\setlength{\tabcolsep}{6pt}\renewcommand{\arraystretch}{1.1}
\begin{longtable}{rrrrrrr}
\caption{Decisions per second for a request with the given number of yes/no questions about one document, released runtime (document shared from 4,096 tokens), released weights, one H200, bf16, 2026-10-06.}\label{tab:J.6}\\
\toprule
{\begin{tabular}[b]{@{}r@{}}\textbf{document}\\\textbf{tokens}\end{tabular}} & \textbf{questions} & \textbf{0.8B} & \textbf{2B} & \textbf{4B} & \textbf{9B} & \textbf{27B} \\
\midrule
\endfirsthead
\multicolumn{7}{l}{\textit{Table~\thetable{} (continued)}}\\
\toprule
{\begin{tabular}[b]{@{}r@{}}\textbf{document}\\\textbf{tokens}\end{tabular}} & \textbf{questions} & \textbf{0.8B} & \textbf{2B} & \textbf{4B} & \textbf{9B} & \textbf{27B} \\
\midrule
\endhead
\bottomrule
\endfoot
316 & 1 & 140 & 119 & 72 & 53 & 18.0 \\
316 & 2 & 182 & 161 & 86 & 61 & 19.7 \\
316 & 4 & 220 & 188 & 96 & 64 & 19.8 \\
316 & 8 & 104 & 156 & 99 & 67 & 22.8 \\
316 & 16 & 262 & 208 & 112 & 73 & 23.1 \\
316 & 64 & 366 & 243 & 116 & 73 & 23.2 \\
316 & 256 & 370 & 241 & 113 & 72 & 22.9 \\
316 & 1,024 & 356 & 232 & 111 & 71 & 22.7 \\
1,099 & 1 & 83 & 60 & 31 & 20.3 & 6.6 \\
1,099 & 2 & 45 & 44 & 34 & 23.6 & 7.6 \\
1,099 & 4 & 80 & 72 & 37 & 24.7 & 7.7 \\
1,099 & 8 & 116 & 80 & 39 & 24.8 & 7.9 \\
1,099 & 16 & 123 & 83 & 40 & 25.1 & 8.0 \\
1,099 & 64 & 129 & 84 & 40 & 25.0 & 7.9 \\
1,099 & 256 & 127 & 83 & 39 & 25.0 & 7.9 \\
1,099 & 1,024 & 126 & 83 & 39 & 25.1 & 8.0 \\
3,217 & 1 & 35 & 24.8 & 11.6 & 7.7 & 2.4 \\
3,217 & 2 & 38 & 27.1 & 12.9 & 8.6 & 2.8 \\
3,217 & 4 & 42 & 28.4 & 13.4 & 8.7 & 2.8 \\
3,217 & 8 & 44 & 29.0 & 13.4 & 8.7 & 2.8 \\
3,217 & 16 & 44 & 29.2 & 13.4 & 8.6 & 2.8 \\
3,217 & 64 & 44 & 28.9 & 13.3 & 8.6 & 2.8 \\
3,217 & 256 & 44 & 28.7 & 13.3 & 8.6 & -- \\
3,217 & 1,024 & 43 & 28.5 & 13.3 & 8.6 & -- \\
6,077 & 1 & 17.1 & 12.8 & 6.1 & 4.1 & 1.3 \\
6,077 & 2 & 18.5 & 17.6 & 10.5 & 7.9 & -- \\
6,077 & 4 & 30 & 29.6 & 19.2 & 14.4 & 5.6 \\
6,077 & 8 & 44 & 45 & 32 & 24.5 & -- \\
6,077 & 16 & 56 & 60 & 47 & 35 & 16.8 \\
6,077 & 64 & 69 & 76 & 63 & 51 & 31 \\
6,077 & 256 & 74 & 78 & 67 & 57 & 37 \\
6,077 & 1,024 & 74 & 76 & 62 & 58 & 39 \\
16,038 & 1 & 6.3 & 4.7 & 2.2 & 1.6 & 0.5 \\
16,038 & 2 & 11.2 & 8.8 & 4.8 & 3.3 & -- \\
16,038 & 4 & 16.5 & 13.8 & 7.6 & 5.5 & 1.9 \\
16,038 & 8 & 20.8 & 17.9 & 10.5 & 8.2 & -- \\
16,038 & 16 & 23.4 & 20.9 & 12.9 & 10.4 & 4.3 \\
16,038 & 64 & 25.9 & 23.7 & 15.6 & 13.6 & 6.1 \\
16,038 & 256 & 26.1 & 24.2 & 16.5 & 14.5 & 6.8 \\
16,038 & 1,024 & 25.5 & 23.7 & 16.7 & 14.5 & 7.0 \\
64,217 & 1 & 1.5 & 1.2 & 0.5 & 0.4 & -- \\
64,217 & 2 & 2.6 & 2.0 & 1.0 & 0.7 & -- \\
64,217 & 4 & 3.9 & 3.3 & 1.7 & 1.3 & -- \\
64,217 & 8 & 5.3 & 4.6 & 2.7 & 2.2 & -- \\
64,217 & 16 & 6.4 & 5.8 & 3.9 & 3.2 & -- \\
64,217 & 64 & 7.5 & 7.2 & 5.7 & 5.4 & -- \\
64,217 & 256 & 7.8 & 7.6 & 6.5 & 6.5 & -- \\
64,217 & 1,024 & 7.6 & 7.7 & 6.7 & 6.8 & -- \\
\end{longtable}
\endgroup

\begin{table}[!htbp]
\renewcommand{\thetable}{J.7}
\centering
\caption{The same with the document shared from 256 tokens.}\label{tab:J.7}
{\small\setlength{\tabcolsep}{6pt}\renewcommand{\arraystretch}{1.1}
\noindent\begin{adjustbox}{max width=\linewidth}
\begin{tabular}{rrrrrrr}
\toprule
{\begin{tabular}[b]{@{}r@{}}\textbf{document}\\\textbf{tokens}\end{tabular}} & \textbf{questions} & \textbf{0.8B} & \textbf{2B} & \textbf{4B} & \textbf{9B} & \textbf{27B} \\
\midrule
316 & 1 & 153 & 124 & 73 & 53 & 17.8 \\
316 & 2 & 225 & 169 & 89 & 62 & 19.7 \\
316 & 4 & 281 & 201 & 100 & 65 & 20.0 \\
316 & 8 & 90 & 88 & 70 & 69 & 28.7 \\
316 & 16 & 165 & 165 & 116 & 95 & 36 \\
316 & 64 & 358 & 295 & 173 & 128 & 44 \\
316 & 256 & 436 & 357 & 195 & 138 & 47 \\
316 & 1,024 & 454 & 366 & 198 & 138 & 47 \\
1,099 & 1 & 85 & 62 & 31 & 20.5 & 6.5 \\
1,099 & 2 & 22.0 & 23.0 & 17.8 & 17.7 & 8.9 \\
1,099 & 4 & 42 & 44 & 34 & 34 & 17.4 \\
1,099 & 8 & 78 & 80 & 63 & 63 & 27.0 \\
1,099 & 16 & 128 & 135 & 100 & 84 & 34 \\
1,099 & 64 & 229 & 214 & 139 & 110 & 41 \\
1,099 & 256 & 266 & 241 & 154 & 116 & 43 \\
1,099 & 1,024 & 268 & 242 & 154 & 115 & 44 \\
3,217 & 1 & 36 & 25.3 & 11.7 & 7.9 & 2.4 \\
3,217 & 2 & 20.6 & 21.3 & 15.8 & 12.3 & 4.6 \\
3,217 & 4 & 37 & 38 & 29.3 & 23.1 & 9.1 \\
3,217 & 8 & 61 & 63 & 50 & 40 & 15.1 \\
3,217 & 16 & 90 & 93 & 72 & 55 & 21.8 \\
3,217 & 64 & 130 & 125 & 94 & 76 & 32 \\
3,217 & 256 & 141 & 135 & 101 & 82 & 36 \\
3,217 & 1,024 & 136 & 129 & 99 & 81 & 36 \\
\bottomrule
\end{tabular}
\end{adjustbox}\par}
\end{table}

The largest difference between a probability read in a request with many questions and the same
question read alone is 0.0078 (0.8B), 0.0046 (2B), 0.0049 (4B), 0.0039 (9B) and 0.0023 (27B) in the
runs of Table~\ref{tab:J.6}.

\begin{table}[!htbp]
\renewcommand{\thetable}{J.8}
\centering
\caption{Peak GPU memory of the process in the runs of Table~\ref{tab:J.6}, in GiB (weights, recorded graphs and the activations of the largest batch).}\label{tab:J.8}
{\small\setlength{\tabcolsep}{6pt}\renewcommand{\arraystretch}{1.1}
\noindent\begin{adjustbox}{max width=\linewidth}
\begin{tabular}{rrrrrr}
\toprule
{\begin{tabular}[b]{@{}r@{}}\textbf{document}\\\textbf{tokens}\end{tabular}} & \textbf{0.8B} & \textbf{2B} & \textbf{4B} & \textbf{9B} & \textbf{27B} \\
\midrule
316 & 6.99 & 9.72 & 17.75 & 27.53 & 64.96 \\
6,077 & 12.48 & 15.00 & 34.89 & 43.92 & 127.95 \\
64,217 & 9.14 & 11.75 & 23.34 & 32.93 & -- \\
\bottomrule
\end{tabular}
\end{adjustbox}\par}
\end{table}

\subsection{Load test and numerics by batch shape}\label{sec:J.8}

In a closed-loop load test of the three-question request with one server per GPU on a node of eight
H200s (2026-10-01), the released server, which answers one request at a time per GPU, reached 81
requests per second with the 27B and 170 with the 35B-A3B. A test server that batches across
requests reached 87 and 316. At 64 rows per forward pass the GPU cost per row was 30.5 ms for the
27B and 7.6 ms for the 35B-A3B: the 27B is bound by compute already at one request, the mixture of
experts by reading its weights at small batches. Probabilities shift slightly with the composition
of a batch in bf16: on 512 development rows by at most 0.04 for the 27B, with one changed choice,
and by at most 0.15 for the 35B-A3B, with two. Repeated runs of the same batches are identical.

A measurement pitfall belongs here. A test server that writes the response headers and the body in
two writes over a kept-alive connection adds 41 ms to every request, because small-packet coalescing
meets delayed acknowledgement. The server-side times of that first run were correct (99 and 50 ms
for the 27B). The latencies of Table~\ref{tab:8.1} are from the released server.
